# Supplementary material for: Standard Gaussian Process is All You Need for High-Dimensional Bayesian Optimization
Source: arXiv:2402.02746 source file (2025-03-11)
Supplement: Supplementary file 1 [file appendix-zhe.tex]

\section{Proofs}\label{sect:proof}
\subsection{Proof of Lemma~\ref{lem:tau-se} }
\begin{proof}
    We intend to solve $\rho^2/e^{\rho^2} < \xi$, which is equivalent to solving
    \[
     \log r - r < \log \xi, 
    \]
    where $r = \rho^2$. 
    We then leverage the fact that $\log r < \sqrt{r}$ when $r > 1$. Since $1/e > \xi$, we know the solution of $\rho$ must be larger than 1, implying that the solution for $r$ is larger than $1$. To meet the inequality, we can solve 
    \[
    \log r - r < \sqrt{r} - r < \log \xi. 
    \]
    It then converts to a quadratic form, 
    \begin{align}
        \sqrt{r} - \sqrt{r}^2 < \log \xi.
    \end{align}
    Note that $\rho = \sqrt{r}$.     It is straightforward to solve this inequality and we can obtain that the inequality holds when
    \[
    \rho > \tau_{\text{SE}} = \frac{1}{2} + \sqrt{\frac{1}{4} - \log \xi}. 
    \]
    
\end{proof}
\subsection{Proof of Lemma~\ref{lem:prob-bound}}\label{sect:bound-proof-1}
\begin{proof}
    First, since each $x_{ik}$ and $x_{jk}$ independently follow $\text{Uniform}(0, 1)$, it is straightforward to obtain $\EE[(x_{ik} - x_{jk})^2] = \frac{1}{6}$. 
    Let us define $\gamma = \|\x_i - \x_j\|^2$. Then we have $\EE[\gamma] = \frac{1}{6}d$.
    According to Hoeffding's inequality,  for all $t>0$,
    \begin{align}
        p(|\gamma - \frac{1}{6}d| \ge t) \le  2\exp\left(-\frac{2t^2}{d}\right). \label{eq:hoeff}
    \end{align}
    Since $\rho = 
    \frac{\sqrt{\gamma}}{\ell_0}$, we have  $p(\rho > \tau) = p(\gamma > \tau^2\ell_0^2)$. Since $d>6\ell_0^2\tau^2$, we set $t = \frac{1}{6}d - \ell_0^2\tau^2>0$, and apply \eqref{eq:hoeff} to obtain
    \[
    p(|\gamma - \frac{1}{6}d| \ge \frac{1}{6}d -  \ell_0^2\tau^2|) \le 2\exp\left(-\frac{2\left(\frac{1}{6}d -  \ell_0^2\tau^2\right)^2}{d}\right)
      = 2 \exp\left(-\frac{\left(d - 6\ell_0^2\tau^2\right)^2}{18d}\right),
    \]
    which is equivalent to
    \begin{align}
        p(|\gamma-\frac{1}{6}d| < \frac{1}{6}d - \ell_0^2\tau^2) > 1 - 2 \exp\left(-\frac{\left(d - 6\ell_0^2\tau^2\right)^2}{18d}\right).\label{eq:bound2}
    \end{align}
Since $p(\gamma > \ell_0^2 \tau^2) \ge p( \ell_0^2 \tau^2 < \gamma < \frac{1}{3}d - \ell_0^2 \tau^2) = 
p(|\gamma - \frac{1}{6}d| < \frac{1}{6}d - \ell_0^2\tau^2)$, combining with \eqref{eq:bound2} we obtain the bound
\[
p(\rho>\tau) = p(\gamma > \ell_0^2 \tau^2) > 1 - 2 \exp\left(-\frac{\left(d - 6\ell_0^2\tau^2\right)^2}{18d}\right).
\]
\end{proof}

\subsection{Proof of Lemma~\ref{lem:tau-matern}}
\begin{proof}
    To solve $\rho^2/e^{\sqrt{5}\rho} < \xi$, it is equivalent to solving
    \[
    \frac{1}{5} \frac{r^2}{e^r} < \xi, \;\;\; r = \sqrt{5}\rho,
    \]
    which is further equivalent to 
    \[
    \log \frac{1}{5} + 2 \log r - r < \log \xi. 
    \]
    We leverage $\log r < \sqrt{r}$ for $r>1$, and solve the upper bound, 
    \[
    \log\frac{1}{5} + 2 \sqrt{r}-r < \log \xi,
    \]
    which gives 
    \begin{align}
        \rho > \tau_{\text{Mat\'ern}} = \frac{1}{\sqrt{5}}\left(1 + \sqrt{1 + \log 1/5 - \log\xi}\right)^2.
    \end{align}
\end{proof}

\subsection{Proof of Lemma~\ref{lem:new-bound}}
\begin{proof}
    First, similar to the proof in Section~\ref{sect:bound-proof-1}, under the uniform distribution on $[0, 1]^d$, from Hoeffding's inequality, we have for all $t>0$,
        \begin{align}
        p(|\gamma - \frac{1}{6}d| \ge t) \le  2\exp\left(-\frac{2t^2}{d}\right). \label{eq:hoeff-again}
    \end{align}

    When we set $\ell_0 = c\sqrt{d}$ such that $c>1/ \sqrt{6}\tau$, we have $\ell_0^2 \tau^2 > d/6 $. Let us choose $t = \ell_0^2\tau^2 - d/6=c^2 \tau^2d - d/6>0$, and apply the Hoeffding's inequality~\eqref{eq:hoeff-again}, 
    \begin{align}
        p\left(|\gamma - d/6 | \ge \ell_0^2\tau^2 - d/6\right) \le 
        2\exp\left(-\frac{2(\ell_0^2\tau^2 - d/6)^2}{d}\right) = 2\exp\left(-2(c^2\tau^2 - \frac{1}{6})^2d\right)
    \end{align}
    Since $p(\rho \ge \tau) = p(\gamma \ge \ell_0^2\tau^2) \le p(|\gamma - d/6 | \ge \ell_0^2\tau^2 - d/6)$, we obtain
    \[
    p(\rho \ge\tau) \le 2\exp\left(-2(c^2\tau^2 - \frac{1}{6})^2d\right).
    \]
\end{proof}

\section{More Experiment Details}
\subsection{Definition of Synthetic Functions}\label{sect:syn-def}
%We denote the function forms and bounds we used in Sec \ref{sec:experiments} below.

\textbf{Stybtang}. We used the following slightly-modified Stybtang function, %The original Stybtang is in form $f(x)=\frac{1}{2}\sum_{i=1}^{D}(x_{i}^{4}-16x_{i}^{2}+5x_{i})$. Our version $f_{\text{V1}}$ is of form,
\[
f(\x)=\frac{1}{2}\sum_{i=1}^{D}\left((x_{i}-c_{i})^{4}-16(x_{i}-c_{i})^{2}+5(x_{i}-c_{i})\right),
\]
where $\x \in [-5, 5]^D$, and we set $[c_1, \dots, c_D]$ as an evenly spaced sequence in $[0, 7.5]$ ($c_1 = 0$ and $c_D = 7.5$). The optimum  is at $\x^\dagger=[c_1 -2.903534, \ldots, c_D - 2.903534]$.

\textbf{Rosenbrock}. 
We used the following Rosenbrock function, 
\[
f(\x)=\sum_{i=1}^{D-1}\left[100\left((x_{i+1}-c_{i+1})-(x_{i}-c_{i})^{2}\right)^{2}+\left(1 - (x_{i}-c_{i})\right)^2\right],
\]
where $\x \in [-2.048, 2.048]^{D}$. We set $[c_{1}, ..., c_D]$ as an evenly spaced sequence in $[-2, 2]$, where $c_{1}=-2$ and  $c_{D}=2$. The optimum is at $x^\dagger =  [c_{1}+1, ..., c_{D}+1]$. 

\textbf{Ackley}. We used the Ackley function defined in~\citep{simulationlib},
\[
f(\x)=-20\text{ exp}\left(-0.2\sqrt{\frac{1}{d}\sum_{i=1}^{d}x_{i}^{2}}\right)-\text{exp}\left(\frac{1}{d}\sum_{i=1}^{d}\text{cos}(2{\pi}x_{i})\right)+20+\text{exp}(1),
\]
where each $x_i \in [-32.768, 32.768]$ and the (global) optimum is at $x^{\dagger}=[0, \ldots, 0]$. 

\textbf{Hartmann6}. The function is given by
\[
f(\x)=-\sum_{i=1}^{4}{\alpha}_{i}{ \exp}\left(-\sum_{j=1}^{6}A_{ij}(x_{j}-P_{ij})^{2}\right),
\]
where each $x_i \in [0, 1]$, $\A=[A_{ij}]$ and $\P = [P_{ij}]$ are two pre-defined matrices as in \citep{simulationlib}.
The global optimum is at $\x^\dagger = [0.20169, 0.150011, 0.476874, 0.275332, 0.6573]$.

\begin{figure*}[!ht]
    \centering
    \includegraphics[width=\textwidth]{BO ICLR 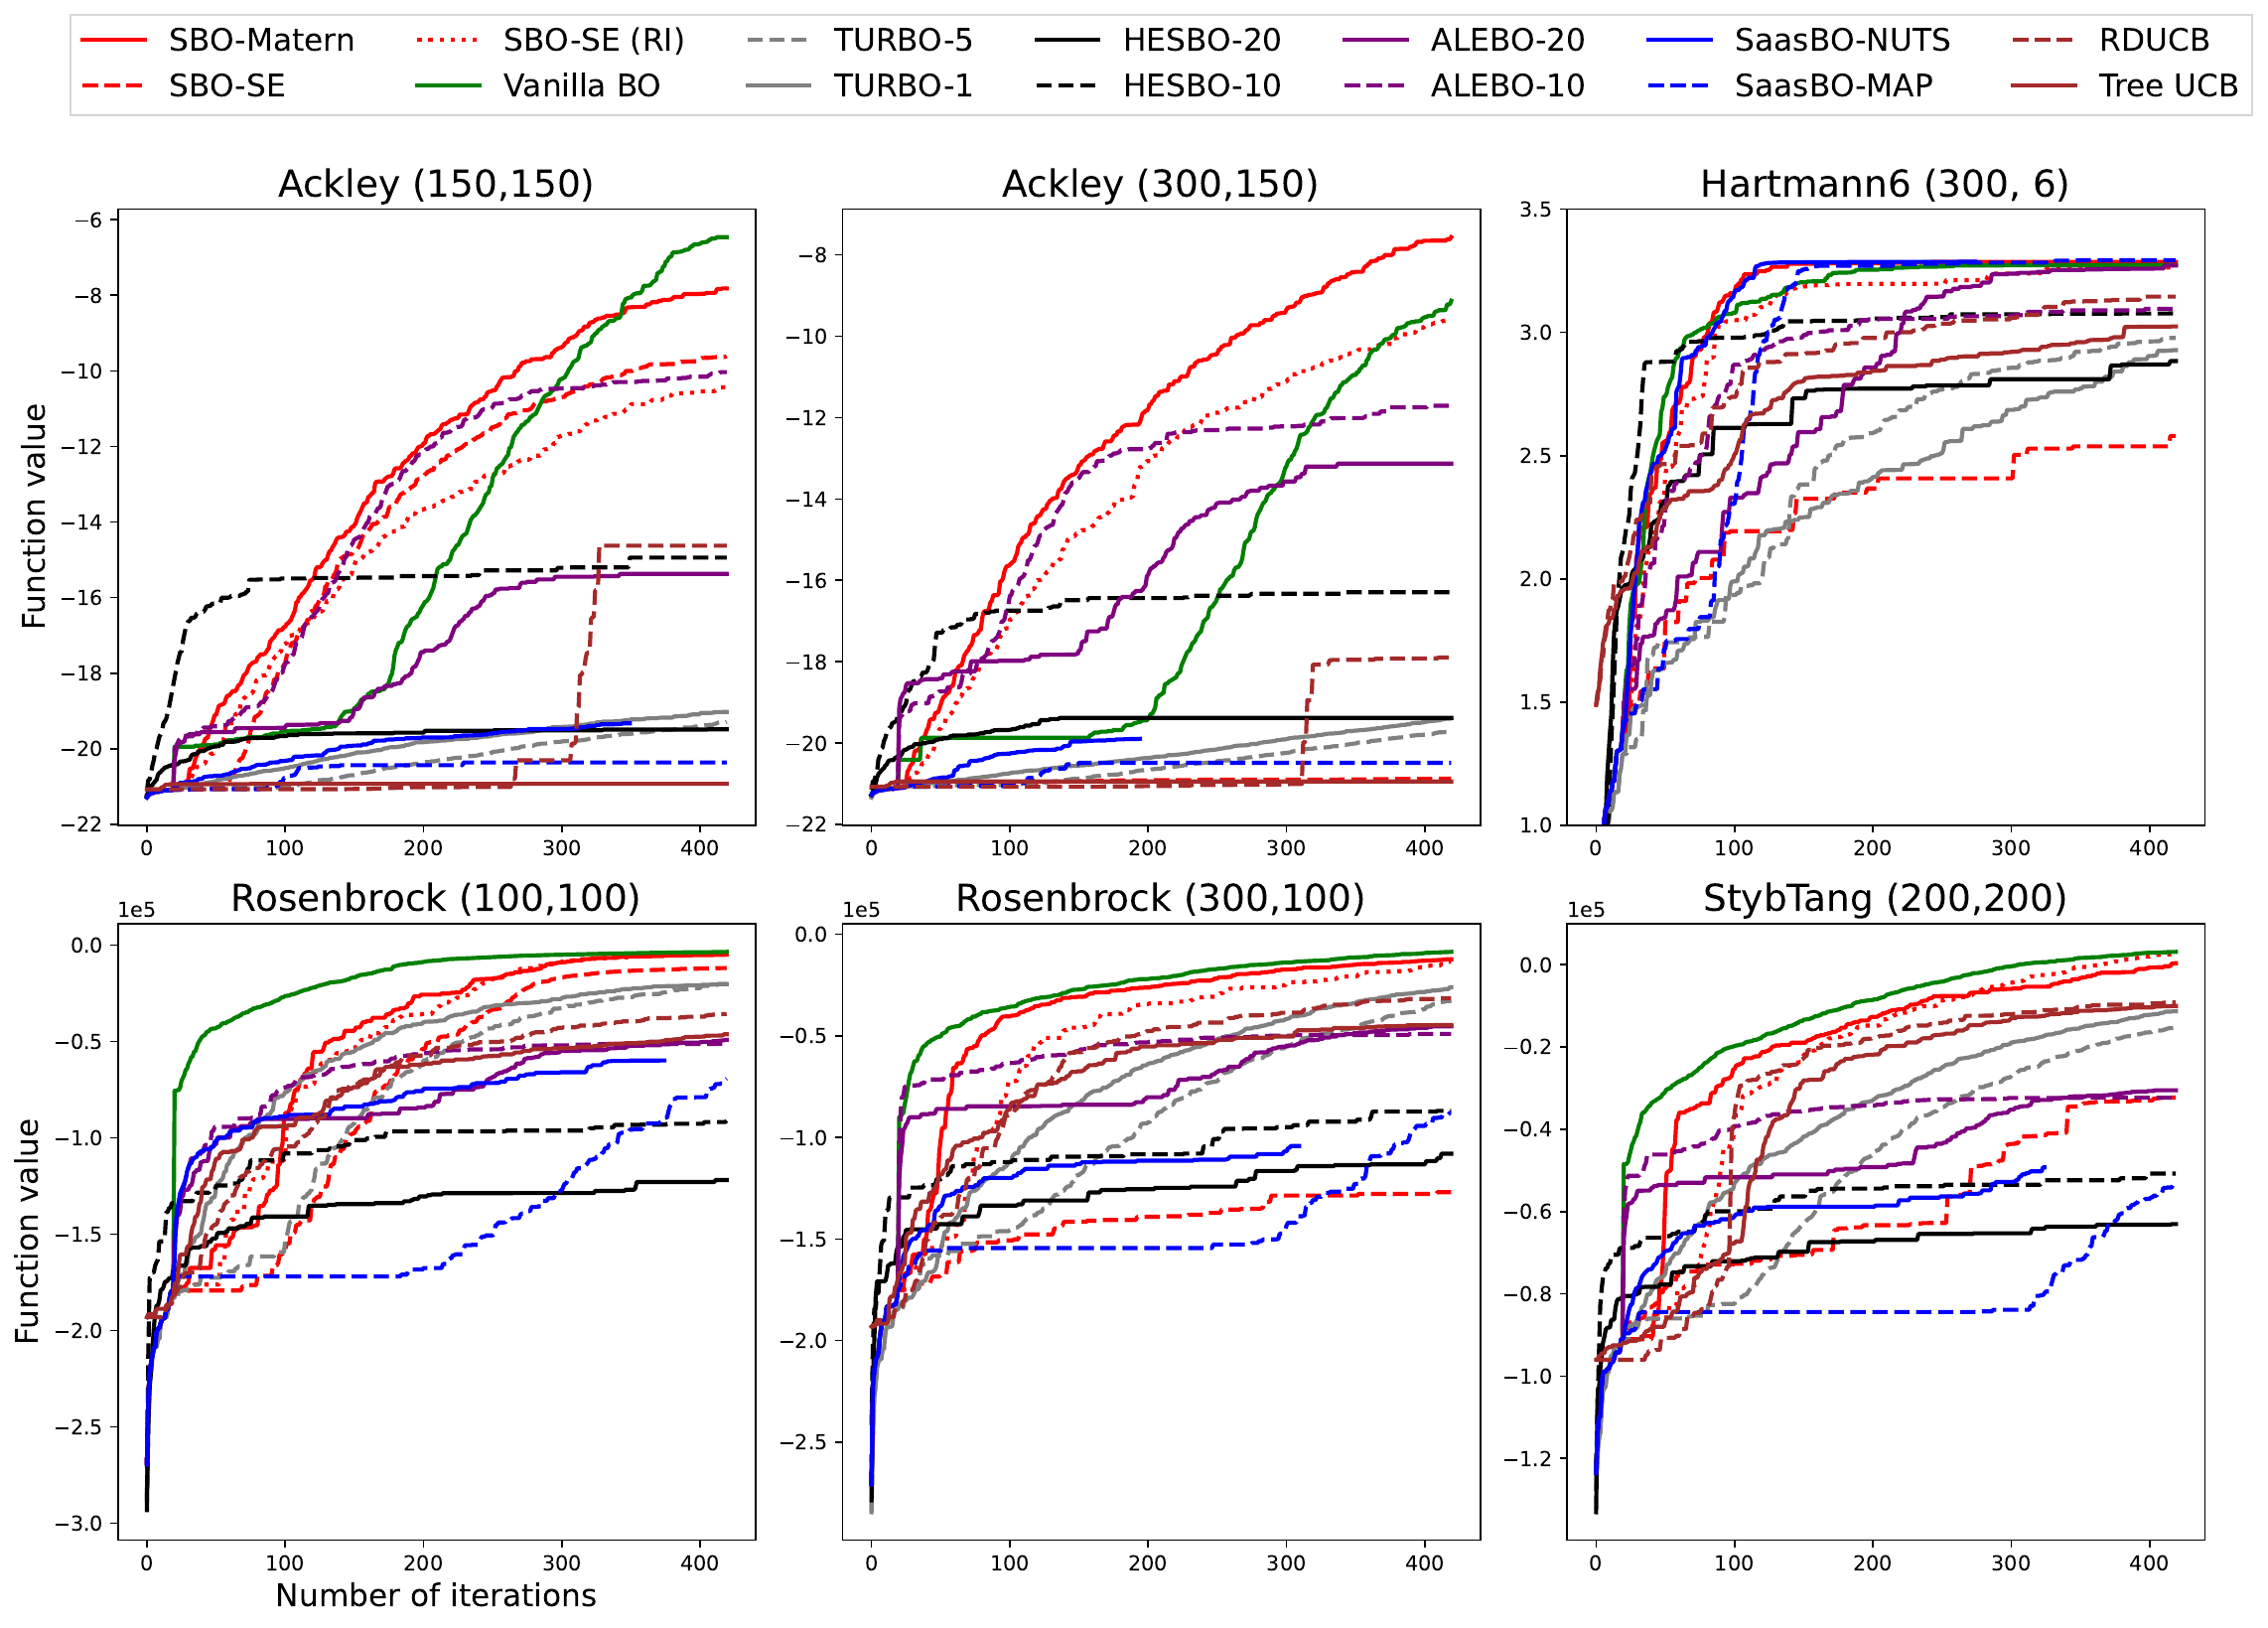}
    \caption{\small Runtime performance: Maximum Function Value Obtained \textit{vs.} Number of Steps in synthetic benchmarks. The results were averaged from 10 runs. \zhec{comment out} }
    \label{fig:syn-running-plot}
\end{figure*}

\begin{figure*}[!ht]
    \centering
    \includegraphics[width=\textwidth]{BO ICLR 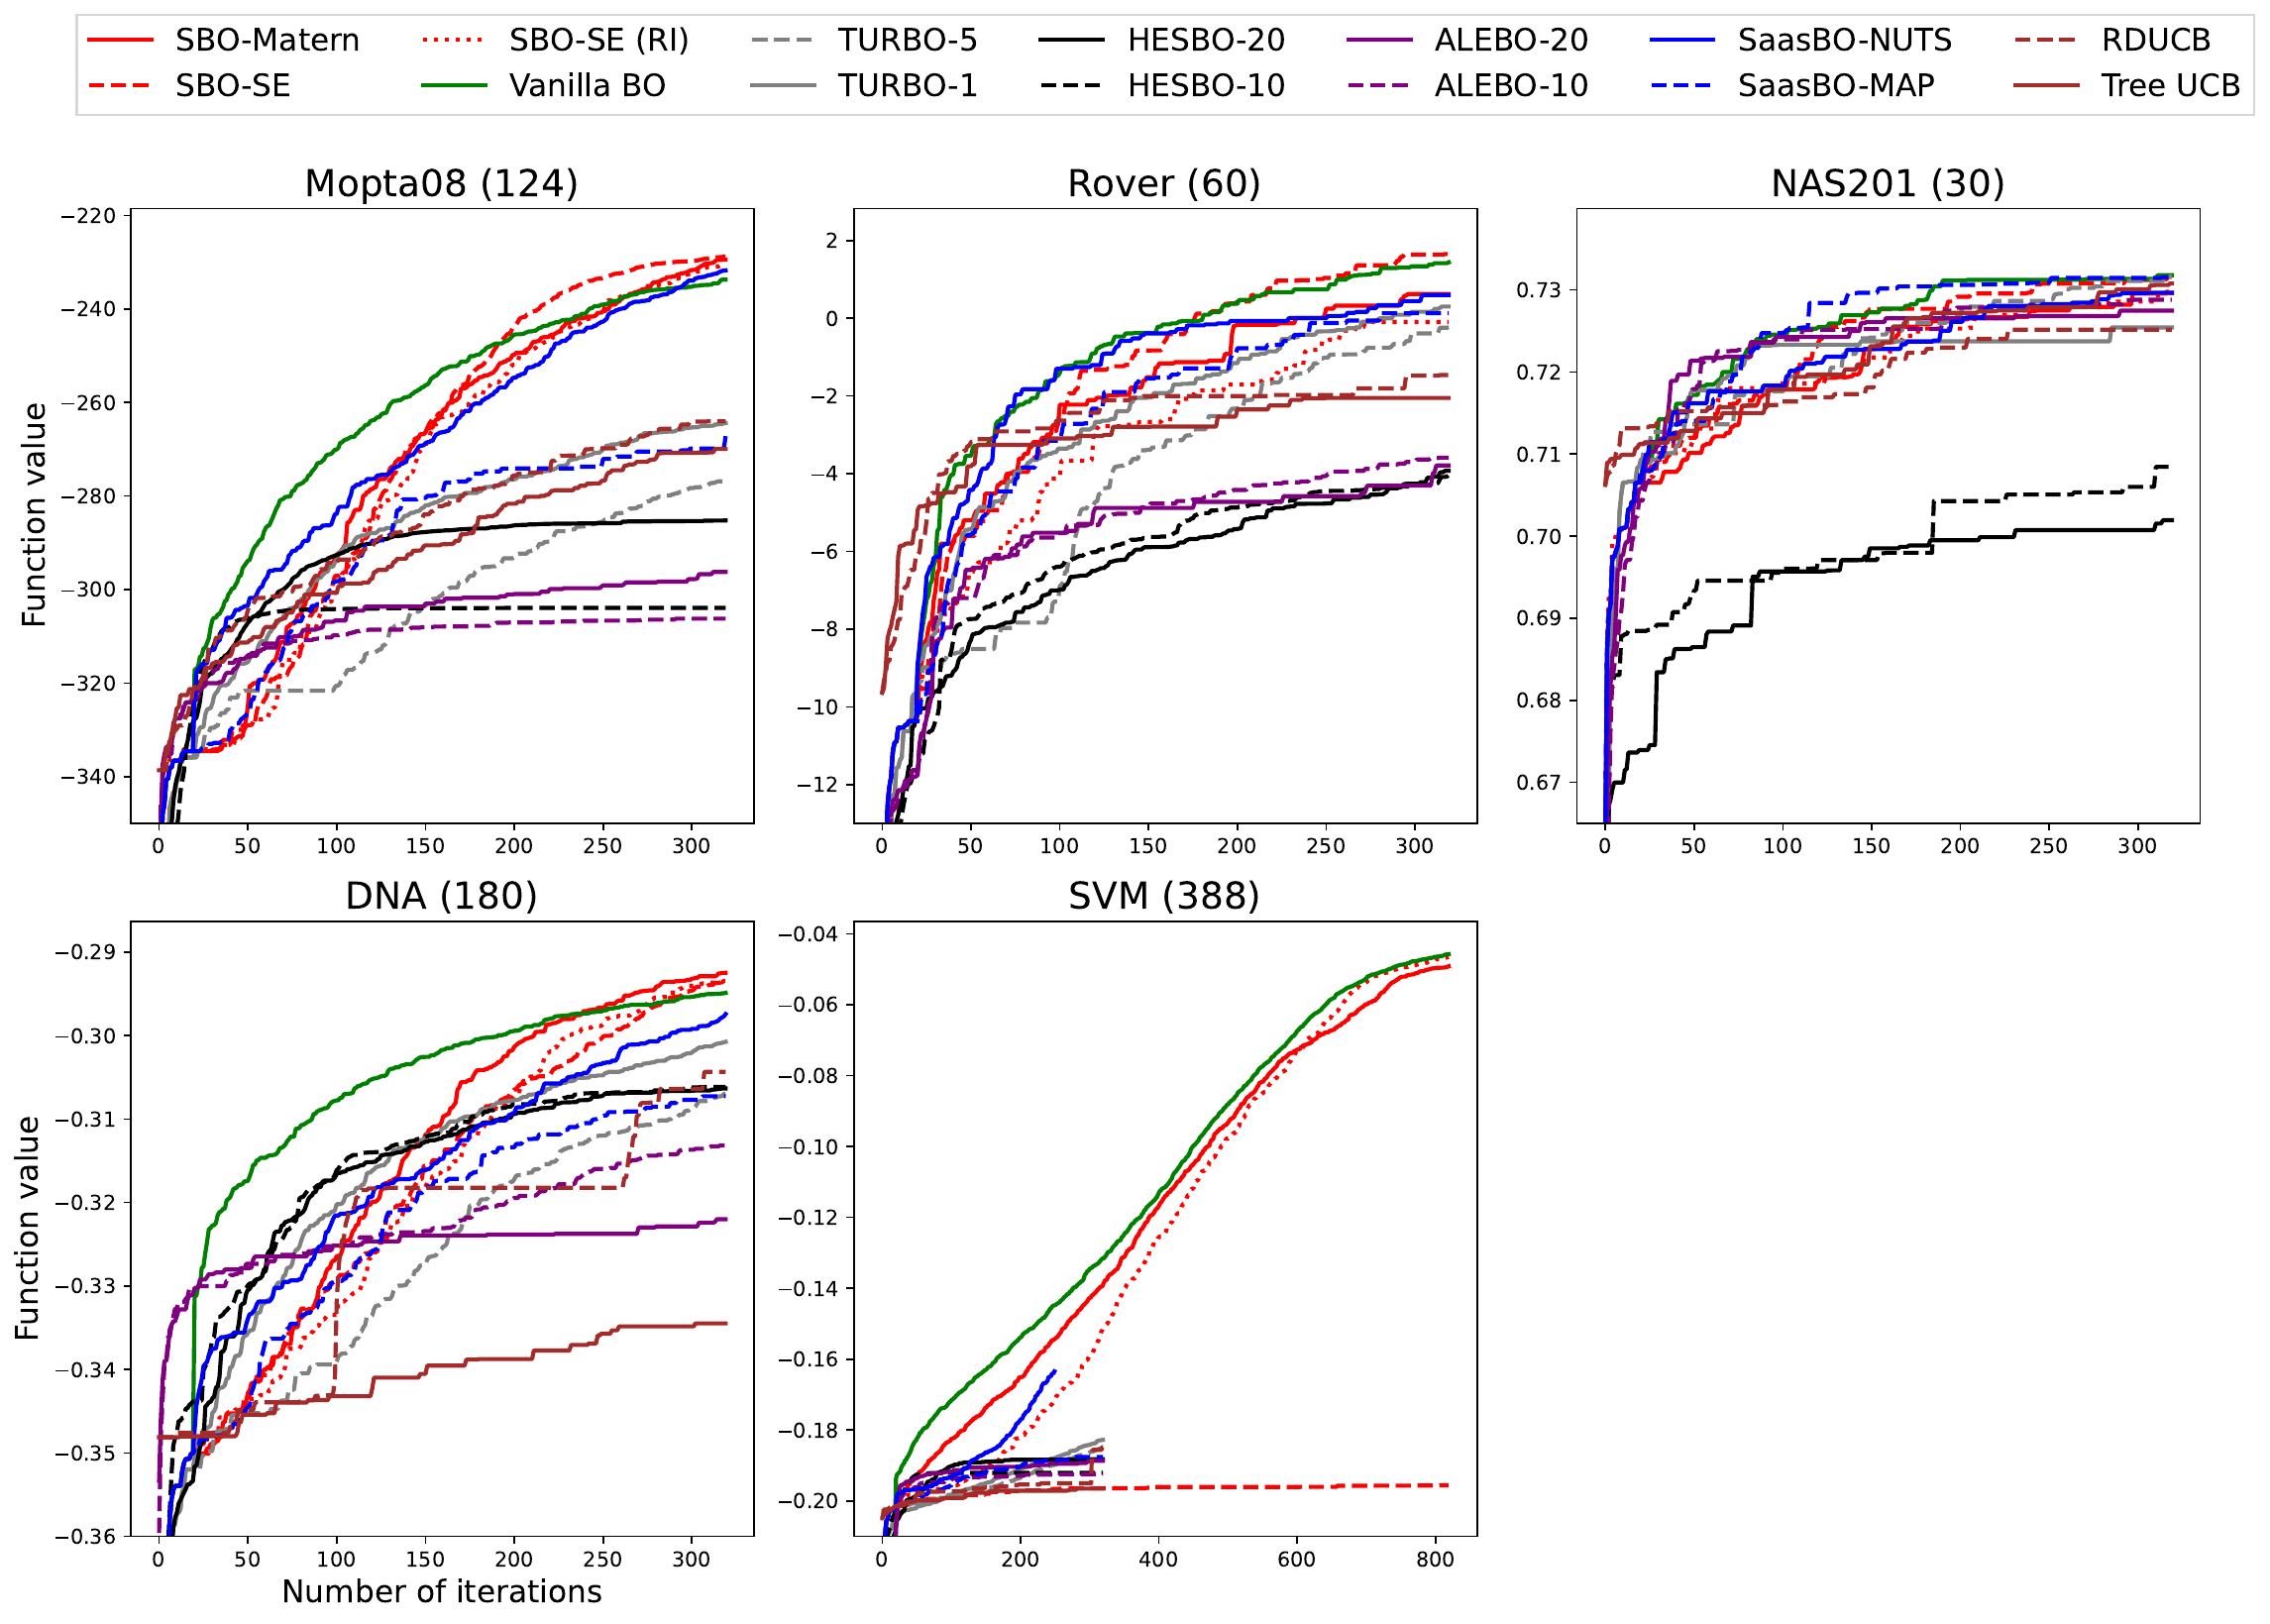}
    \caption{\small Runtime performance: Maximum Function Value Obtained \textit{vs.} Number of Steps in real-world benchmarks. The results were averaged from 10 runs. \zhec{need to discard; replace with a single running plot with standard eror bars}}
    \label{fig:running-real}
\end{figure*}

\begin{figure*}[!ht]
    \centering
    \includegraphics[width=\textwidth]{BO ICLR 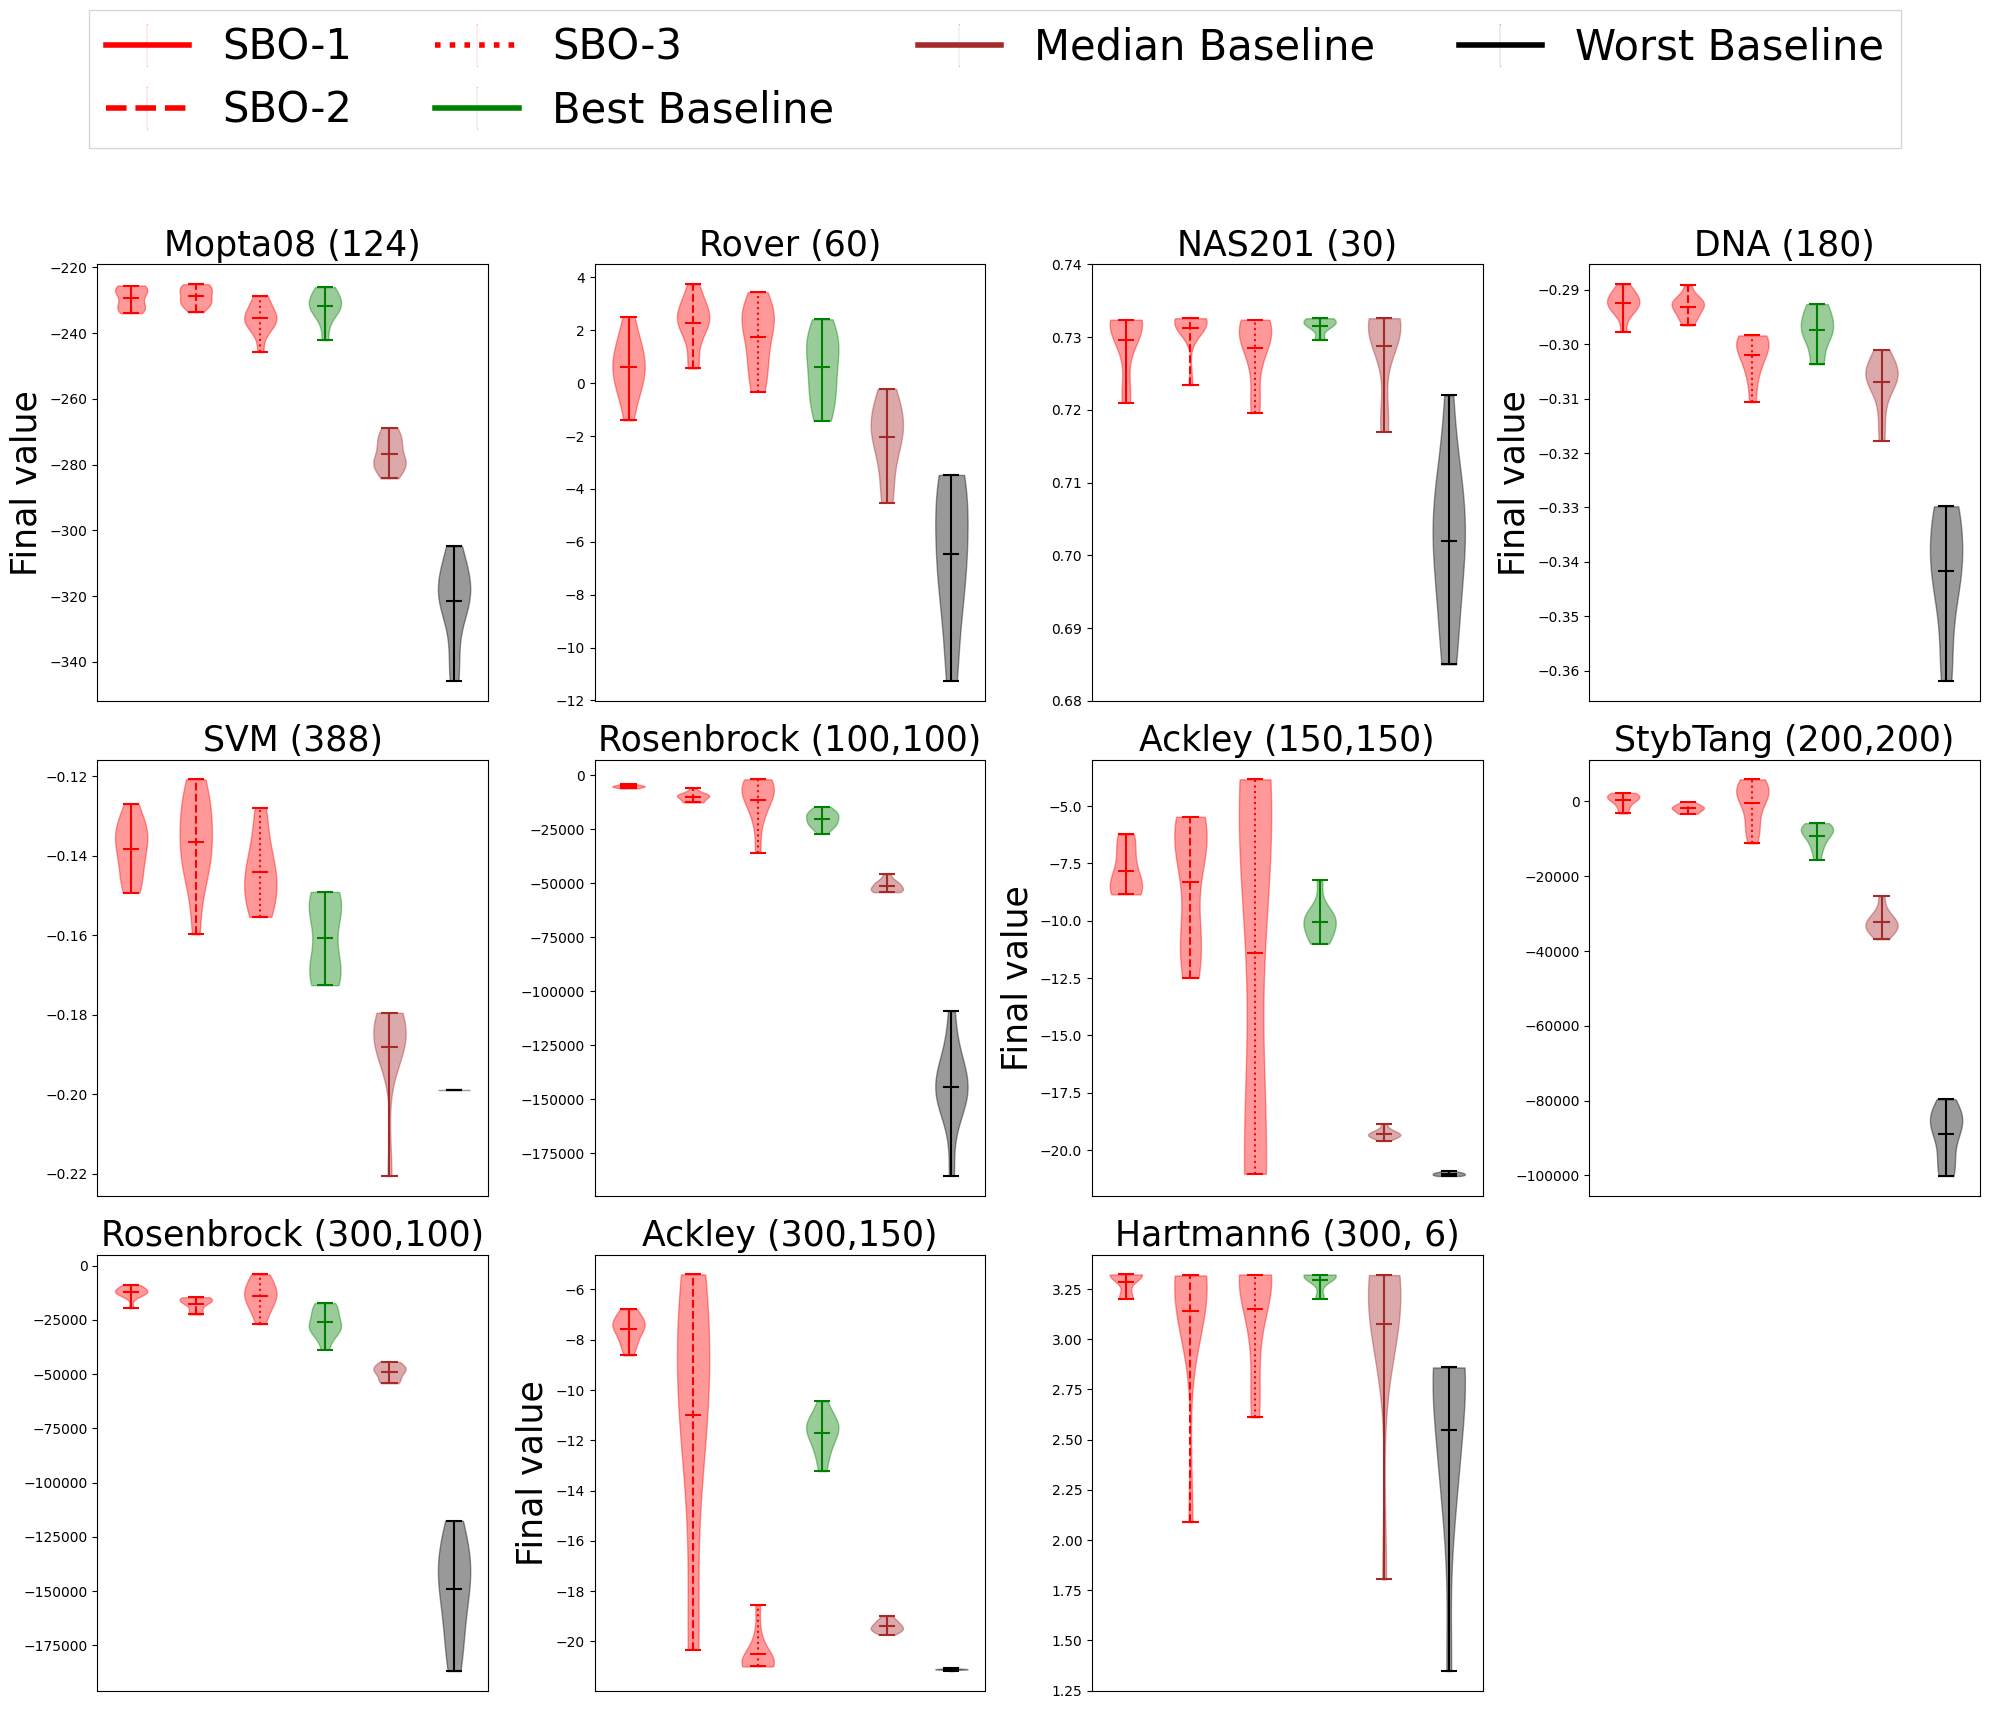}
    \caption{\small Ultimate optimization performance: Maximum Function Value obtained at the end of optimization loop, including SBO-3, namely training with a single length-scale parameter in Mat\'ern-5/2 kernel. The results were collect from 10 runs.}
    \label{fig:final-all-sbo3}
\end{figure*}
\begin{figure*}[!ht]
    \centering
    \includegraphics[width=\textwidth]{BO ICLR 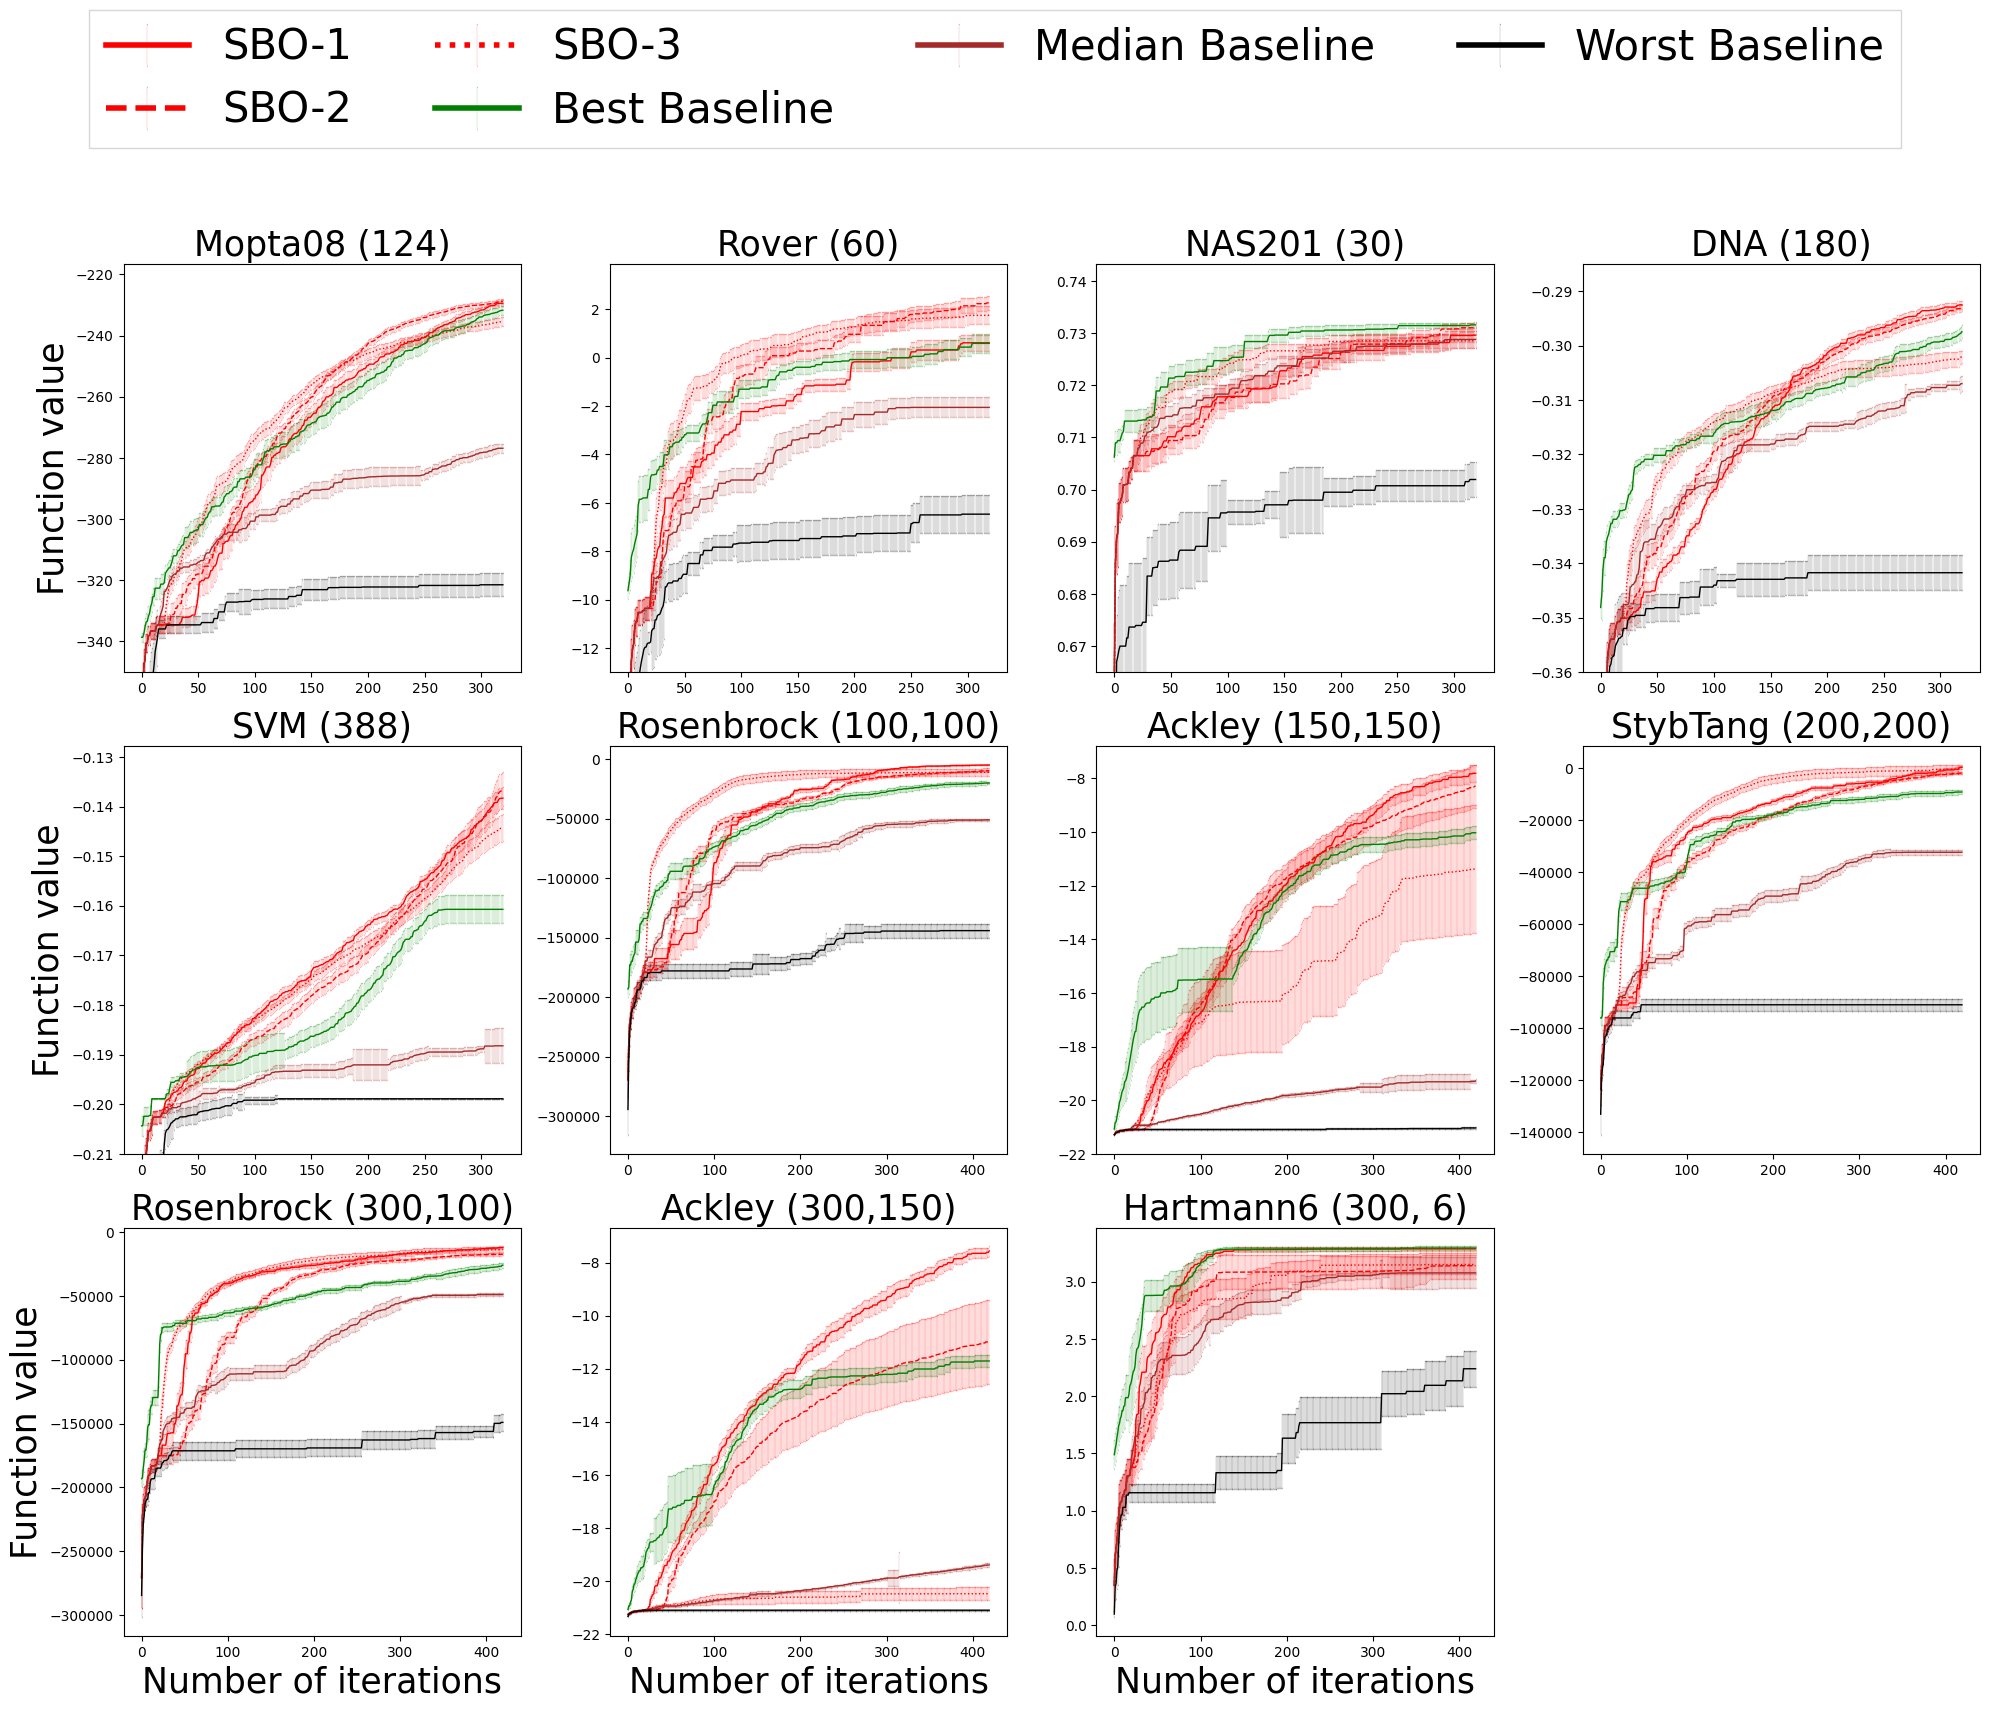}
    \caption{\small Runtime performance: Maximum Function Value obtained \textit{vs.} Number of Steps in real-world benchmarks, including SBO-3, namely training with a single length-scale parameter in Mat\'ern-5/2 kernel. The results were averaged from 10 runs. The shaded region depicts the standard deviation. }
    \label{fig:running-all-with-std-sbo3}
\end{figure*}

\subsection{Implementation}\label{sect:impl}
\begin{itemize}
    \item \textbf{ALEBO.} We used ALEBO implementation shared by the  Adaptive Experimentation (AX) Platform  (version 0.2.2). The source code is at  \url{https://github.com/facebook/Ax/blob/main/ax/models/torch/alebo.py}.
    \item \textbf{HESBO.} We used HESBO implementation of the original authors (\url{https://github.com/aminnayebi/HesBO}).
    \item \textbf{TURBO.} We used the original TURBO implementation (\url{https://github.com/uber-research/TuRBO})
    \item \textbf{SaasBO-NUTS.} We used the original implementation of the authors  (\url{https://github.com/martinjankowiak/saasbo}). %and the re-implementation in BoTorch. The original implementation yield better result, but with a higher runtime. All reported experiment results is from original implementation.
    \item \textbf{SaasBO-MAP.} The SaasBO implementation available to the public does not include the version using MAP estimation.  We therefore implemented this method based on the original paper~\citep{eriksson2021highdimensional}. All the hyperparameter settings follow exactly the same as the original paper.
    \item \textbf{RDUCB and Tree UCB.} The implementation of both methods is publicly available at \url{https://github.com/huawei-noah/HEBO/tree/master/RDUCB}.
    \item \textbf{BNN Laplace and BNN HMC.} {For BNN Laplace, we used the implementation at \url{https://github.com/wiseodd/laplace-bayesopt}, and for BNN HMC, we used the implementation at \url{https://github.com/yucenli/bnn-bo}. To identify the architecture of the neural network, we perform leave-one-out cross-validation on the initial dataset for each task. The layer width and depth were selected from \{1, 2, 3\} $\times$ \{32, 64, 128, 256\}. The activation function for BNN Laplace is ReLU and for BNN HMC is Tanh, which is the default choice of each method. For BNN Laplace, the training was conducted by maximizing marginal likelihood with ADAM, with learning rate of 1E-01, and weight decay of 1E-03. For HMC, the BNN is pre-trained by maximizing log likelihood with ADAM. Then followed by HMC sampling procedure. We used their adaptive step size schedule for the Leap frog, and the number of steps was set to 100.}
\end{itemize}

\subsection{Computing Environment}
\label{sect:compute-env}
We conducted the experimental investigations on a large computer cluster equipped with Intel Cascade Lake Platinum 8268 chips.

\begin{table*}[h!]
\small
\centering
\begin{tabular}{lrrrrr}
\toprule
{} &  Mopta08 (124) &   Rover (60) &  NAS201 (30) &   DNA (180) &    SVM (388) \\
\midrule
{ARD Mat\'ern-MAP} &    7.39 &    9.99 &    7.81 &    9.77 &    13.55 \\
{ARD Mat\'ern-MLE} &    11.23 &    9.84 &    5.76 &    14.34 &    32.16 \\
{ARD Mat\'ern-NUTS}&    492.62 &   404.17  &   393.62  &   575.03  &   768.29\\
{SaasBO-MAP        } &    46.53 &   41.36 &   42.35 &    51.33 &    67.37 \\
{SaasBO-NUTS          } &   985.76 &  375.06 &  229.07 &  1739.56 &  2269.50 \\
\bottomrule
\end{tabular}
\caption{Average running time (in seconds) per optimization step in real-world benchmark tasks.}
\label{tb:real-runtime}
\end{table*}
\begin{table*}[h!]
\small
\centering
\begin{tabular}{lcccccc}
\toprule
    {} &  Rosenbrock &   Ackley &  Stybtang &  Rosenbrock &  Ackley &  Hartmann6 \\
     & (100,100) & (150, 150) & (200, 200) & (300, 100) & (300, 150) & (300, 6) \\
    \midrule
    {ARD Mat\'ern-MAP} &           8.52 &    36.26 &        21.42 &             16.36 &       25.90 &       51.56 \\
    {ARD Mat\'ern-MLE} &           8.85 &    12.94 &        13.67 &             12.63 &       9.99 &       8.81 \\
    {ARD Mat\'ern-NUTS} &   857.21  &   850.23  &   1120.28 &   1276.42 &   1049.78 &   948.25\\
    {SaasBO-MAP       } &          70.17 &    70.69 &        66.35 &            100.79 &      85.86 &      85.72 \\
    {SaasBO-NUTS            } &        1294.90 &  1621.60 &      1511.99 &           1938.53 &     925.80 &    2204.54 \\
\bottomrule
\end{tabular}
\caption{\small Average running time (in seconds) per optimization step on synthetic benchmark tasks.}
\label{tb:syn-runtime}
\end{table*}

%\begin{wraptable}{r}{0.55\textwidth}
\begin{table}
%\vspace{-0.15in}
\centering
\small
\begin{tabular}{c | c} 
\hline\hline
 \textit{Method} & \textit{Structural Assumption} \\
 \hline
   ALEBO, HESBO & {Low-dim embedding} \\ 
  %\hline
  SaasBO & Partial variable dependency\\ 
%\hline
 RDUCB, Tree UCB & Additive function decomposition \\
% \hline
  SBO, TURBO, BNN & None\\ \hline
\end{tabular}
\caption{\small BO methods and their structural assumption about the target function.} \label{tb:method-assumptions}
\label{table:1}
\end{table}
%\vspace{-0.1in}
%\end{wraptable}

\begin{figure}[H]
    \centering
    \includegraphics[width=\textwidth]{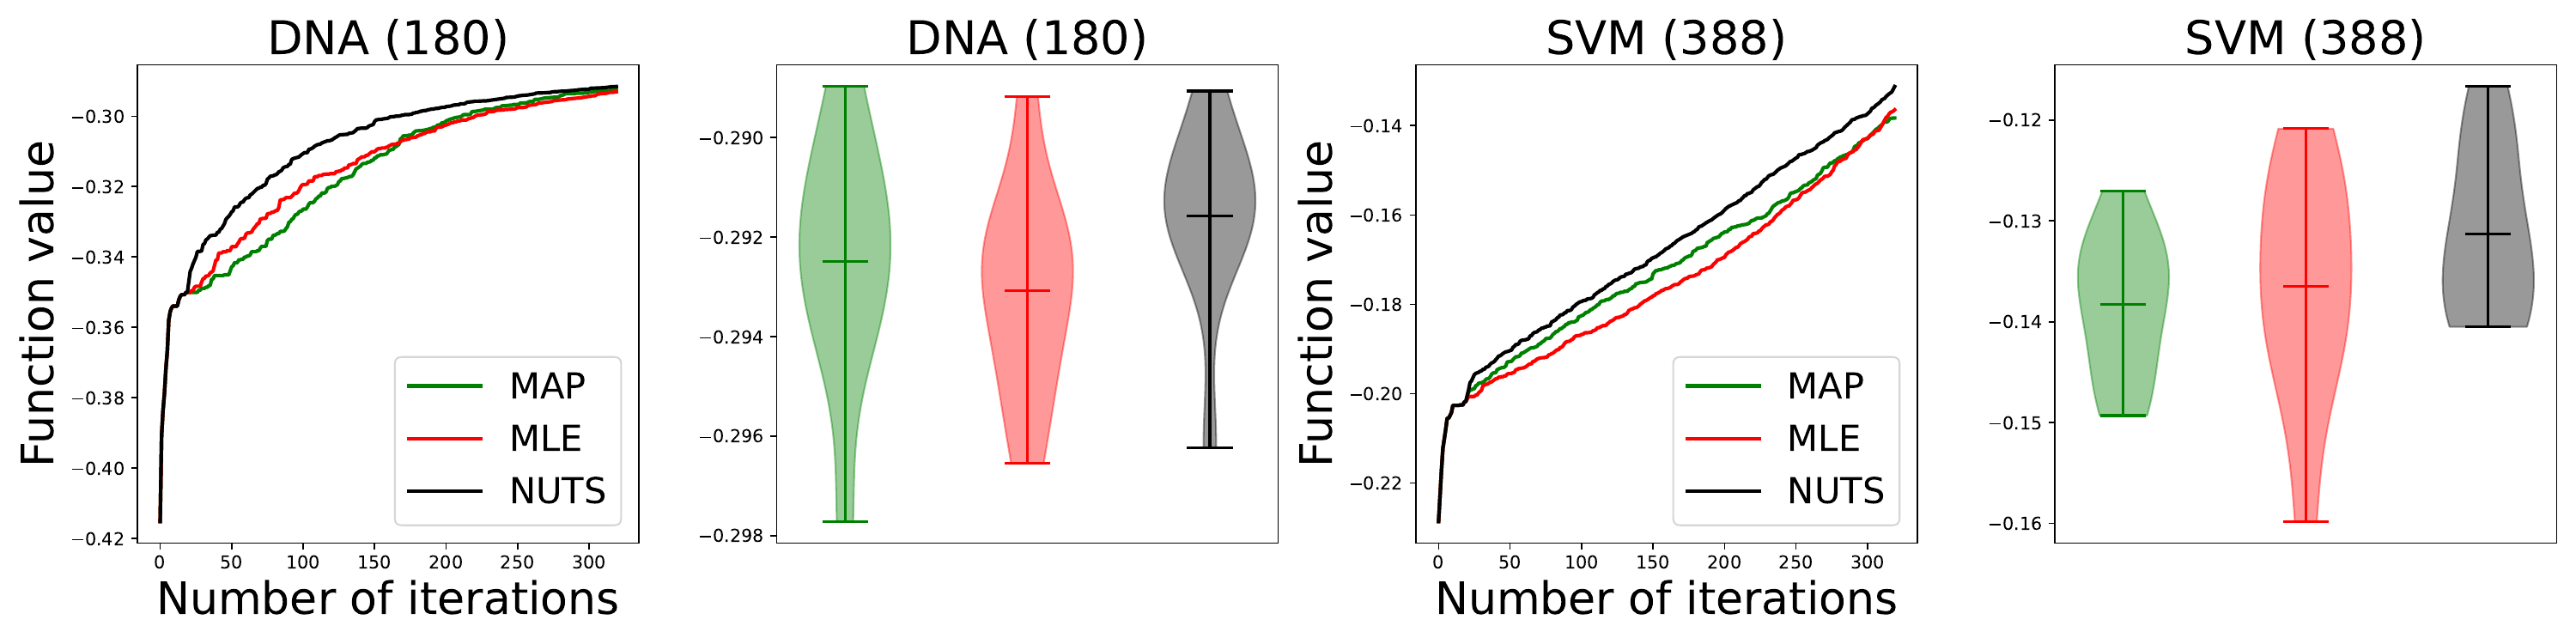}
	\caption{\small Optimization performance when using ARD Mat\'ern trained with MAP and MLE, and NUTS on SVM (388) and DNA (180). The results were summarized from 10 runs.}
 \label{fig:op-performance-gpard-nuts}
\end{figure}
\begin{figure*}[t]
    \centering
    \includegraphics[width=\textwidth]{BO ICLR 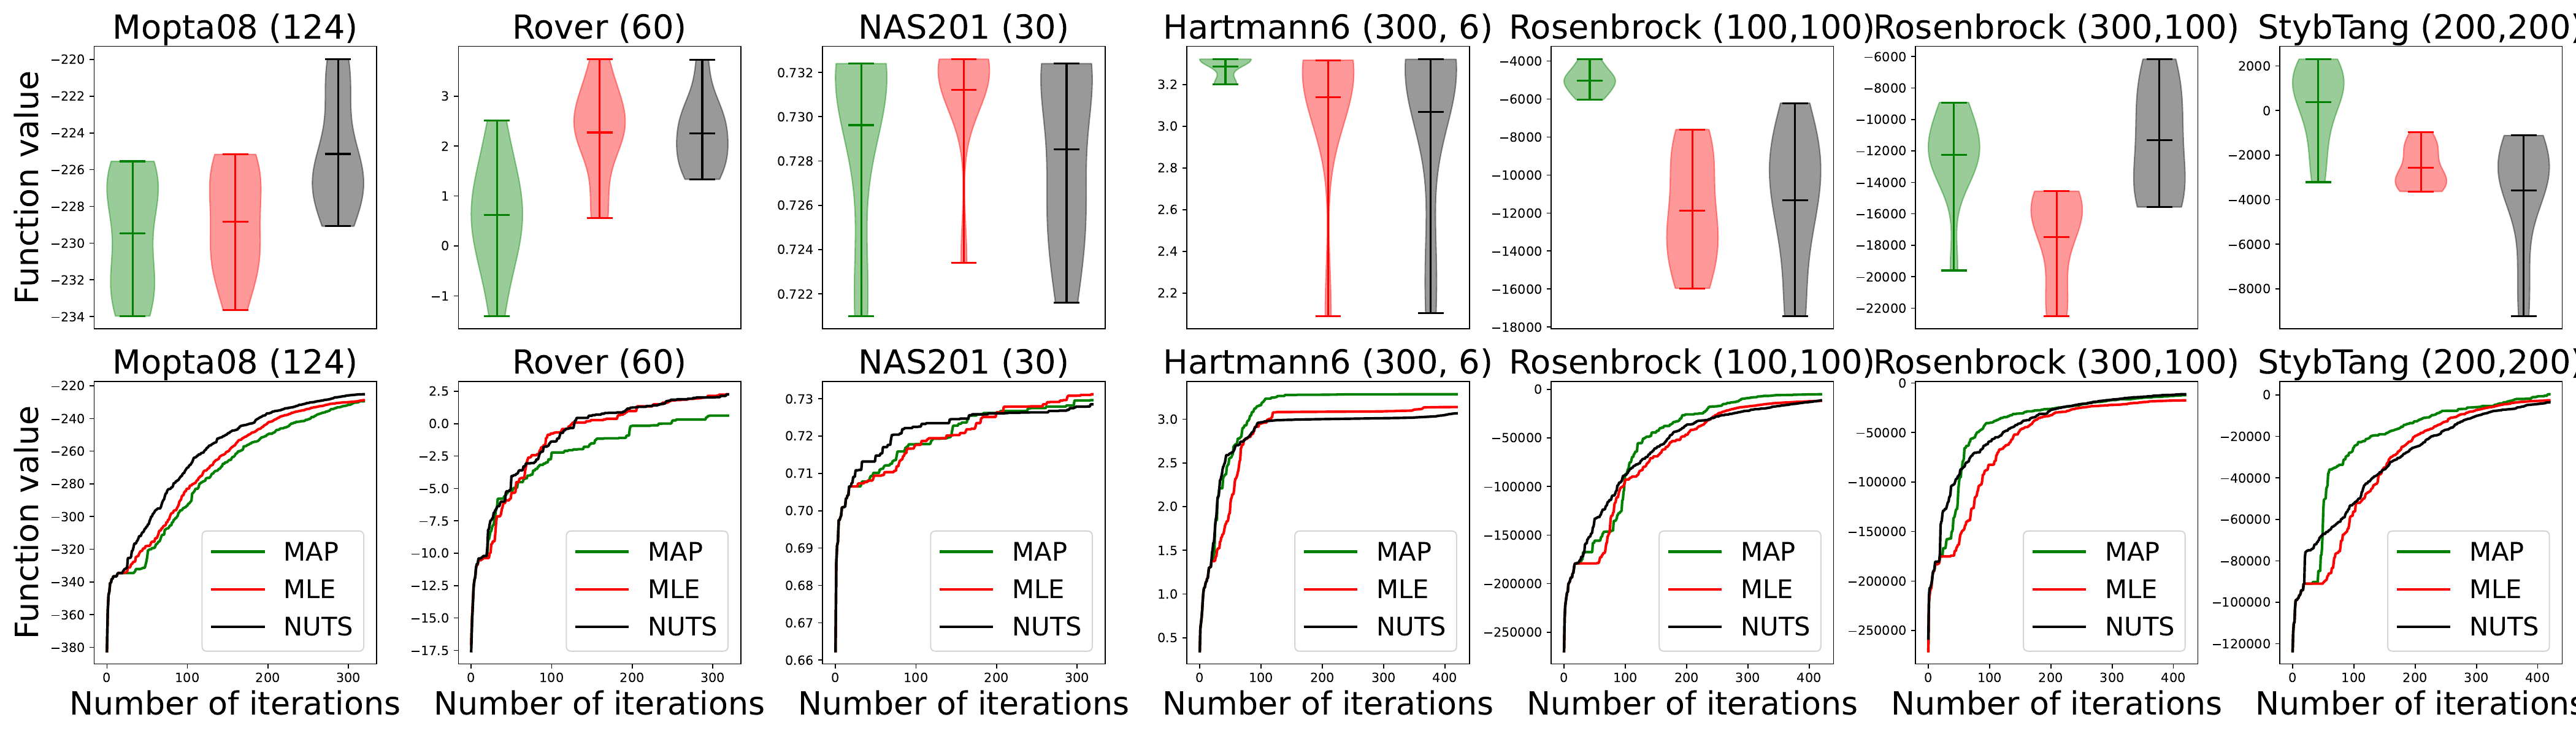}
    \caption{\small Optimization performance using MLE training,  MAP training with a diffuse prior over the length-scale parameters, and  NUTS on the rest of benchmarks. The results were summarized from 10 runs.}
    \label{fig:op-performance-gpard-nuts-rest}
\end{figure*}

\section{Additional Results}\label{sect:fail}

\subsection{BNN-based BO and Standard BO with a Single Length-Scale}

Due to the space limit, we did not report the results of the BNN-based BO in the main paper. Here, we supplement the comparison with the aforementioned two BNN-based BO approaches, \textit{BNN Laplace} and \textit{BNN HMC}, as specified in Section~\ref{sect:impl}. 
In addition, we also tested SBO with a single length-scale. We used the Mat\'ern kernel. The results are reported in Fig. XX and XX \zhec{BNN-BO and single-scale BO}.  Across all the benchmarks, the performance of the BNN based methods is worse than the median of GP based methods. In cases, such as SVM, Hartmann6 (300, 6) and Rosenbrock, the performance of the BNN based methods is close to or overlapping with the performance of the worst GP baselines. This might be due to that under low data regimes, it is more challenging for a neural network to capture the shape of the target function and quantify the uncertainty, especially for high-dimensional targets. 

Interestingly, even using a single length-scale parameter,  the standard BO, namely SBO-Single --- as long as it does not encounter gradient vanishing ---  still consistently shows superior performance, which closely matches ARD Mat\'ern across most tasks, except for Ackley(300, 150), SBO-Single struggled in finding right locations to query, leading to poor performance.

\subsection{Alternative Ways to   GP Training}
%MLE training and its BO performance
\subsubsection{Maximum Likelihood Estimation (MLE)}
In the main paper, we report the SBO performance when training GP via MAP estimation. We then examined another popular GP training approach, MLE training. We used ADAM optimization~\citep{kingma2014adam}\footnote{We also experimented with using L-BFGS for MLE training. However, L-BFGS frequently encounters numerical issues and often fails to reliably complete model training. This is consistent with findings reported in~\citep{hvarfner2024vanilla}. The issue likely arises because, without constraints or regularization on parameters like the length-scales and amplitude, L-BFGS tends to explore too aggressively, leading to numerical instability.} to perform MLE, with learning rate $0.1$ and the maximum number of epochs was set to $500$. We employed ARD Mat\'ern kernel. The ultimate and running optimization performance is shown in Fig. XX and XX. \zhec{figure about SBO with MLE training} As we can see, the BO performance of using MAP and MLE training is close, without significant difference between the two.

\subsubsection{MAP Training with Alternative Priors}
Second, we examined MAP training with alternative prior choices over the length-scale parameters. In the main paper, we use a diffuse prior, \texttt{Uniform(0.001, 30)}. In practice, another commonly used choice is a concentrated Gamma prior, \eg \texttt{Gamma(3, 6)}, which is the default choice in the popular BO library BoTorch. To see how it is concentrated, in Fig. \ref{fig:pdf} we compare its probability density curve with other priors, including the aforementioned uniform prior and the diffuse Gamma priors over the amplitude and noise variance.

We observe that the prior distribution $\texttt{Gamma(3, 6)}$  places a large probability mass around its mean 0.5, strongly regularizing the length-scale parameters toward this value. According to our theoretical analysis (see Section~\ref{sect:theory}), this introduces a significant risk of gradient vanishing in high-dimensional settings, potentially leading to failure in GP training.

To verify the risk,  we examined the alignment between the prediction and the ground-truth across the test examples from Mopta08 (124) and DNA (180).  As depicted in Fig. \ref{fig:alignment-more} (third and fourth column), the concentrated prior leads to a severe prediction deviation from the ground-truth, indicating failure in learning the target function. This observation aligns with findings reported in the SaasBO paper~\citep{eriksson2021highdimensional} (see Fig.1 of that paper). 

We further investigated the impact of this prior within the optimization loop.
As shown in Fig \ref{fig:final-Gamma36} and \ref{fig:runtime-Gamma36}, after placing the prior Gamma(3,6) over each length-scale parameter, the BO performance  drops substantially across many tasks, such as Mopta08 (124), SVM (388) and Ackley(150, 150), no matter using ADAM or LBFGS to conduct training.

\begin{figure*}[!ht]
    \centering
    \includegraphics[width=\textwidth]{BO ICLR 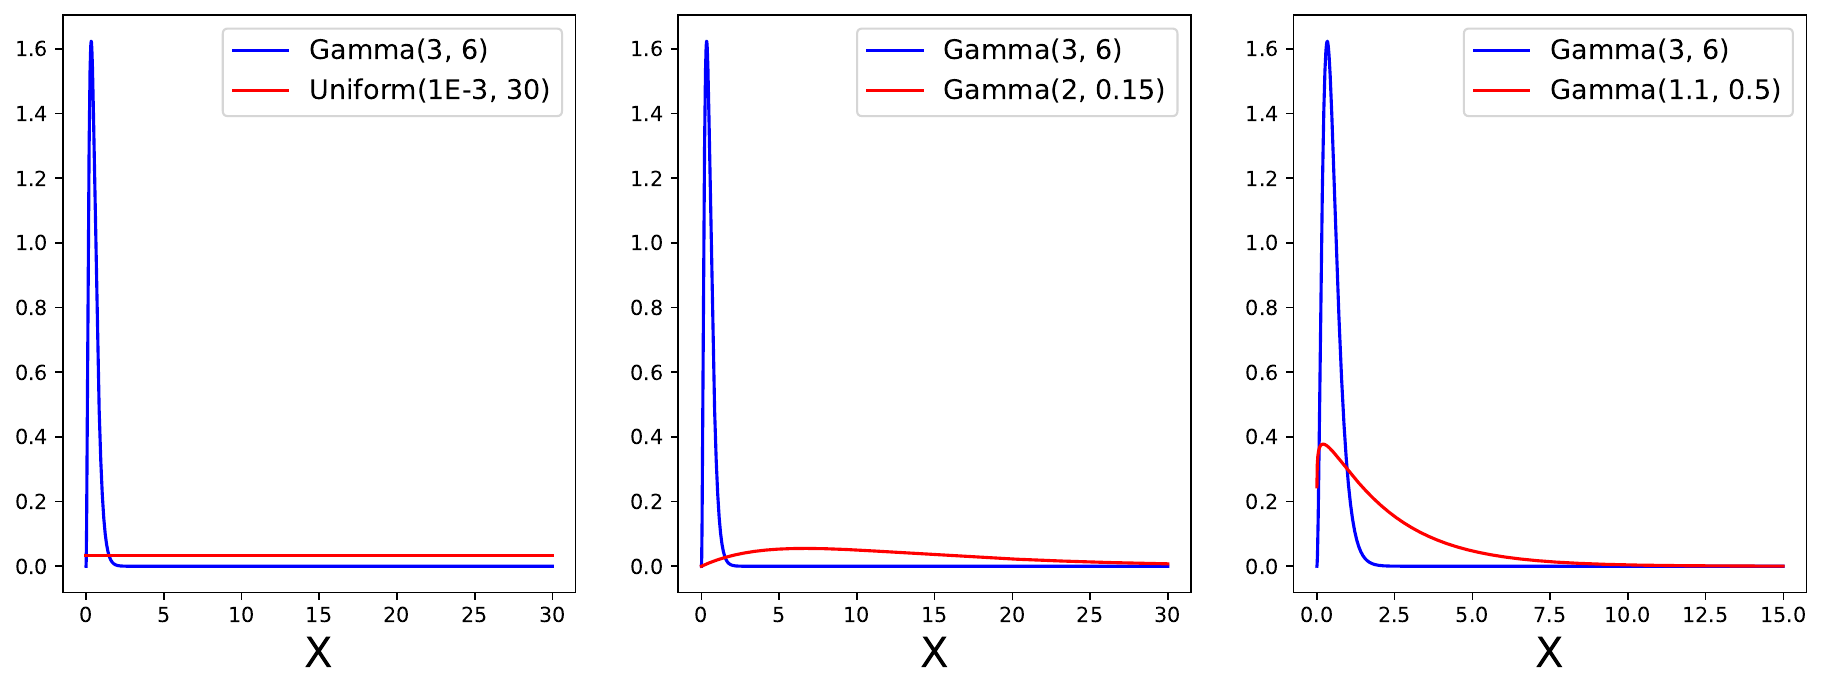}
    \caption{\small Probability density curves. Gamma(2, 0.15) and Gamma(1.1, 0.5) are the priors for the amplitude and noise variance, respectively.}
    \label{fig:pdf}
\end{figure*}

\begin{figure*}[!ht]
    \centering
    \includegraphics[width=\textwidth]{BO ICLR 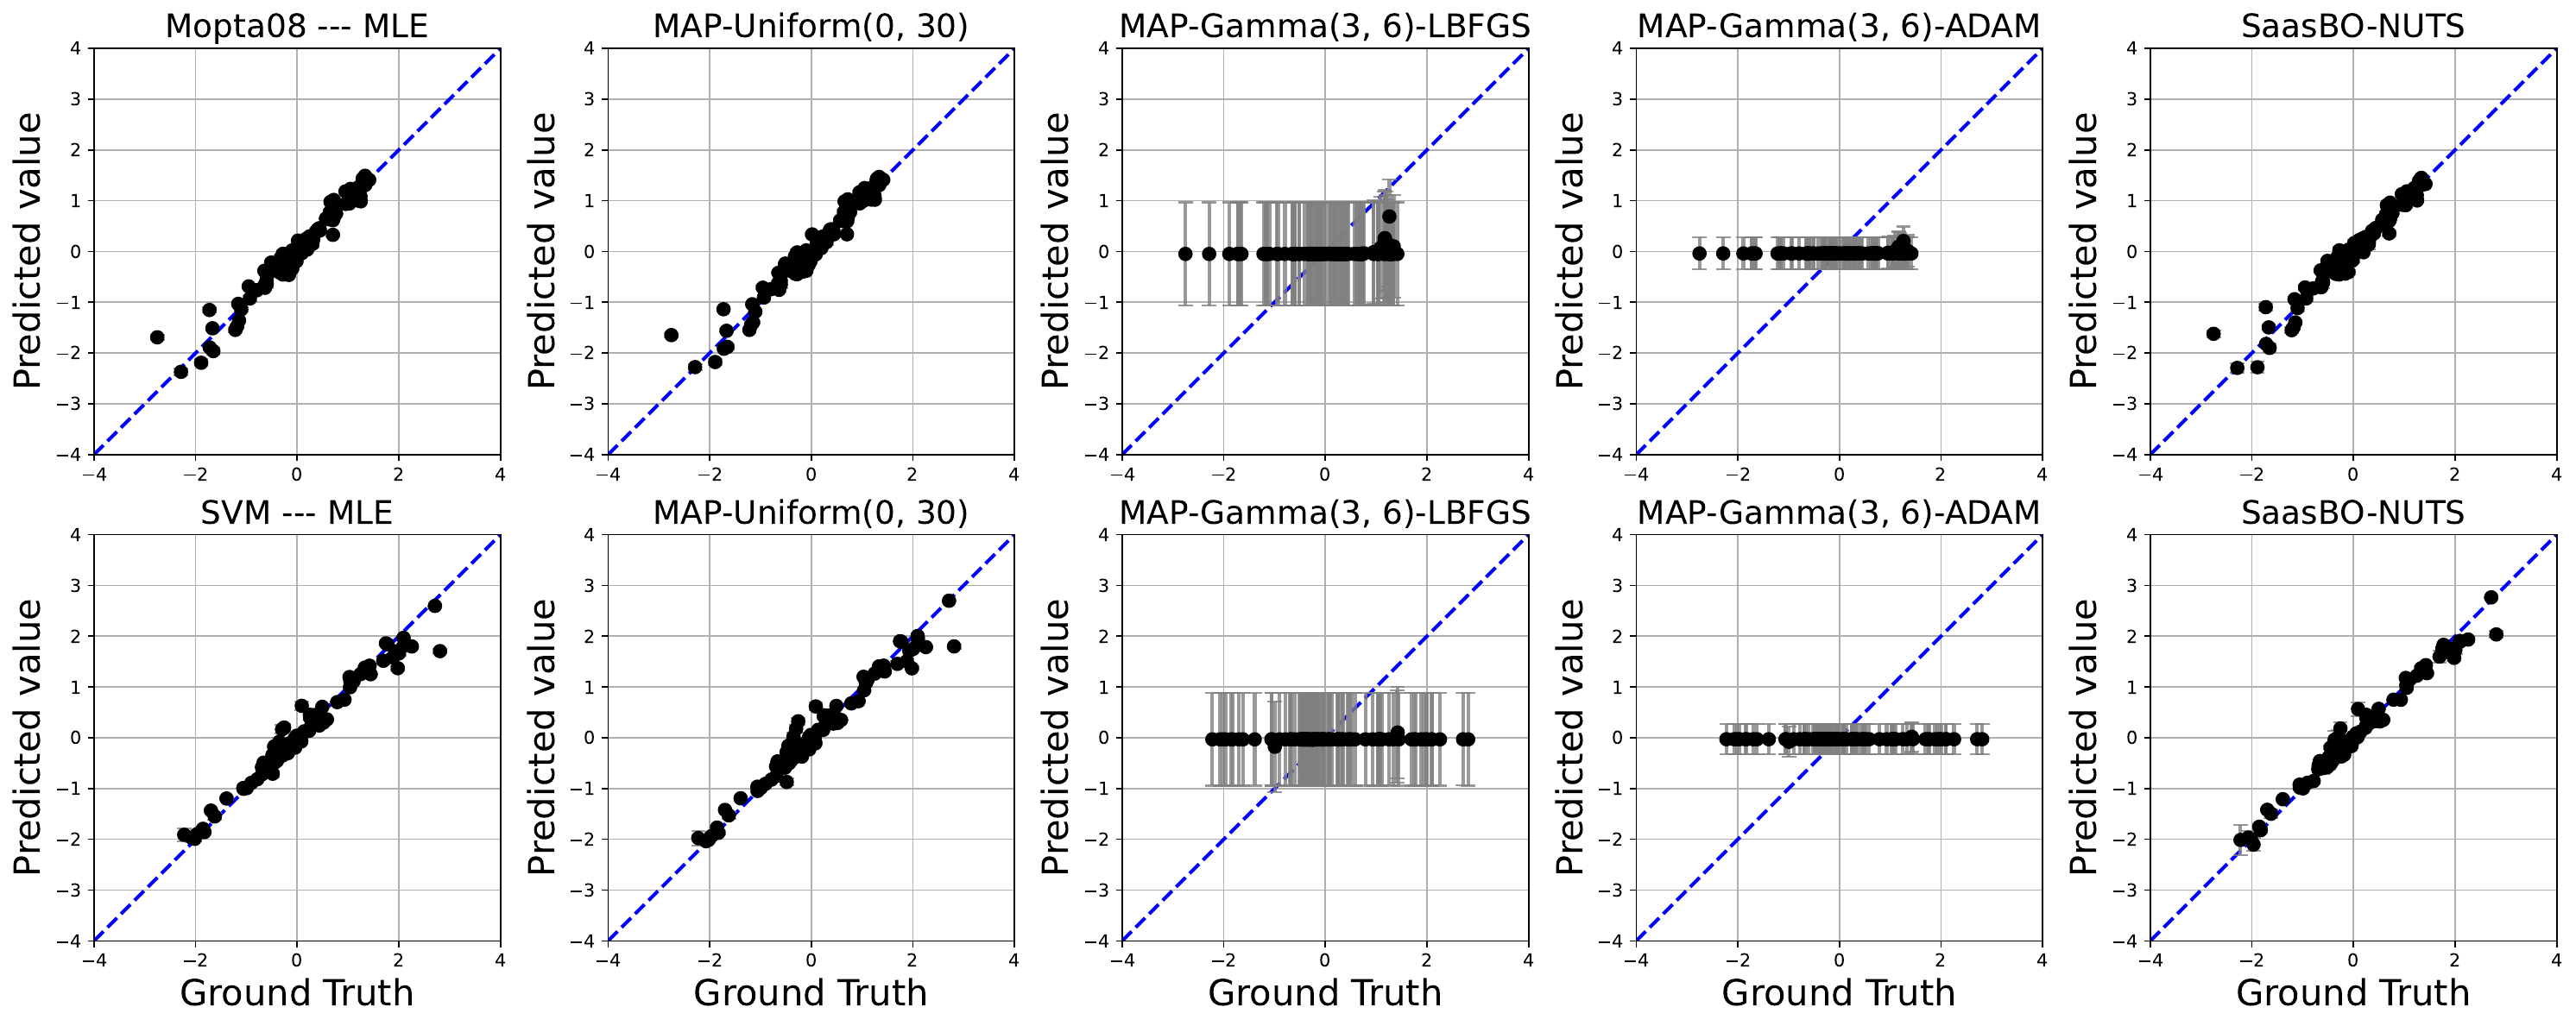}
    \caption{\small Alignment between the prediction (y-axis) and ground-truth function values (x-axis). \zhec{need updating?}}
    \label{fig:alignment-more}
\end{figure*}

\begin{figure*}[!ht]
    \centering
    \includegraphics[width=\textwidth]{BO ICLR 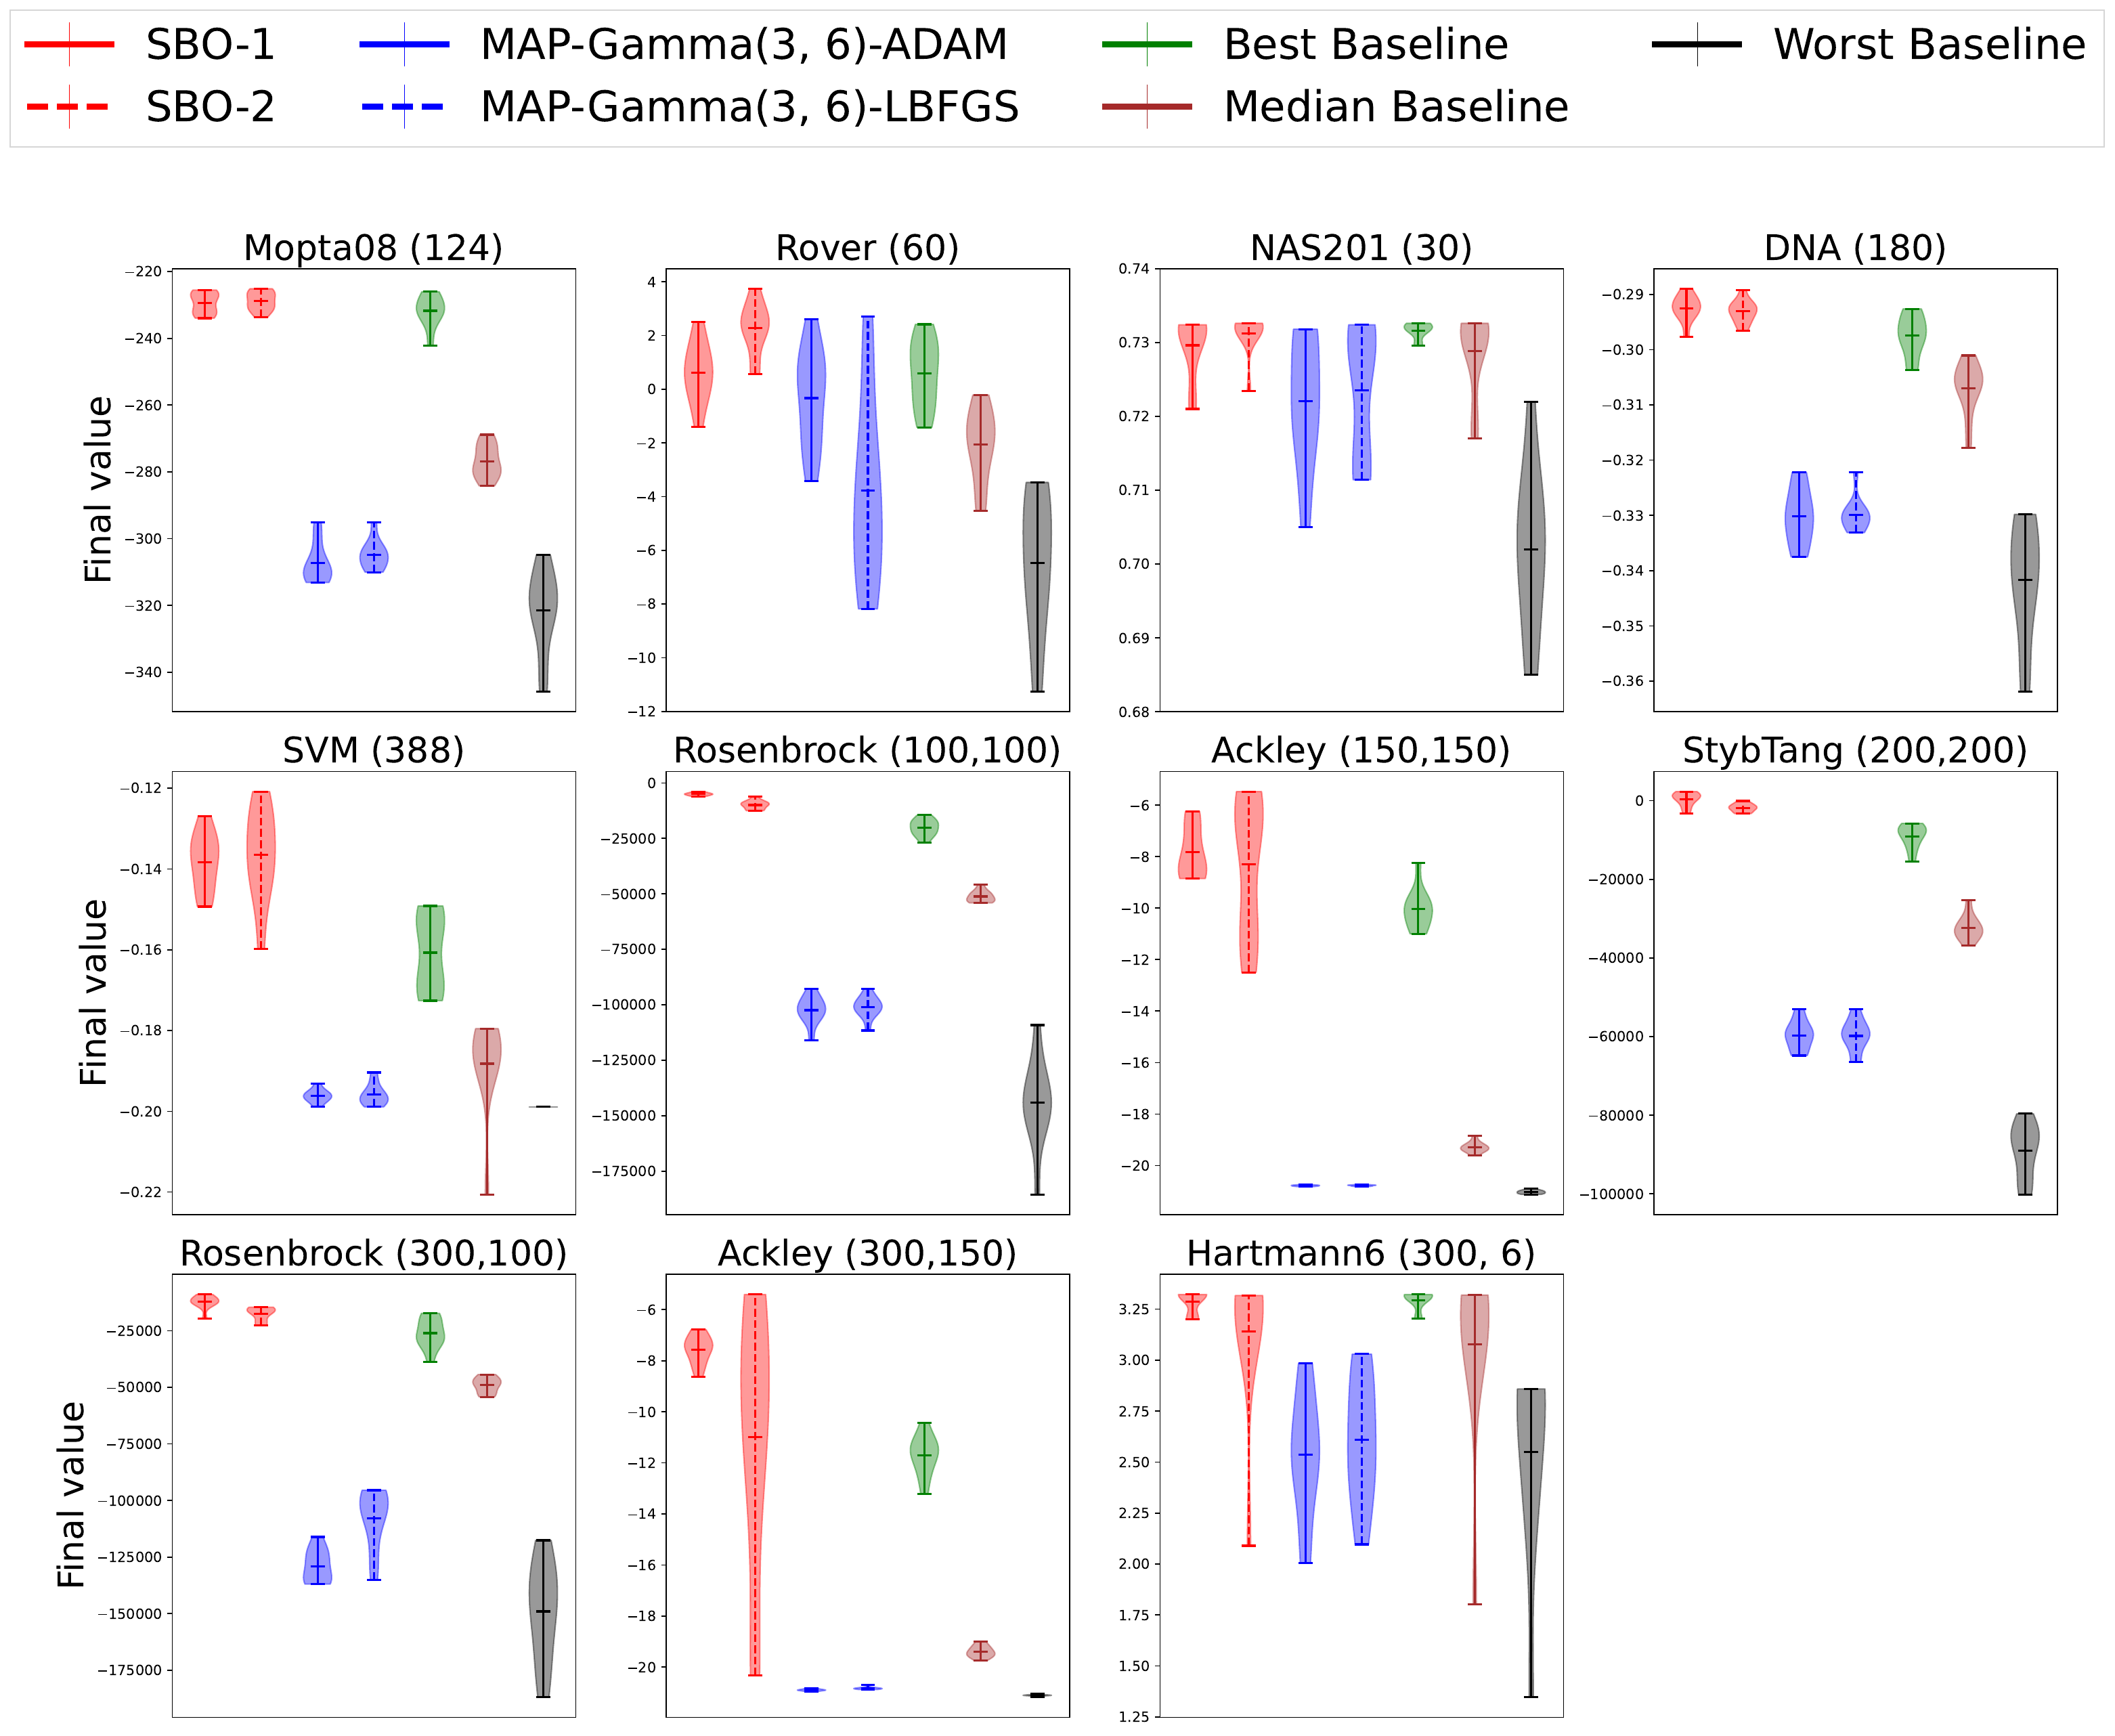}
    \caption{\small Ultimate optimization performance using a diffuse prior, Uniform(0.001, 30), \textit{vs.} a concentrated Gamma prior, Gamma(3,6),  over the length scale parameters. SBO-1 and SBO-2 use Uniform(0.001, 30). \cmt{Maximum Function Value Obtained at the end of optimization loop. The results were collect from 10 runs.}}
    \label{fig:final-Gamma36}
\end{figure*}

\begin{figure*}[!ht]
    \centering
    \includegraphics[width=\textwidth]{BO ICLR 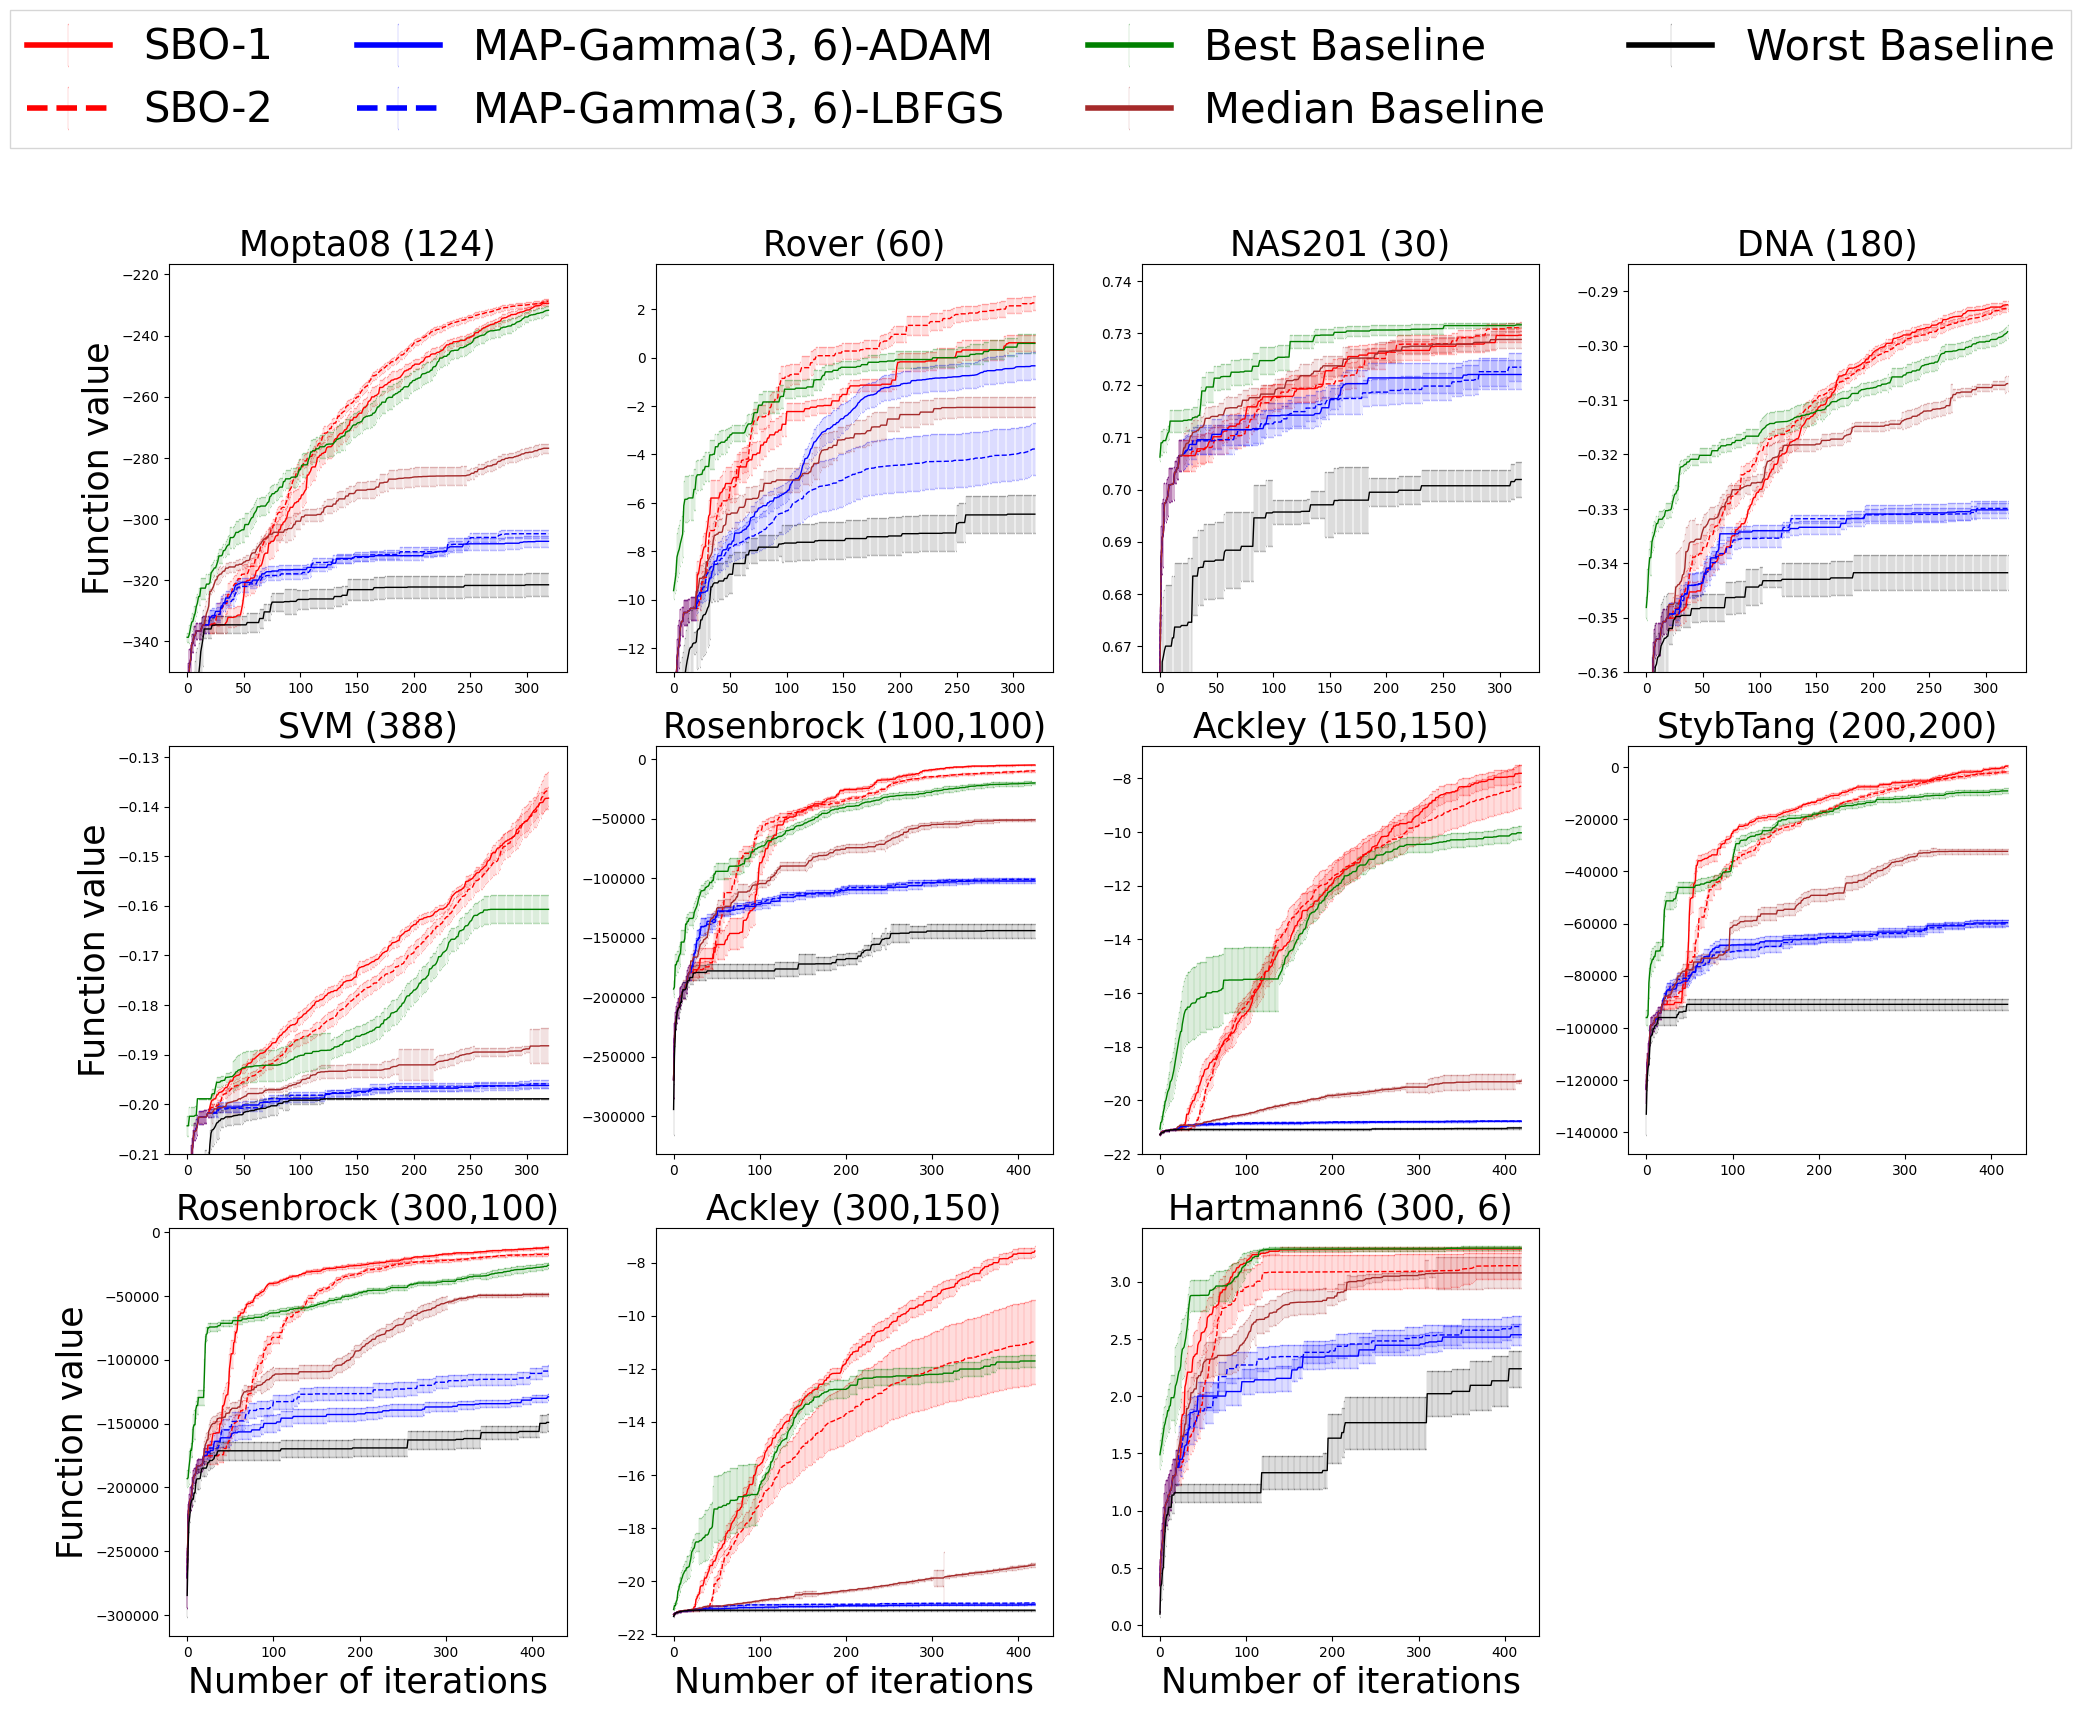}
    \caption{\small Runtime optimization performance using a diffuse prior, Uniform(0.001, 30), \textit{vs.} a concentrated Gamma prior, Gamma(3,6),  over the length scale parameters. SBO-1 and SBO-2 use Uniform(0.001, 30). \cmt{
    Maximum Function Value Obtained at the end of optimization loop. The results were collect from 10 runs.}}
    \label{fig:runtime-Gamma36}
\end{figure*}

\subsubsection{Fully Bayesian Training}
Third, we investigated whether a fully Bayesian training approach would yield substantial improvements in BO. In particular, we can use MCMC to perform posterior inference of the GP parameters, and then integrate them out during the prediction. We conducted another round of BO experiments. For each step, we used NUTS to train GP with ARD Mat\'ern. We adopted the same settings as used in SaasBO-NUTS~\citep{eriksson2021highdimensional}: where the mean parameter is assigned the standard Gaussian prior $\N(0,1)$, amplitude $\text{Gamma}(2, 0.15)$, and noise variance $\text{Gamma}(0.9, 10)$. We then assigned a uniform prior over each length-scale, $\text{Uniform}(0.001, 30)$. 
The number of warm up steps was set to 512, and after the warm up stage, we ran 256 steps, and selected the samples at every 16-th step as the posterior samples. We show the running and final optimization performance in Fig \ref{fig:op-performance-gpard-nuts} , and Appendix Fig.~\ref{fig:op-performance-gpard-nuts-rest}. 
We also show the average running time per optimization step in Table \ref{tb:real-runtime} and Table \ref{tb:syn-runtime}.
It can be observed that while NUTS contributes to a slight improvement in several tasks, the enhancement is marginal.

However, running NUTS is much more computationally costly compared to doing MAP and MLE. For example, on DNA, NUTS takes  59x and 40x running time of MAP and MLE, respectively, on average in each step.  
\textit{Therefore, for practical purposes, using MAP or MLE for GP training appears sufficient. It is computationally efficient, and the sacrifice of optimization performance is minimal compared to much more costly training methods like NUTS.}

\subsection{Different Choice of $\lambda$ in UCB}\label{sect:lam-choice}
We examined how the exploration parameter $\lambda$ in UCB influences the BO performance in high-dimensional optimization. To this end, we used ARD Ma\'ern kernel and varied $\lambda$ from \{0.5, 1.0, 1.5, 2.0\}. We conducted MLE training via ADAM optimization. 
We show the ultimate and runtime optimization performance in Fig. \ref{fig:final-lambda} and \ref{fig:running-lambda}, respectively. 
It can be seen that, in most benchmarks (Mopta08, Rover, NAS201, DNA, \etc), the performance with different $\lambda$'s is close. However, on DNA, SVM and Ackley, the performance of $\lambda=0.5$ is typically worse than the bigger choice of $\lambda$. This might be due to that those problems are more challenging (\eg Ackley has many local minima), a larger exploration level ($\lambda$) is needed to identify better optimization outcomes.

\subsection{Alternative Acquisition Functions}
Finally, we evaluated three other  acquisition functions for high-dimensional optimization: Expected Improvement (EI), log-EI and Thompson sampling (TS). 
At each step, EI computes the expected improvement upon the best sample so far, 
\begin{align}
    \text{EI}(\x) = (\mu(\x) - f(\x^*) )\Psi\left(\frac{\mu(\x) - f(\x^*)}{\sqrt{v(\x)}}\right) + \sqrt{v(\x)}\Phi\left(\frac{\mu(\x)-f(\x^*)}{\sqrt{v(\x)}}\right),
\end{align}
where $\Psi(\cdot)$ and $\Phi(\cdot)$ are the CDF and PDF of the standard Gaussian distribution, $\x^*$ is the best sample that gives the largest function value among all the queries up to the current step, 
$\mu(\x)$ and $\sqrt{v(\x)}$ are the posterior mean and standard deviation of $f(\x)$ given current training data. We used BOTorch to maximize EI through L-BFGS. 
The most recent work~\citep{ament2023unexpected} introduced log-EI to overcome the numerical challenges in optimizing the original EI acquisition function. Accordingly, we also tested log-EI using the BoTorch implementation. To conduct TS at each step, we used Sobol Sequence~\citep{sobol1967distribution} to sample 3K inputs in the domain, and jointly sampled the 3K function values from the GP posterior. We then selected the input with the largest function value as the next query. We denote this method by TS-3K. To explore more input candidates, we also employed the Lancos and conjugate gradient descent to approximate the posterior covariance matrix, and sampled 10K input candidates from Sobol Sequence. We denote this method as TS-10K. We used BOTorch implementation of both methods. We used ARD Mat\'ern kernel and MLE training at each step. 

\zhec{add EI, log-EI and TS results here.}
The ultimate and runtime optimization performance for using EI, TS-3K and TS-10K, are shown in Fig. \ref{fig:final-acqf} and \ref{fig:running-acqf}, respectively. As we can see, in most cases, such as Mopta08 (128), SVM (388), DNA (180) and Rosenbrock (100, 100), both EI and TS perform worse than UCB, and also worse than the best baseline. On Ackley(150, 150) and Ackley(300, 150), the performance of EI and TS are even among the worst.
The failure of EI might arise from the gradient vanishing during the optimization, as pointed by the recent work~\citep{ament2024unexpected}. The failure of the TS might be due to the high-dimension of the input space. A few thousand  candidates might not be sufficient to cover the whole space; as a result, the selected queries are inferior in indicating  the best direction to optimize the target function. The use of log-EI performed excellently, achieving results comparable to those obtained with UCB. 

\begin{figure*}[!ht]
    \centering
    \includegraphics[width=\textwidth]{BO ICLR 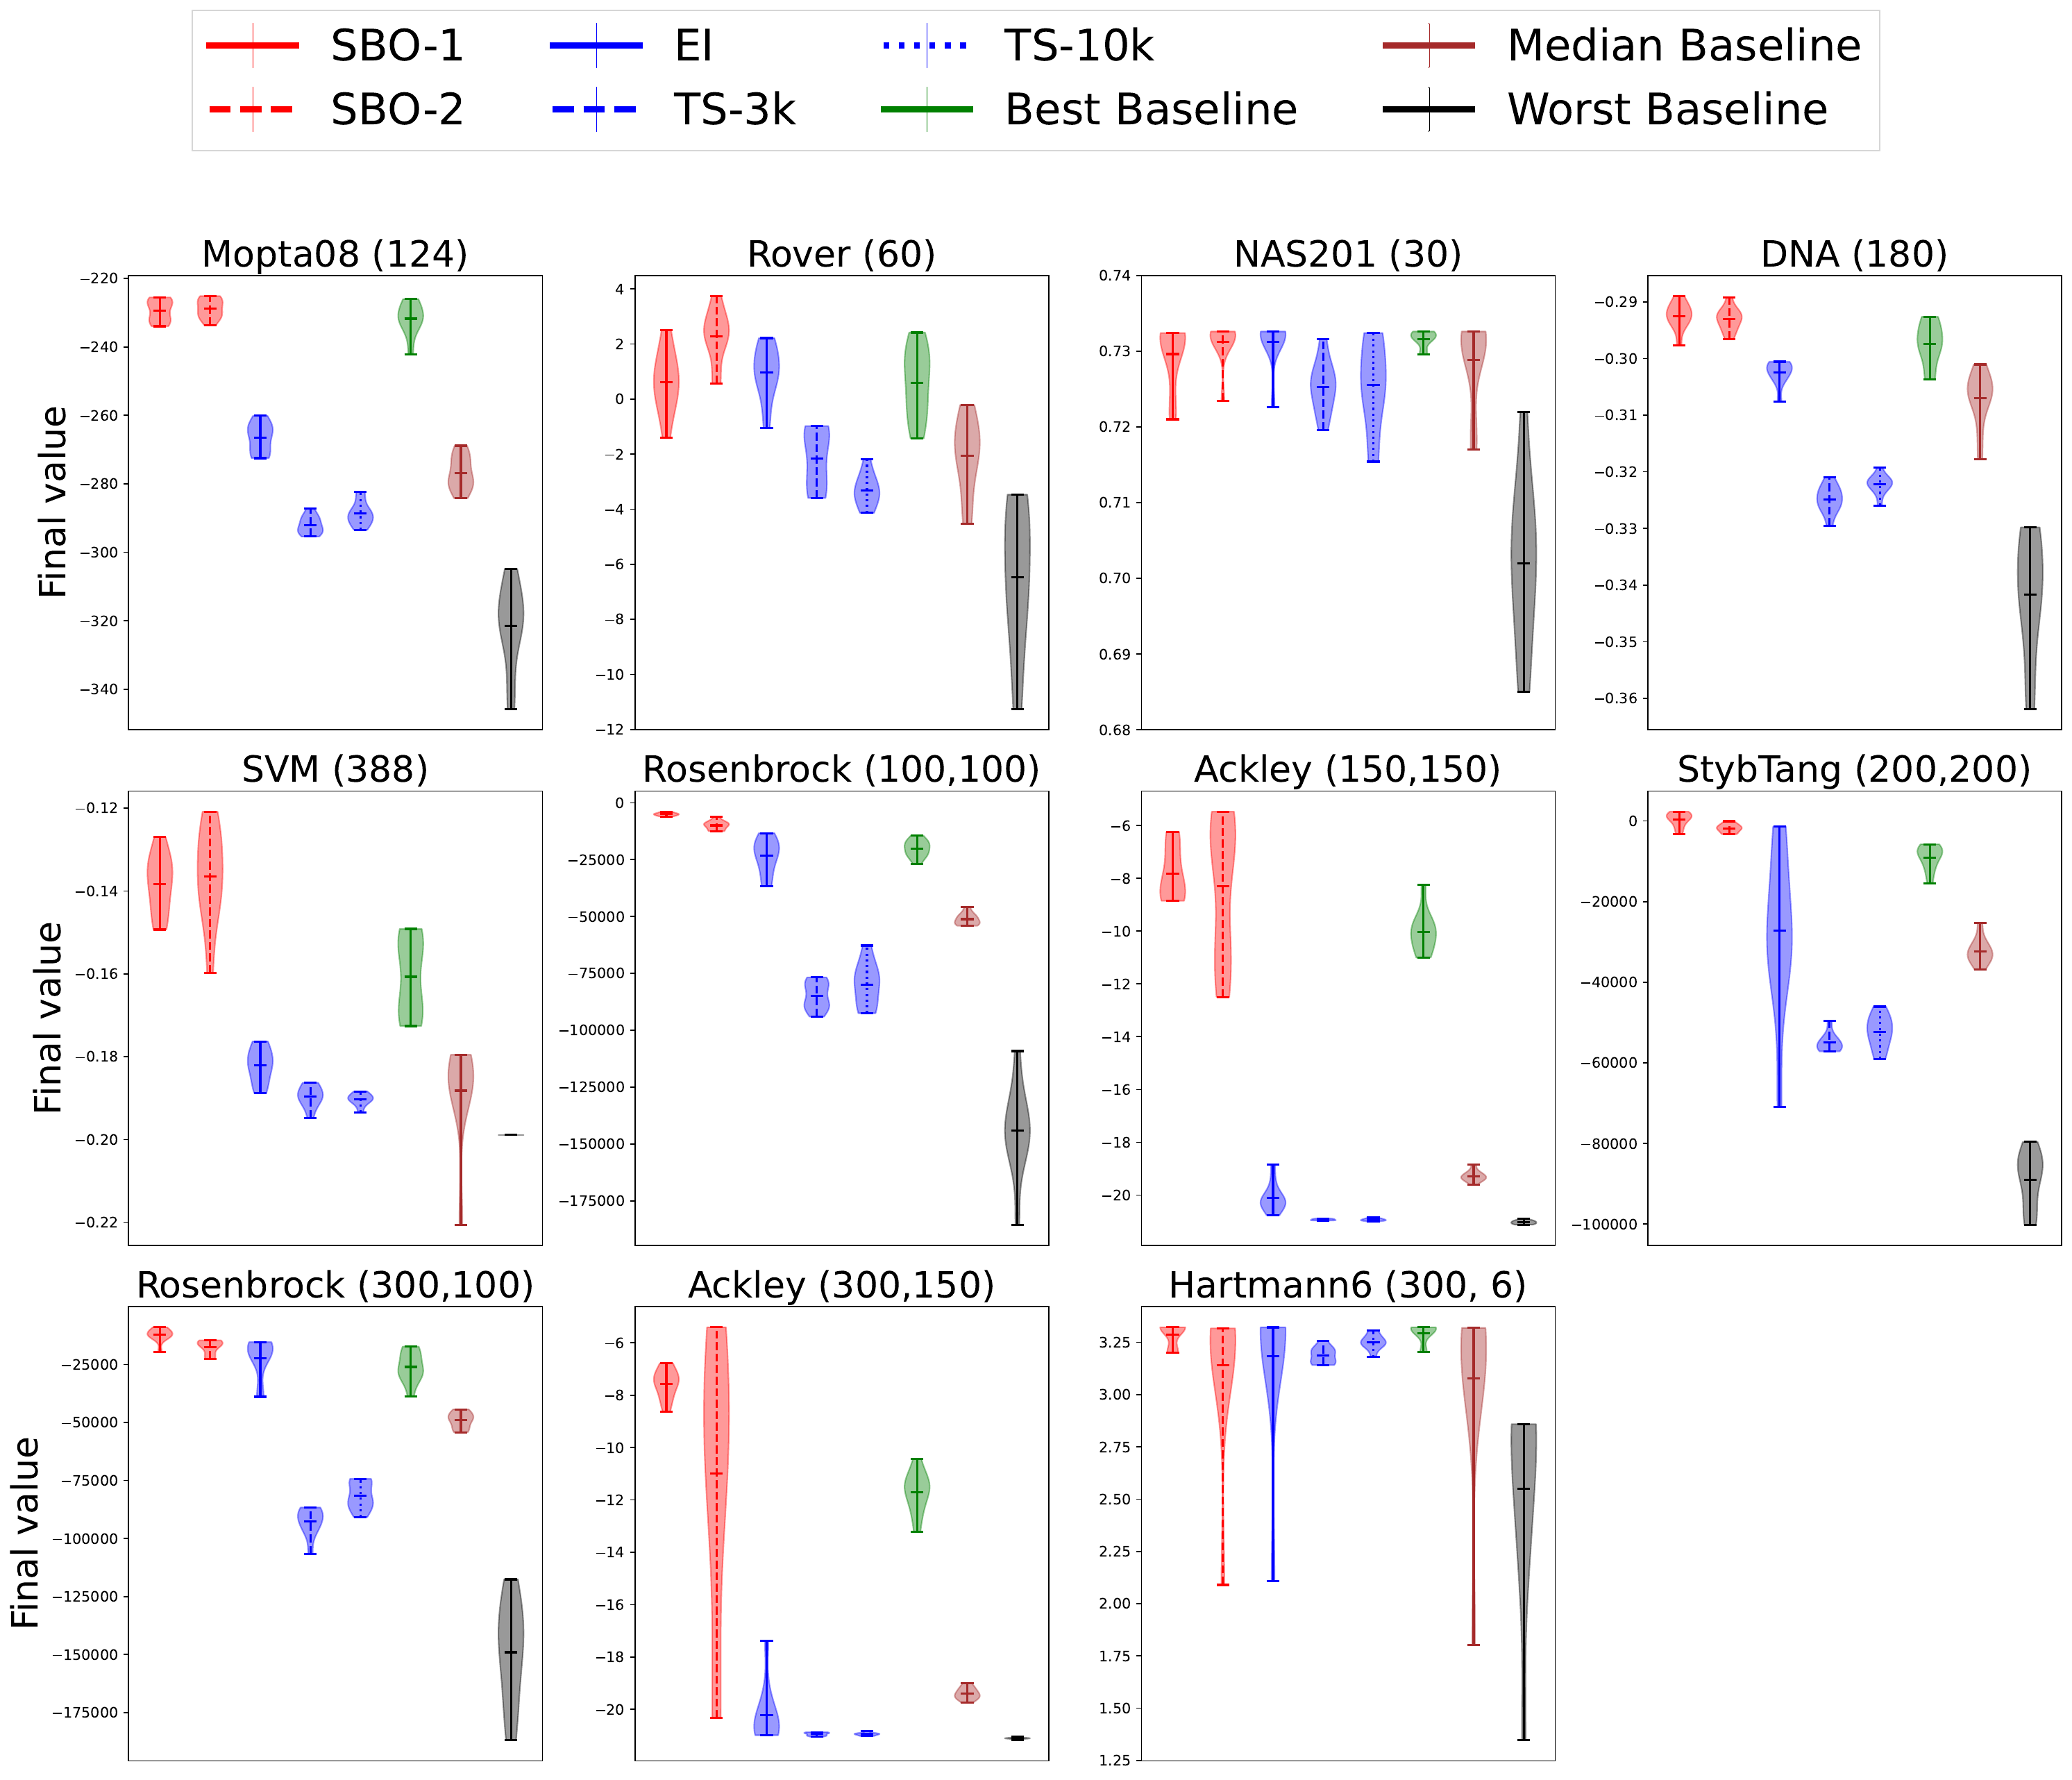}
    \caption{\small Ultimate performance with different acquisition functions. Note that SBO-1 and SBO-2 use UCB. \cmt{Maximum Function Value Obtained at the end of optimization loop. The results were collect from 10 runs.}}
    \label{fig:final-acqf}
\end{figure*}
\begin{figure*}[!ht]
    \centering
    \includegraphics[width=\textwidth]{BO ICLR 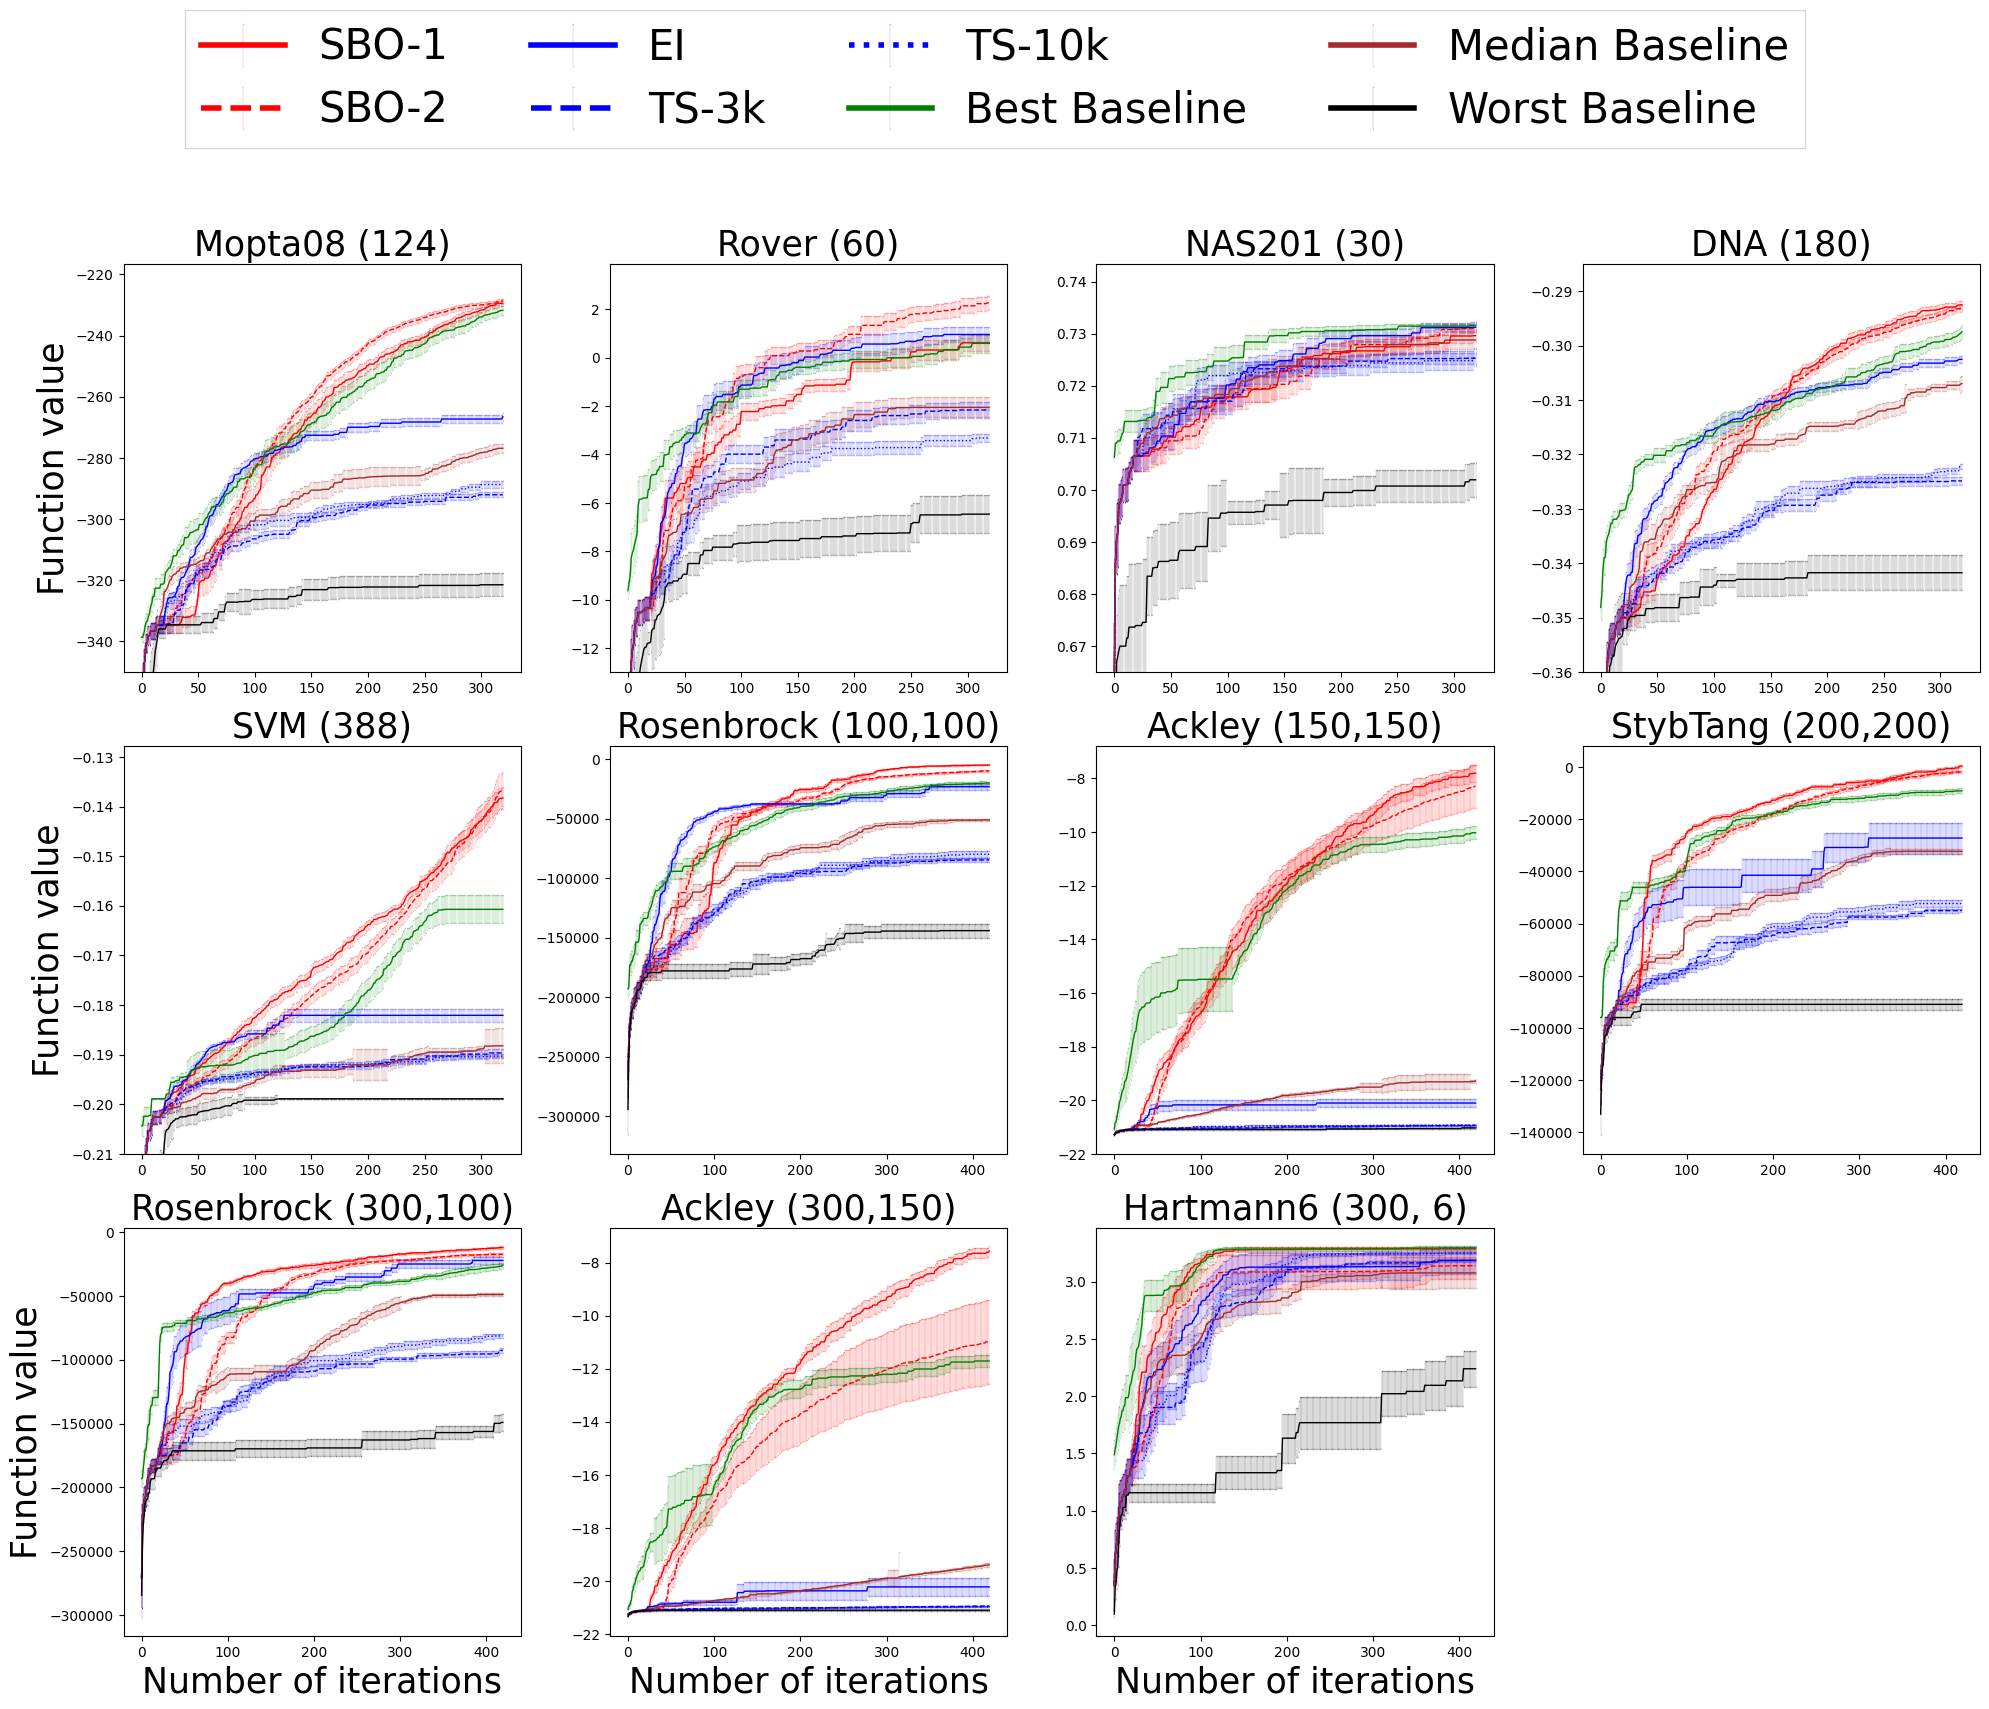}
    \caption{\small Runtime performance with different acquisition functions. Note that SBO-1 and SBO-2 use UCB. \cmt{Maximum Function Value Obtained at the end of optimization loop. The results were collect from 10 runs.}}
    \label{fig:running-acqf}
\end{figure*}

\begin{figure*}[!ht]
    \centering
    \includegraphics[width=\textwidth]{BO ICLR 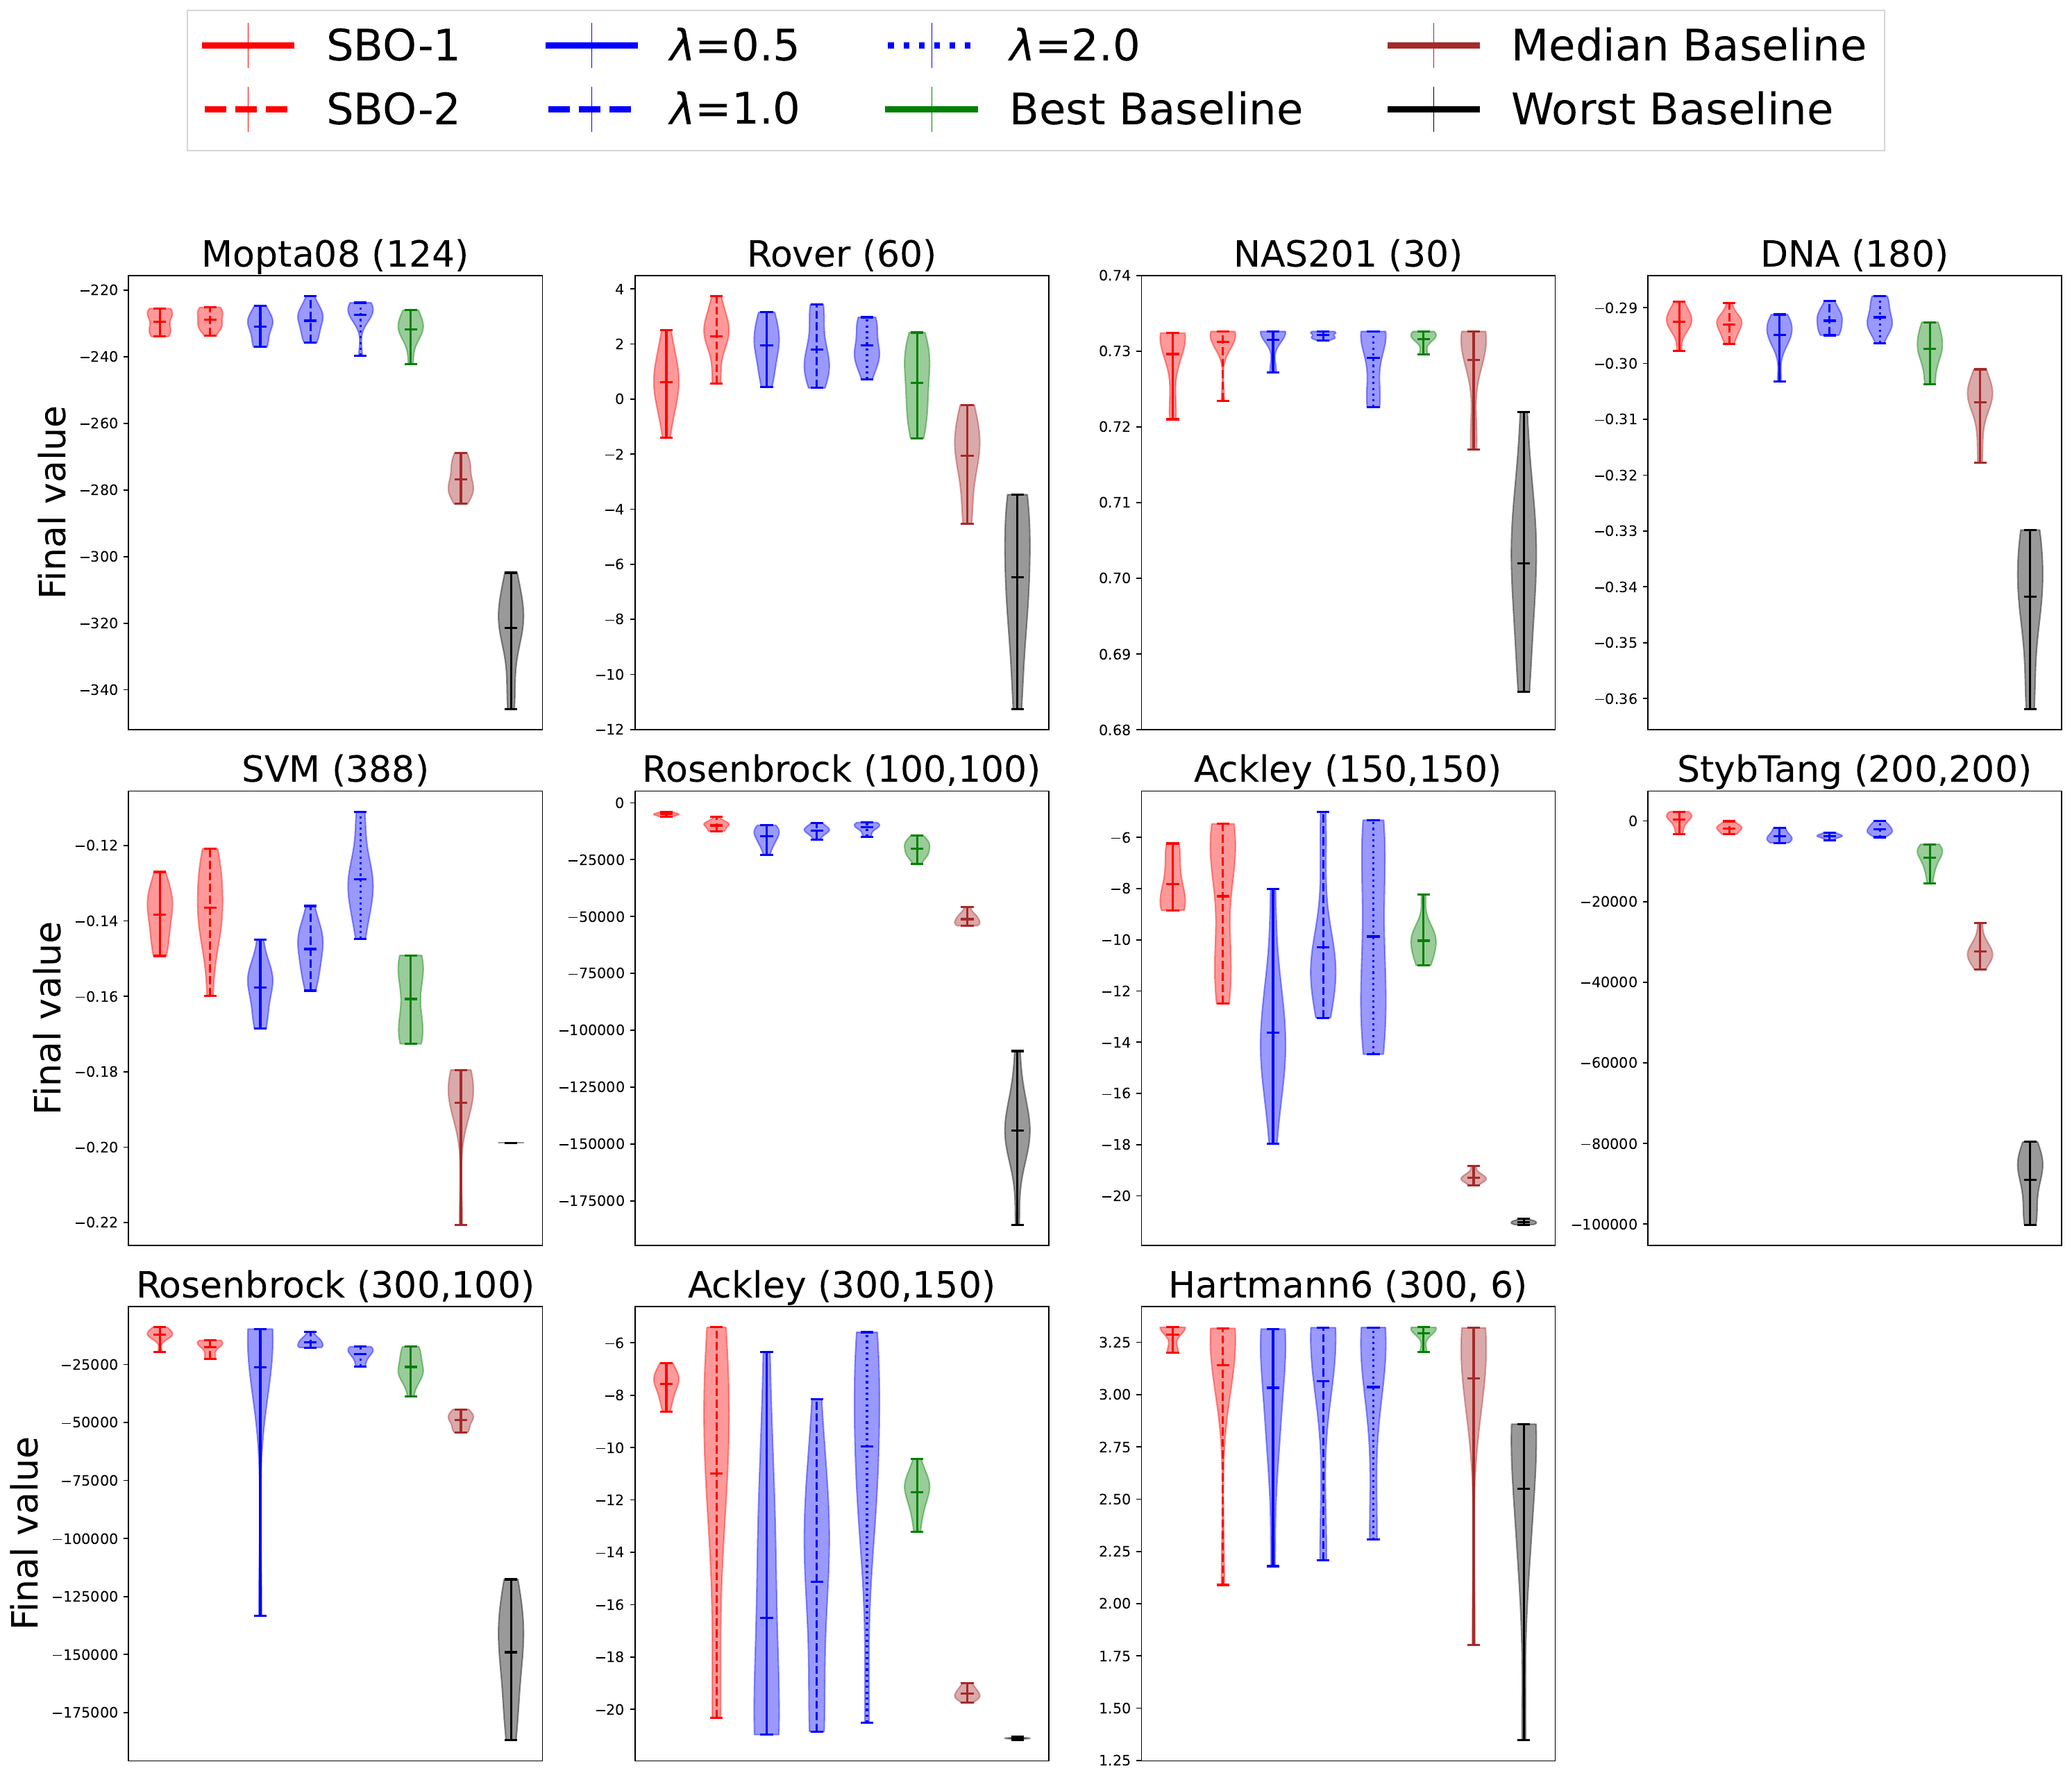}
    \caption{\small Ultimate optimization performance with different exploration level  $\lambda$ in UCB. Note that SBO-1 and SBO-2 use $\lambda=1.5$.
    \cmt{Maximum Function Value Obtained at the end of optimization loop. The results were collect from 10 runs. $\lambda$ varied from \{0.5, 1.0, 1.5, 2.0\}.}}
    \label{fig:final-lambda}
\end{figure*}
\begin{figure*}[!ht]
    \centering
    \includegraphics[width=\textwidth]{BO ICLR 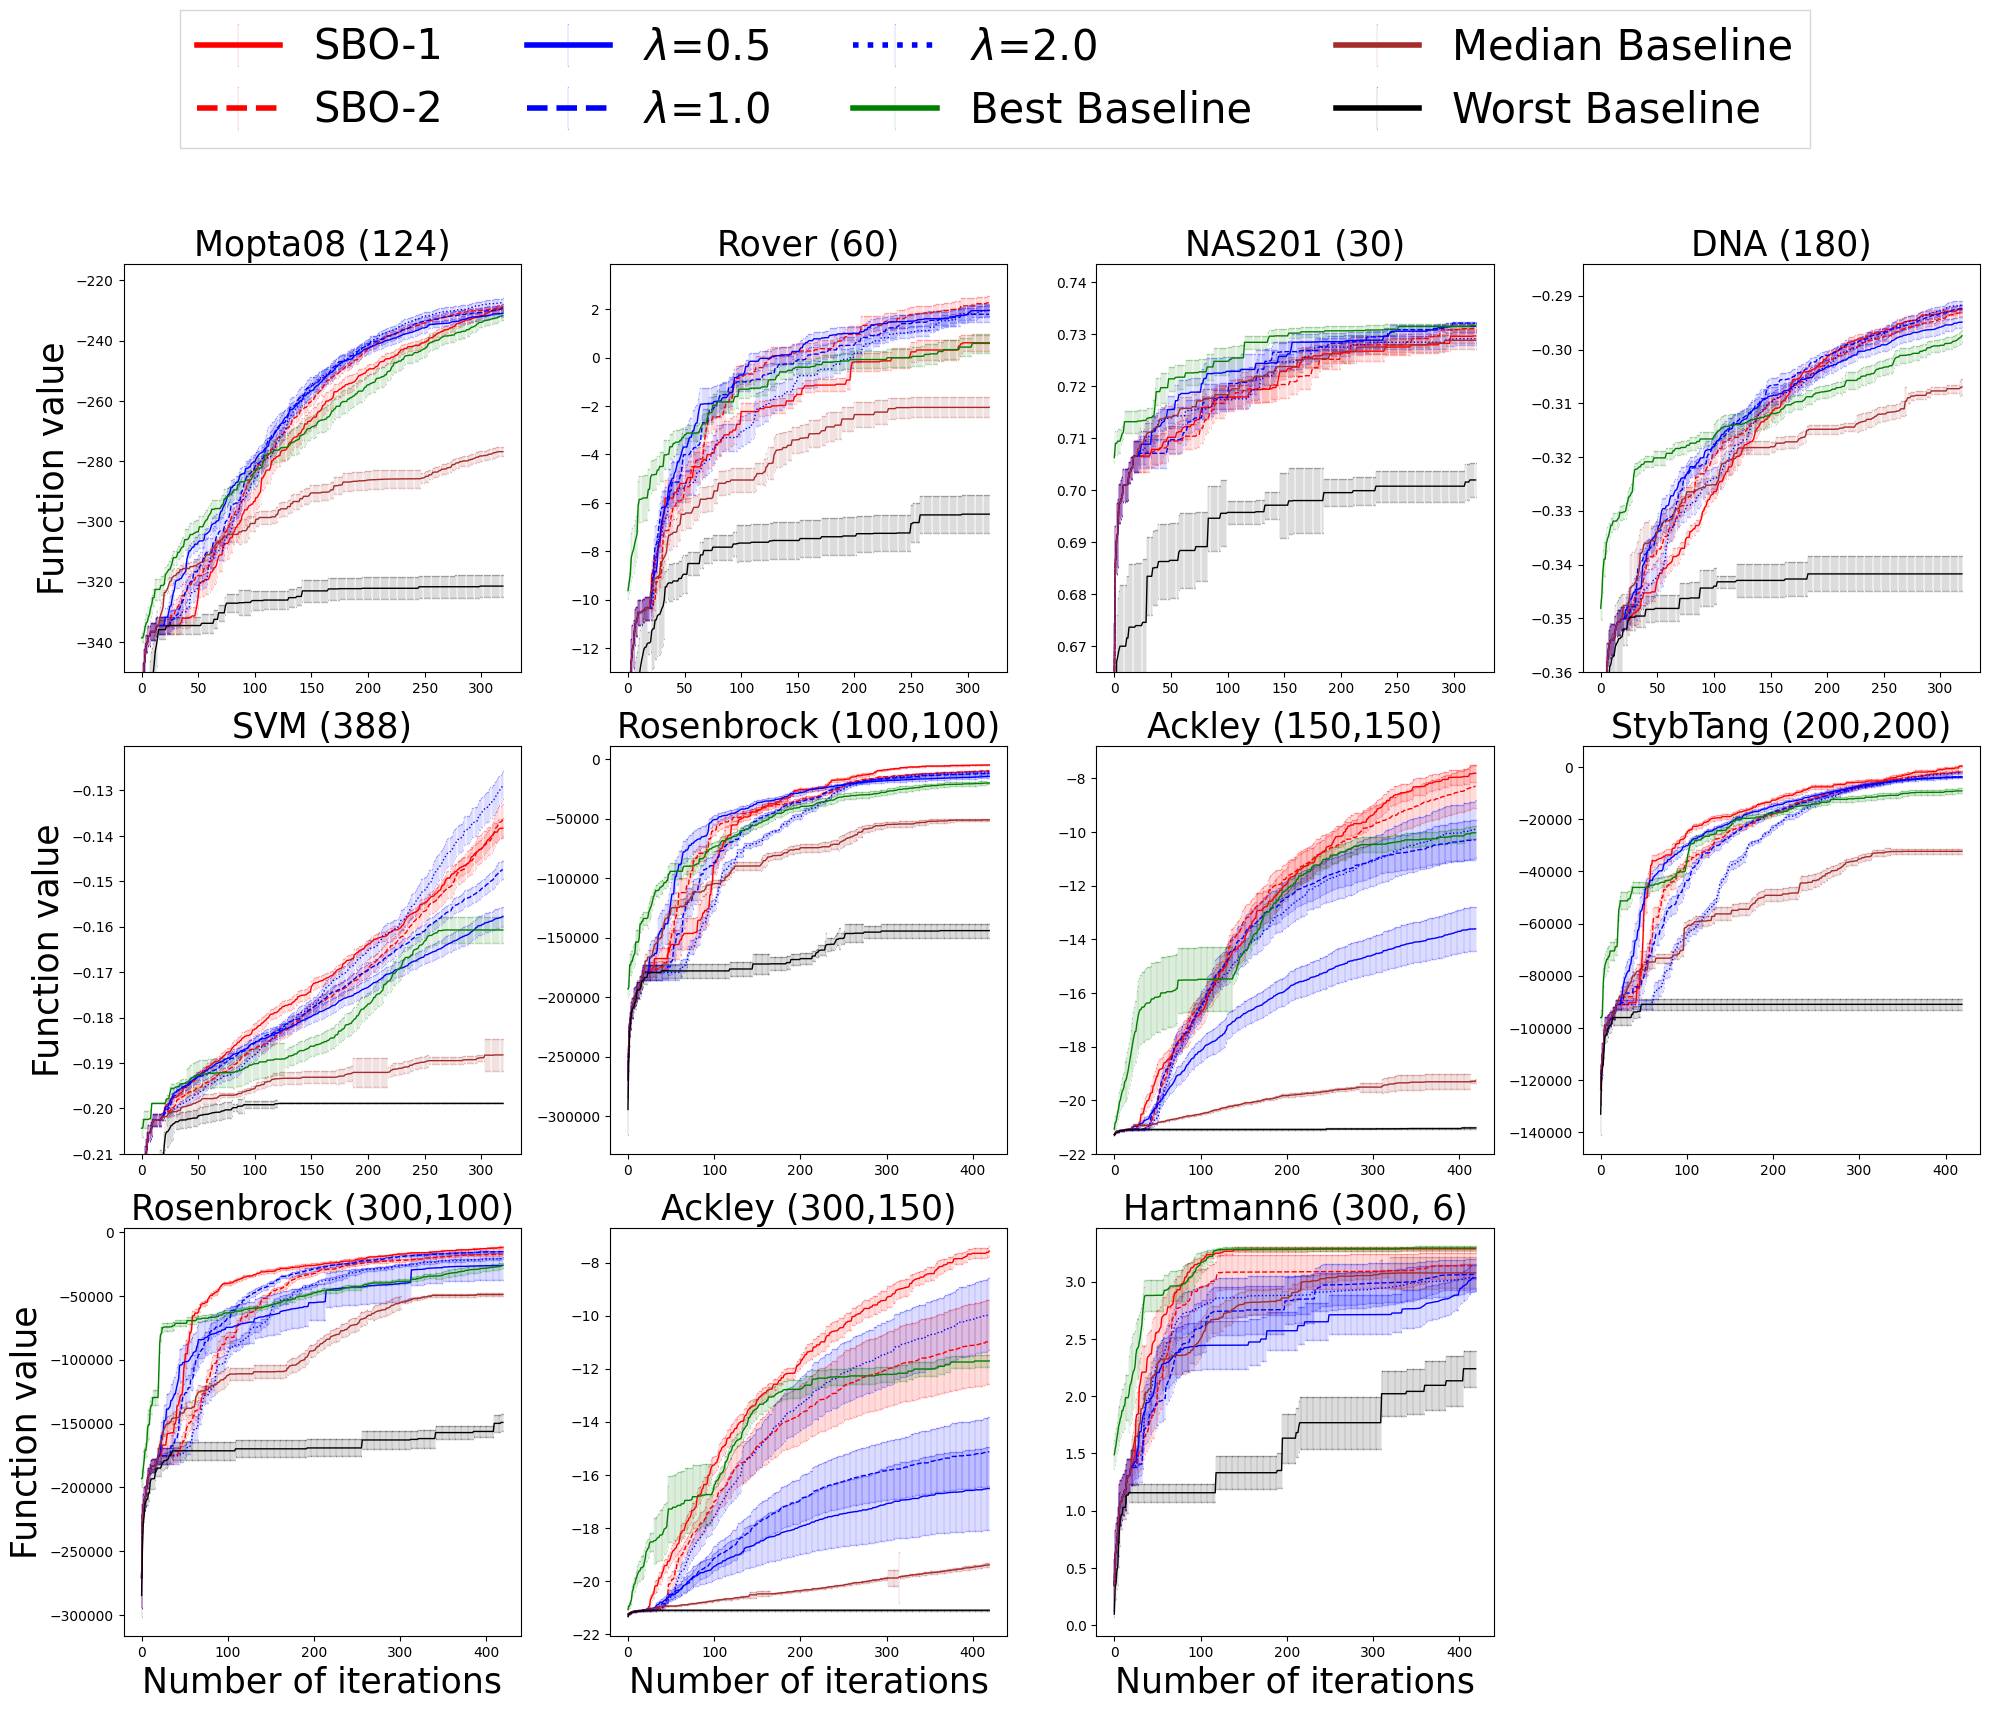}
    \caption{\small Runtime optimization performance with different exploration level  $\lambda$ in UCB. Note that SBO-1 and SBO-2 use $\lambda=1.5$. \cmt{Maximum Function Value Obtained at the end of optimization loop. The results were collect from 10 runs. $\lambda$ varied from \{0.5, 1.0, 1.5, 2.0\}.}}
    \label{fig:running-lambda}
\end{figure*}

\section{Limitation and Discussion}
\label{sec:limitation}
We evaluated Standard Bayesian Optimization on 5 real-world benchmarks and 6 synthetic functions that are most commonly used in previous HDBO works. We acknowledge that there are infinitely more  high-dimensional optimization problems that can be used for evaluation. In general, we hope after our work, future HDBO paper can include Standard BO with proper settings as their baseline methods. Hence, we can attain a better understanding about the potential of Standard BO in high dimensional functions. Moreover, we will seek for theoretical justifications and guarantees on SBO in high-dimensional settings.  We would like to also seek for a theoretical explanation of the failure modes.
