# Supplementary material for: Standard Gaussian Process is All You Need for High-Dimensional Bayesian Optimization
Source: arXiv:2402.02746 source file (2025-03-11)
Supplement: Supplementary file 2 [file appendix_zt.tex]

\section{Proofs}\label{sect:proof}
\subsection{Proof of Lemma~\ref{lem:tau-se} }
\begin{proof}
    We intend to solve $\rho^2/e^{\rho^2} < \xi$, which is equivalent to solving
    \[
     \log r - r < \log \xi, 
    \]
    where $r = \rho^2$. 
    We then leverage the fact that $\log r < \sqrt{r}$ when $r > 1$. Since $1/e > \xi$, we know the solution of $\rho$ must be larger than 1, implying that the solution for $r$ is larger than $1$. To meet the inequality, we can solve 
    \[
    \log r - r < \sqrt{r} - r < \log \xi. 
    \]
    It then converts to a quadratic form, 
    \begin{align}
        \sqrt{r} - \sqrt{r}^2 < \log \xi.
    \end{align}
    Note that $\rho = \sqrt{r}$.     It is straightforward to solve this inequality and we can obtain that the inequality holds when
    \[
    \rho > \tau_{\text{SE}} = \frac{1}{2} + \sqrt{\frac{1}{4} - \log \xi}. 
    \]
    
\end{proof}
\subsection{Proof of Lemma~\ref{lem:prob-bound}}\label{sect:bound-proof-1}
\begin{proof}
    First, since each $x_{ik}$ and $x_{jk}$ independently follow $\text{Uniform}(0, 1)$, it is straightforward to obtain $\EE[(x_{ik} - x_{jk})^2] = \frac{1}{6}$. 
    Let us define $\gamma = \|\x_i - \x_j\|^2$. Then we have $\EE[\gamma] = \frac{1}{6}d$.
    According to Hoeffding's inequality,  for all $t>0$,
    \begin{align}
        p(|\gamma - \frac{1}{6}d| \ge t) \le  2\exp\left(-\frac{2t^2}{d}\right). \label{eq:hoeff}
    \end{align}
    Since $\rho = 
    \frac{\sqrt{\gamma}}{\ell_0}$, we have  $p(\rho > \tau) = p(\gamma > \tau^2\ell_0^2)$. Since $d>6\ell_0^2\tau^2$, we set $t = \frac{1}{6}d - \ell_0^2\tau^2>0$, and apply \eqref{eq:hoeff} to obtain
    \[
    p(|\gamma - \frac{1}{6}d| \ge \frac{1}{6}d -  \ell_0^2\tau^2|) \le 2\exp\left(-\frac{2\left(\frac{1}{6}d -  \ell_0^2\tau^2\right)^2}{d}\right)
      = 2 \exp\left(-\frac{\left(d - 6\ell_0^2\tau^2\right)^2}{18d}\right),
    \]
    which is equivalent to
    \begin{align}
        p(|\gamma-\frac{1}{6}d| < \frac{1}{6}d - \ell_0^2\tau^2) > 1 - 2 \exp\left(-\frac{\left(d - 6\ell_0^2\tau^2\right)^2}{18d}\right).\label{eq:bound2}
    \end{align}
Since $p(\gamma > \ell_0^2 \tau^2) \ge p( \ell_0^2 \tau^2 < \gamma < \frac{1}{3}d - \ell_0^2 \tau^2) = 
p(|\gamma - \frac{1}{6}d| < \frac{1}{6}d - \ell_0^2\tau^2)$, combining with \eqref{eq:bound2} we obtain the bound
\[
p(\rho>\tau) = p(\gamma > \ell_0^2 \tau^2) > 1 - 2 \exp\left(-\frac{\left(d - 6\ell_0^2\tau^2\right)^2}{18d}\right).
\]
\end{proof}

\subsection{Proof of Lemma~\ref{lem:tau-matern}}
\begin{proof}
    To solve $\rho^2/e^{\sqrt{5}\rho} < \xi$, it is equivalent to solving
    \[
    \frac{1}{5} \frac{r^2}{e^r} < \xi, \;\;\; r = \sqrt{5}\rho,
    \]
    which is further equivalent to 
    \[
    \log \frac{1}{5} + 2 \log r - r < \log \xi. 
    \]
    We leverage $\log r < \sqrt{r}$ for $r>1$, and solve the upper bound, 
    \[
    \log\frac{1}{5} + 2 \sqrt{r}-r < \log \xi,
    \]
    which gives 
    \begin{align}
        \rho > \tau_{\text{Mat\'ern}} = \frac{1}{\sqrt{5}}\left(1 + \sqrt{1 + \log 1/5 - \log\xi}\right)^2.
    \end{align}
\end{proof}

\subsection{Proof of Lemma~\ref{lem:new-bound}}
\begin{proof}
    First, similar to the proof in Section~\ref{sect:bound-proof-1}, under the uniform distribution on $[0, 1]^d$, from Hoeffding's inequality, we have for all $t>0$,
        \begin{align}
        p(|\gamma - \frac{1}{6}d| \ge t) \le  2\exp\left(-\frac{2t^2}{d}\right). \label{eq:hoeff-again}
    \end{align}

    When we set $\ell_0 = c\sqrt{d}$ such that $c>1/ \sqrt{6}\tau$, we have $\ell_0^2 \tau^2 > d/6 $. Let us choose $t = \ell_0^2\tau^2 - d/6=c^2 \tau^2d - d/6>0$, and apply the Hoeffding's inequality~\eqref{eq:hoeff-again}, 
    \begin{align}
        p\left(|\gamma - d/6 | \ge \ell_0^2\tau^2 - d/6\right) \le 
        2\exp\left(-\frac{2(\ell_0^2\tau^2 - d/6)^2}{d}\right) = 2\exp\left(-2(c^2\tau^2 - \frac{1}{6})^2d\right)
    \end{align}
    Since $p(\rho \ge \tau) = p(\gamma \ge \ell_0^2\tau^2) \le p(|\gamma - d/6 | \ge \ell_0^2\tau^2 - d/6)$, we obtain
    \[
    p(\rho \ge\tau) \le 2\exp\left(-2(c^2\tau^2 - \frac{1}{6})^2d\right).
    \]
\end{proof}

\section{More Experiment Details}
\subsection{Definition of Synthetic Functions}\label{sect:syn-def}
%We denote the function forms and bounds we used in Sec \ref{sec:experiments} below.

\textbf{Stybtang}. We used the following slightly-modified Stybtang function, %The original Stybtang is in form $f(x)=\frac{1}{2}\sum_{i=1}^{D}(x_{i}^{4}-16x_{i}^{2}+5x_{i})$. Our version $f_{\text{V1}}$ is of form,
\[
f(\x)=\frac{1}{2}\sum_{i=1}^{D}\left((x_{i}-c_{i})^{4}-16(x_{i}-c_{i})^{2}+5(x_{i}-c_{i})\right),
\]
where $\x \in [-5, 5]^D$, and we set $[c_1, \dots, c_D]$ as an evenly spaced sequence in $[0, 7.5]$ ($c_1 = 0$ and $c_D = 7.5$). The optimum  is at $\x^\dagger=[c_1 -2.903534, \ldots, c_D - 2.903534]$.

\textbf{Rosenbrock}. 
We used the following Rosenbrock function, 
\[
f(\x)=\sum_{i=1}^{D-1}\left[100\left((x_{i+1}-c_{i+1})-(x_{i}-c_{i})^{2}\right)^{2}+\left(1 - (x_{i}-c_{i})\right)^2\right],
\]
where $\x \in [-2.048, 2.048]^{D}$. We set $[c_{1}, ..., c_D]$ as an evenly spaced sequence in $[-2, 2]$, where $c_{1}=-2$ and  $c_{D}=2$. The optimum is at $x^\dagger =  [c_{1}+1, ..., c_{D}+1]$. 

\textbf{Ackley}. We used the Ackley function defined in~\citep{simulationlib},
\[
f(\x)=-20\text{ exp}\left(-0.2\sqrt{\frac{1}{d}\sum_{i=1}^{d}x_{i}^{2}}\right)-\text{exp}\left(\frac{1}{d}\sum_{i=1}^{d}\text{cos}(2{\pi}x_{i})\right)+20+\text{exp}(1),
\]
where each $x_i \in [-32.768, 32.768]$ and the (global) optimum is at $x^{\dagger}=[0, \ldots, 0]$. 

\textbf{Hartmann6}. The function is given by
\[
f(\x)=-\sum_{i=1}^{4}{\alpha}_{i}{ \exp}\left(-\sum_{j=1}^{6}A_{ij}(x_{j}-P_{ij})^{2}\right),
\]
where each $x_i \in [0, 1]$, $\A=[A_{ij}]$ and $\P = [P_{ij}]$ are two pre-defined matrices as in \citep{simulationlib}.
The global optimum is at $\x^\dagger = [0.20169, 0.150011, 0.476874, 0.275332, 0.6573]$.

\begin{figure*}[!ht]
    \centering
    \includegraphics[width=\textwidth]{BO ICLR 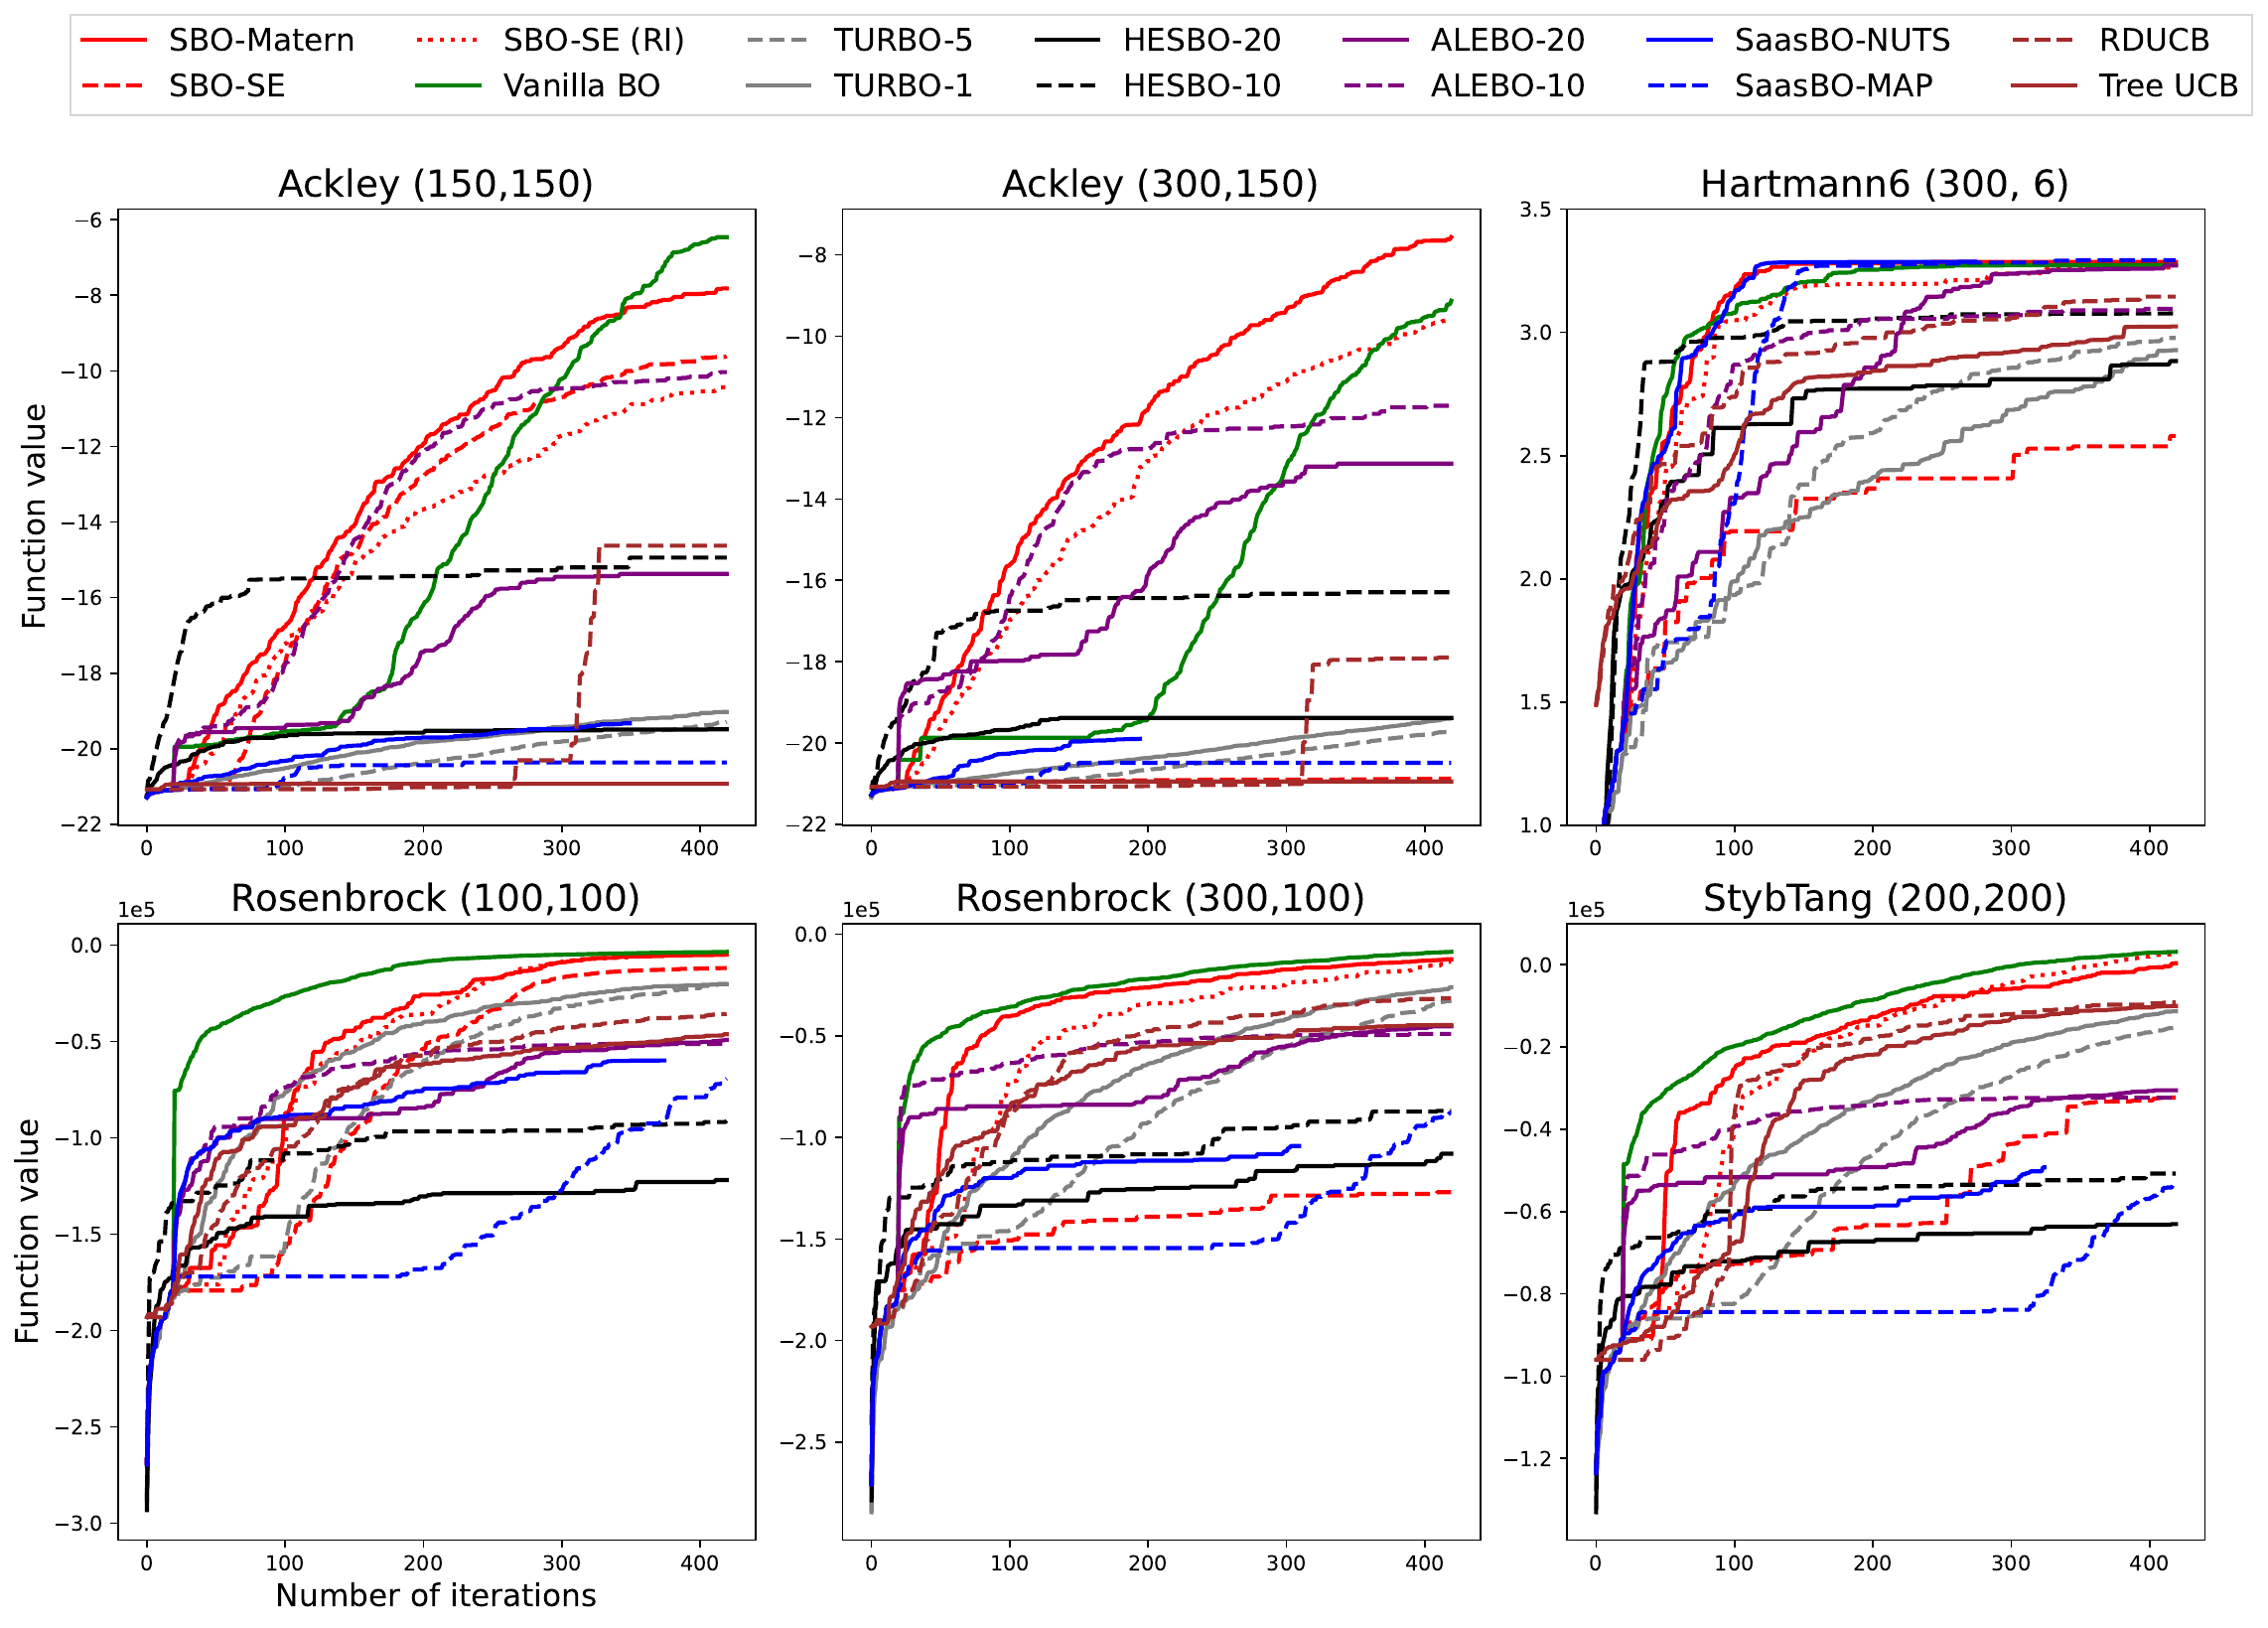}
    \caption{\small Runtime performance: Maximum Function Value Obtained \textit{vs.} Number of Steps in synthetic benchmarks. The results were averaged from 10 runs. }
    \label{fig:syn-running-plot}
\end{figure*}

\begin{figure*}[!ht]
    \centering
    \includegraphics[width=\textwidth]{BO ICLR 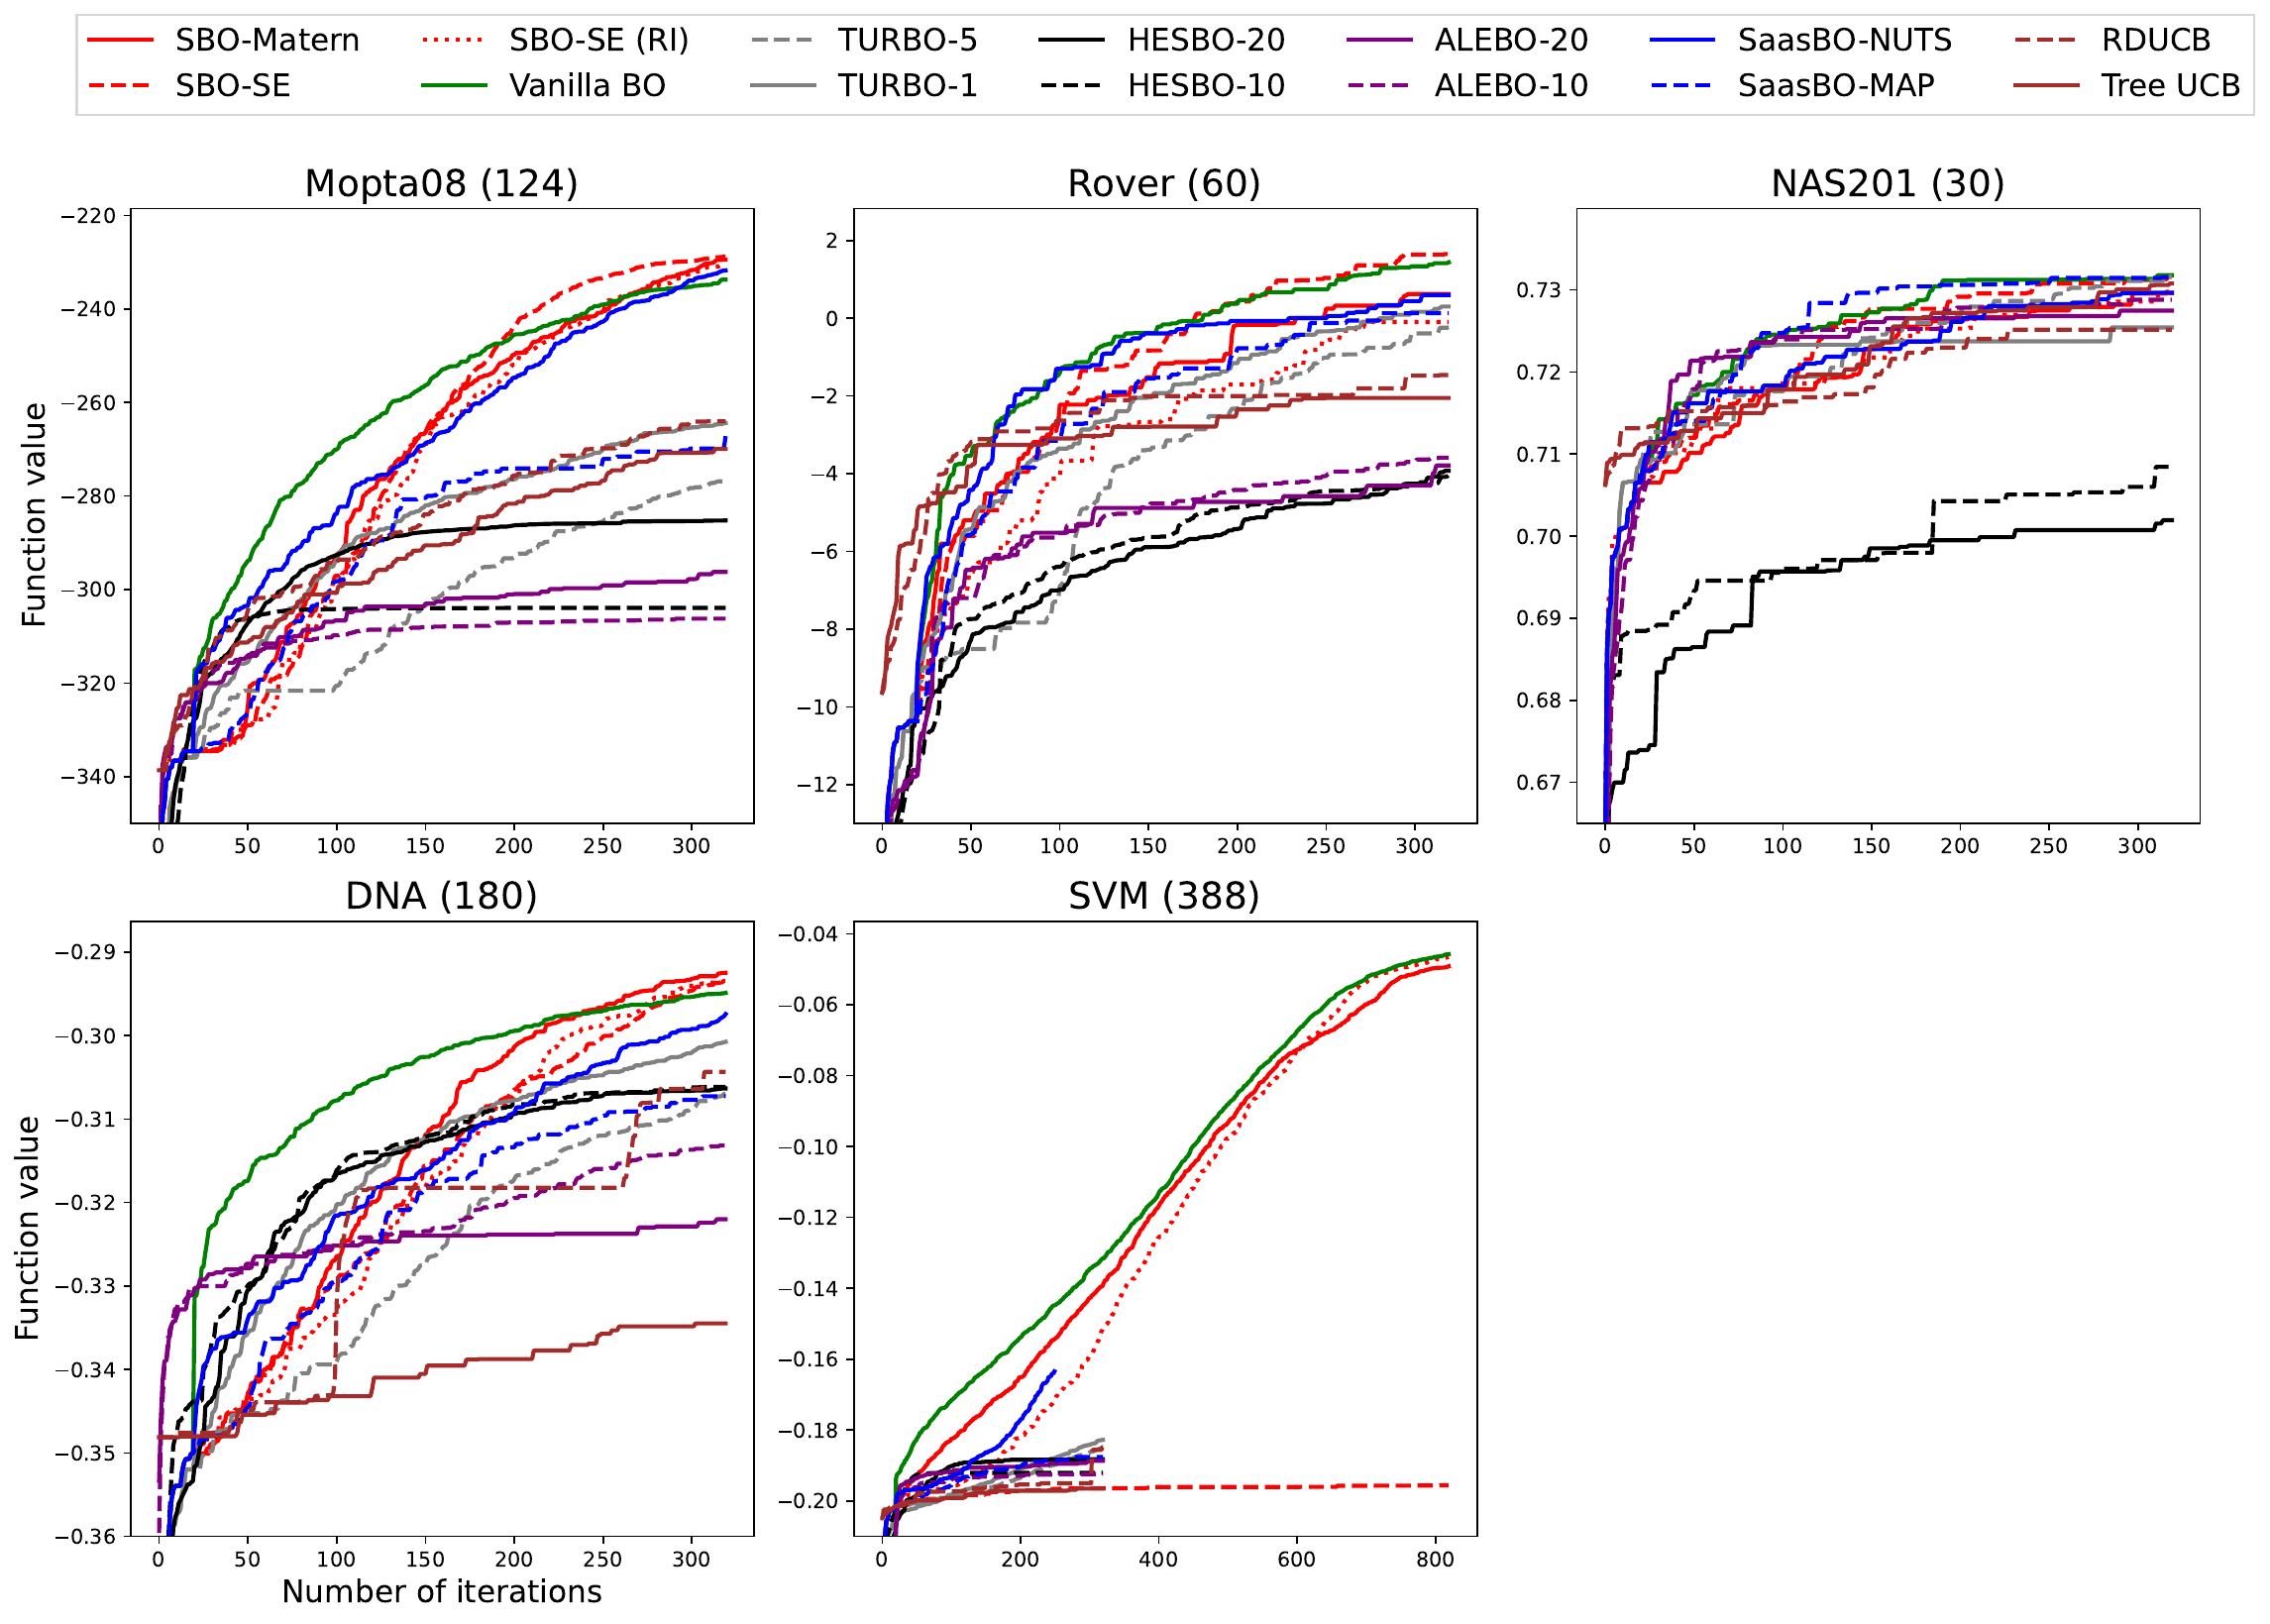}
    \caption{\small Runtime performance: Maximum Function Value Obtained \textit{vs.} Number of Steps in real-world benchmarks. The results were averaged from 10 runs.}
    \label{fig:running-real}
\end{figure*}

\begin{figure*}[!ht]
    \centering
    \includegraphics[width=\textwidth]{BO ICLR 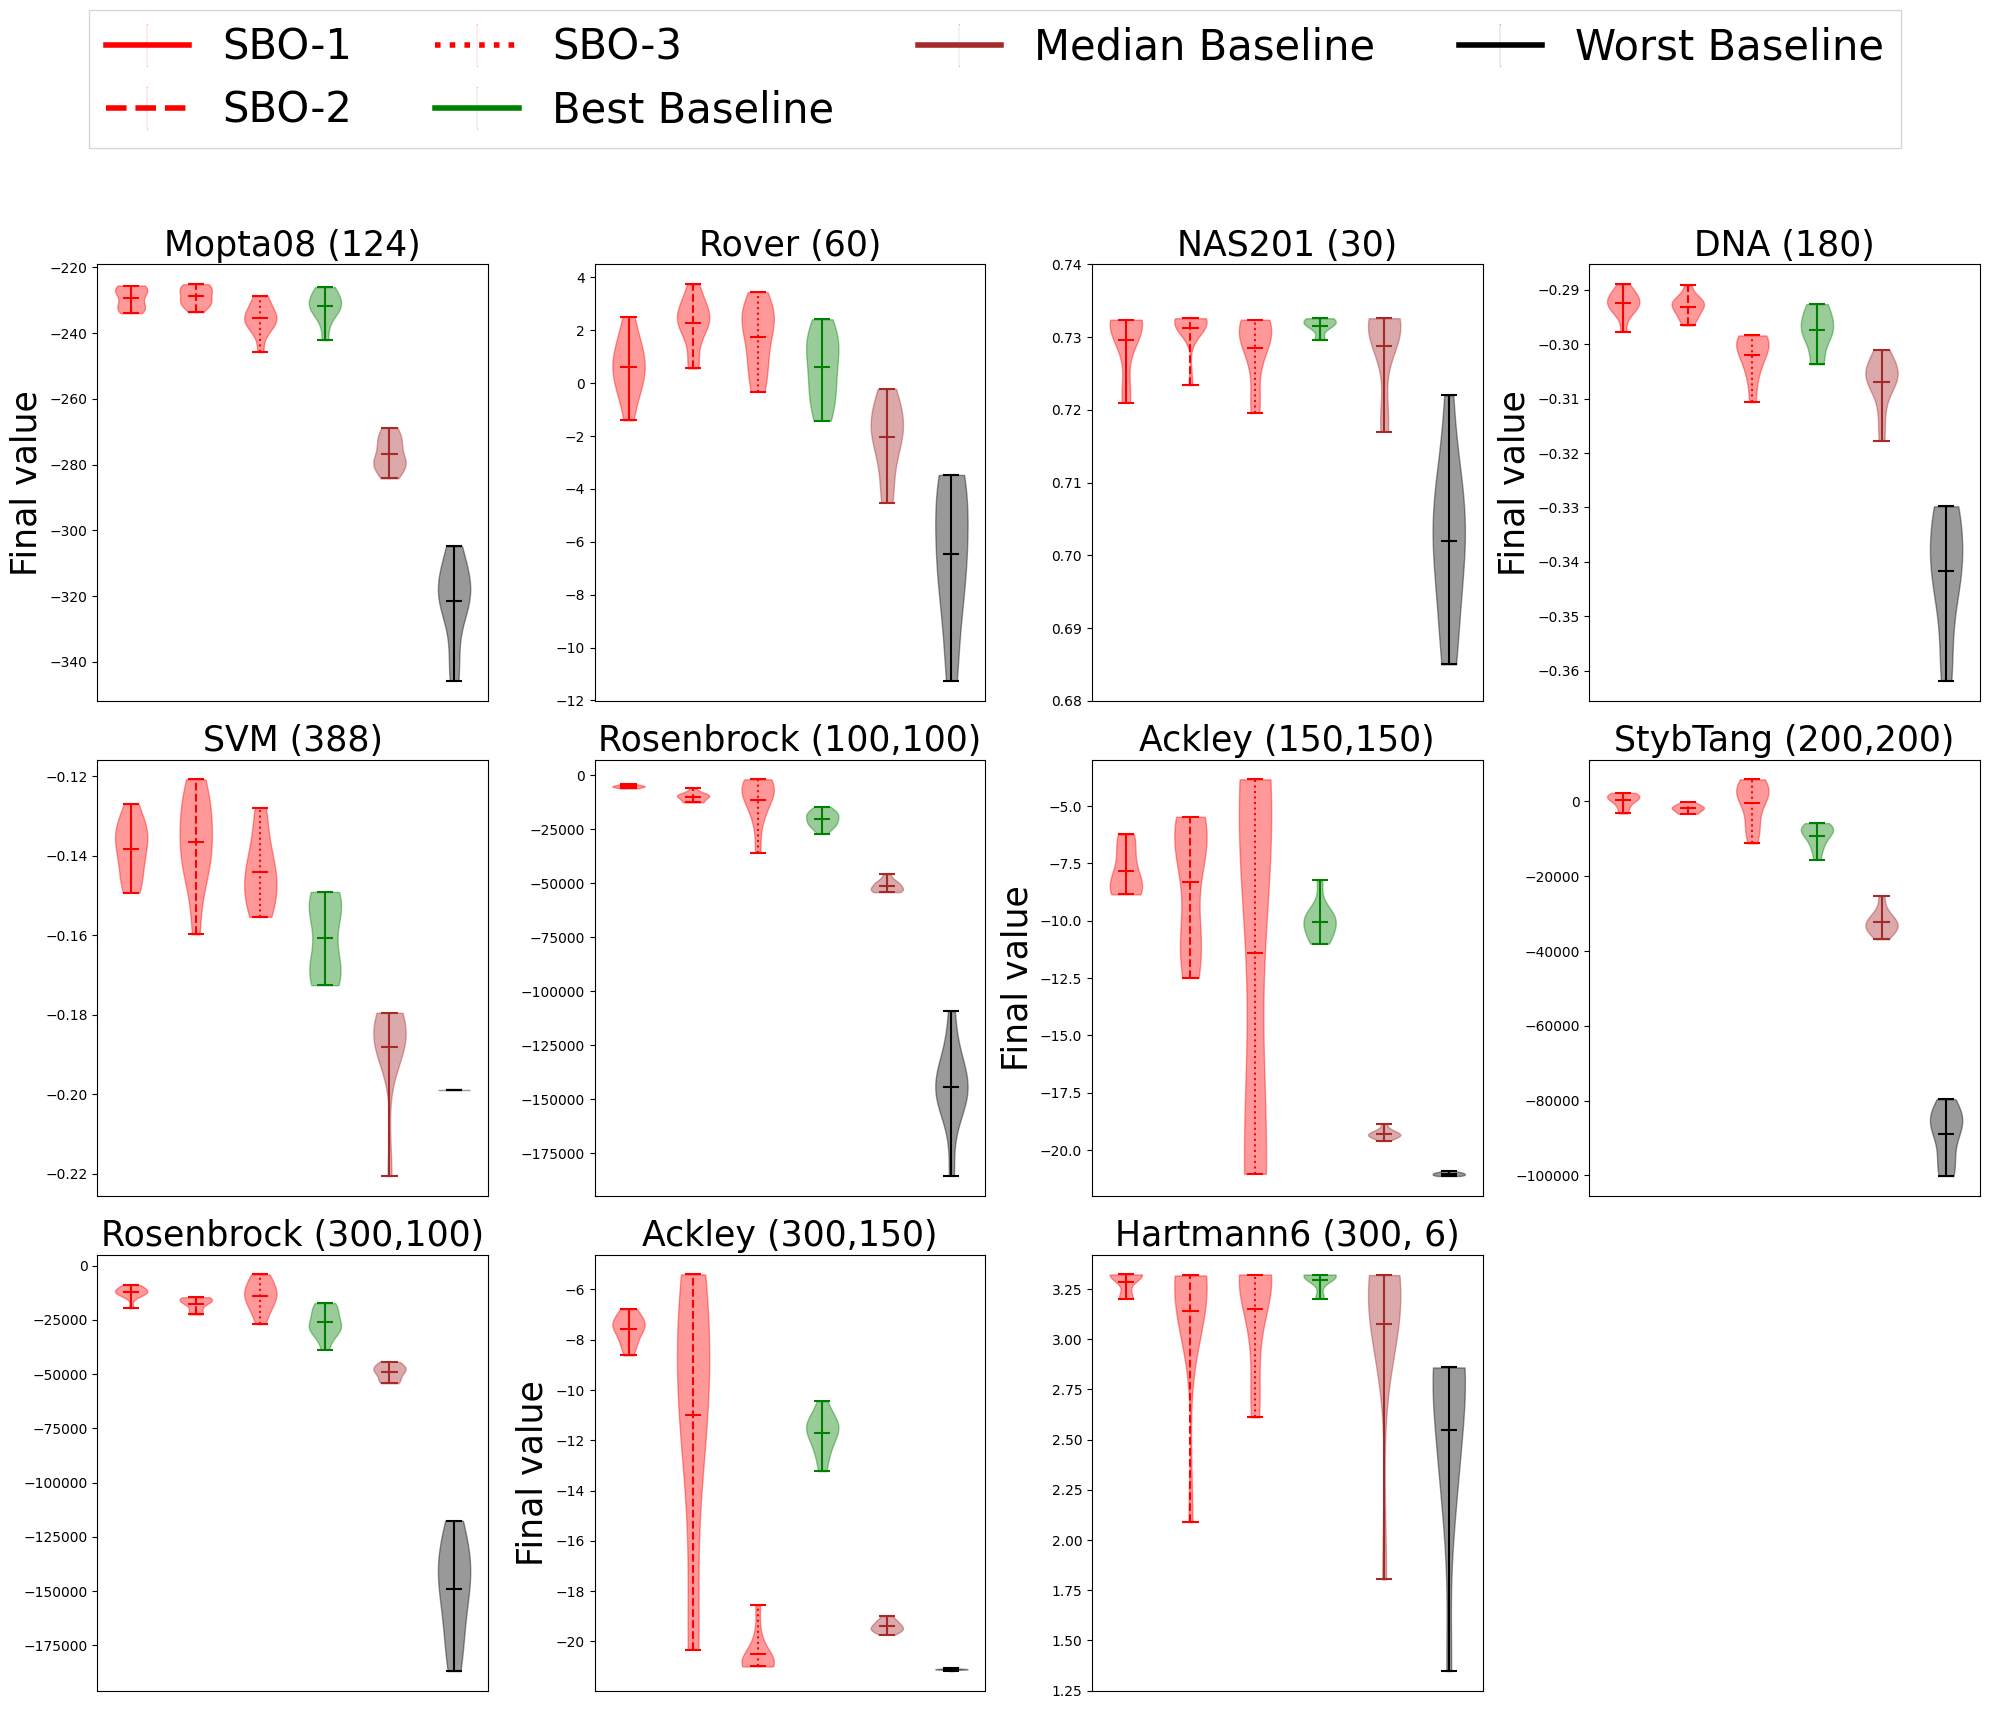}
    \caption{\small Ultimate optimization performance: Maximum Function Value obtained at the end of optimization loop, including SBO-3, namely training with a single length-scale parameter in Mat\'ern-5/2 kernel. The results were collect from 10 runs.}
    \label{fig:final-all-sbo3}
\end{figure*}
\begin{figure*}[!ht]
    \centering
    \includegraphics[width=\textwidth]{BO ICLR 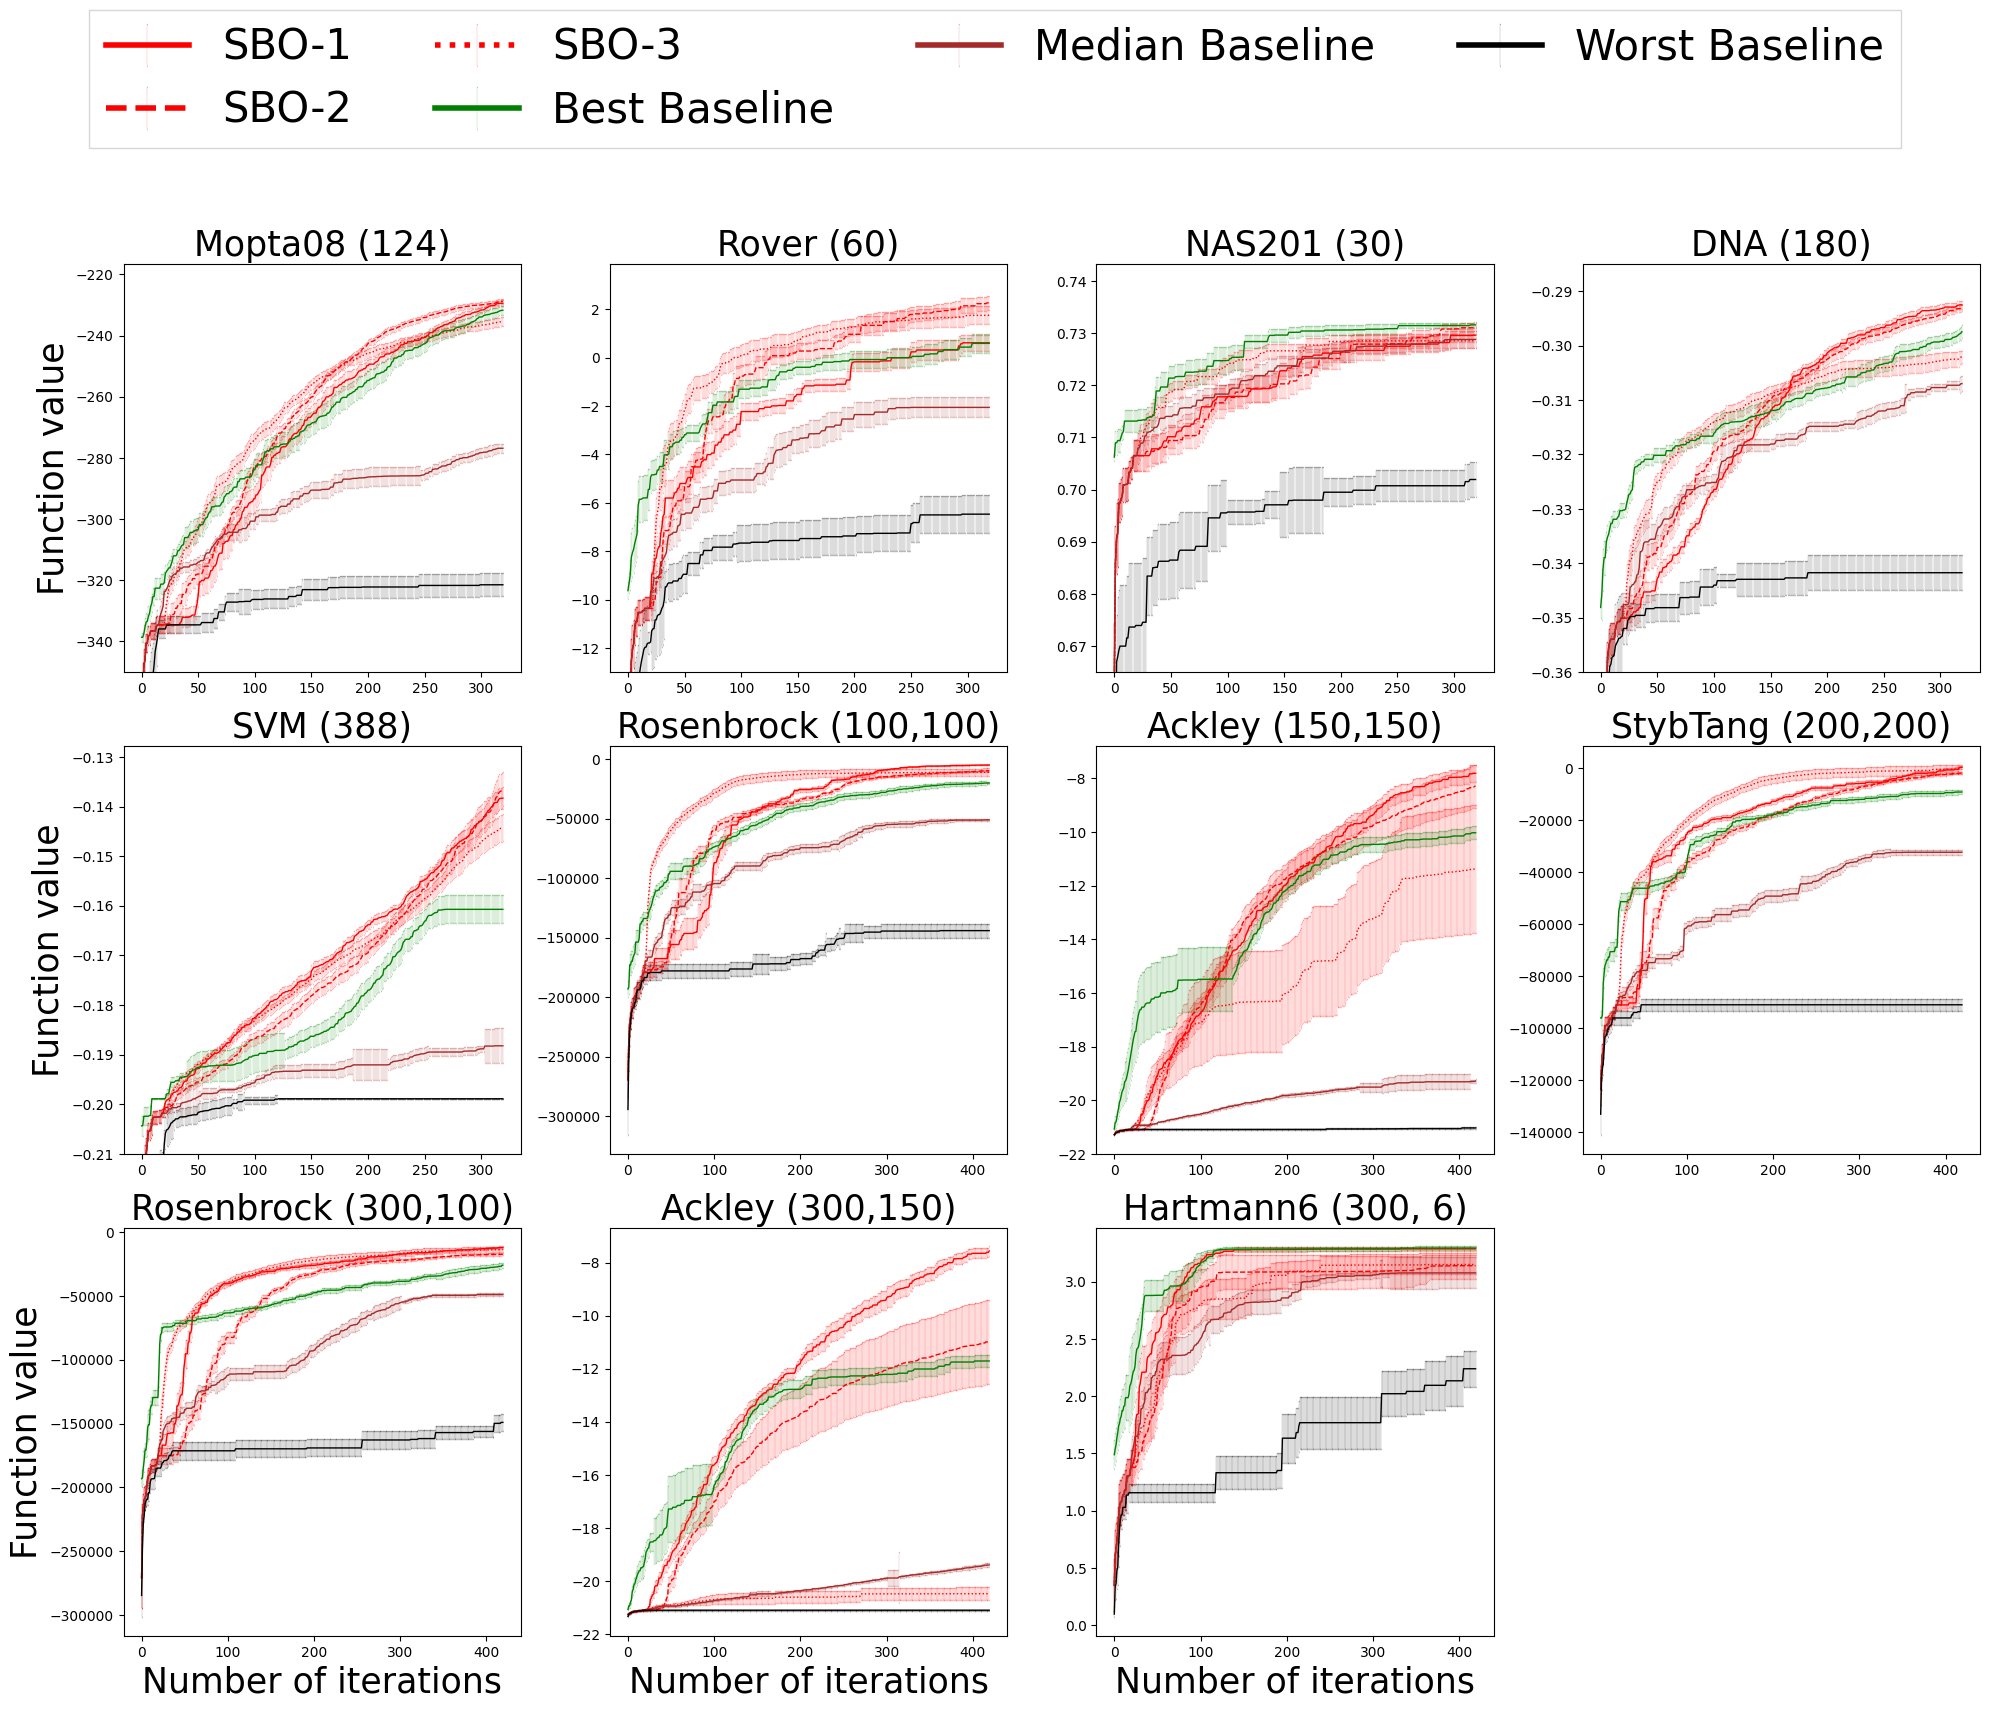}
    \caption{\small Runtime performance: Maximum Function Value obtained \textit{vs.} Number of Steps in real-world benchmarks, including SBO-3, namely training with a single length-scale parameter in Mat\'ern-5/2 kernel. The results were averaged from 10 runs. The shaded region depicts the standard deviation. }
    \label{fig:running-all-with-std-sbo3}
\end{figure*}

\subsection{Implementation}\label{sect:impl}
\begin{itemize}
    \item \textbf{ALEBO.} We used ALEBO implementation shared by the  Adaptive Experimentation (AX) Platform  (version 0.2.2). The source code is at  \url{https://github.com/facebook/Ax/blob/main/ax/models/torch/alebo.py}.
    \item \textbf{HESBO.} We used HESBO implementation of the original authors (\url{https://github.com/aminnayebi/HesBO}).
    \item \textbf{TURBO.} We used the original TURBO implementation (\url{https://github.com/uber-research/TuRBO})
    \item \textbf{SaasBO-NUTS.} We used the original implementation of the authors  (\url{https://github.com/martinjankowiak/saasbo}). %and the re-implementation in BoTorch. The original implementation yield better result, but with a higher runtime. All reported experiment results is from original implementation.
    \item \textbf{SaasBO-MAP.} The SaasBO implementation available to the public does not include the version using MAP estimation.  We therefore implemented this method based on the original paper~\citep{eriksson2021highdimensional}. All the hyperparameter settings follow exactly the same as the original paper.
    \item \textbf{RDUCB and Tree UCB.} The implementation of both methods is publicly available at \url{https://github.com/huawei-noah/HEBO/tree/master/RDUCB}.
    \item \textbf{BNN Laplace and BNN HMC.} {For BNN Laplace, we used the implementation at \url{https://github.com/wiseodd/laplace-bayesopt}, and for BNN HMC, we used the implementation at \url{https://github.com/yucenli/bnn-bo}. To identify the architecture of the neural network, we perform leave-one-out cross-validation on the initial dataset for each task. The layer width and depth were selected from \{1, 2, 3\} $\times$ \{32, 64, 128, 256\}. The activation function for BNN Laplace is ReLU and for BNN HMC is Tanh, which is the default choice of each method. For BNN Laplace, the training was conducted by maximizing marginal likelihood with ADAM, with learning rate of 1E-01, and weight decay of 1E-03. For HMC, the BNN is pre-trained by maximizing log likelihood with ADAM. Then followed by HMC sampling procedure. We used their adaptive step size schedule for the Leap frog, and the number of steps was set to 100.}
\end{itemize}

\subsection{Computing Environment}
\label{sect:compute-env}
We conducted the experimental investigations on a large computer cluster equipped with Intel Cascade Lake Platinum 8268 chips.

\begin{table*}[h!]
\small
\centering
\begin{tabular}{lrrrrr}
\toprule
{} &  Mopta08 (124) &   Rover (60) &  NAS201 (30) &   DNA (180) &    SVM (388) \\
\midrule
{ARD Mat\'ern-MAP} &    7.39 &    9.99 &    7.81 &    9.77 &    13.55 \\
{ARD Mat\'ern-MLE} &    11.23 &    9.84 &    5.76 &    14.34 &    32.16 \\
{ARD Mat\'ern-NUTS}&    492.62 &   404.17  &   393.62  &   575.03  &   768.29\\
{SaasBO-MAP        } &    46.53 &   41.36 &   42.35 &    51.33 &    67.37 \\
{SaasBO-NUTS          } &   985.76 &  375.06 &  229.07 &  1739.56 &  2269.50 \\
\bottomrule
\end{tabular}
\caption{Average running time (in seconds) per optimization step in real-world benchmark tasks.}
\label{tb:real-runtime}
\end{table*}
\begin{table*}[h!]
\small
\centering
\begin{tabular}{lcccccc}
\toprule
    {} &  Rosenbrock &   Ackley &  Stybtang &  Rosenbrock &  Ackley &  Hartmann6 \\
     & (100,100) & (150, 150) & (200, 200) & (300, 100) & (300, 150) & (300, 6) \\
    \midrule
    {ARD Mat\'ern-MAP} &           8.52 &    36.26 &        21.42 &             16.36 &       25.90 &       51.56 \\
    {ARD Mat\'ern-MLE} &           8.85 &    12.94 &        13.67 &             12.63 &       9.99 &       8.81 \\
    {ARD Mat\'ern-NUTS} &   857.21  &   850.23  &   1120.28 &   1276.42 &   1049.78 &   948.25\\
    {SaasBO-MAP       } &          70.17 &    70.69 &        66.35 &            100.79 &      85.86 &      85.72 \\
    {SaasBO-NUTS            } &        1294.90 &  1621.60 &      1511.99 &           1938.53 &     925.80 &    2204.54 \\
\bottomrule
\end{tabular}
\caption{\small Average running time (in seconds) per optimization step on synthetic benchmark tasks.}
\label{tb:syn-runtime}
\end{table*}

%\begin{wraptable}{r}{0.55\textwidth}
\begin{table}
%\vspace{-0.15in}
\centering
\small
\begin{tabular}{c | c} 
\hline\hline
 \textit{Method} & \textit{Structural Assumption} \\
 \hline
   ALEBO, HESBO & {Low-dim embedding} \\ 
  %\hline
  SaasBO & Partial variable dependency\\ 
%\hline
 RDUCB, Tree UCB & Additive function decomposition \\
% \hline
  SBO, TURBO, BNN & None\\ \hline
\end{tabular}
\caption{\small BO methods and their structural assumption about the target function.} \label{tb:method-assumptions}
\label{table:1}
\end{table}
%\vspace{-0.1in}
%\end{wraptable}

\begin{figure*}[t]
    \centering
    \includegraphics[width=\textwidth]{BO ICLR 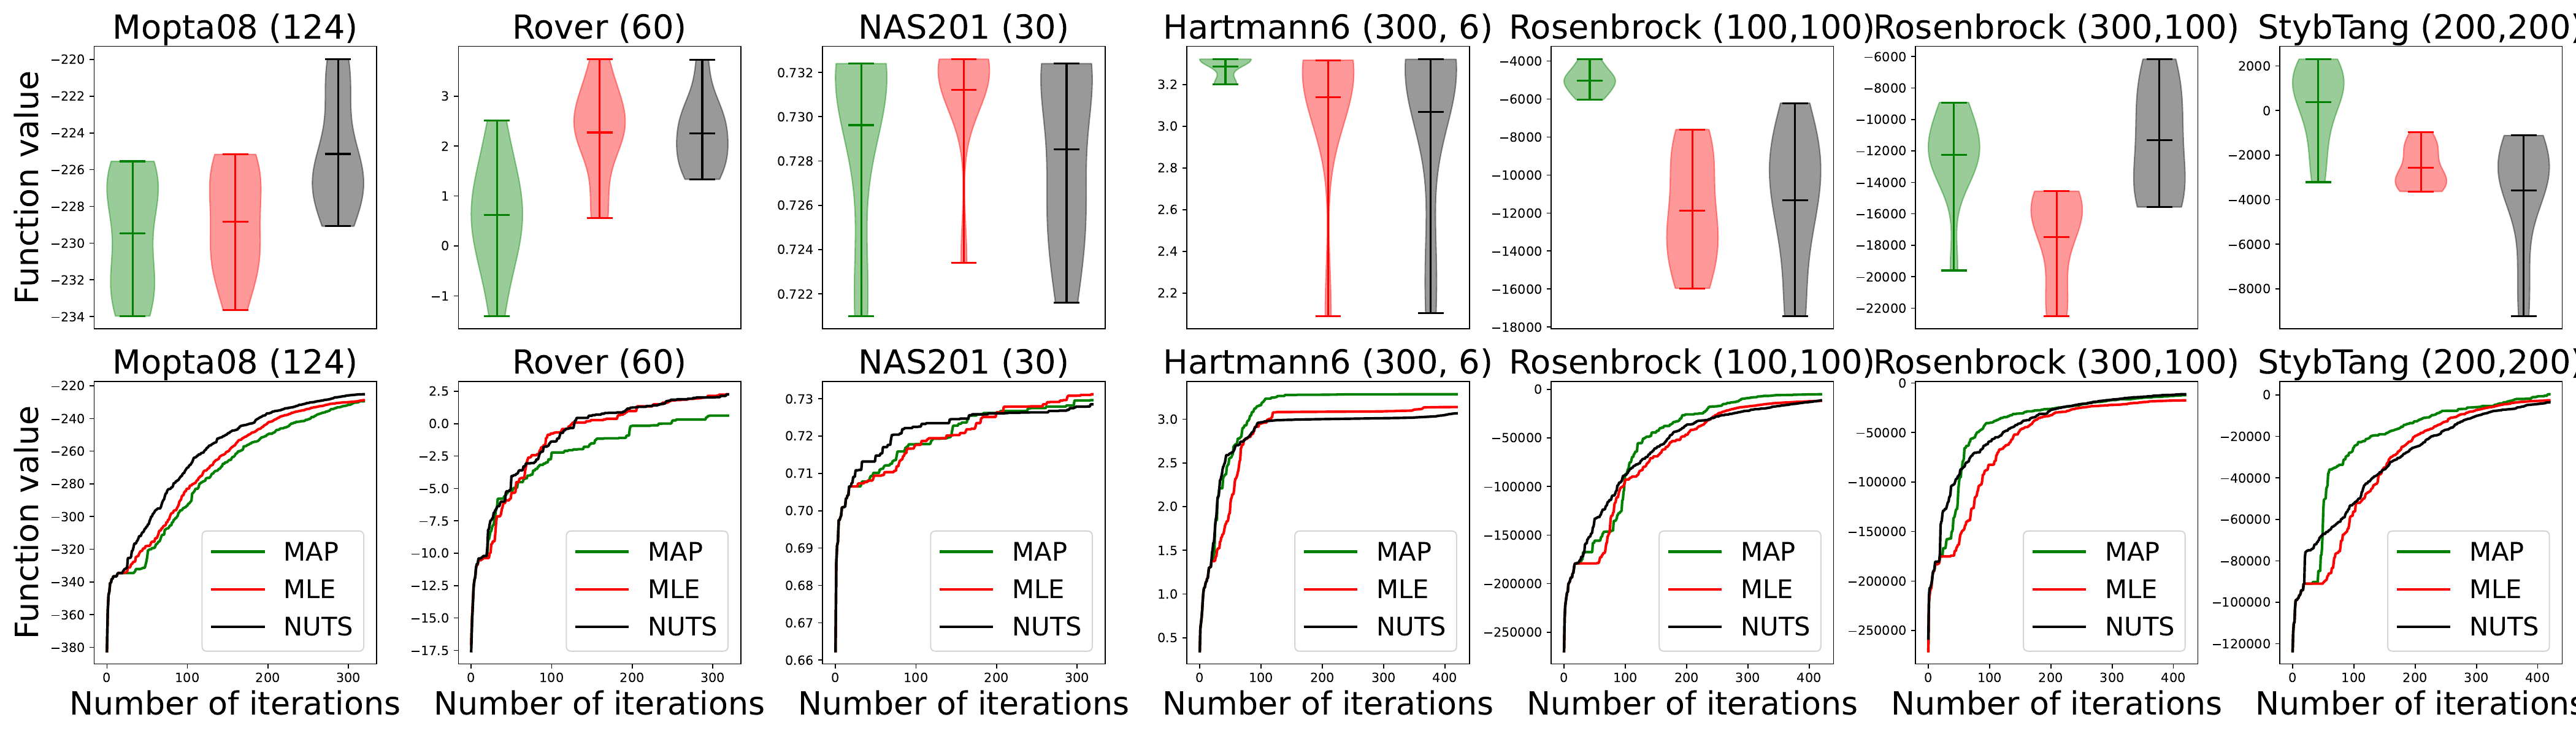}
    \caption{\small Optimization performance using MLE training,  MAP training with a diffuse prior over the length-scale parameters, and  NUTS on the rest of benchmarks. The results were summarized from 10 runs.}
    \label{fig:op-performance-gpard-nuts-rest}
\end{figure*}

\section{Additional Ablation Studies}\label{sect:fail}

In this section, we conducted a careful ablation study to investigate alternative popular  settings in executing standard BO.  From these settings, we identified a few failure modes during high-dimensional optimization. We provided analysis and discussions accordingly. 

\subsection{GP Training}
First, we examined MLE training with LBFGS. We found that, however, LBFGS often incurs numerical issues, and cannot reliably finish model training. This is consistent with the report in other works~\citep{hvarfner2024vanilla}. The issue might be because that without constraints (or regularization) over the parameters (such as the length-scales and amplitude), the exploration of LBFGS tends to be overly aggressive, which easily cause numerical problems. Hence, using stochastic optimization, like ADAM, might be a wise choice for MLE training.

Second, we examined MAP training with alternative prior choices over the length-scale parameters. In the main paper, we use a diffuse prior, \texttt{Uniform(0.001, 30)}. In practice, another commonly used choice is a concentrated Gamma prior, \eg \texttt{Gamma(3, 6)}, which is the default choice in the popular BO library BoTorch. To see how it is concentrated, in Fig. \ref{fig:pdf} we compare its probability density curve with other priors, including the aforementioned uniform prior and the diffuse Gamma priors over the amplitude and noise variance. 

We found that employing a concentrated prior over the length-scale parameters will severely deteriorate the high-dimensional optimization performance. 
As shown in Fig \ref{fig:runtime-Gamma36}, after placing the prior Gamma(3,6) over each length-scale parameter, both the ultimate and runtime optimization performance  drops substantially across many tasks, such as Mopta08 (124), SVM (388) and Ackley(150, 150), no matter using ADAM or LBFGS to conduct training. To figure out the reason, we further investigated the surrogate learning performance. Following the same setting as in Fig. \ref{fig:pred-alignment}, we examined the prediction alignment after applying the prior Gamma(3,6) over the length-scale parameters. As depicted in Fig. \ref{fig:alignment-more} (third and fourth column), this concentrated prior leads to a severe prediction deviation from the ground-truth, indicating failure in learning the target function. This is consistent with the report in the SaasBO paper~\citep{eriksson2021highdimensional} (see Fig.1 of that paper). 
The quantitative results shown in Table \ref{tb:mse-surrogate-gamm36} and \ref{tb:test-ll-surrogate-gamma36} further confirm the substantially worse prediction accuracy as compared with GP training with a diffuse prior. {In addition, we notice that the previous work\citep{li2024study} have also tested standard BO using Gamma(3,6) as the prior over the length-scale parameters. In their high-dimensional optimization experiments (see Fig. 5 of that paper), standard BO performs badly. We used our setting (SBO-1 and SBO-2) to re-run one experiment that maximizes a high-dimensional polynomial function. It turns out that both SBO-1 and SBO-2 can surpass the best method I-BNN reported by that paper.   } 

Together these results have shown that a concentrated prior can severely limit GP's capacity for high-dimensional function estimation, leading to inferior performance in high-dimensional optimization.

\begin{figure*}[!ht]
    \centering
    \includegraphics[width=\textwidth]{BO ICLR 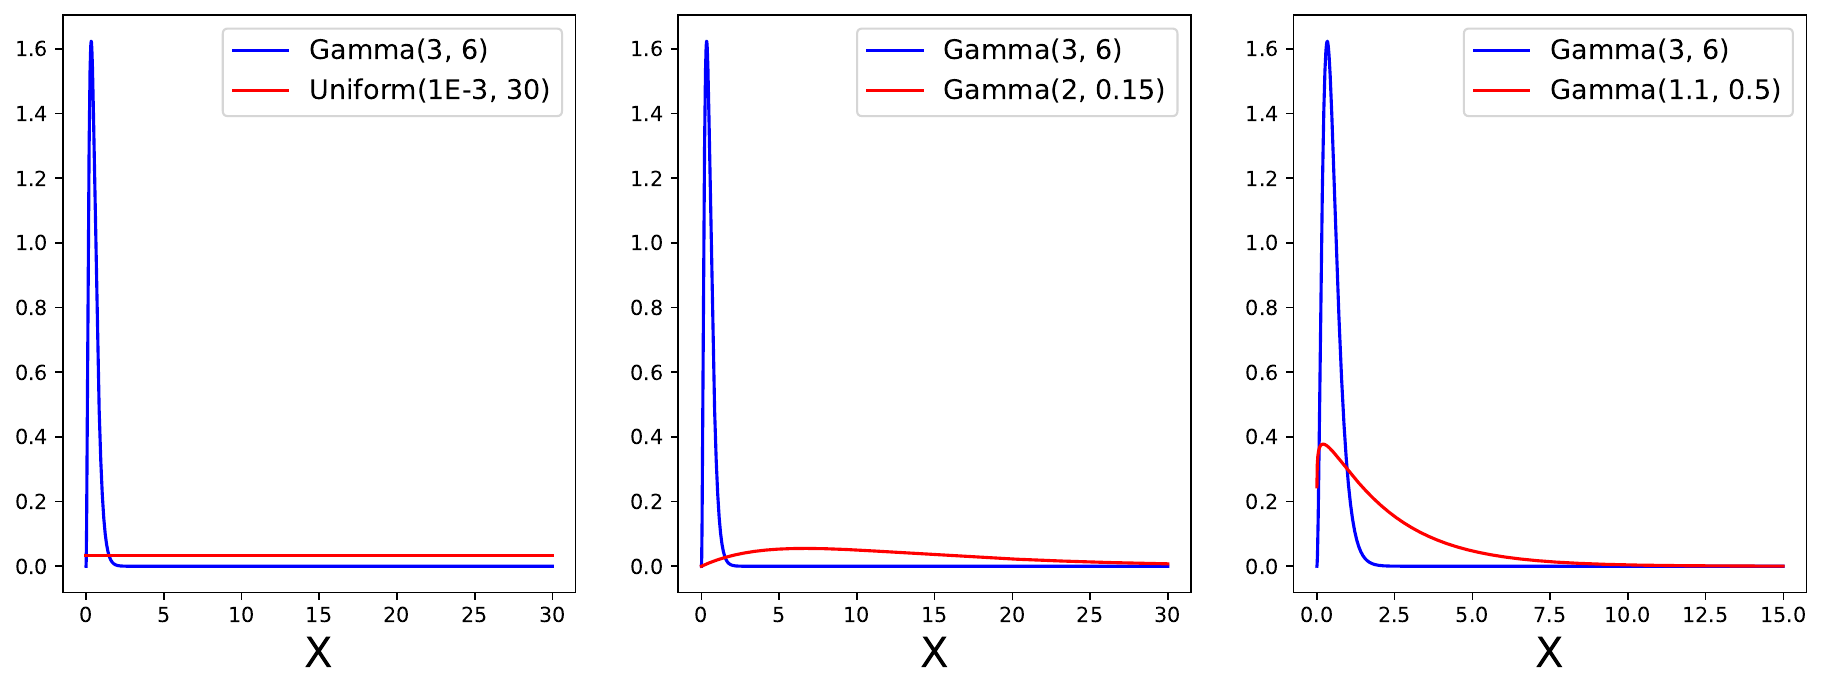}
    \caption{\small Probability density curves. Gamma(2, 0.15) and Gamma(1.1, 0.5) are the priors for the amplitude and noise variance, respectively.}
    \label{fig:pdf}
\end{figure*}

%\xuc{Also in 5.1, Fig. 1 of SaasBO \cite{eriksson2021highdimensional}, the only setting that could reproduce such a bad GP surrogate performance is using Gamma(3, 6) prior over length-scale, as shown in Fig. \ref{fig:gp-surrpgate-SaasBO}}

\begin{figure*}[!ht]
    \centering
    \includegraphics[width=\textwidth]{BO ICLR 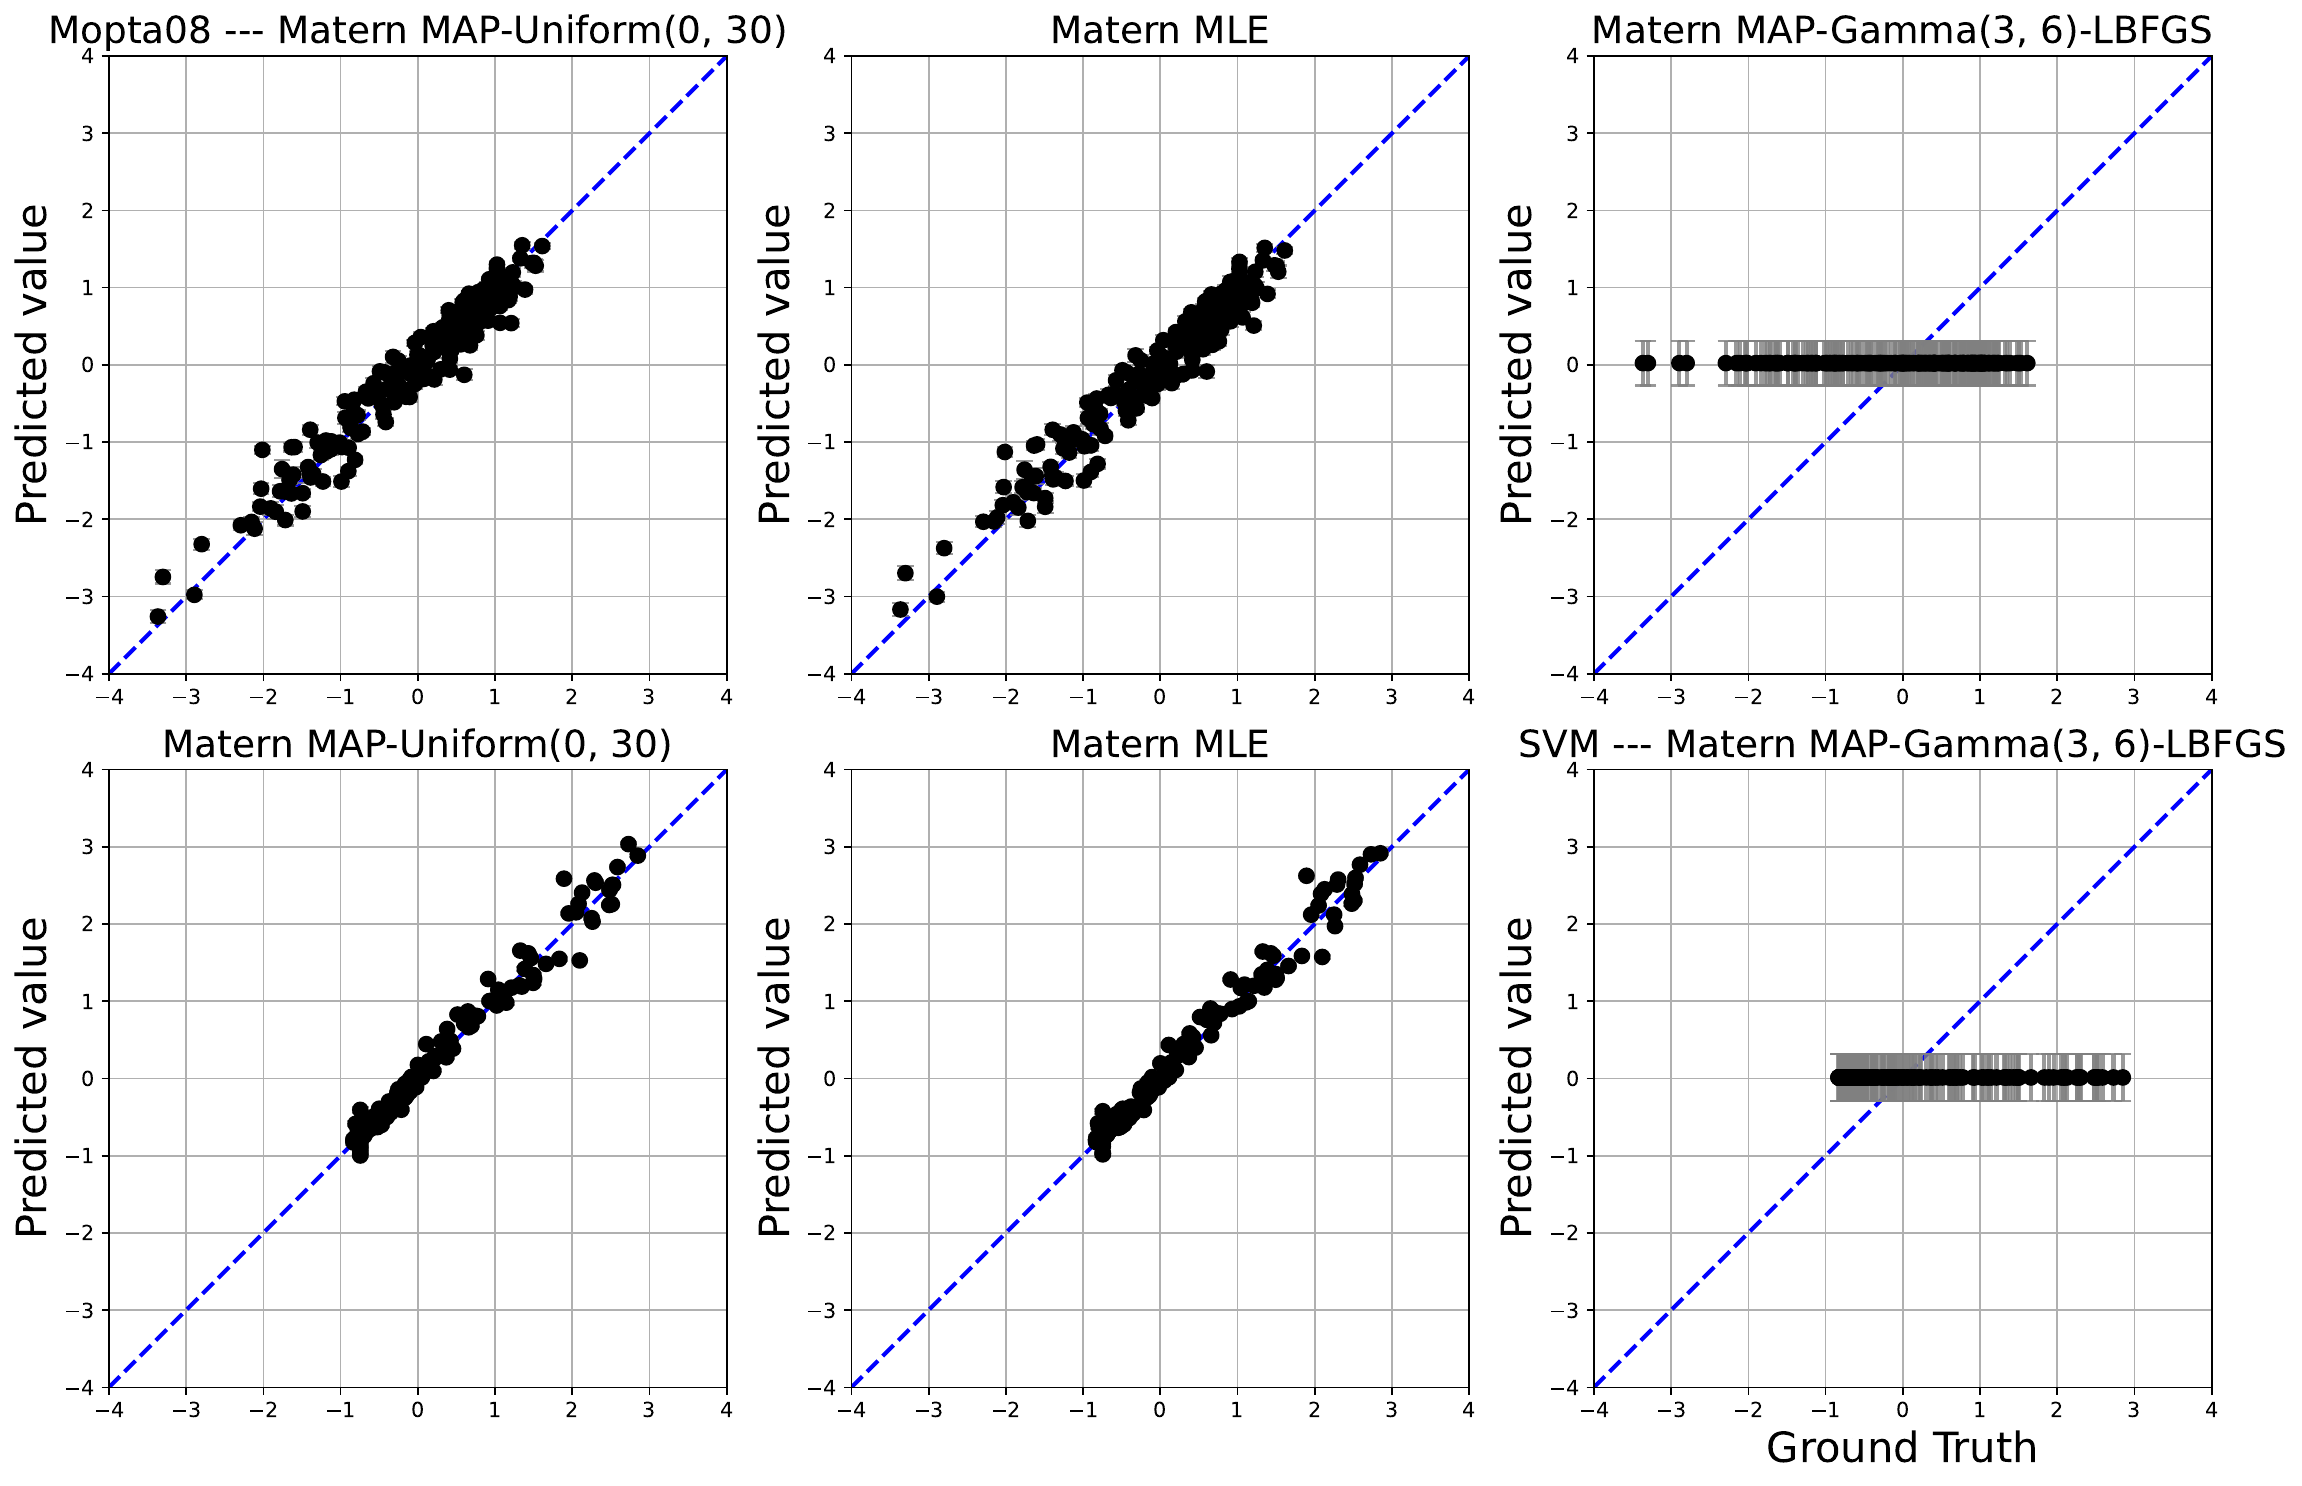}
    \caption{\small Alignment between the prediction (y-axis) and ground-truth function values (x-axis). \cmt{Reproducing GP surrogate performance in SaasBO. We used the same benchmark functions as Fig. 1 of SaasBO\cite{eriksson2021highdimensional}. The first row is Mopta08, which has 124 dimensions. The second row is SVM, which has 388 dimensions.}}
    \label{fig:alignment-more}
\end{figure*}

\begin{table*}[h!]
\small
\centering
\begin{tabular}{lcccc}
\toprule
%{\textit{Task}} &   MLE &  MAP-Uniform(1E-3, 30) &  MAP-Gamma(3, 6)-LBFGS  &  MAP-Gamma(3, 6)-ADAM \\
\multirow{2}{*}{\textit{Task}} &   \multirow{2}{*}{MLE} &  \multirow{2}{*}{MAP-Uniform(1E-3, 30)} &  MAP-Gamma(3, 6)  &  MAP-Gamma(3, 6) \\
& & & LBFGS & ADAM\\
\midrule
{Mopta08(124)}      & \textbf{0.034}$\pm$0.006 & 0.035$\pm$0.005 & 0.837$\pm$0.112 & 0.856$\pm$0.114 \\
{Rover(60)}         & 0.327$\pm$0.078 & \textbf{0.323}$\pm$0.075 & 0.78$\pm$0.154 & 0.819$\pm$0.115 \\
{DNA(180)}          & \textbf{0.149}$\pm$0.038 & 0.166$\pm$0.049 & 1.014$\pm$0.097 & 1.026$\pm$0.101 \\
{SVM(388) }         & \textbf{0.034}$\pm$0.01 & 0.039$\pm$0.01 & 1.057$\pm$0.066 & 1.06$\pm$0.067 \\
{Ackley(150, 150)}  & \textbf{0.017}$\pm$0.008 & 0.026$\pm$0.007 & 0.019$\pm$0.004 & 0.019$\pm$0.005 \\
{Ackley(300, 150)}  & \textbf{0.023}$\pm$0.006 & 0.07$\pm$0.047 & 0.431$\pm$0.09 & 0.459$\pm$0.092 \\
{Hartmann6(300, 6)} & \textbf{0.017}$\pm$0.013 & 0.178$\pm$0.325 & 0.881$\pm$0.045 & 0.906$\pm$0.034 \\
{Rosenbrock(100, 100)} & 0.084$\pm$0.013 & \textbf{0.081}$\pm$0.012 & 0.9$\pm$0.156 & 0.925$\pm$0.172 \\
{Rosenbrock(300, 100)} & \textbf{0.09}$\pm$0.064 & 0.116$\pm$0.078 & 0.971$\pm$0.222 & 1.001$\pm$0.217 \\
{Stybtang(200, 200)} & \textbf{0.043}$\pm$0.018 & 0.054$\pm$0.024 & 0.698$\pm$0.05 & 0.732$\pm$0.034 \\
\bottomrule
\end{tabular}
\caption{Mean Squared Error(MSE) averaged from five runs. The best results are bolded.  \cmt{of GP surrogate model based on different training settings. The results were averaged over five runs. Top 1 best method is bolded. For MAP estimation, we place Uniform prior and Gamma prior over lengthscales. For Uniform prior, we set it as Uniform(1E-10, 30.0). For Gamma prior, we set it as Gamma(3.0, 6.0).}}
\label{tb:mse-surrogate-gamm36}
\end{table*}

\begin{table*}[h!]
\small
\centering
\begin{tabular}{lcccc}
\toprule
%{\textit{Task}} &   MLE &  MAP-Uniform(1E-3, 30) & MAP-Gamma(3, 6)-LBFGS  &  MAP-Gamma(3, 6)-ADAM \\
\multirow{2}{*}{\textit{Task}} &   \multirow{2}{*}{MLE} &  \multirow{2}{*}{MAP-Uniform(1E-3, 30)} &  MAP-Gamma(3, 6)  &  MAP-Gamma(3, 6) \\
& & & LBFGS & ADAM\\
\midrule
{Mopta08(124)}      & \textbf{0.57}$\pm$0.08 & 0.542$\pm$0.104 & -1.337$\pm$0.058 & -1.715$\pm$0.212 \\
{Rover(60)}         & \textbf{-0.975}$\pm$0.216 & -1.062$\pm$0.286 & -1.24$\pm$0.111 & -1.322$\pm$0.073 \\
{DNA(180)}          & \textbf{-0.256}$\pm$0.261 & -0.388$\pm$0.35 & -1.426$\pm$0.054 & -2.026$\pm$0.183 \\
{SVM(388) }         & \textbf{0.581}$\pm$0.119 & 0.504$\pm$0.128 & -1.453$\pm$0.038 & -2.095$\pm$0.129 \\
{Ackley(150, 150)}  & 0.428$\pm$0.222 & 0.14$\pm$0.218 & \textbf{0.451}$\pm$0.088 & 0.445$\pm$0.087 \\
{Ackley(300, 150)}  & \textbf{0.232}$\pm$0.155 & -0.257$\pm$0.528 & -1.006$\pm$0.091 & -1.037$\pm$0.087 \\
{Hartmann6(300, 6)} & \textbf{1.2}$\pm$0.169 & 0.67$\pm$0.867 & -1.344$\pm$0.029 & -1.618$\pm$0.128 \\
{Rosenbrock(100, 100)} & \textbf{0.64}$\pm$0.081 & 0.606$\pm$0.1 & -1.308$\pm$0.083 & -1.598$\pm$0.42 \\
{Rosenbrock(300, 100)} & \textbf{0.518}$\pm$0.225 & 0.347$\pm$0.325 & -1.411$\pm$0.134 & -1.967$\pm$0.413 \\
{Stybtang(200, 200)} & \textbf{0.574}$\pm$0.164 & 0.421$\pm$0.228 & -1.251$\pm$0.017 & -1.41$\pm$0.067 \\
\bottomrule
\end{tabular}
\caption{Test log likelihood averaged from five runs. The best results are bolded. \cmt{of GP surrogate model based on different training settings. The results were averaged over five runs. Top 1 best method is bolded. For MAP estimation, we place Uniform prior and Gamma prior over length-scales. For Uniform prior, we set it as Uniform(1E-10, 30.0). For Gamma prior, we set it as Gamma(3.0, 6.0).}}
\label{tb:test-ll-surrogate-gamma36}
\end{table*}

\begin{figure*}[!ht]
    \centering
    \includegraphics[width=\textwidth]{BO ICLR 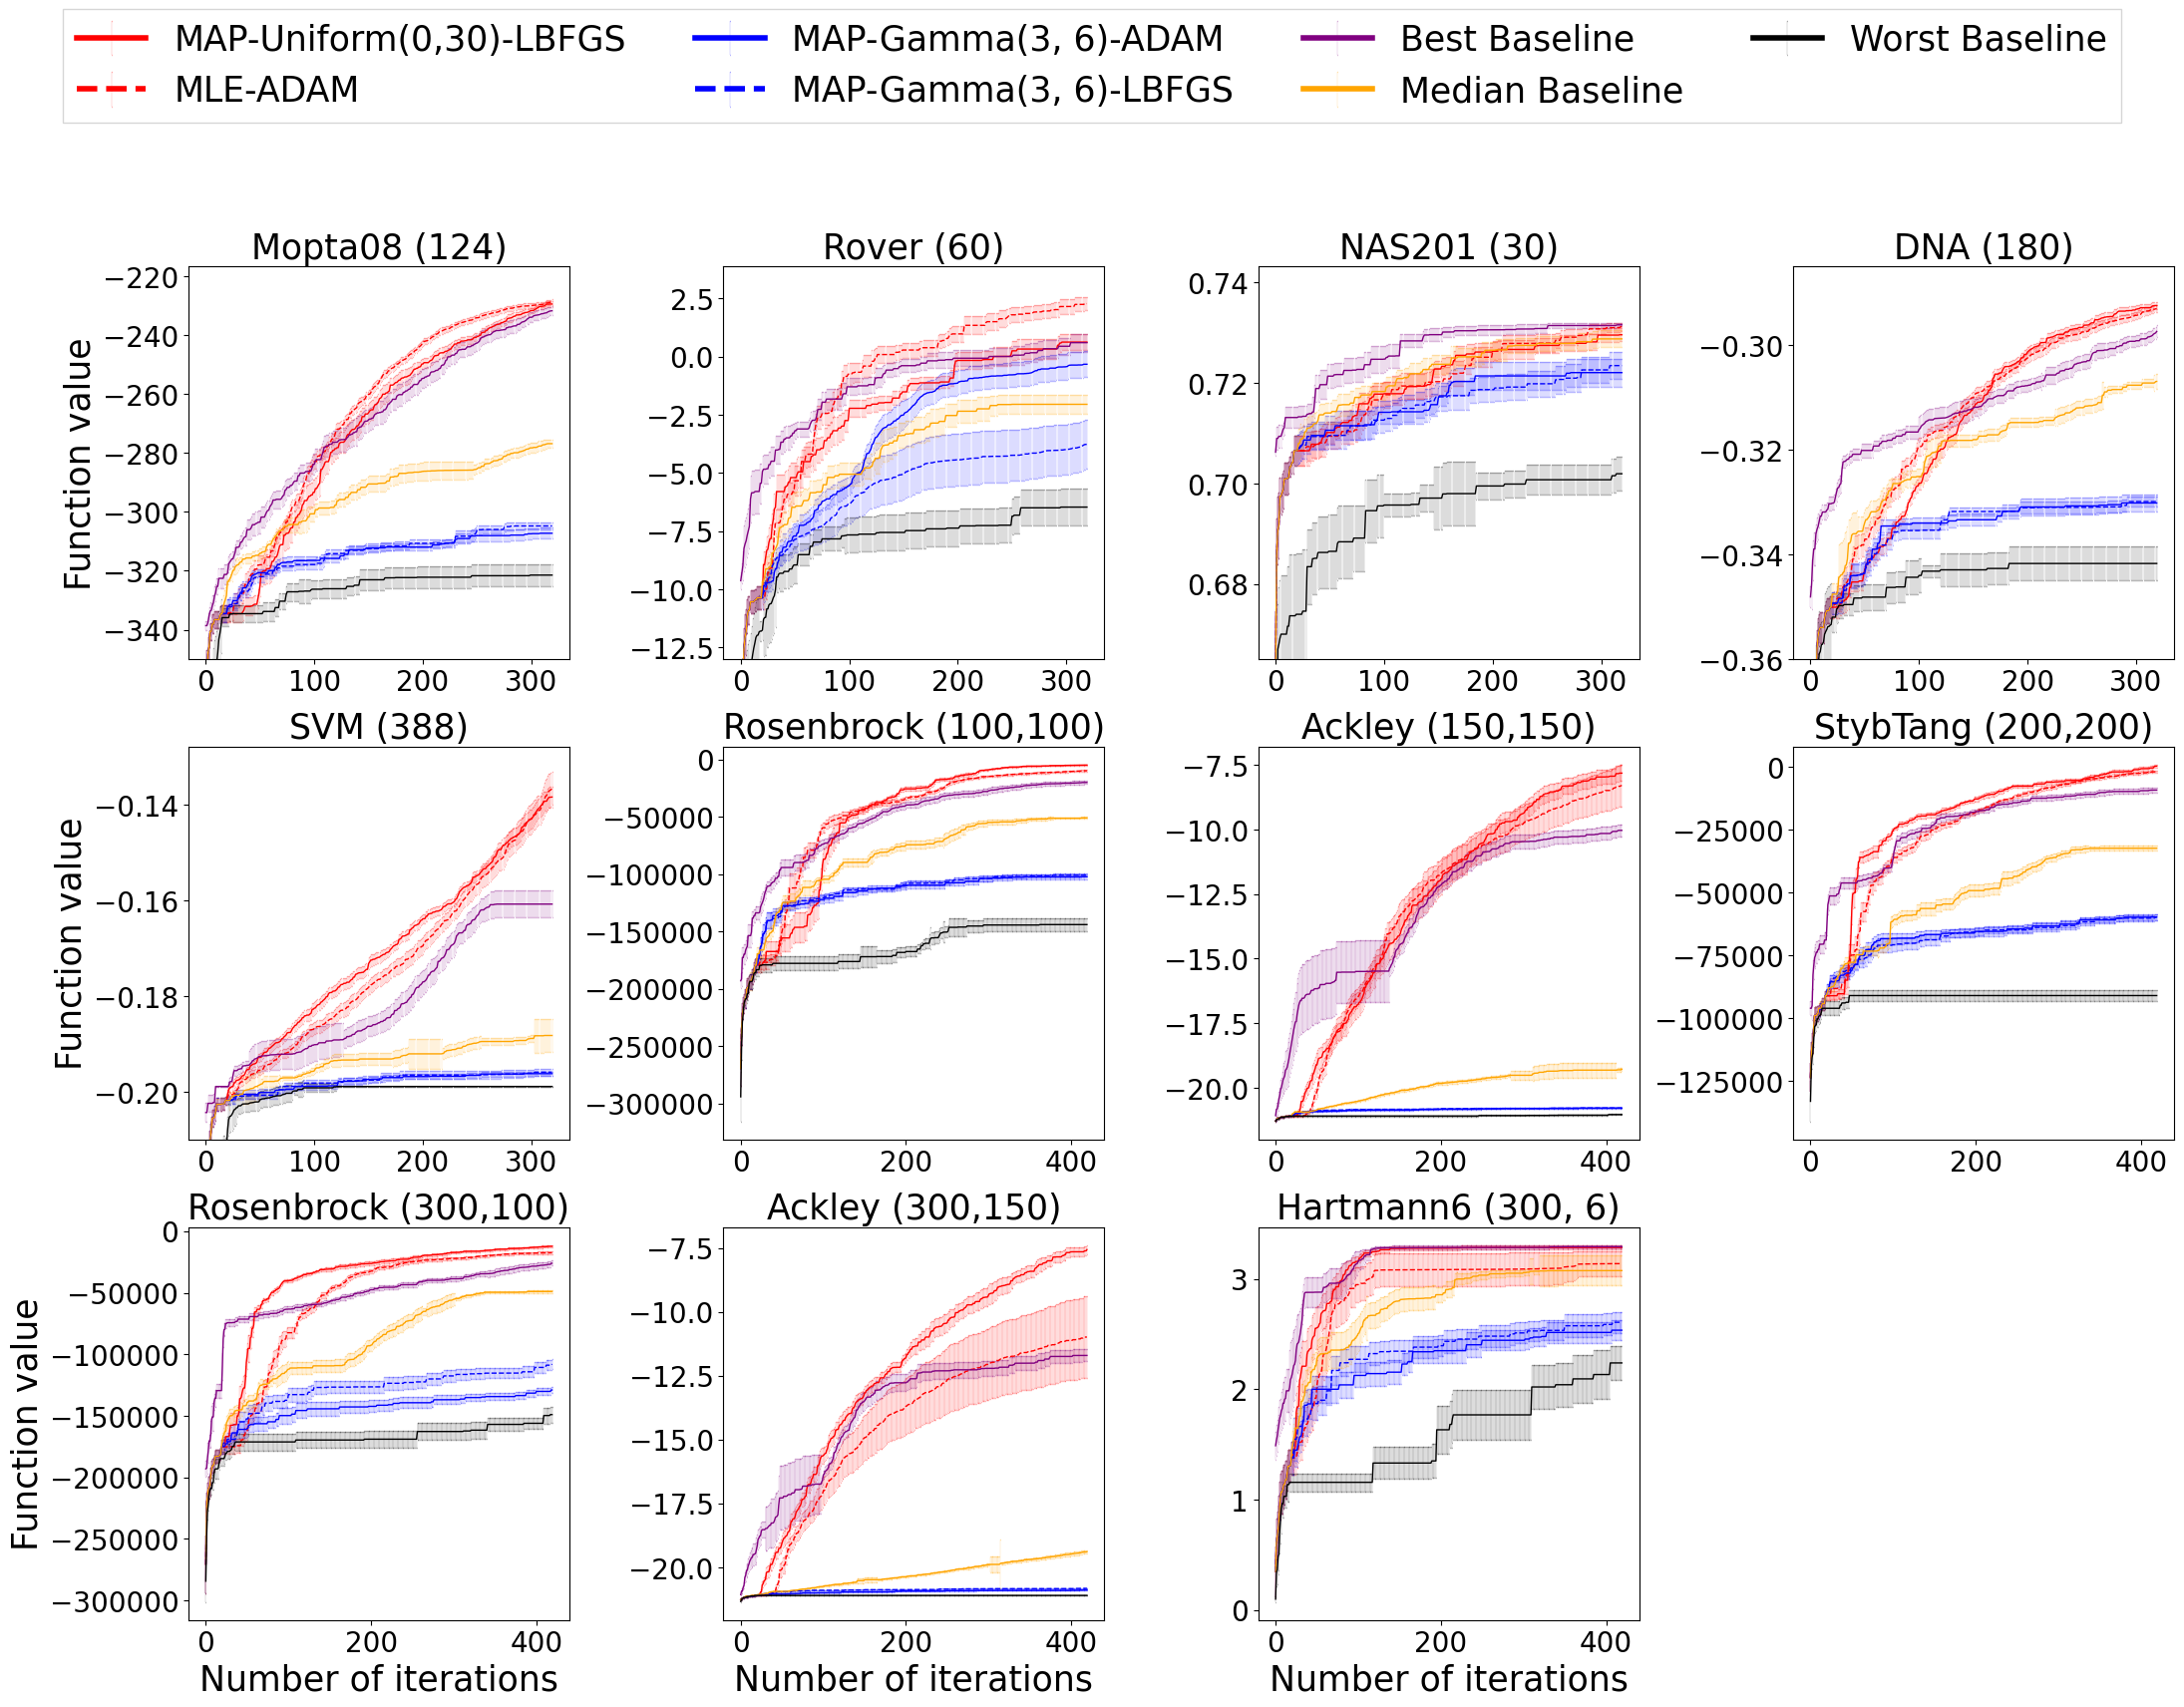}
    \caption{\small Runtime optimization performance using a diffuse prior, Uniform(0.001, 30), \textit{vs.} a concentrated Gamma prior, Gamma(3,6),  over the length scale parameters. SBO-1 and SBO-2 use Uniform(0.001, 30). \cmt{
    Maximum Function Value Obtained at the end of optimization loop. The results were collect from 10 runs.}}
    \label{fig:runtime-Gamma36}
\end{figure*}

\subsection{Alternative Acquisition Functions}
Next, we examined two other popular acquisition functions used in BO: Expected Improvement (EI) and Thompson sampling (TS). 
At each step, EI computes the expected improvement upon the best sample so far, 
\begin{align}
    \text{EI}(\x) = (\mu(\x) - f(\x^*) )\Psi\left(\frac{\mu(\x) - f(\x^*)}{\sqrt{v(\x)}}\right) + \sqrt{v(\x)}\Phi\left(\frac{\mu(\x)-f(\x^*)}{\sqrt{v(\x)}}\right),
\end{align}
where $\Psi(\cdot)$ and $\Phi(\cdot)$ are the CDF and PDF of the standard Gaussian distribution, $\x^*$ is the best sample that gives the largest function value among all the queries up to the current step, 
$\mu(\x)$ and $\sqrt{v(\x)}$ are the posterior mean and standard deviation of $f(\x)$ given current training data. We used BOTorch to maximize EI through L-BFGS. To conduct TS at each step, we used Sobol Sequence~\citep{sobol1967distribution} to sample 3K inputs in the domain, and jointly sampled the 3K function values from the GP posterior. We then selected the input with the largest function value as the next query. We denote this method by TS-3K. To explore more input candidates, we also employed the Lancos and conjugate gradient descent to approximate the posterior covariance matrix, and sampled 10K input candidates from Sobol Sequence. We denote this method as TS-10K. We used BOTorch implementation of both methods. We used ARD Mat\'ern kernel and MLE training at each step. 

The ultimate and runtime optimization performance for using EI, TS-3K and TS-10K, are shown in Fig. \ref{fig:final-acqf} and \ref{fig:running-acqf}, respectively. As we can see, in most cases, such as Mopta08 (128), SVM (388), DNA (180) and Rosenbrock (100, 100), both EI and TS perform worse than UCB, and also worse than the best baseline. On Ackley(150, 150) and Ackley(300, 150), the performance of EI and TS are even among the worst.
%\xuc{For all benchmarks besides Hartmann6, EI performed better than TS-3k and TS-10k. Interestingly, Thompson sampling performed rather well on Hartmann 6, which is better than UCB and EI with MLE training, but still inferior than UCB with MAP estimation and LBFGS as optimization.}

The limitation of EI might arise from the gradient vanishing during the optimization, as pointed by the recent work~\citep{ament2024unexpected}. A remedy is to use log-EI as the acquisition function. The failure of the TS might be due to the high-dimension of the input space. A few thousand  candidates might not be sufficient to cover the whole space; as a result, the selected queries are inferior in indicating  the best direction to optimize the target function. %\xuc{Also, unlike EI and UCB, the scale of exploration for Thompson sampling depends purely on the quantity of random point generator.}

\begin{figure*}[!ht]
    \centering
    \includegraphics[width=\textwidth]{BO ICLR 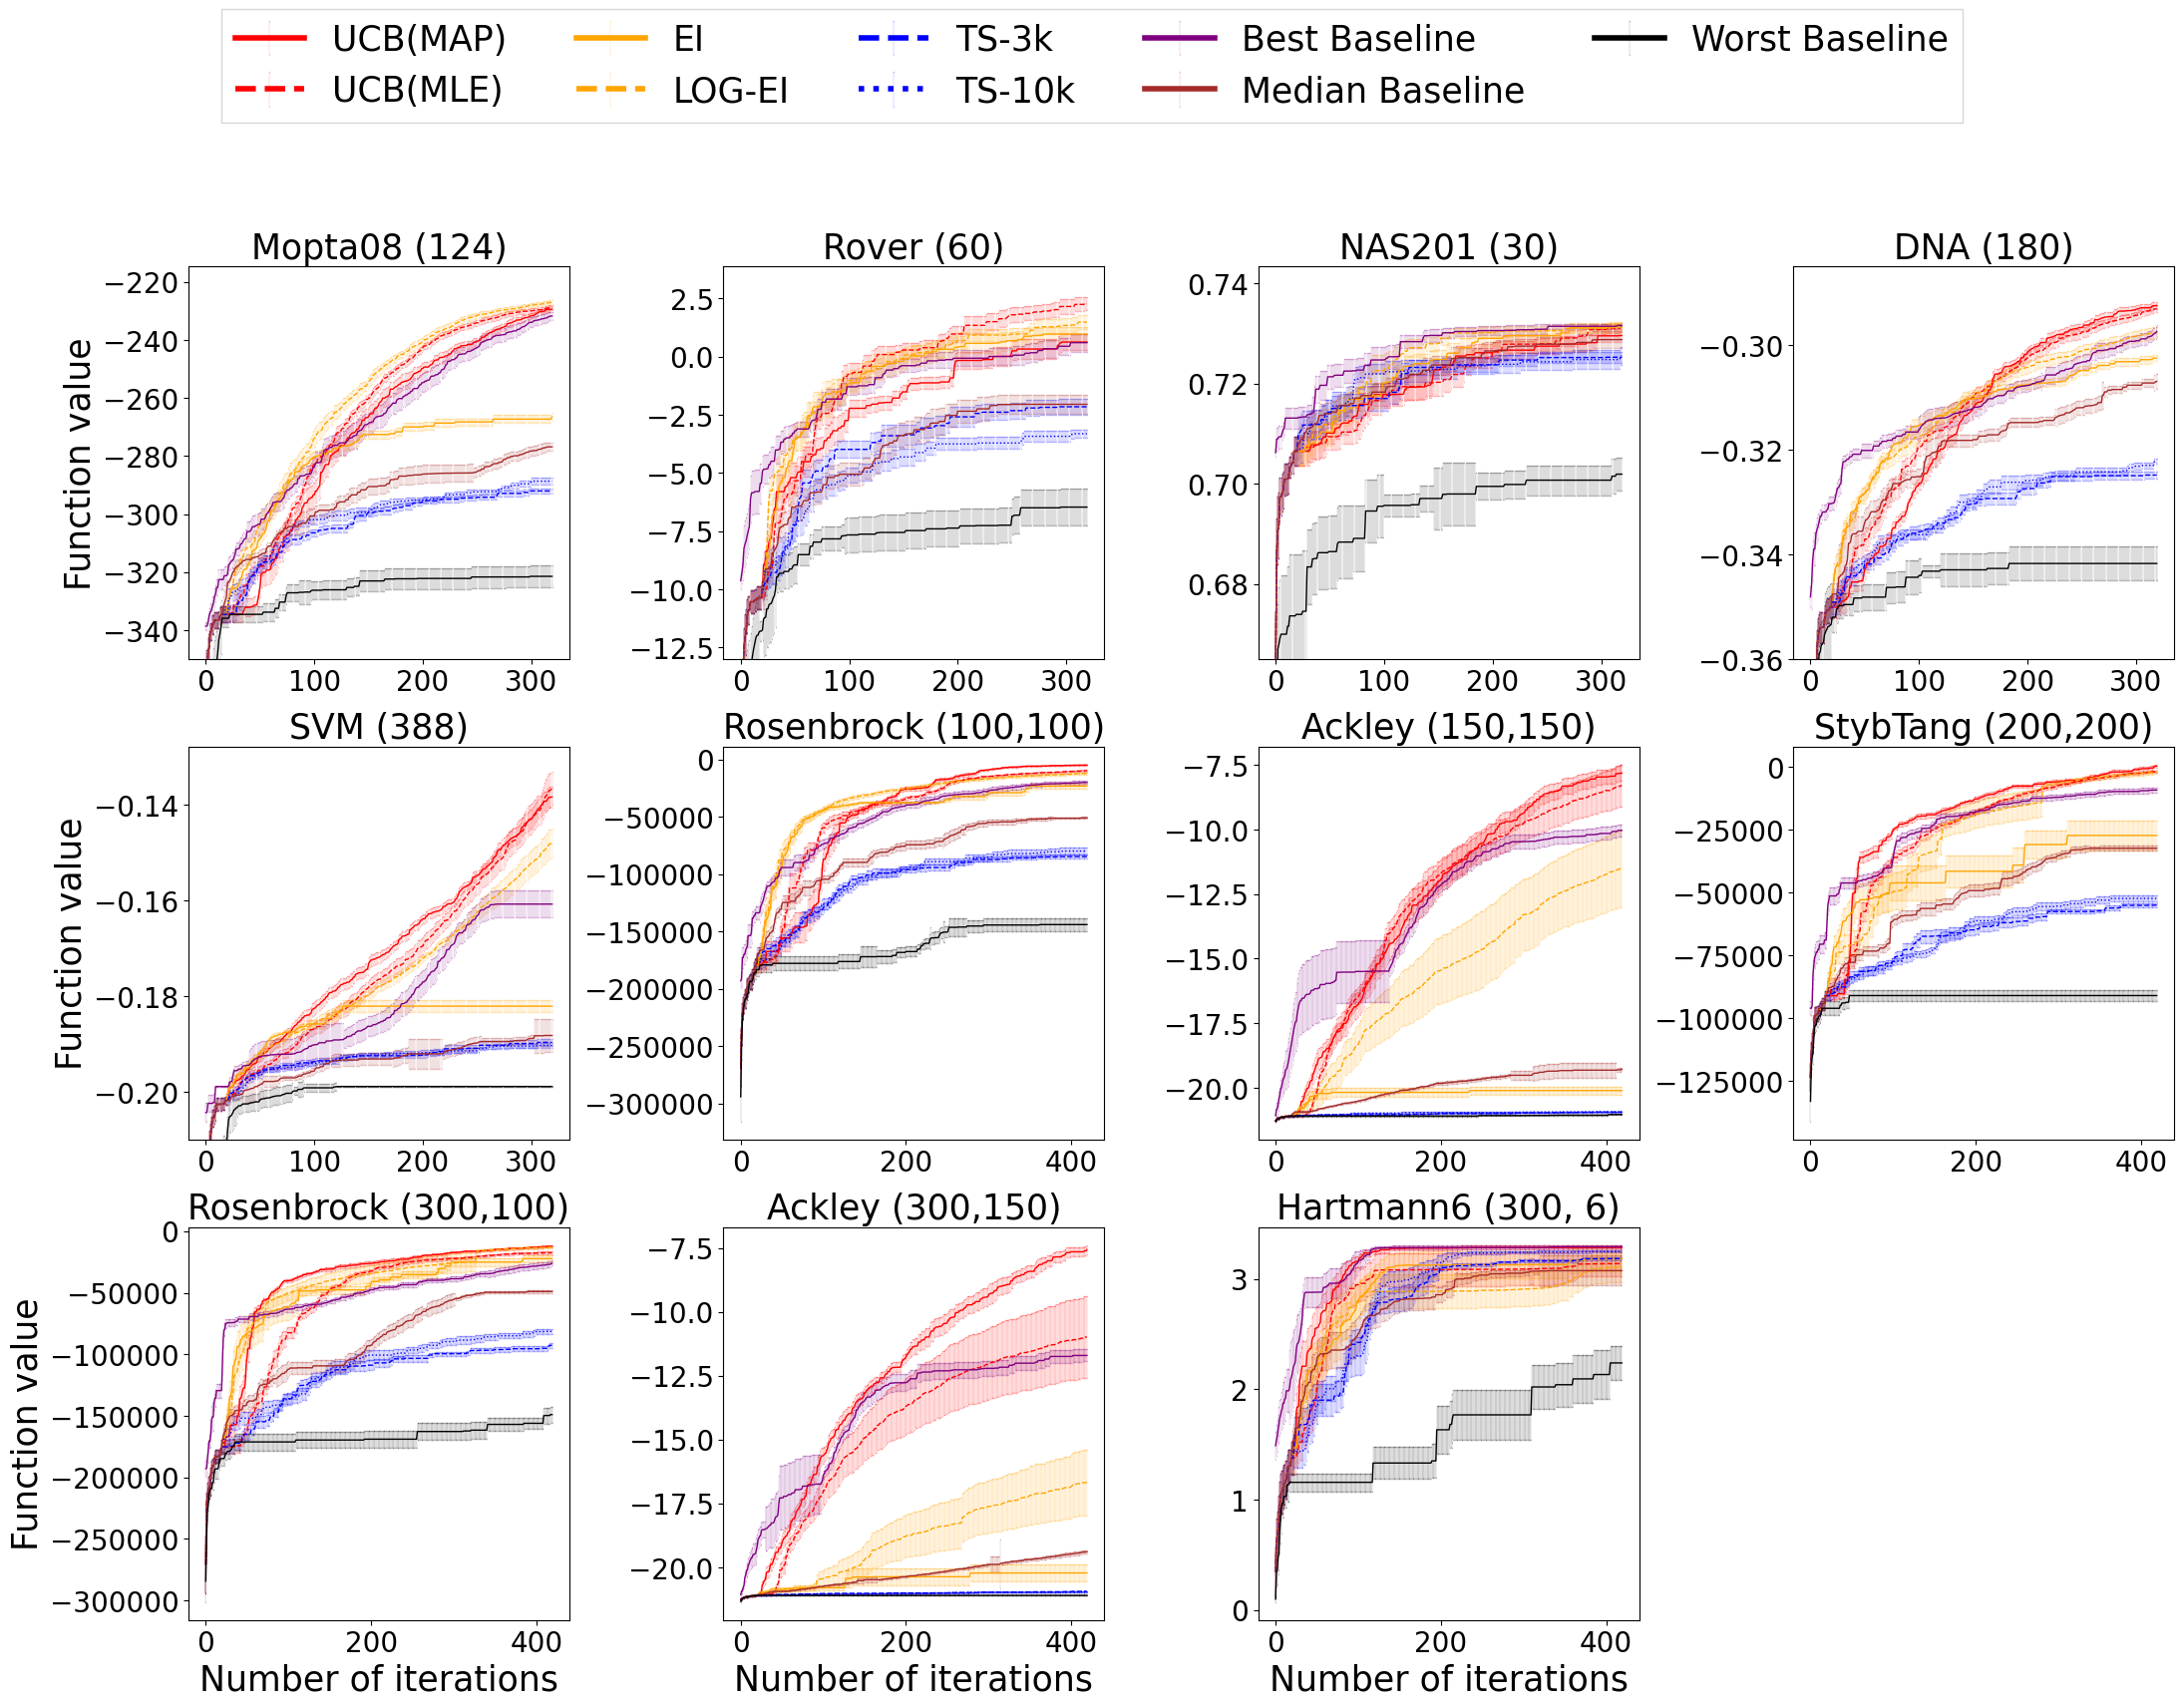}
    \caption{\small Runtime performance with different acquisition functions. Note that SBO-1 and SBO-2 use UCB. \cmt{Maximum Function Value Obtained at the end of optimization loop. The results were collect from 10 runs.}}
    \label{fig:running-acqf}
\end{figure*}

\subsection{Different Choice of $\lambda$ in UCB}\label{sect:lam-choice}
%\xuc{I moved previous ablation section(sec B) to here.}

Finally, we examined how the exploration parameter $\lambda$ in UCB (see \eqref{eq:ucb}) influences the performance in high-dimensional optimization. To this end, we used ARD Ma\'ern kernel and varied $\lambda$ from \{0.5, 1.0, 1.5, 2.0\}. We conducted MLE training via ADAM optimization. %We conducted MLE for GP training at each step. 
We show the ultimate and runtime optimization performance in Fig. \ref{fig:final-lambda} and \ref{fig:running-lambda}, respectively. 
It can be seen that, in most benchmarks (Mopta08, Rover, NAS201, DNA, \etc), the performance with different $\lambda$'s is close. However, on DNA, SVM and Ackley, the performance of $\lambda=0.5$ is typically worse than the bigger choice of $\lambda$. This might be due to that those problems are more challenging (\eg Ackley has many local minima), a larger exploration level ($\lambda$) is needed to identify better optimization outcomes. 

%\xuc{As we can see, for majority benchmark functions(Mopta08, Rover, DNA, SVM, Rosenbrock(100, 100), StybTang), GP-ARD with MLE training achieved better BO performance than the best SOTA HDBO method. And there is a clear gap between $\lambda$=0.5 and other choice of $\lambda$ on DNA, SVM, Ackley, Rosenbrock(300, 100), where the performance of $\lambda$=0.5 being significantly inferior. For functions(Ackley) that are known with local optimal, we can see that a larger $\lambda$ will yield better BO performance.}

\begin{figure*}[!ht]
    \centering
    \includegraphics[width=\textwidth]{BO ICLR 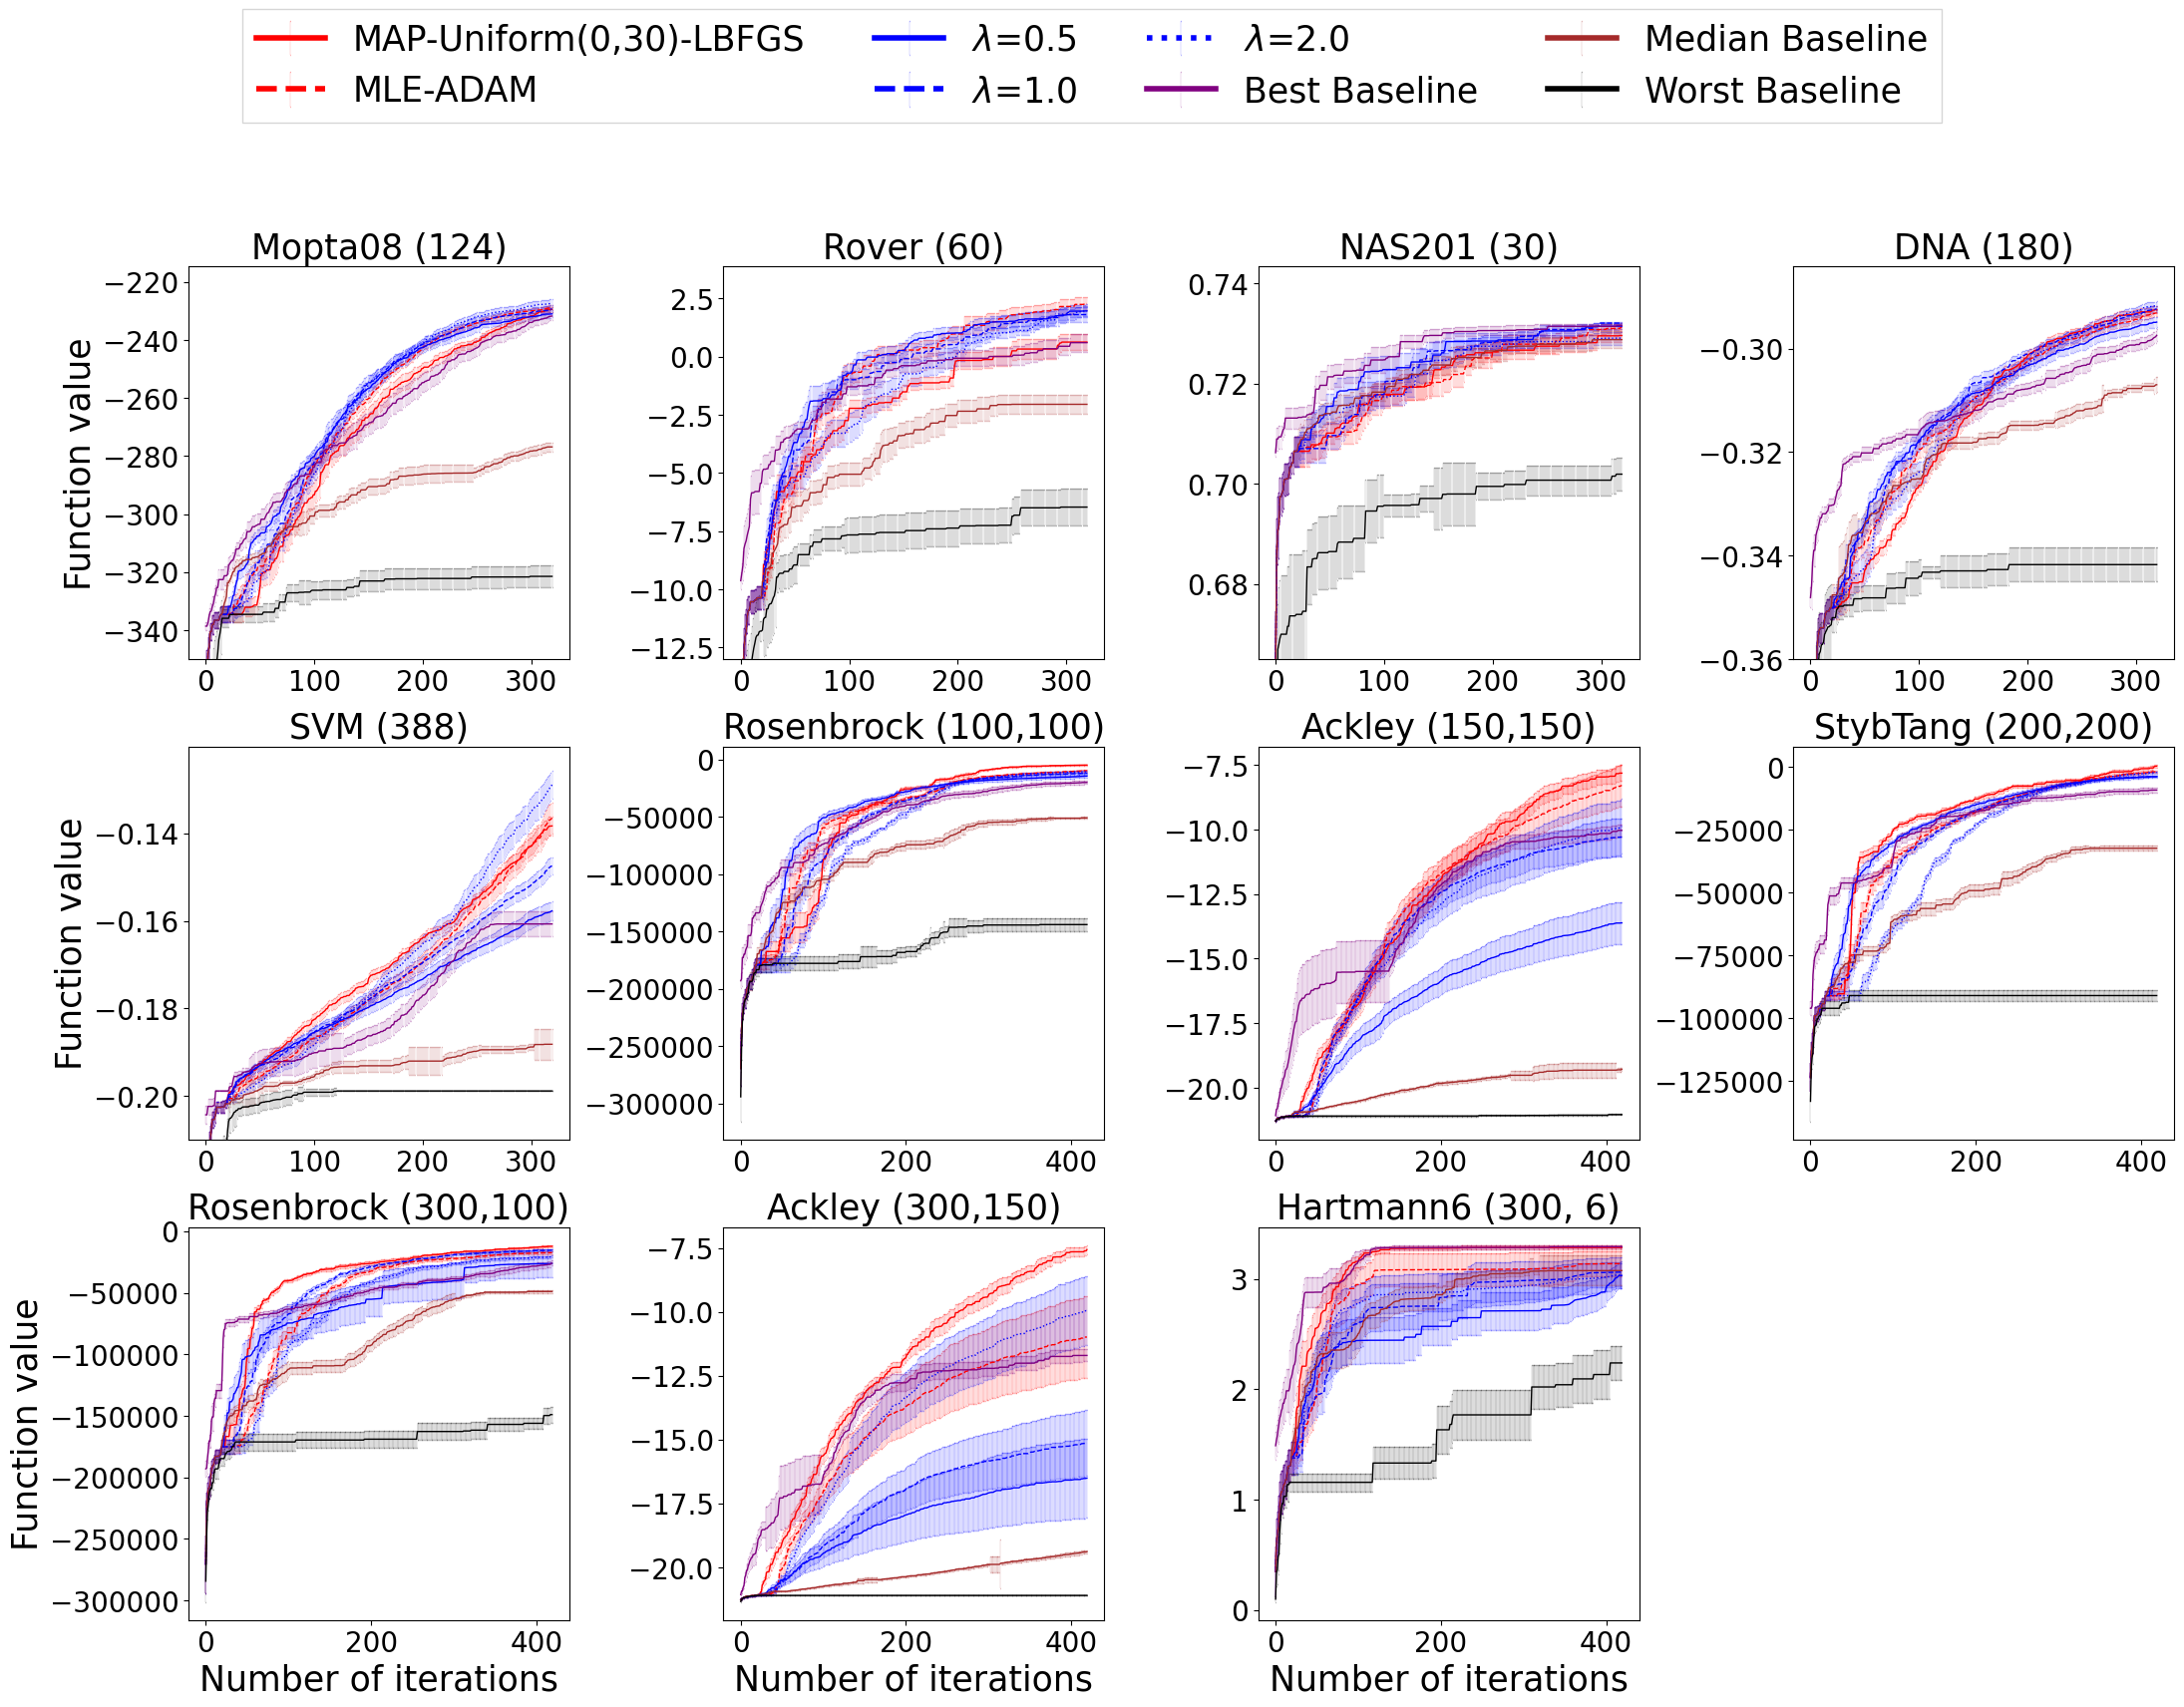}
    \caption{\small Runtime optimization performance with different exploration level  $\lambda$ in UCB. Note that SBO-1 and SBO-2 use $\lambda=1.5$. \cmt{Maximum Function Value Obtained at the end of optimization loop. The results were collect from 10 runs. $\lambda$ varied from \{0.5, 1.0, 1.5, 2.0\}.}}
    \label{fig:running-lambda}
\end{figure*}

\section{Limitation and Discussion}
\label{sec:limitation}
We evaluated Standard Bayesian Optimization on 5 real-world benchmarks and 6 synthetic functions that are most commonly used in previous HDBO works. We acknowledge that there are infinitely more  high-dimensional optimization problems that can be used for evaluation. In general, we hope after our work, future HDBO paper can include Standard BO with proper settings as their baseline methods. Hence, we can attain a better understanding about the potential of Standard BO in high dimensional functions. Moreover, we will seek for theoretical justifications and guarantees on SBO in high-dimensional settings.  We would like to also seek for a theoretical explanation of the failure modes.
