# Supplementary material for: Standard Gaussian Process is All You Need for High-Dimensional Bayesian Optimization
Source: arXiv:2402.02746 source file (2025-03-11)
Supplement: Supplementary file 3 [file appendix-old.tex]

\section{More Experiment Details}
\subsection{Definition of Synthetic Functions}\label{sect:syn-def}
%We denote the function forms and bounds we used in Sec \ref{sec:experiments} below.

\textbf{Stybtang}. We used the following slightly-modified Stybtang function, %The original Stybtang is in form $f(x)=\frac{1}{2}\sum_{i=1}^{D}(x_{i}^{4}-16x_{i}^{2}+5x_{i})$. Our version $f_{\text{V1}}$ is of form,
\[
f(\x)=\frac{1}{2}\sum_{i=1}^{D}\left((x_{i}-c_{i})^{4}-16(x_{i}-c_{i})^{2}+5(x_{i}-c_{i})\right),
\]
where $\x \in [-5, 5]^D$, and we set $[c_1, \dots, c_D]$ as an evenly spaced sequence in $[0, 7.5]$ ($c_1 = 0$ and $c_D = 7.5$). The optimum  is at $\x^\dagger=[c_1 -2.903534, \ldots, c_D - 2.903534]$.


\textbf{Rosenbrock}. 
We used the following Rosenbrock function, 
\[
f(\x)=\sum_{i=1}^{D-1}\left[100\left((x_{i+1}-c_{i+1})-(x_{i}-c_{i})^{2}\right)^{2}+\left(1 - (x_{i}-c_{i})\right)^2\right],
\]
where $\x \in [-2.048, 2.048]^{D}$. We set $[c_{1}, ..., c_D]$ as an evenly spaced sequence in $[-2, 2]$, where $c_{1}=-2$ and  $c_{D}=2$. The optimum is at $x^\dagger =  [c_{1}+1, ..., c_{D}+1]$. 

\textbf{Ackley}. We used the Ackley function defined in~\citep{simulationlib},
\[
f(\x)=-20\text{ exp}\left(-0.2\sqrt{\frac{1}{d}\sum_{i=1}^{d}x_{i}^{2}}\right)-\text{exp}\left(\frac{1}{d}\sum_{i=1}^{d}\text{cos}(2{\pi}x_{i})\right)+20+\text{exp}(1),
\]
where each $x_i \in [-32.768, 32.768]$ and the (global) optimum is at $x^{\dagger}=[0, \ldots, 0]$. 

\textbf{Hartmann6}. The function is given by
\[
f(\x)=-\sum_{i=1}^{4}{\alpha}_{i}{ \exp}\left(-\sum_{j=1}^{6}A_{ij}(x_{j}-P_{ij})^{2}\right),
\]
where each $x_i \in [0, 1]$, $\A=[A_{ij}]$ and $\P = [P_{ij}]$ are two pre-defined matrices as in \citep{simulationlib}.
The global optimum is at $\x^\dagger = [0.20169, 0.150011, 0.476874, 0.275332, 0.6573]$.


\begin{figure*}[!ht]
    \centering
    \includegraphics[width=\textwidth]{BO ICLR 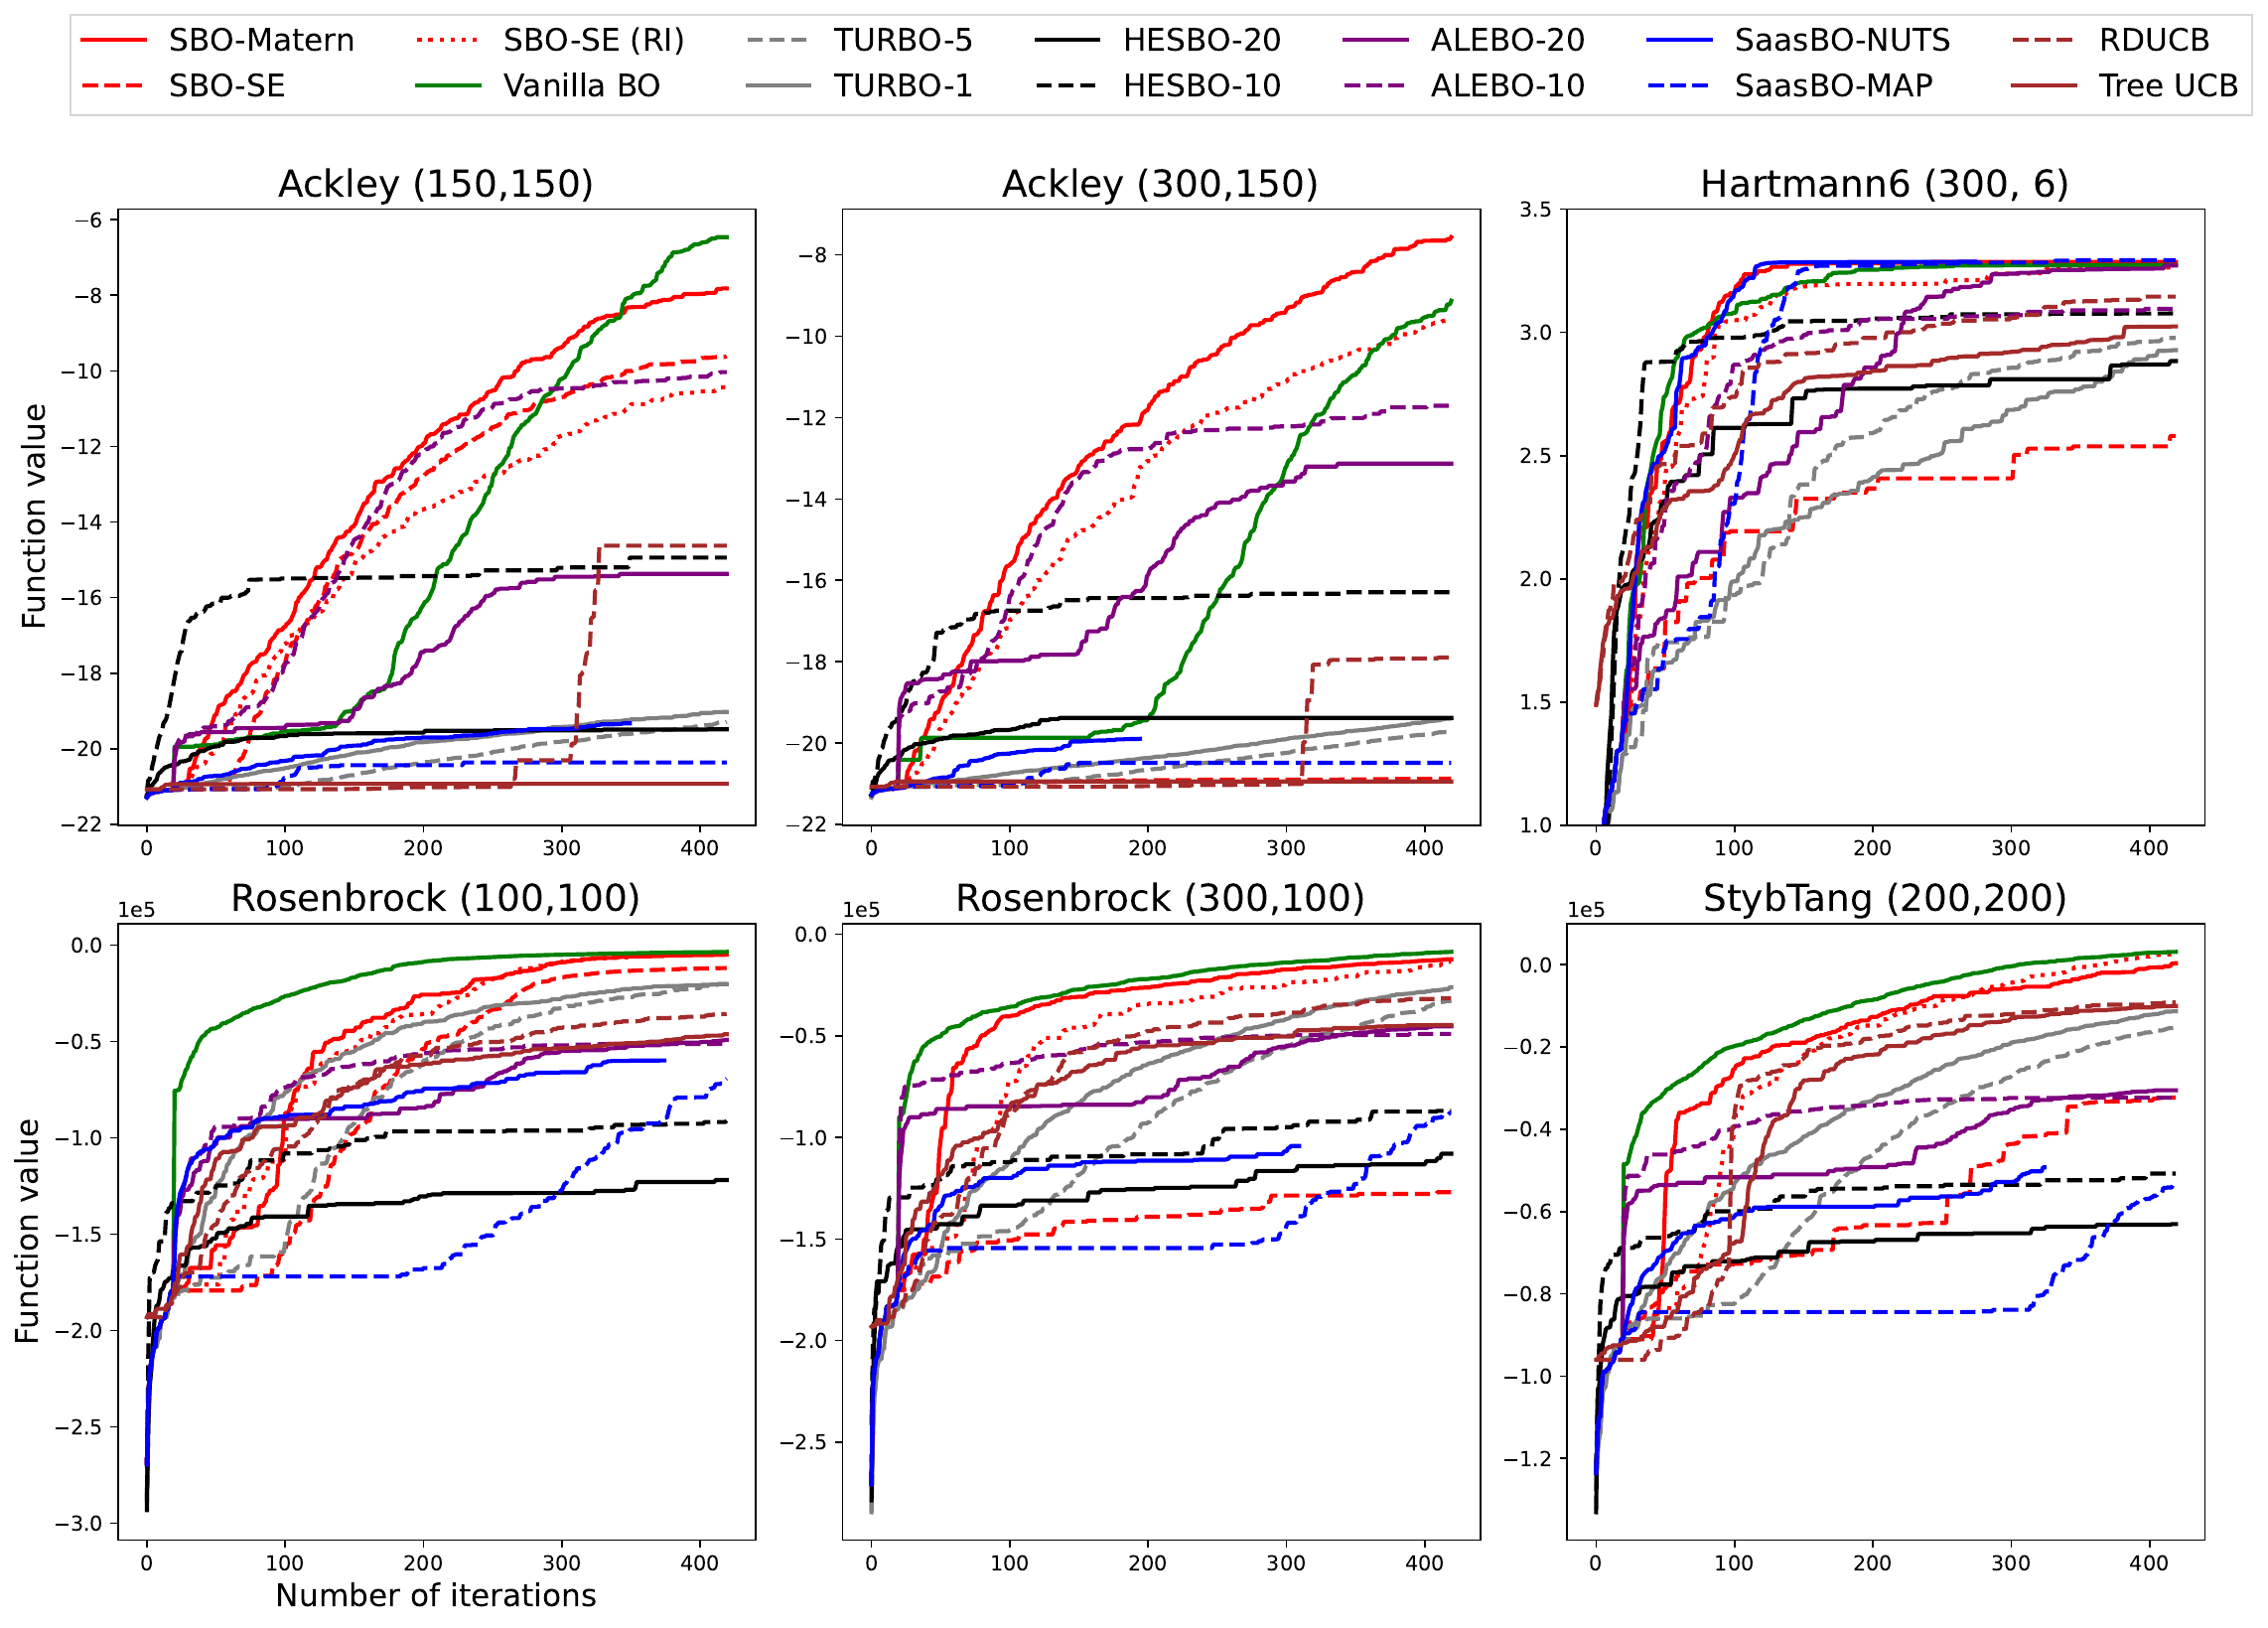}
    \caption{\small Runtime performance: Maximum Function Value Obtained \textit{vs.} Number of Steps in synthetic benchmarks. The results were averaged from 10 runs. }
    \label{fig:syn-running-plot}
\end{figure*}

\begin{figure*}[!ht]
    \centering
    \includegraphics[width=\textwidth]{BO ICLR 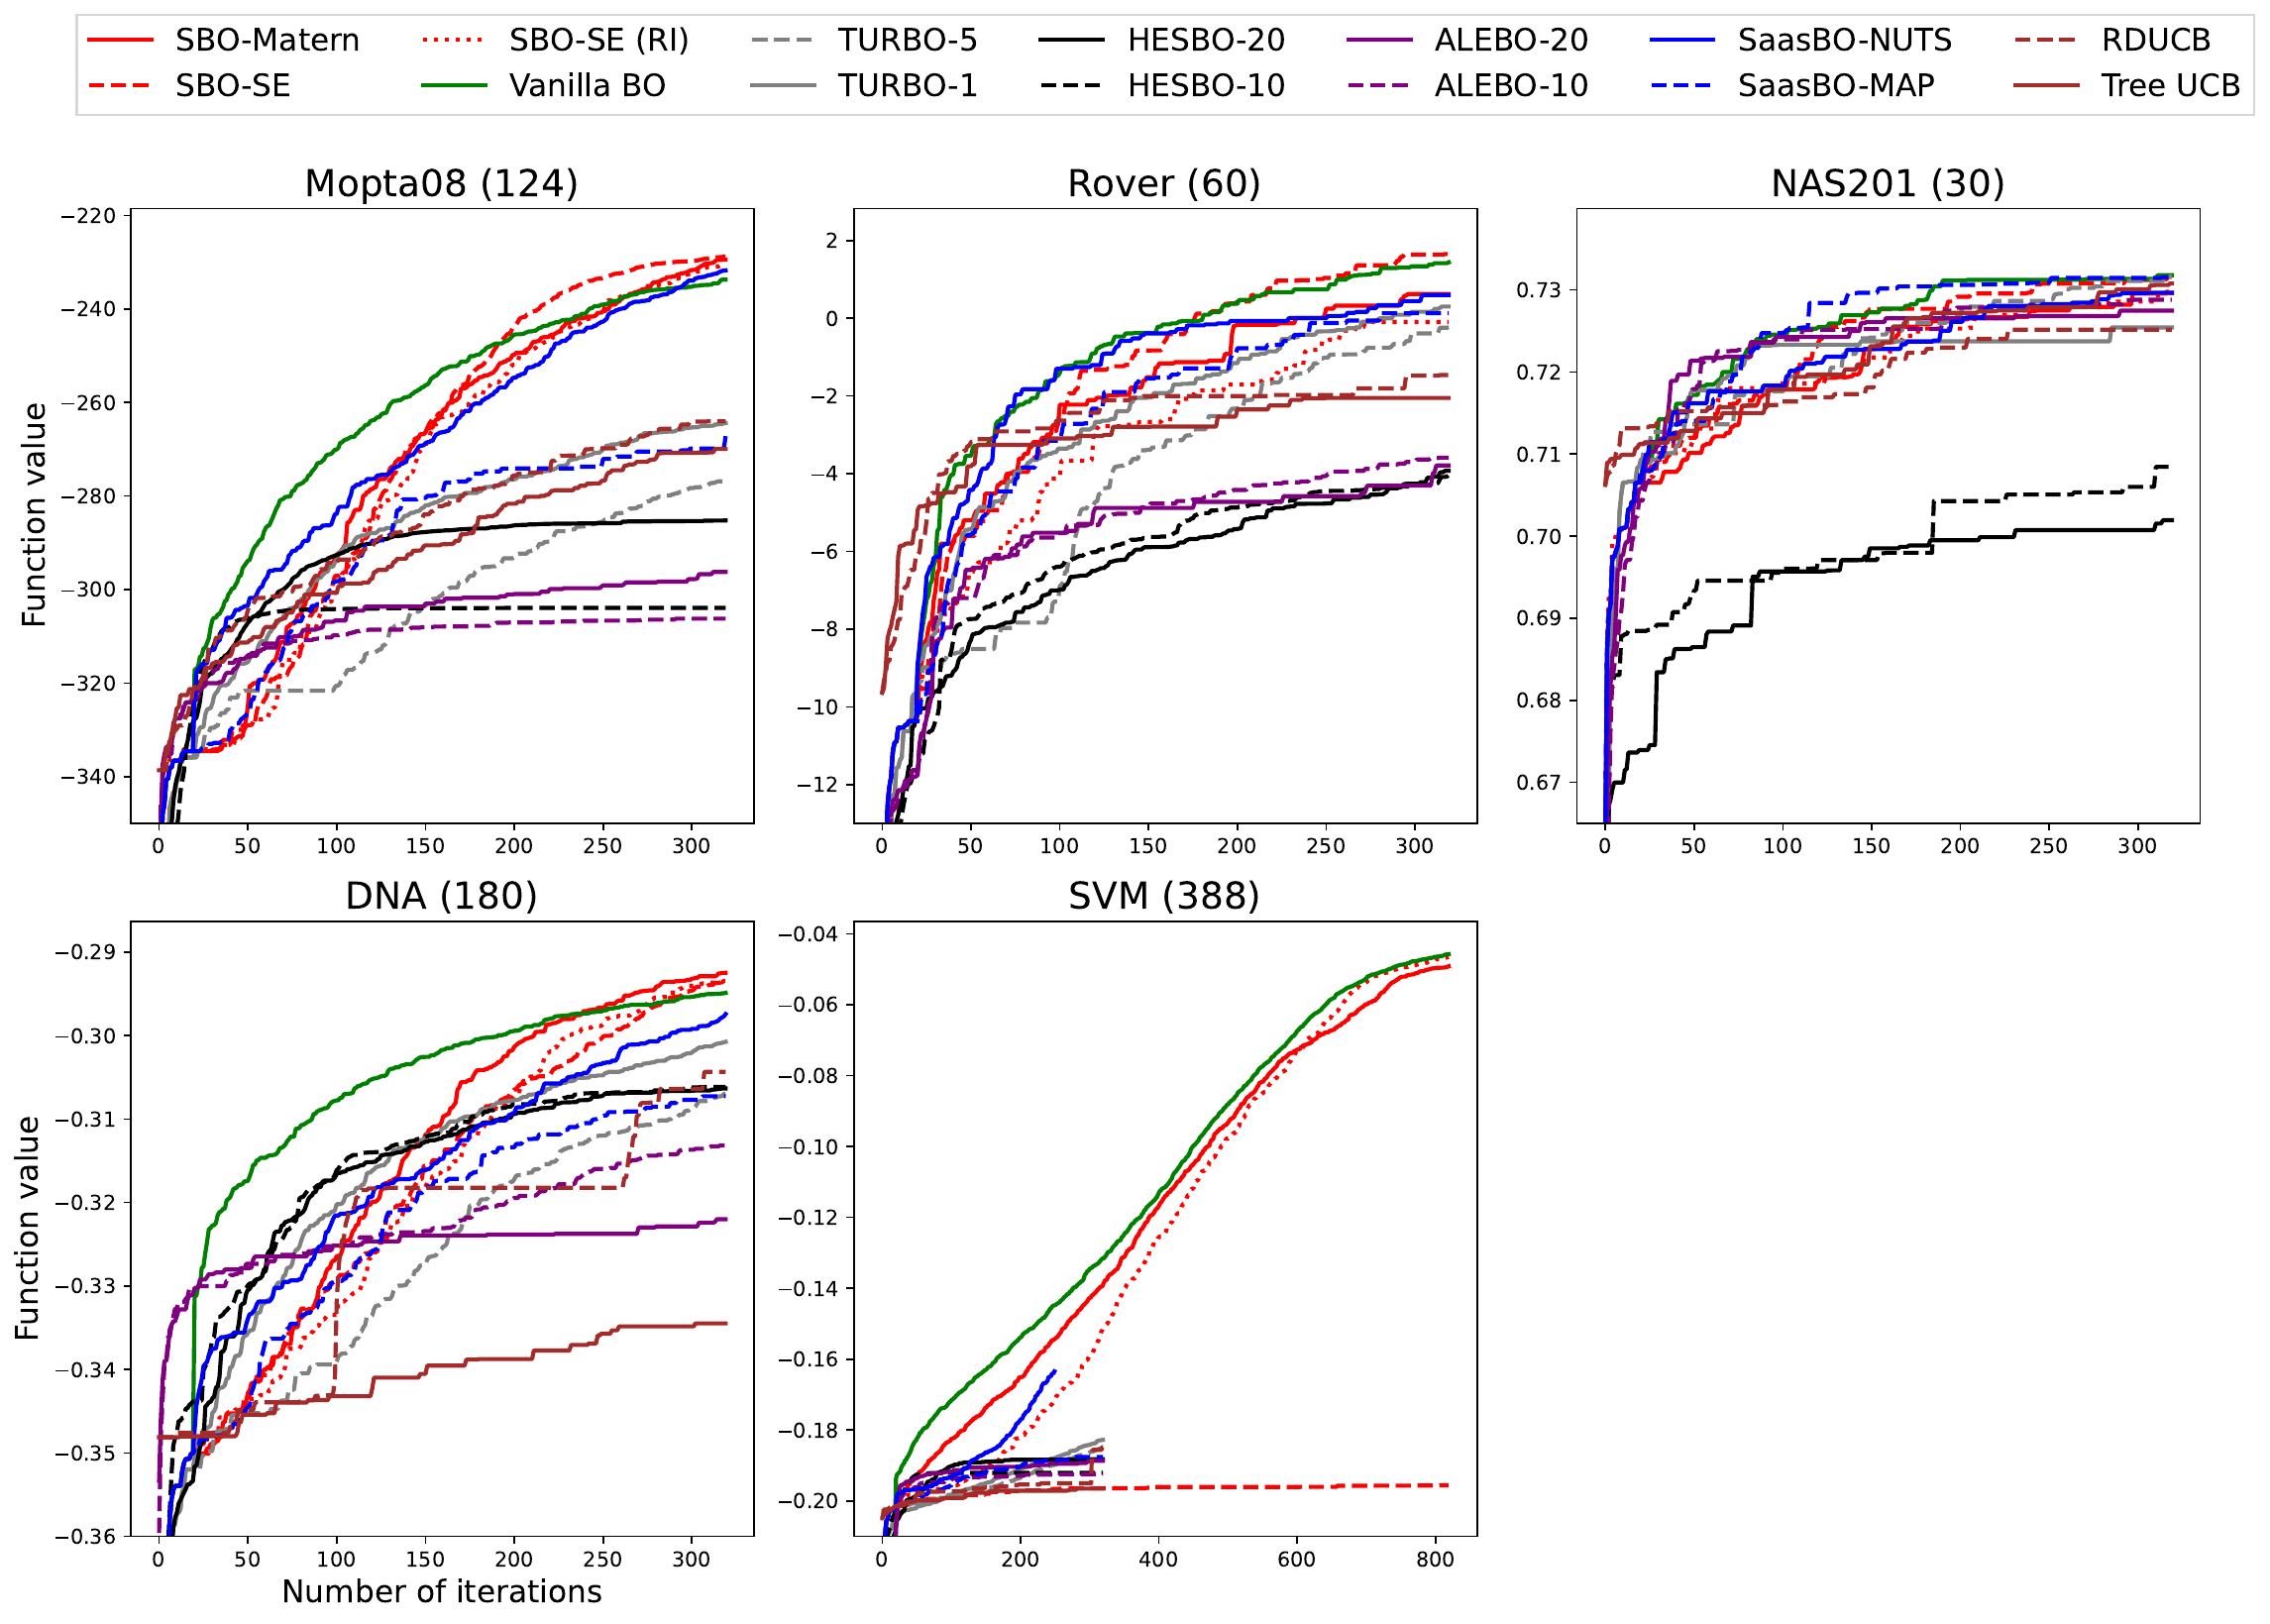}
    \caption{\small Runtime performance: Maximum Function Value Obtained \textit{vs.} Number of Steps in real-world benchmarks. The results were averaged from 10 runs.}
    \label{fig:running-real}
\end{figure*}

\begin{figure*}[!ht]
    \centering
    \includegraphics[width=\textwidth]{BO ICLR 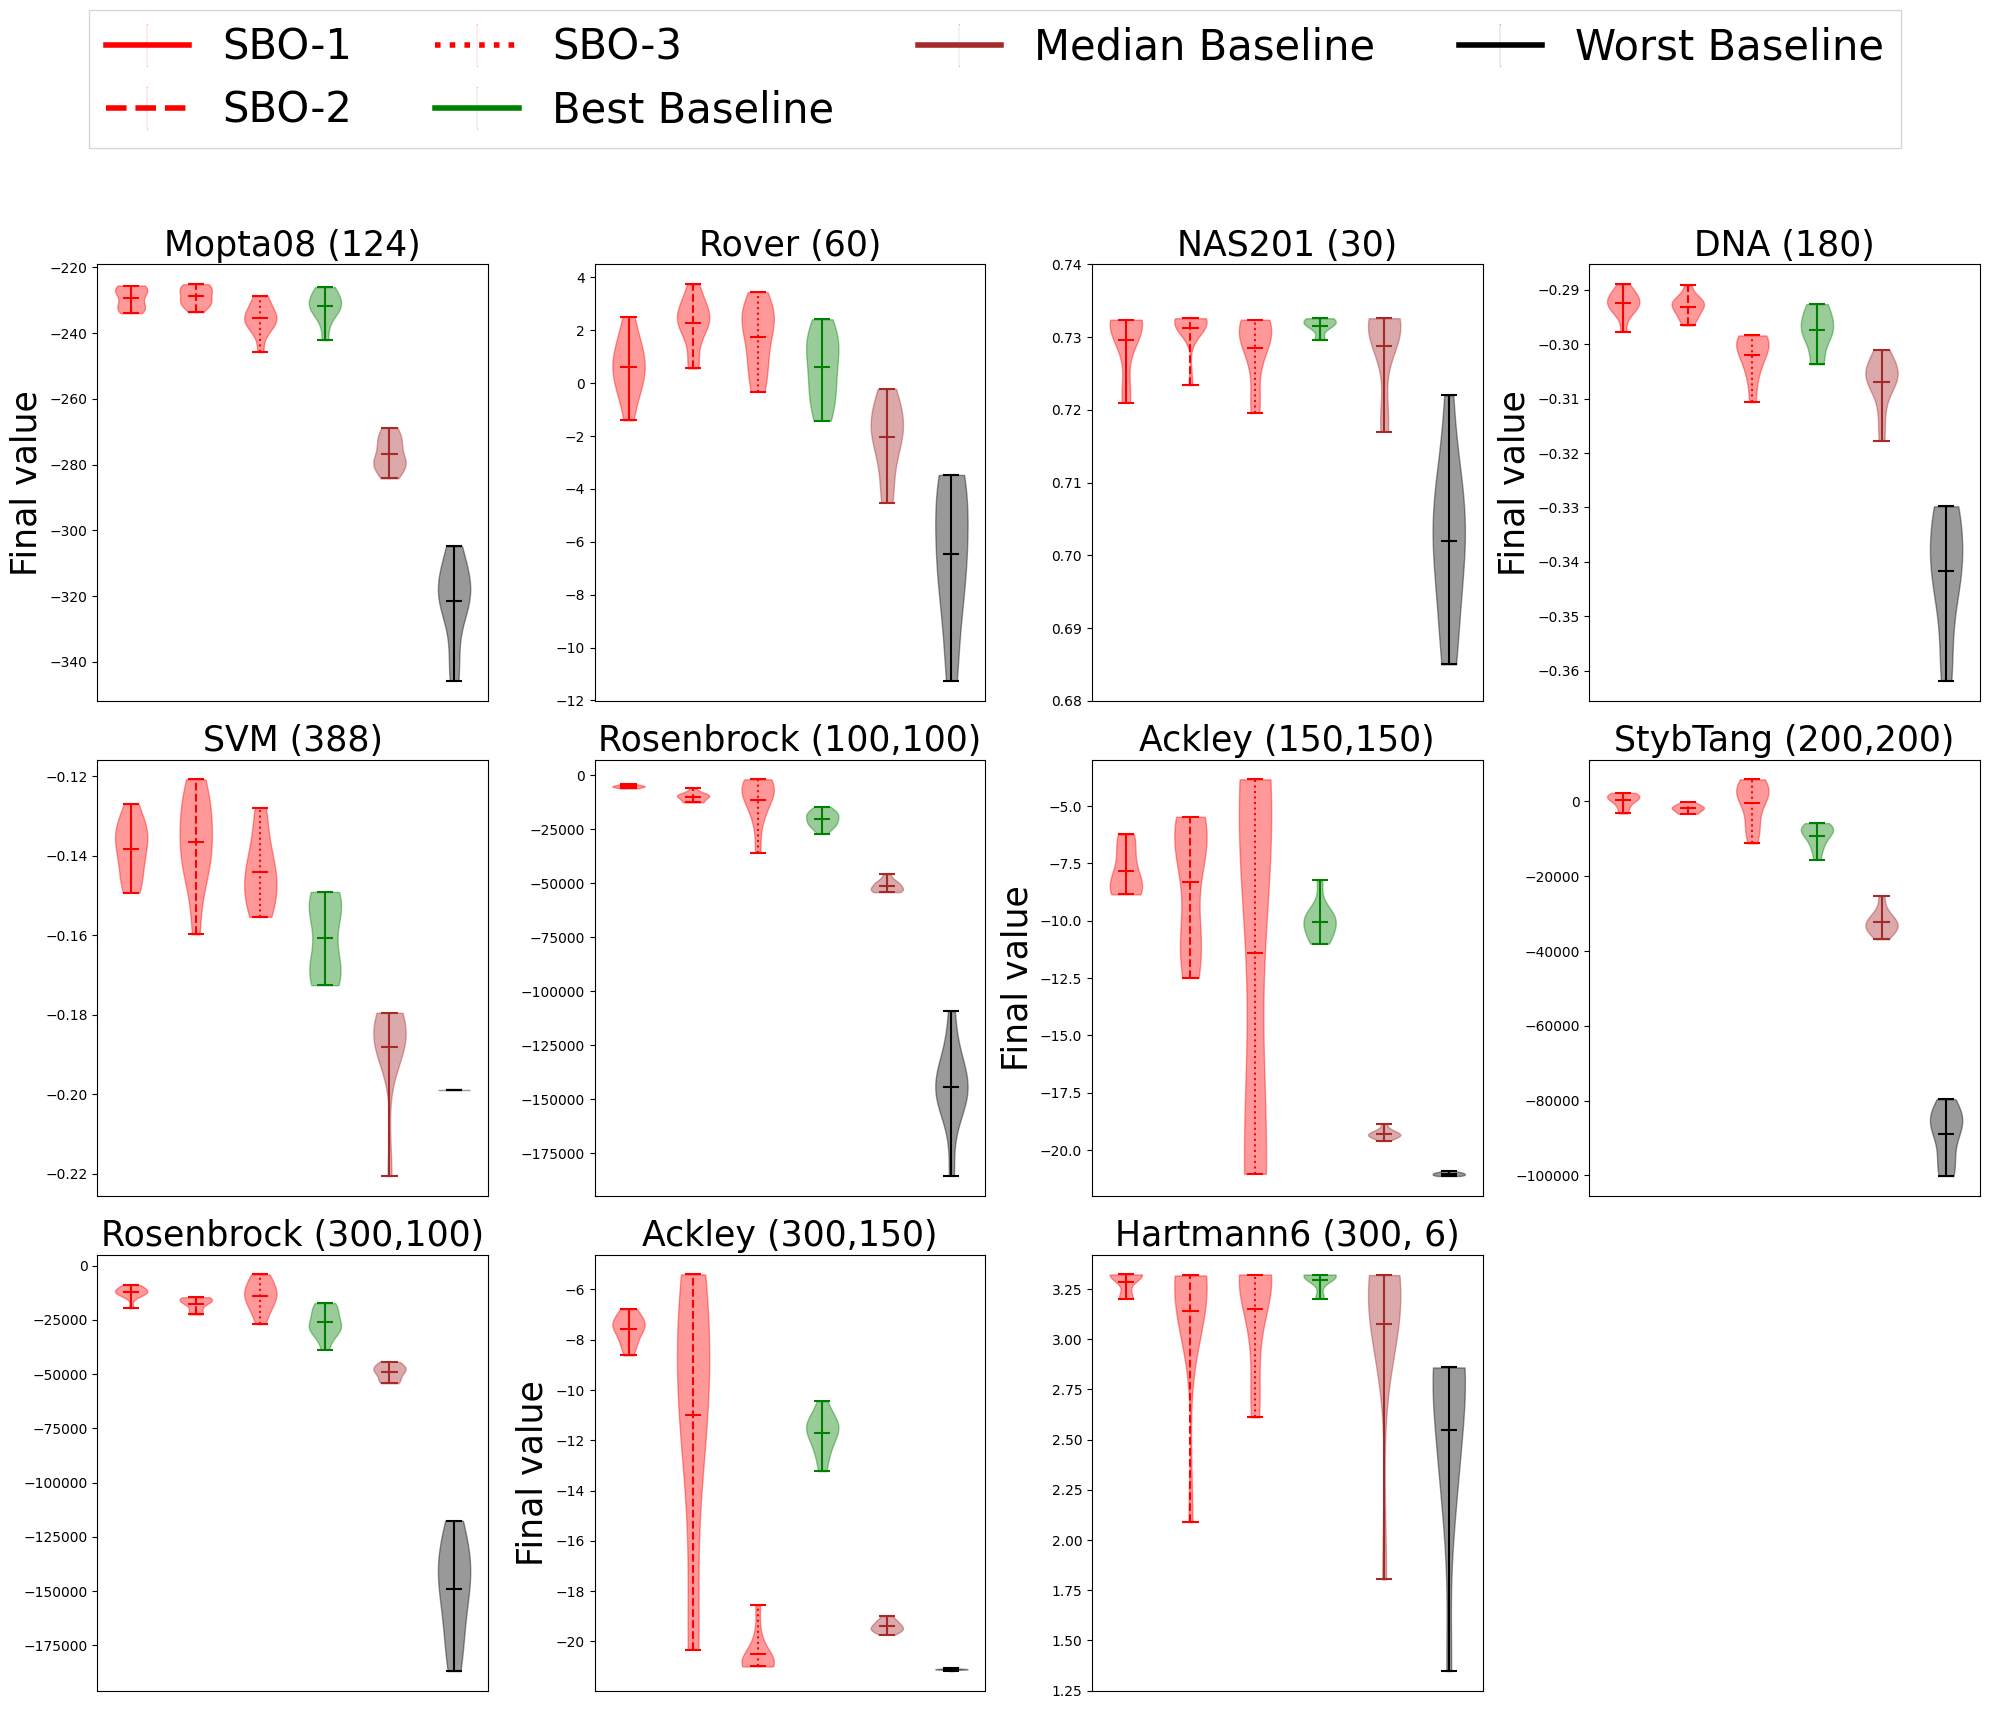}
    \caption{\small Ultimate optimization performance: Maximum Function Value obtained at the end of optimization loop, including SBO-3, namely training with a single length-scale parameter in Mat\'ern-5/2 kernel. The results were collect from 10 runs.}
    \label{fig:final-all-sbo3}
\end{figure*}
\begin{figure*}[!ht]
    \centering
    \includegraphics[width=\textwidth]{BO ICLR 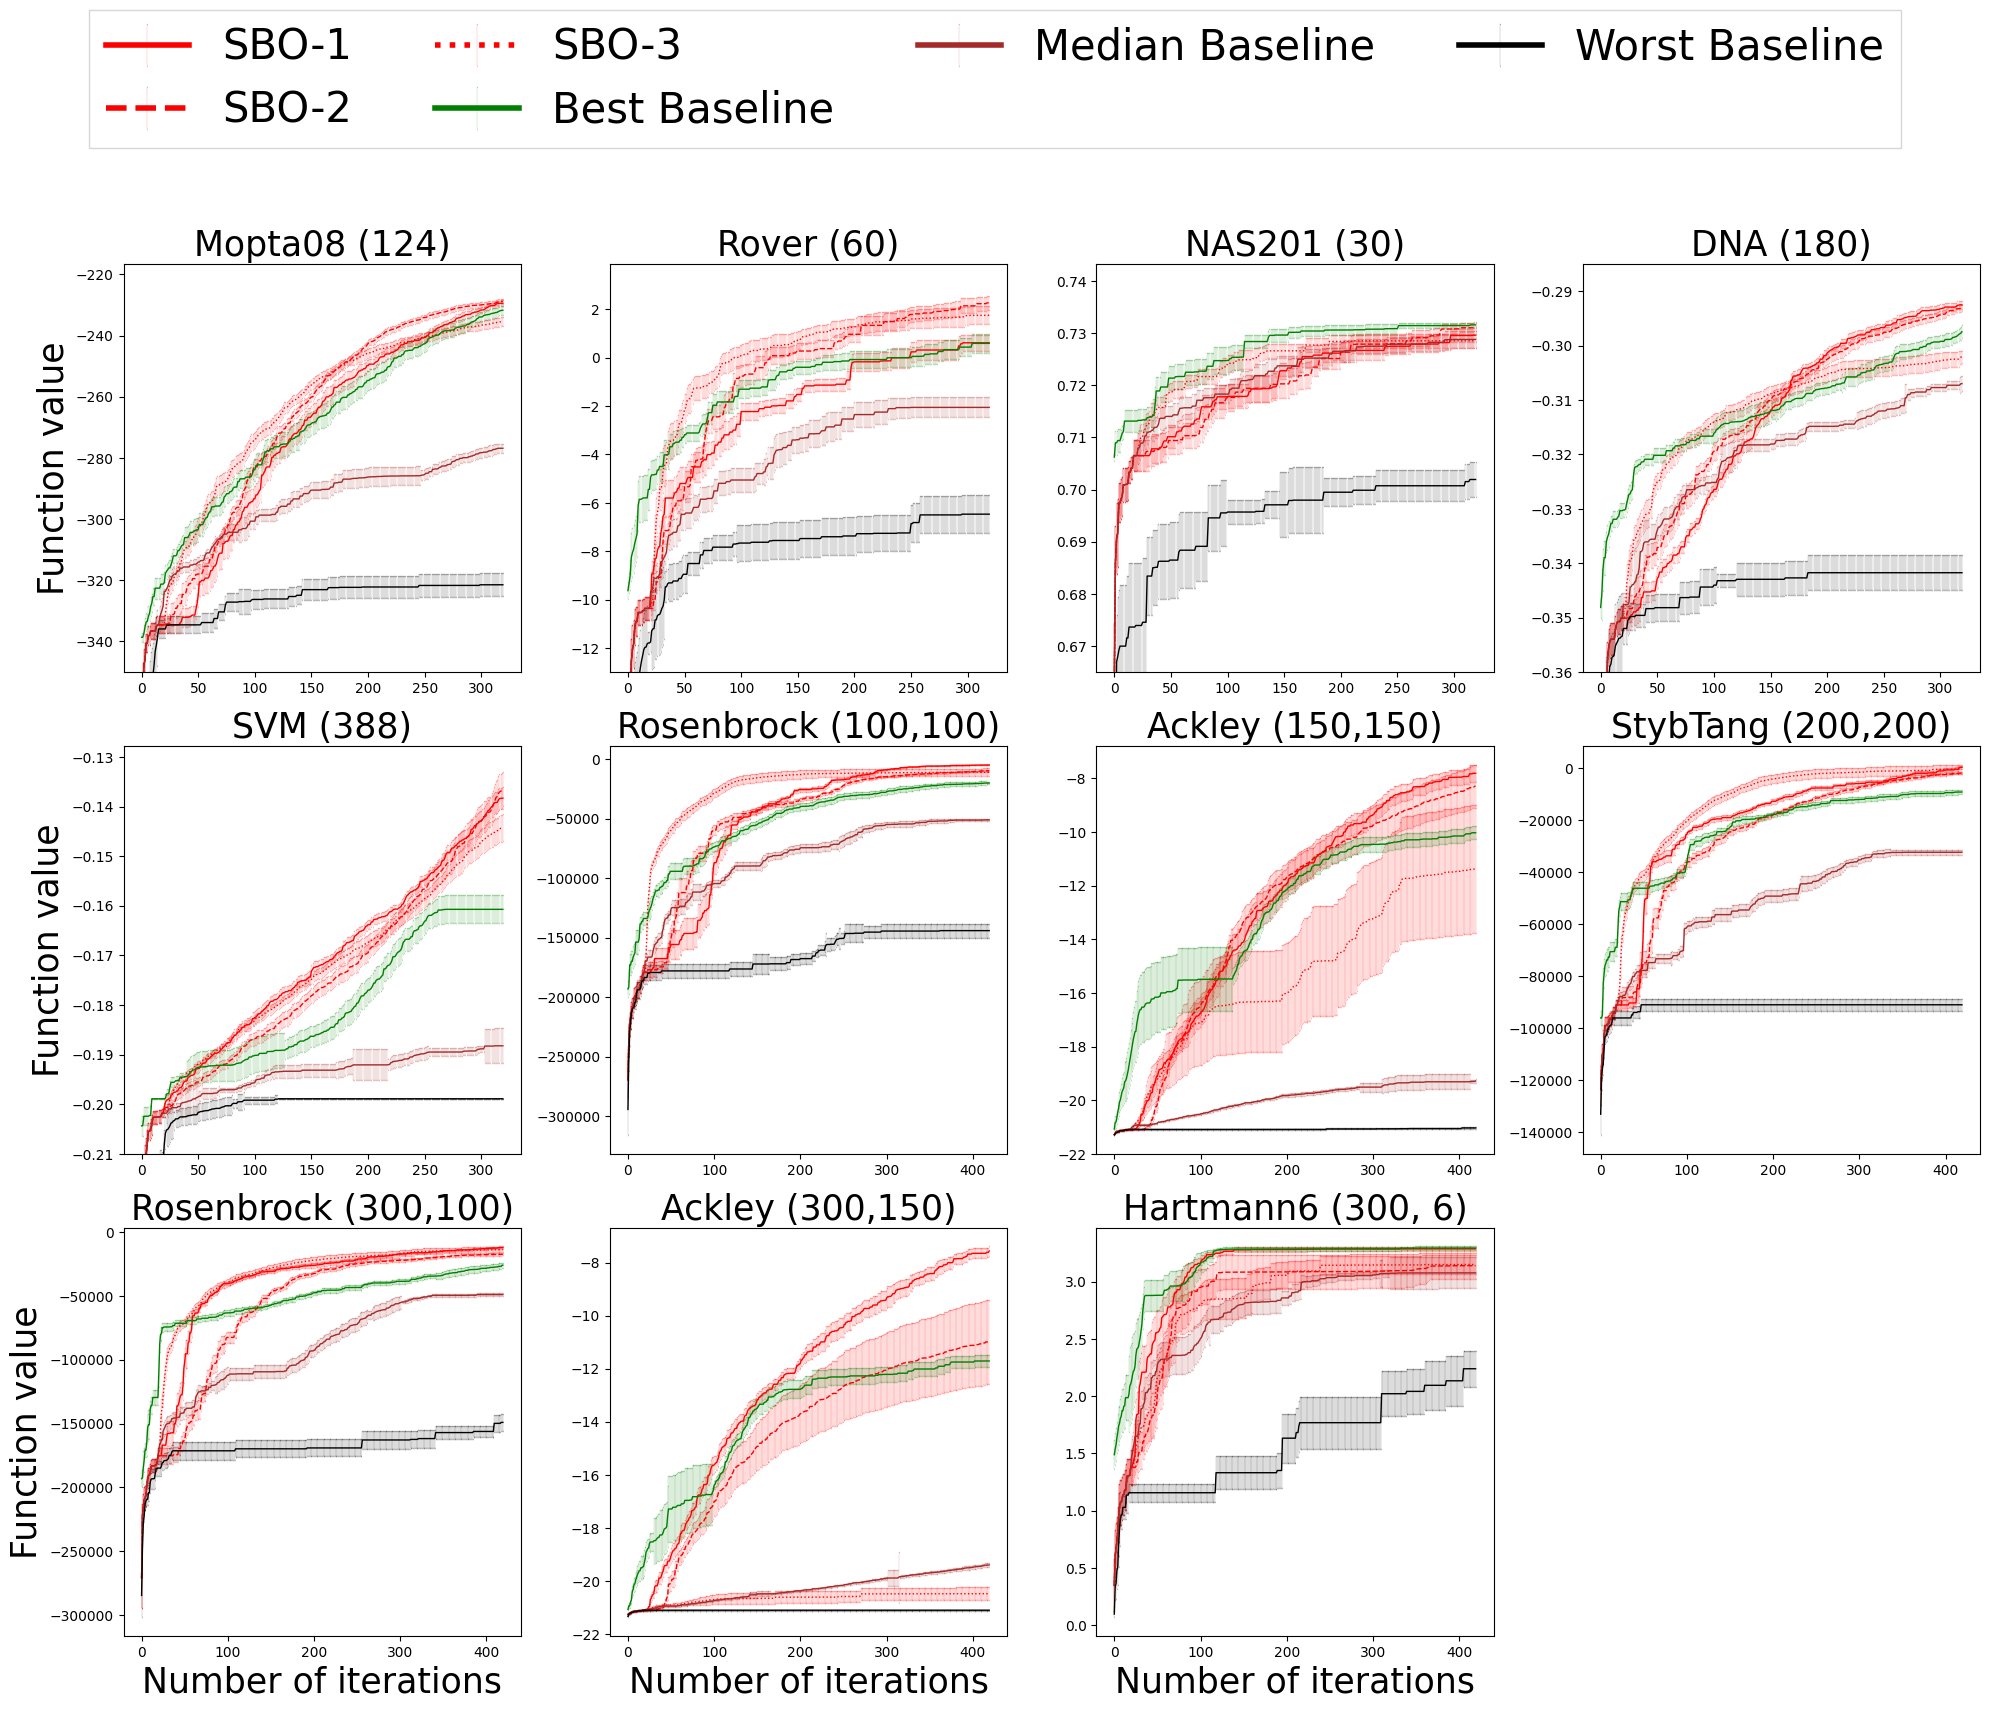}
    \caption{\small Runtime performance: Maximum Function Value obtained \textit{vs.} Number of Steps in real-world benchmarks, including SBO-3, namely training with a single length-scale parameter in Mat\'ern-5/2 kernel. The results were averaged from 10 runs. The shaded region depicts the standard deviation. }
    \label{fig:running-all-with-std-sbo3}
\end{figure*}



% \begin{table*}[h!]
% \centering
% \begin{tabular}{lrrrrr}
% \toprule
% {} &  Mopta08 (124) &   Rover (60) &  NAS201 (30) &   DNA (180) &    SVM (388) \\
% \midrule
% \textbf{GP    } &     3.96 &    2.84 &    2.71 &     4.43 &     8.82 \\
% \textbf{GPARD} &    11.23 &    9.84 &    5.76 &    14.34 &    32.16 \\
% \textbf{GPARD-NUTS}&    492.62 &   404.17  &   393.62  &   575.03  &   768.29\\
% \textbf{TURBO-1            } &     0.52 &    0.34 &    0.29 &     0.71 &    12.45 \\
% \textbf{TURBO-5            } &     1.25 &    1.07 &    0.59 &     1.49 &    13.06 \\
% \textbf{HESBO-10           } &     0.97 &    1.83 &    5.17 &     1.31 &    11.06 \\
% \textbf{HESBO-20           } &     1.19 &    3.01 &    8.07 &     1.64 &    11.36 \\
% \textbf{ALEBO-10           } &    41.54 &   32.61 &   60.65 &    54.47 &    46.37 \\
% \textbf{ALEBO-20           } &   108.46 &  102.84 &  123.17 &   120.90 &   113.71 \\
% \textbf{SaasBO-MAP        } &    46.53 &   41.36 &   42.35 &    51.33 &    67.37 \\
% \textbf{SaasBO-NUTS          } &   985.76 &  375.06 &  229.07 &  1739.56 &  2269.50 \\
% \textbf{RDUCB             } &     2.23 &    0.97 &    0.76 &     4.64 &    25.93 \\
% \textbf{Tree UCB          } &     1.45 &    0.89 &    0.40 &     1.33 &    12.85 \\
% \bottomrule
% \end{tabular}
% \caption{Average runtime per iteration on real world benchmarks in second.}
% \label{table:real runtime}
% \end{table*}




% \cmt{
% \begin{table*}[h!]
% \centering
% \begin{tabular}{lrrrrrr}
% \toprule
%     {} &  Rosenbrock &   Ackley &  Stybtang &  Rosenbrock &  Ackley &  Hartmann6 \\
%     (D, d) & (100,100) & (150, 150) & (200, 200) & (300, 100) & (300, 150) & (300, 6)\\
%     \midrule
%     \textbf{GP    } &           4.86 &     5.11 &         5.70 &              6.27 &       6.23 &       6.67 \\
%     \textbf{GPARD} &           8.85 &    12.94 &        13.67 &             12.63 &       9.99 &       8.81 \\
%     \textbf{GPARD-NUTS} &   857.21  &   850.23  &   1120.28 &   1276.42 &   1049.78 &   948.25\\
%     \textbf{TURBO-1            } &           0.39 &     0.35 &         0.41 &              0.39 &       0.38 &       0.39 \\
%     \textbf{TURBO-5            } &           1.28 &     1.25 &         1.30 &              1.24 &       1.31 &       1.34 \\
%     \textbf{HESBO-10           } &           0.17 &     0.99 &         0.17 &              0.31 &       1.24 &       1.00 \\
%     \textbf{HESBO-20          } &           0.16 &     1.34 &         0.16 &              0.32 &       1.58 &       1.04 \\
%     \textbf{ALEBO-10           } &          57.43 &    34.55 &        58.95 &             71.19 &      35.36 &      52.35 \\
%     \textbf{ALEBO-20           } &         158.10 &   124.25 &       159.75 &            177.19 &     140.99 &     152.54 \\
%     \textbf{SaasBO-MAP       } &          70.17 &    70.69 &        66.35 &            100.79 &      85.86 &      85.72 \\
%     \textbf{SaasBO-NUTS            } &        1294.90 &  1621.60 &      1511.99 &           1938.53 &     925.80 &    2204.54 \\
%     \textbf{RDUCB             } &           2.70 &     4.37 &         6.65 &             12.65 &      12.36 &      13.54 \\
%     \textbf{Tree UCB          } &           1.13 &     1.25 &         2.72 &              4.56 &       2.50 &       2.14 \\
% \bottomrule
% \end{tabular}
% \caption{Average running time per training iteration (in seconds) in synthetic benchmark tasks.}
% \label{tb:syn-runtime}
% \end{table*}
% }

% \subsection{NN-Prune Details}\label{sect:nn-prune}
% Given specific per-layer pruning rates $\x = [x_1, \ldots, x_{151}]$, the pruning procedure is as follows. The weights in each layer $i$ are first ranked according to their magnitudes, and the bottom $x_i$ portion of the weights are removed. The pruned network is then fine tuned on Tiny ImageNet~\citep{Le2015TinyIV}. The prediction accuracy after pruning and fine tuning on a separate test dataset is used as the target function. To respect the global pruning rate constraint $\alpha$, we add to the objective a soft penalty term $-\lambda\cdot\max(\alpha - \beta, 0)$, where $\beta$ is the global pruning rate reflected from $\x$. Note that the penalty is only incurred when $\alpha>\beta$. When $\alpha < \beta$, namely, the network is pruned to be sparser than the expected level, the test accuracy typically experienced a significant decline. Consequently, the optimization process  automatically adjusts to increase $\beta$. 
% We set $\lambda = 8.0$ to introduce a strong penalty. In our experiment, we employed $\alpha=0.5$.

%  Neural network pruning\citep{blalock2020state} is aimed to prune out large amount neurons inside a trained neural network and keep the pruned ones with high accuracy. In other word, we want to reduced size of a neural network, without losing too much on performance. Modern neural networks are giant in size, Resnet152\citep{he2015deep} has more than 60 Million parameters. It has been shown that pruning out reasonable percentage of weights can still preserve most of its performance \citep{blalock2020state}. In this benchmark, we used Resnet152. And prune out neurons with a small absolute magnitude. Since most neuron appears in convolutional layer, we will only perform pruning on those layer, which means we have a 151 dimensional input space. We define pruning rate to be a continuous number in $[0, 1]$, 0 means no pruning and 1 means prune out everything. Suppose a neural network has $\M$ prunable layers, each layer has $N_{*}$ neurons, and total number of neurons before pruning is $N_{total}=\sum_{i=1}^{M}N_{i}$. Now we can define our benchmark function as follow,
% $$f_{\textit{NNP}}(x;\gamma)=g(x;\gamma)-\lambda \times \text{max}(\alpha-\beta, 0) \text{, where } x\in[0, 1]^{D}$$
% Here $\gamma$ is a dataset, $g : [0, 1]^{D} \rightarrow [0, 1]$ is a black-box function that take pruning rate per layer as input and return testing accuracy on $\gamma$ by the pruned neural network. $\lambda$ is a predefined positive constant, which represent penalty rate. $\alpha$ is a predefined global pruning rate. $\beta=\frac{N\cdot x}{N_{total}}$, it indicates pruning rate of $x$. In our experiments, we set $\lambda=8.0$ and $\alpha=0.5$ so we can have enough signal from $f_{\textit{NNP}}$ for training surrogate model in BO, while prune out around half of parameters in Resnet152. We set $\gamma$ as Tiny ImageNet\citep{Le2015TinyIV} for faster inference speed compared with full ImageNet\citep{5206848}. In our experiments, We initialized $g$ as a fine-tuned version of Resnet-152 on Tiny ImageNet.

% \begin{figure*}[!ht]
%     \centering
%     \includegraphics[width=\textwidth]{BO ICLR 2025/figs/others/BO_choices.png}
%     \caption{Different setting for traditional BO(GP, GPARD) we evaluated. Blue box is the setting we used in \ref{sec:experiments}.}
%     \label{fig:6}
% \end{figure*}

% \section{Traditional BO performance difference under different settings}
% \label{APP_B}
% In this section, we added results of GP and GP-ARD performance under different setting. \ref{fig:6} is a clear view of all different settings we tested on,

% For both GP and GPARD, we tested with 8 different settings. To make comparison clear, we will compare settings with only one difference each time, and fix other setting options. We run experiments on all previous benchmark functions besides Neural network pruning. 

% \subsection{$\lambda$ value in UCB}
% As previously discussed in \ref{acqf}, $\lambda$ value in UCB controls level of exploration. We tested the effect on different choices of $\lambda=1.0, 1,5$ and we didn't notice any significant different in performance on most benchmark functions. Results are displayed in \ref{fig:7} and \ref{fig:8}. The only benchmark that has a clear different is full rank Ackley and low rank Ackley. In those two benchmark functions, a larger $\lambda=1.5$ value yield better performance. In our opinion, this is because Ackley function has a lot of local optimal. A larger $\lambda$ will lead to more exploration, and avoid stuck at local optimal.
% \begin{figure*}[!ht]
%     \centering
%     \includegraphics[width=\textwidth]{BO ICLR 2025/figs/others/lambda.png}
%     \caption{Traditional BO performance with different $\lambda$ value. Mean value is shown in this plot.}
%     \label{fig:7}
% \end{figure*}

% \begin{figure*}[!ht]
%     \centering
%     \includegraphics[width=\textwidth]{BO ICLR 2025/figs/others/lambda_violin.png}
%     \caption{Traditional BO performance with different $\lambda$ value.Final iteration values with mean, extremas and variance are shown in this plot.}
%     \label{fig:8}
% \end{figure*}

% \begin{figure*}[!ht]
%     \centering
%     \includegraphics[width=\textwidth]{BO ICLR 2025/figs/others/acqf_ls_constraint.png}
%     \caption{Traditional BO performance with different acquisition functions and different lengthscale constraints. Mean value is shown in this plot.}
%     \label{fig:9}
% \end{figure*}

% \begin{figure*}[!ht]
%     \centering
%     \includegraphics[width=\textwidth]{BO ICLR 2025/figs/others/acqf_ls_constraint_violin.png}
%     \caption{Traditional BO performance with different acquisition functions and different lengthscale constraints. Final iteration values with mean, extremas and variance are shown in this plot.}
%     \label{fig:10}
% \end{figure*}

% \subsection{UCB vs EI}
% Despite both EI and UCB encourage next point with high mean and high variance, maximizing them will yield different solutions. So we compared traditional BO with UCB and EI in \ref{fig:9} and \ref{fig:10}. Based on empirical results, traditional BO generally works better with UCB. The only case that EI works extremely well compared with UCB is Hartmann6. It performance is comparable to ALEBO(d=20) and SaasBO. The setting is GPARD with EI as acquisition function and use exponential function for positive lengthscale constraint. We will discuss lengthscale constraints in next subsection.

% \subsection{Lengthscale constraints}
% Lengthscale constraints is the most overlooked factor in traditional BO. First, kernel lengthscales must be positive. If we are training kernel parameters by maximizing log likelihood with gradient methods, then we need to place a positive constraint over lengthscale parameters. The most common one is Exponential function, while Softplus is the default in GPytorch\citep{gardner2021gpytorch}. For results shown in \ref{fig:9} and \ref{fig:10}, the choice of lengthscale constraint is the most crucial setting among all. Exponential constraint has the worst performance for most cases. This is not obvious in GP, but devastating for GPARD. See red line(GPARD-UCB-Exp) and yellow line(GPARD-UCB-Softplus) in \ref{fig:10} for clear comparison.

% \subsection{Posterior sampling vs maximizing log likelihood}
% The last aspect is training methods. Point estimation(MLL) is the most common approach to learn GP parameters, due to its efficiency. Nonetheless, posterior sampling with MCMC is still a powerful way to acquire GP parameters. We compared performance difference of MLL and posterior sampling in \ref{fig:11} and \ref{fig:12}. We used No-U-Turn-Sampler(NUTS), which is an adaptive variant of the Hamiltonian Monte Carlo (HMC) method.  We didn't notice any particular performance difference between MLL and posterior sampling. GPARD-UCB-MLL and GPARD-UCB-NUTS both performed quite well, besides two Ackley functions, where NUTS seems to be not working at all. We believe this is also because Ackley function has a lot of local optimal and MLL can actually create randomness, which will avoid stuck at local optimal.

\subsection{Implementation}\label{sect:impl}
\begin{itemize}
    \item \textbf{ALEBO.} We used ALEBO implementation shared by the  Adaptive Experimentation (AX) Platform  (version 0.2.2). The source code is at  \url{https://github.com/facebook/Ax/blob/main/ax/models/torch/alebo.py}.
    \item \textbf{HESBO.} We used HESBO implementation of the original authors (\url{https://github.com/aminnayebi/HesBO}).
    \item \textbf{TURBO.} We used the original TURBO implementation (\url{https://github.com/uber-research/TuRBO})
    \item \textbf{SaasBO-NUTS.} We used the original implementation of the authors  (\url{https://github.com/martinjankowiak/saasbo}). %and the re-implementation in BoTorch. The original implementation yield better result, but with a higher runtime. All reported experiment results is from original implementation.
    \item \textbf{SaasBO-MAP.} The SaasBO implementation available to the public does not include the version using MAP estimation.  We therefore implemented this method based on the original paper~\citep{eriksson2021highdimensional}. All the hyperparameter settings follow exactly the same as the original paper.
    \item \textbf{RDUCB and Tree UCB.} The implementation of both methods is publicly available at \url{https://github.com/huawei-noah/HEBO/tree/master/RDUCB}.
    \item \textbf{BNN Laplace and BNN HMC.} {For BNN Laplace, we used the implementation at \url{https://github.com/wiseodd/laplace-bayesopt}, and for BNN HMC, we used the implementation at \url{https://github.com/yucenli/bnn-bo}. To identify the architecture of the neural network, we perform leave-one-out cross-validation on the initial dataset for each task. The layer width and depth were selected from \{1, 2, 3\} $\times$ \{32, 64, 128, 256\}. The activation function for BNN Laplace is ReLU and for BNN HMC is Tanh, which is the default choice of each method. For BNN Laplace, the training was conducted by maximizing marginal likelihood with ADAM, with learning rate of 1E-01, and weight decay of 1E-03. For HMC, the BNN is pre-trained by maximizing log likelihood with ADAM. Then followed by HMC sampling procedure. We used their adaptive step size schedule for the Leap frog, and the number of steps was set to 100.}
\end{itemize}

\subsection{Computing Environment}
\label{sect:compute-env}
We conducted the experimental investigations on a large computer cluster equipped with Intel Cascade Lake Platinum 8268 chips. 


\begin{table*}[h!]
\small
\centering
\begin{tabular}{lccccc}
\toprule
{\textit{Task}} &   ARD Mat\'ern &  Mat\'ern &  SaasBO &  Proj-GP &  Add-GP \\
\midrule
{Mopta08(124)}      & \textbf{0.570}$\pm$0.08 & -0.277$\pm$0.101 & \textbf{0.560}$\pm$0.064 & -0.962$\pm$0.183 & -0.089$\pm$0.105 \\
{Rover(60)}         & -0.975$\pm$0.216 & \textbf{-0.647}$\pm$0.158 & \textbf{-0.638}$\pm$0.14 & -0.995$\pm$0.116 & -0.703$\pm$0.125 \\
{DNA(180)}          & \textbf{-0.256}$\pm$0.261 & -0.666$\pm$0.102 & \textbf{-0.183}$\pm$0.158 & -1.137$\pm$0.143 & -0.679$\pm$0.143 \\
{SVM(388) }         & \textbf{0.581}$\pm$0.119 & -0.179$\pm$0.042 & \textbf{0.650}$\pm$0.12 & -0.837$\pm$0.095 & 0.062$\pm$0.129 \\
{Ackley(150, 150)}  & 0.428$\pm$0.222 & \textbf{0.633}$\pm$0.067 & \textbf{0.574}$\pm$0.068 & -0.006$\pm$0.268 & 0.569$\pm$0.066 \\
{Ackley(300, 150)}  & 0.232$\pm$0.155 & \textbf{0.252}$\pm$0.057 & \textbf{0.279}$\pm$0.077 & -0.372$\pm$0.185 & 0.220$\pm$0.074 \\
{Hartmann6(300, 6)} & \textbf{1.200}$\pm$0.169 & -0.625$\pm$0.079 & \textbf{1.528}$\pm$0.564 & -0.927$\pm$0.084 & -0.617$\pm$0.118 \\
{Rosenbrock(100, 100)} & \textbf{0.640}$\pm$0.081 & 0.445$\pm$0.062 & \textbf{0.526}$\pm$0.08 & -0.466$\pm$0.182 & 0.521$\pm$0.057 \\
{Rosenbrock(300, 100)} & \textbf{0.518}$\pm$0.225 & 0.121$\pm$0.155 & \textbf{0.357}$\pm$0.21 & -0.706$\pm$0.209 & 0.189$\pm$0.2 \\
{Stybtang(200, 200)} & \textbf{0.574}$\pm$0.164 & 0.563$\pm$0.073 & 0.543$\pm$0.067 & -0.458$\pm$0.069 & \textbf{0.582}$\pm$0.072 \\
\bottomrule
\end{tabular}
\caption{Test log likelihood of each surrogate model. The results were averaged over five runs. Bolded are the best and second best results.}
\label{tb:test-ll}
\end{table*}

\begin{table*}[h!]
\small
\centering
\begin{tabular}{lrrrrr}
\toprule
{} &  Mopta08 (124) &   Rover (60) &  NAS201 (30) &   DNA (180) &    SVM (388) \\
\midrule
{ARD Mat\'ern-MAP} &    7.39 &    9.99 &    7.81 &    9.77 &    13.55 \\
{ARD Mat\'ern-MLE} &    11.23 &    9.84 &    5.76 &    14.34 &    32.16 \\
{ARD Mat\'ern-NUTS}&    492.62 &   404.17  &   393.62  &   575.03  &   768.29\\
{SaasBO-MAP        } &    46.53 &   41.36 &   42.35 &    51.33 &    67.37 \\
{SaasBO-NUTS          } &   985.76 &  375.06 &  229.07 &  1739.56 &  2269.50 \\
\bottomrule
\end{tabular}
\caption{Average running time (in seconds) per optimization step in real-world benchmark tasks.}
\label{tb:real-runtime}
\end{table*}
\begin{table*}[h!]
\small
\centering
\begin{tabular}{lcccccc}
\toprule
    {} &  Rosenbrock &   Ackley &  Stybtang &  Rosenbrock &  Ackley &  Hartmann6 \\
     & (100,100) & (150, 150) & (200, 200) & (300, 100) & (300, 150) & (300, 6) \\
    \midrule
    {ARD Mat\'ern-MAP} &           8.52 &    36.26 &        21.42 &             16.36 &       25.90 &       51.56 \\
    {ARD Mat\'ern-MLE} &           8.85 &    12.94 &        13.67 &             12.63 &       9.99 &       8.81 \\
    {ARD Mat\'ern-NUTS} &   857.21  &   850.23  &   1120.28 &   1276.42 &   1049.78 &   948.25\\
    {SaasBO-MAP       } &          70.17 &    70.69 &        66.35 &            100.79 &      85.86 &      85.72 \\
    {SaasBO-NUTS            } &        1294.90 &  1621.60 &      1511.99 &           1938.53 &     925.80 &    2204.54 \\
\bottomrule
\end{tabular}
\caption{\small Average running time (in seconds) per optimization step on synthetic benchmark tasks.}
\label{tb:syn-runtime}
\end{table*}

%\begin{wraptable}{r}{0.55\textwidth}
\begin{table}
%\vspace{-0.15in}
\centering
\small
\begin{tabular}{c | c} 
\hline\hline
 \textit{Method} & \textit{Structural Assumption} \\
 \hline
   ALEBO, HESBO & {Low-dim embedding} \\ 
  %\hline
  SaasBO & Partial variable dependency\\ 
%\hline
 RDUCB, Tree UCB & Additive function decomposition \\
% \hline
  SBO, TURBO, BNN & None\\ \hline
\end{tabular}
\caption{\small BO methods and their structural assumption about the target function.} \label{tb:method-assumptions}
\label{table:1}
\end{table}
%\vspace{-0.1in}
%\end{wraptable}


\begin{figure*}[t]
    \centering
    \includegraphics[width=\textwidth]{BO ICLR 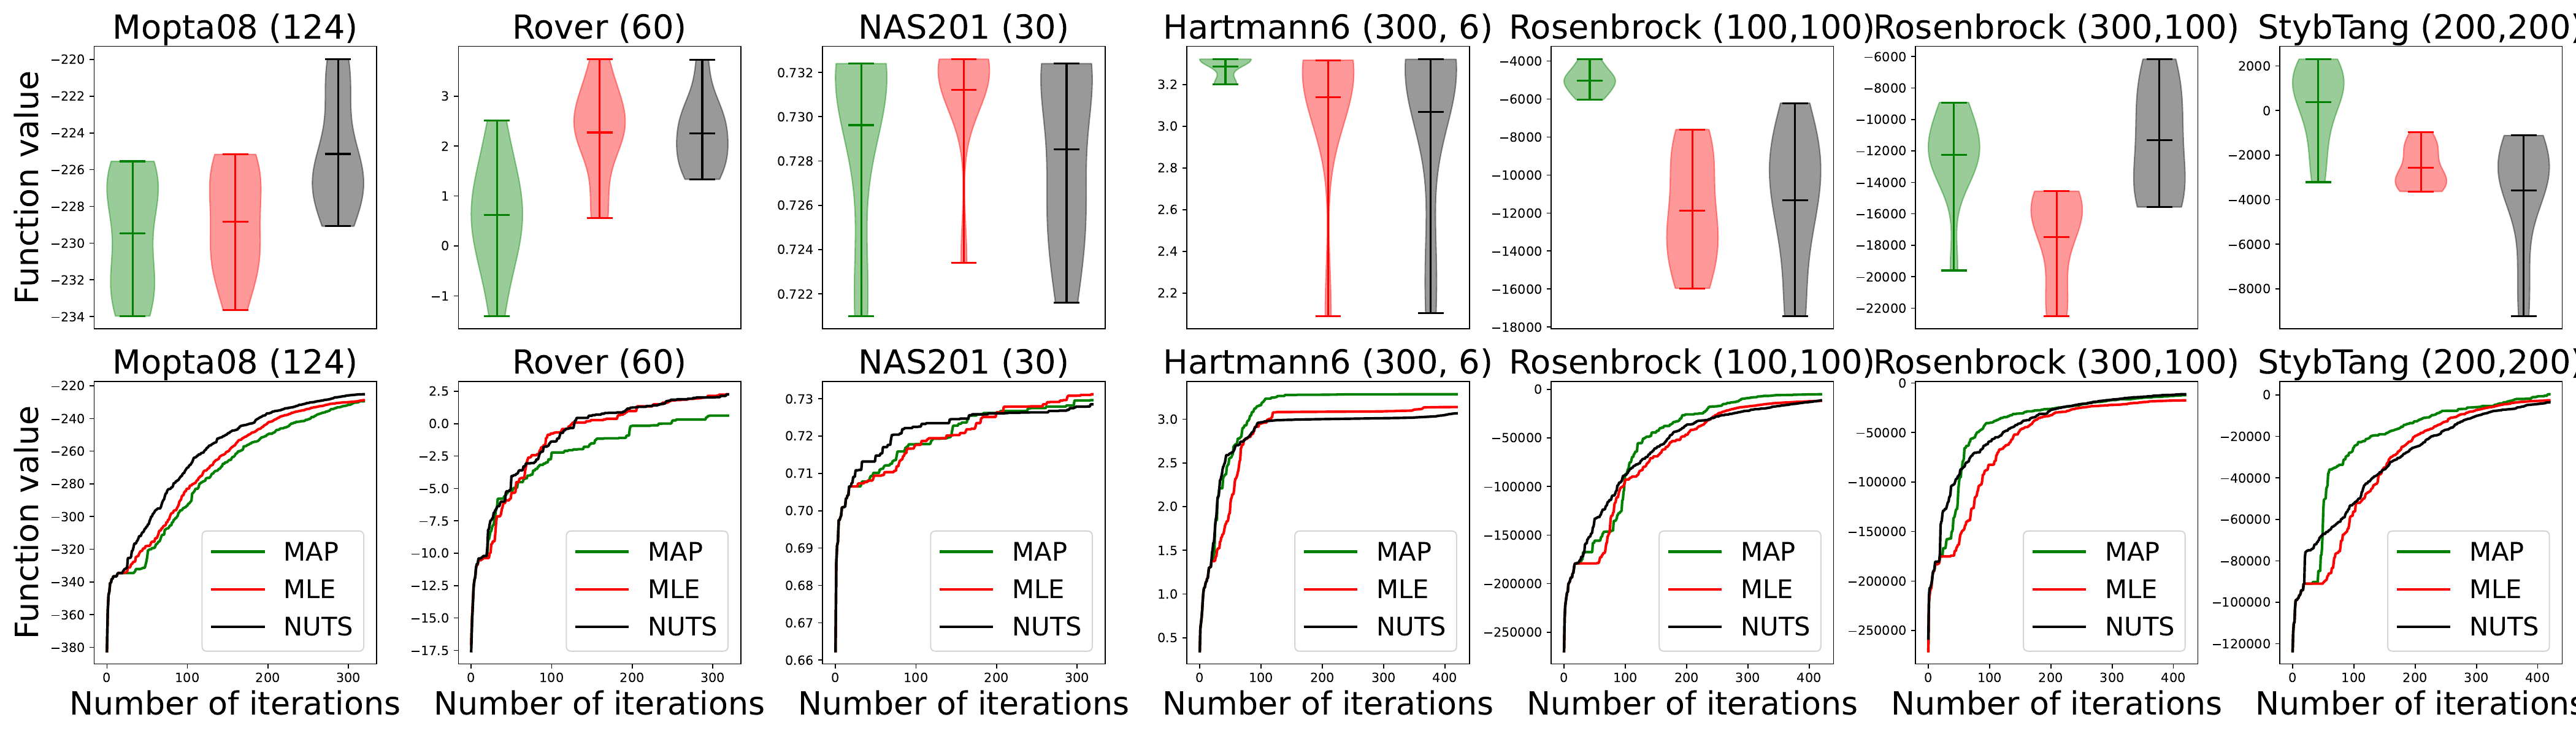}
    \caption{\small Optimization performance using MLE training,  MAP training with a diffuse prior over the length-scale parameters, and  NUTS on the rest of benchmarks. The results were summarized from 10 runs.}
    \label{fig:op-performance-gpard-nuts-rest}
\end{figure*}

\section{Proofs}\label{sect:proof}
\subsection{Proof of Lemma~\ref{lem:tau-se} }
\begin{proof}
    We intend to solve $\rho^2/e^{\rho^2} < \xi$, which is equivalent to solving
    \[
     \log r - r < \log \xi, 
    \]
    where $r = \rho^2$. 
    We then leverage the fact that $\log r < \sqrt{r}$ when $r > 1$. Since $1/e > \xi$, we know the solution of $\rho$ must be larger than 1, implying that the solution for $r$ is larger than $1$. To meet the inequality, we can solve 
    \[
    \log r - r < \sqrt{r} - r < \log \xi. 
    \]
    It then converts to a quadratic form, 
    \begin{align}
        \sqrt{r} - \sqrt{r}^2 < \log \xi.
    \end{align}
    Note that $\rho = \sqrt{r}$.     It is straightforward to solve this inequality and we can obtain that the inequality holds when
    \[
    \rho > \tau_{\text{SE}} = \frac{1}{2} + \sqrt{\frac{1}{4} - \log \xi}. 
    \]
    
\end{proof}
\subsection{Proof of Lemma~\ref{lem:prob-bound}}\label{sect:bound-proof-1}
\begin{proof}
    First, since each $x_{ik}$ and $x_{jk}$ independently follow $\text{Uniform}(0, 1)$, it is straightforward to obtain $\EE[(x_{ik} - x_{jk})^2] = \frac{1}{6}$. 
    Let us define $\gamma = \|\x_i - \x_j\|^2$. Then we have $\EE[\gamma] = \frac{1}{6}d$.
    According to Hoeffding's inequality,  for all $t>0$,
    \begin{align}
        p(|\gamma - \frac{1}{6}d| \ge t) \le  2\exp\left(-\frac{2t^2}{d}\right). \label{eq:hoeff}
    \end{align}
    Since $\rho = 
    \frac{\sqrt{\gamma}}{\ell_0}$, we have  $p(\rho > \tau) = p(\gamma > \tau^2\ell_0^2)$. Since $d>6\ell_0^2\tau^2$, we set $t = \frac{1}{6}d - \ell_0^2\tau^2>0$, and apply \eqref{eq:hoeff} to obtain
    \[
    p(|\gamma - \frac{1}{6}d| \ge \frac{1}{6}d -  \ell_0^2\tau^2|) \le 2\exp\left(-\frac{2\left(\frac{1}{6}d -  \ell_0^2\tau^2\right)^2}{d}\right)
      = 2 \exp\left(-\frac{\left(d - 6\ell_0^2\tau^2\right)^2}{18d}\right),
    \]
    which is equivalent to
    \begin{align}
        p(|\gamma-\frac{1}{6}d| < \frac{1}{6}d - \ell_0^2\tau^2) > 1 - 2 \exp\left(-\frac{\left(d - 6\ell_0^2\tau^2\right)^2}{18d}\right).\label{eq:bound2}
    \end{align}
Since $p(\gamma > \ell_0^2 \tau^2) \ge p( \ell_0^2 \tau^2 < \gamma < \frac{1}{3}d - \ell_0^2 \tau^2) = 
p(|\gamma - \frac{1}{6}d| < \frac{1}{6}d - \ell_0^2\tau^2)$, combining with \eqref{eq:bound2} we obtain the bound
\[
p(\rho>\tau) = p(\gamma > \ell_0^2 \tau^2) > 1 - 2 \exp\left(-\frac{\left(d - 6\ell_0^2\tau^2\right)^2}{18d}\right).
\]
\end{proof}

\subsection{Proof of Lemma~\ref{lem:tau-matern}}
\begin{proof}
    To solve $\rho^2/e^{\sqrt{5}\rho} < \xi$, it is equivalent to solving
    \[
    \frac{1}{5} \frac{r^2}{e^r} < \xi, \;\;\; r = \sqrt{5}\rho,
    \]
    which is further equivalent to 
    \[
    \log \frac{1}{5} + 2 \log r - r < \log \xi. 
    \]
    We leverage $\log r < \sqrt{r}$ for $r>1$, and solve the upper bound, 
    \[
    \log\frac{1}{5} + 2 \sqrt{r}-r < \log \xi,
    \]
    which gives 
    \begin{align}
        \rho > \tau_{\text{Mat\'ern}} = \frac{1}{\sqrt{5}}\left(1 + \sqrt{1 + \log 1/5 - \log\xi}\right)^2.
    \end{align}
\end{proof}

\subsection{Proof of Lemma~\ref{lem:new-bound}}
\begin{proof}
    First, similar to the proof in Section~\ref{sect:bound-proof-1}, under the uniform distribution on $[0, 1]^d$, from Hoeffding's inequality, we have for all $t>0$,
        \begin{align}
        p(|\gamma - \frac{1}{6}d| \ge t) \le  2\exp\left(-\frac{2t^2}{d}\right). \label{eq:hoeff-again}
    \end{align}

    When we set $\ell_0 = c\sqrt{d}$ such that $c>1/ \sqrt{6}\tau$, we have $\ell_0^2 \tau^2 > d/6 $. Let us choose $t = \ell_0^2\tau^2 - d/6=c^2 \tau^2d - d/6>0$, and apply the Hoeffding's inequality~\eqref{eq:hoeff-again}, 
    \begin{align}
        p\left(|\gamma - d/6 | \ge \ell_0^2\tau^2 - d/6\right) \le 
        2\exp\left(-\frac{2(\ell_0^2\tau^2 - d/6)^2}{d}\right) = 2\exp\left(-2(c^2\tau^2 - \frac{1}{6})^2d\right)
    \end{align}
    Since $p(\rho \ge \tau) = p(\gamma \ge \ell_0^2\tau^2) \le p(|\gamma - d/6 | \ge \ell_0^2\tau^2 - d/6)$, we obtain
    \[
    p(\rho \ge\tau) \le 2\exp\left(-2(c^2\tau^2 - \frac{1}{6})^2d\right).
    \]
\end{proof}

\section{Ablation Study and Failure Modes With Other Settings}\label{sect:fail}
%\section{Failure Modes and settings for Standard Bayesian optimization}\label{sect:fail}
%\xuc{I changed the section title a little bit. Previous title is commented out.}

%In this section, we investigated alternative settings in executing standard BO. \xuc{Since we have shown in main paper that SBO is able to perform great in high dimension, and previous paper all claimed that Standard BO does not work well empirically for functions above 15 dimensions. We would like to know if that believe is caused by failure mode and settings.} With these settings, we \xuc{indeed} found failure modes in high-dimensional optimization problems, and provided analysis and discussion. \xuc{We will begin with the settings that degenerate BO performance the most, and end with settings that only mildly affect BO performance.}

In this section, we conducted a careful ablation study to investigate alternative popular  settings in executing standard BO.  From these settings, we identified a few failure modes during high-dimensional optimization. We provided analysis and discussions accordingly. 

\subsection{GP Training}
First, we examined MLE training with LBFGS. We found that, however, LBFGS often incurs numerical issues, and cannot reliably finish model training. This is consistent with the report in other works~\citep{hvarfner2024vanilla}. The issue might be because that without constraints (or regularization) over the parameters (such as the length-scales and amplitude), the exploration of LBFGS tends to be overly aggressive, which easily cause numerical problems. Hence, using stochastic optimization, like ADAM, might be a wise choice for MLE training.

Second, we examined MAP training with alternative prior choices over the length-scale parameters. In the main paper, we use a diffuse prior, \texttt{Uniform(0.001, 30)}. In practice, another commonly used choice is a concentrated Gamma prior, \eg \texttt{Gamma(3, 6)}, which is the default choice in the popular BO library BoTorch. To see how it is concentrated, in Fig. \ref{fig:pdf} we compare its probability density curve with other priors, including the aforementioned uniform prior and the diffuse Gamma priors over the amplitude and noise variance. 

We found that employing a concentrated prior over the length-scale parameters will severely deteriorate the high-dimensional optimization performance. 
As shown in Fig \ref{fig:final-Gamma36} and \ref{fig:runtime-Gamma36}, after placing the prior Gamma(3,6) over each length-scale parameter, both the ultimate and runtime optimization performance  drops substantially across many tasks, such as Mopta08 (124), SVM (388) and Ackley(150, 150), no matter using ADAM or LBFGS to conduct training. To figure out the reason, we further investigated the surrogate learning performance. Following the same setting as in Fig. \ref{fig:pred-alignment}, we examined the prediction alignment after applying the prior Gamma(3,6) over the length-scale parameters. As depicted in Fig. \ref{fig:alignment-more} (third and fourth column), this concentrated prior leads to a severe prediction deviation from the ground-truth, indicating failure in learning the target function. This is consistent with the report in the SaasBO paper~\citep{eriksson2021highdimensional} (see Fig.1 of that paper). 
The quantitative results shown in Table \ref{tb:mse-surrogate-gamm36} and \ref{tb:test-ll-surrogate-gamma36} further confirm the substantially worse prediction accuracy as compared with GP training with a diffuse prior. {In addition, we notice that the previous work\citep{li2024study} have also tested standard BO using Gamma(3,6) as the prior over the length-scale parameters. In their high-dimensional optimization experiments (see Fig. 5 of that paper), standard BO performs badly. We used our setting (SBO-1 and SBO-2) to re-run one experiment that maximizes a high-dimensional polynomial function. It turns out that both SBO-1 and SBO-2 can surpass the best method I-BNN reported by that paper.   } 

Together these results have shown that a concentrated prior can severely limit GP's capacity for high-dimensional function estimation, leading to inferior performance in high-dimensional optimization. 

%Note that, in BoTorch, the default priors over the amplitude and the noise variance are \texttt{Gamma(2.0, 0.15}) and \texttt{Gamma(1.1, 0.05)}, both of which are much more spreaded than \texttt{Gamma(3,6)}; see Fig. XX. 
%We found that, employing such as 



%\xuc{We acknowledge that our BO setting in main paper is not the most conventional in BO community. The most common setting is Gamma(3, 6) prior over lengthscale and trained with MAP estimation using LBFGS, which is the default setting for BO in Botorch (\textbf{singletaskgp}).}

%In this section, we examined training GP with MAP estimation with alternative choices of priors and more ADAM epochs. 

%First, we investigated the most commonly used prior over the length-scale parameter. That is Gamma(3, 6), the default choice in BOTorch library(\textbf{singletaskgp}). This is a concentrated Gamma prior, \xuc{where $\Phi(Gamma(3, 6))(1.40) \approx 0.99$.}
%However, we found that .... \xuc{As shown in Fig. \ref{fig:running-GP-training}, \ref{fig:final-GP-training} and Table \ref{tb:mse-GP-training}, there is a quite noticeable performance gap between a diffuse prior over length-scale parameters with MAP estimation, or MLE without any prior over length-scale and Gamma(3, 6) prior with MAP training. \textbf{We have noticed that some previous work\cite{li2024study} have included Standard BO used Botorch default setting, which is Gamma(3, 6) prior with MAP estimation. We re-run their Polynomial experiment with SBO-1, SBO-2. And the result is better than their I-BNN, which is the best method in their plot.} We would like to argue that the major cause for Standard BO to have such a bad performance in previous paper is due to prior selection. As we can see in the following, there is no other setting that could degenerate BO performance this much compare to a bad prior choice. To better illustrate how concentrate Gamma(3, 6) is, we included a CDF plot in Fig. \ref{fig:gamma-cdf}. }

\begin{figure*}[!ht]
    \centering
    \includegraphics[width=\textwidth]{BO ICLR 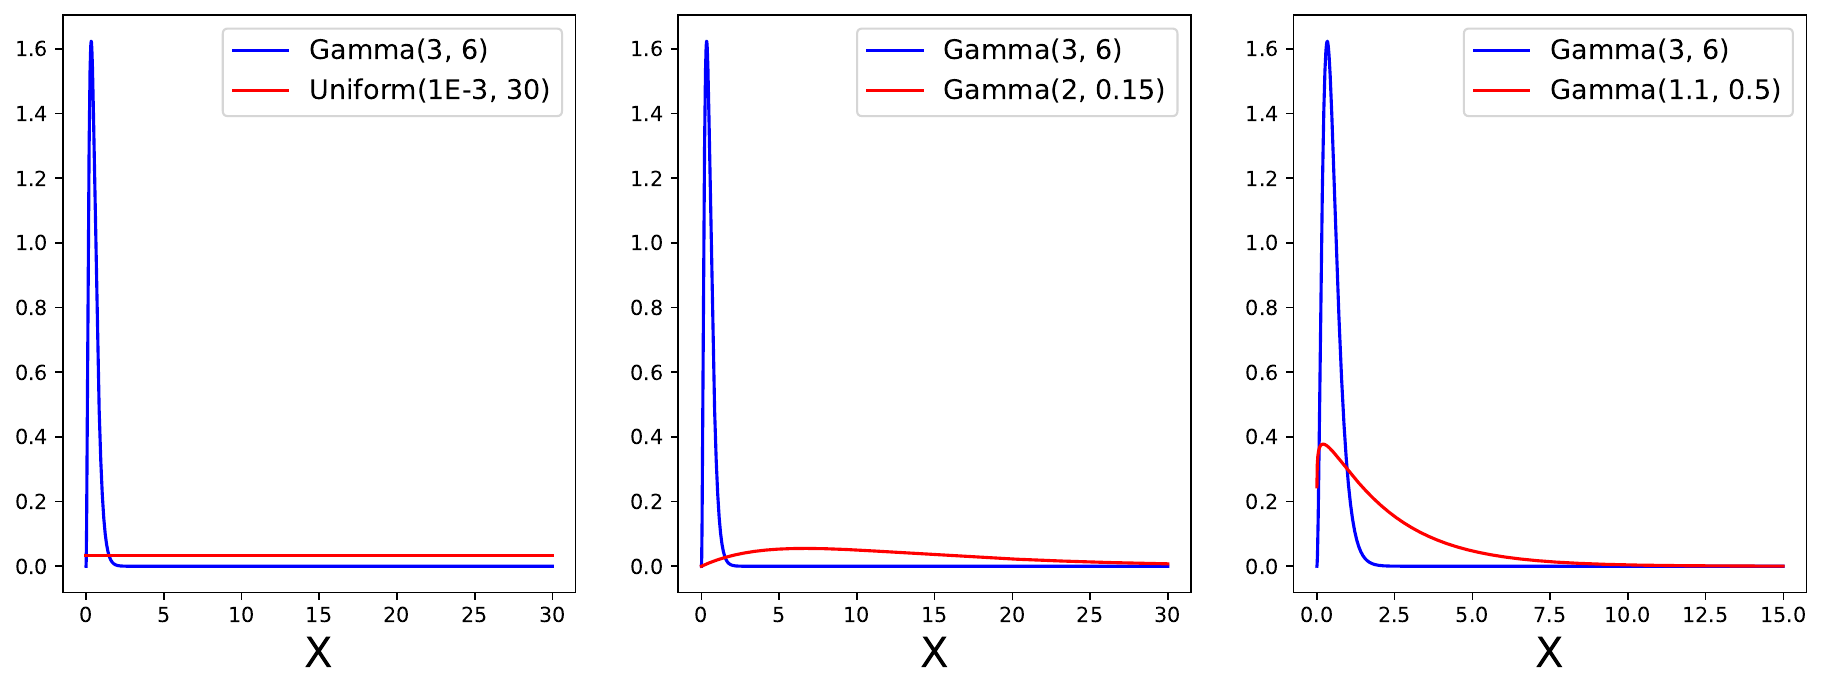}
    \caption{\small Probability density curves. Gamma(2, 0.15) and Gamma(1.1, 0.5) are the priors for the amplitude and noise variance, respectively.}
    \label{fig:pdf}
\end{figure*}

%\xuc{Also in 5.1, Fig. 1 of SaasBO \cite{eriksson2021highdimensional}, the only setting that could reproduce such a bad GP surrogate performance is using Gamma(3, 6) prior over length-scale, as shown in Fig. \ref{fig:gp-surrpgate-SaasBO}}

\begin{figure*}[!ht]
    \centering
    \includegraphics[width=\textwidth]{BO ICLR 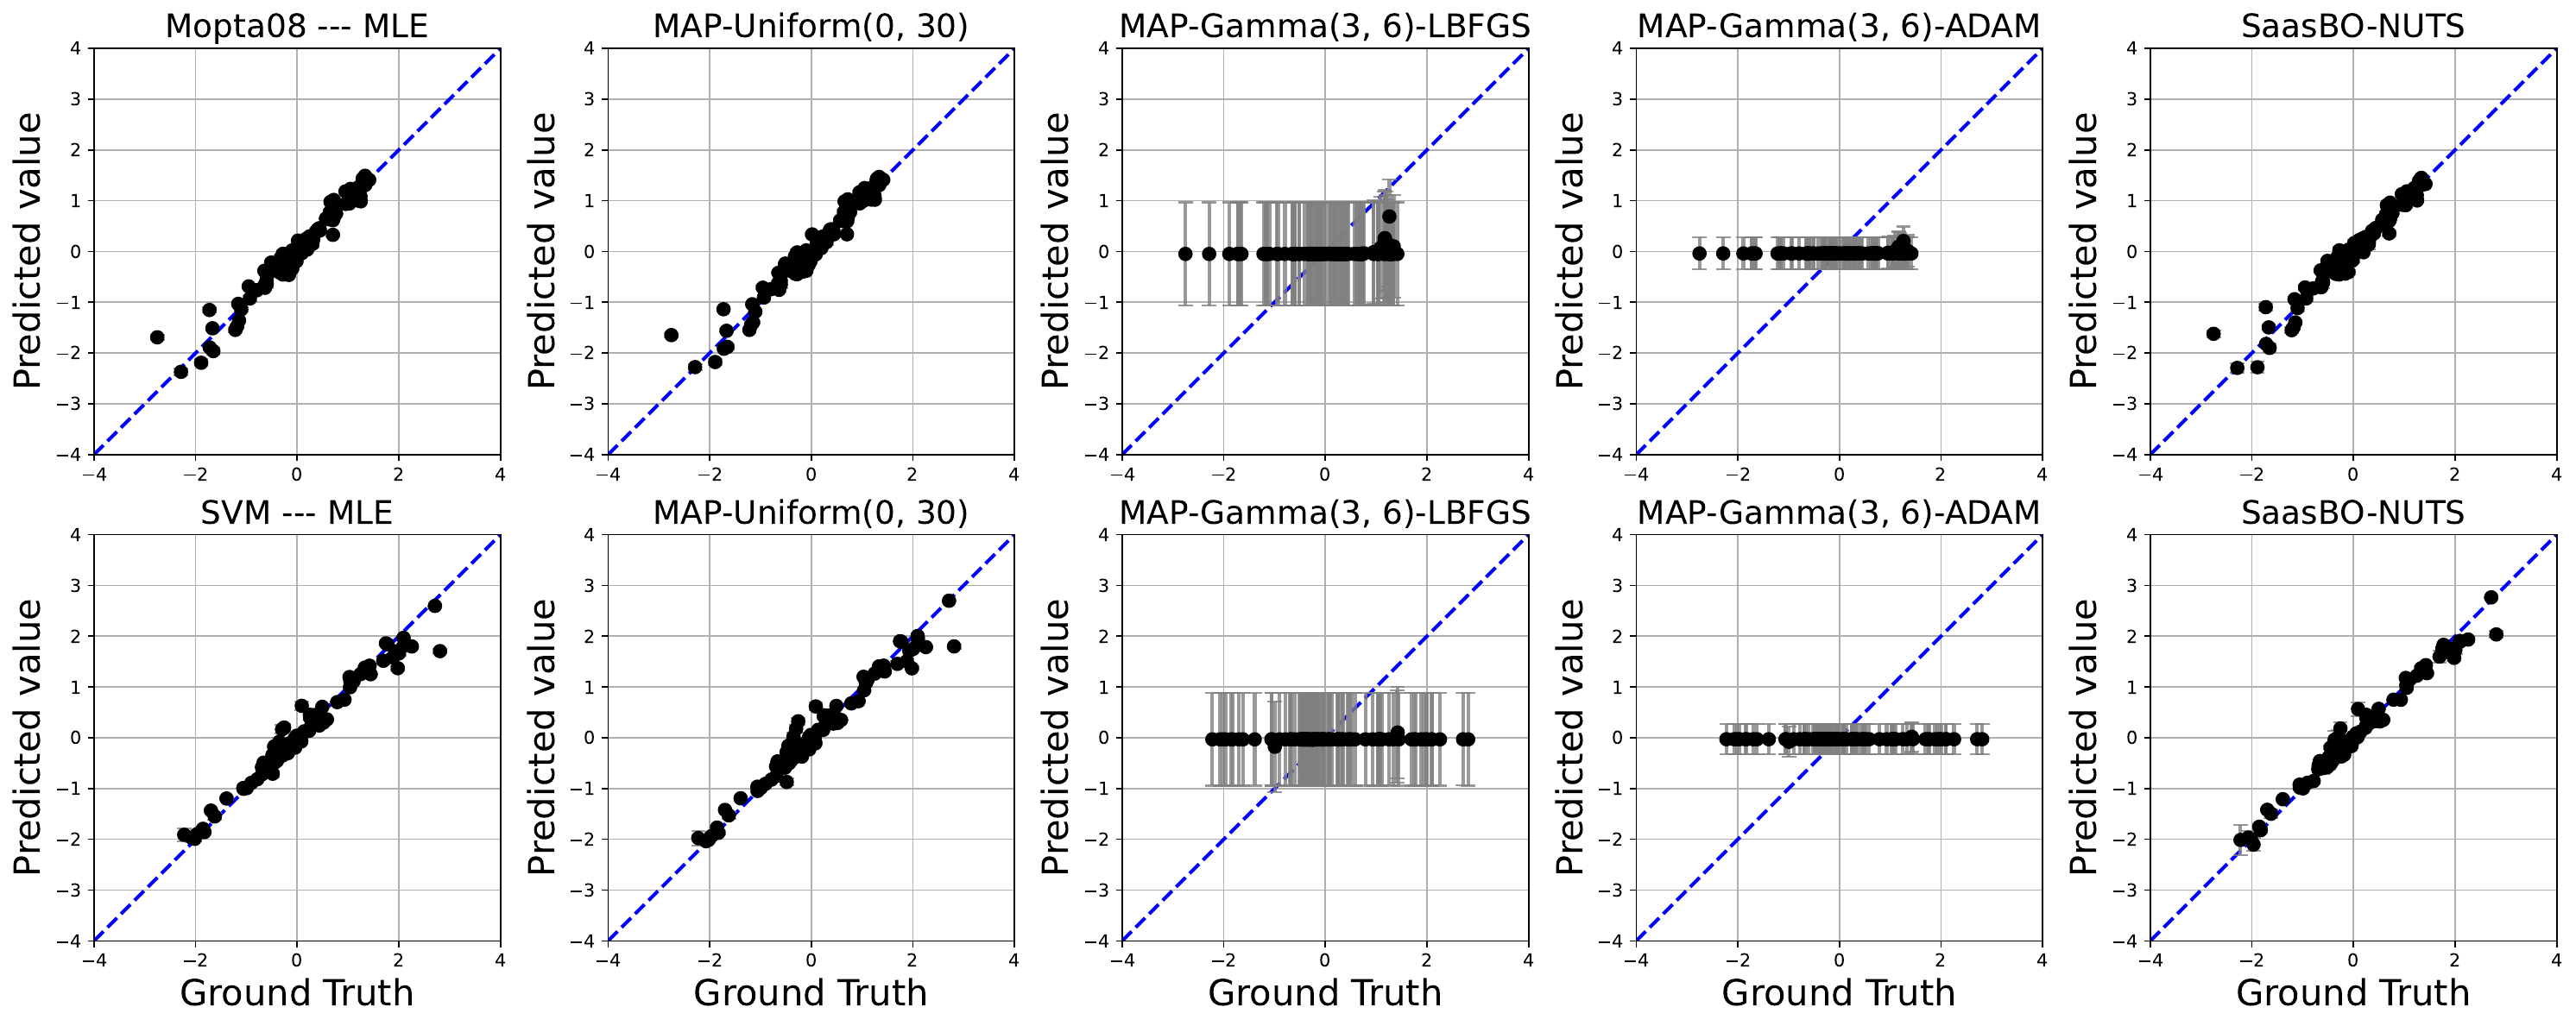}
    \caption{\small Alignment between the prediction (y-axis) and ground-truth function values (x-axis). \cmt{Reproducing GP surrogate performance in SaasBO. We used the same benchmark functions as Fig. 1 of SaasBO\cite{eriksson2021highdimensional}. The first row is Mopta08, which has 124 dimensions. The second row is SVM, which has 388 dimensions.}}
    \label{fig:alignment-more}
\end{figure*}

%Second, to examine if 500 epochs are sufficient for ADAM training, we tested with 1500 epochs and examined the optimization performance. \xuc{We didn't add this into plot, but would be fast to add that in Fig. \ref{fig:running-GP-training}, \ref{fig:final-GP-training}.}

\begin{table*}[h!]
\small
\centering
\begin{tabular}{lcccc}
\toprule
%{\textit{Task}} &   MLE &  MAP-Uniform(1E-3, 30) &  MAP-Gamma(3, 6)-LBFGS  &  MAP-Gamma(3, 6)-ADAM \\
\multirow{2}{*}{\textit{Task}} &   \multirow{2}{*}{MLE} &  \multirow{2}{*}{MAP-Uniform(1E-3, 30)} &  MAP-Gamma(3, 6)  &  MAP-Gamma(3, 6) \\
& & & LBFGS & ADAM\\
\midrule
{Mopta08(124)}      & \textbf{0.034}$\pm$0.006 & 0.035$\pm$0.005 & 0.837$\pm$0.112 & 0.856$\pm$0.114 \\
{Rover(60)}         & 0.327$\pm$0.078 & \textbf{0.323}$\pm$0.075 & 0.78$\pm$0.154 & 0.819$\pm$0.115 \\
{DNA(180)}          & \textbf{0.149}$\pm$0.038 & 0.166$\pm$0.049 & 1.014$\pm$0.097 & 1.026$\pm$0.101 \\
{SVM(388) }         & \textbf{0.034}$\pm$0.01 & 0.039$\pm$0.01 & 1.057$\pm$0.066 & 1.06$\pm$0.067 \\
{Ackley(150, 150)}  & \textbf{0.017}$\pm$0.008 & 0.026$\pm$0.007 & 0.019$\pm$0.004 & 0.019$\pm$0.005 \\
{Ackley(300, 150)}  & \textbf{0.023}$\pm$0.006 & 0.07$\pm$0.047 & 0.431$\pm$0.09 & 0.459$\pm$0.092 \\
{Hartmann6(300, 6)} & \textbf{0.017}$\pm$0.013 & 0.178$\pm$0.325 & 0.881$\pm$0.045 & 0.906$\pm$0.034 \\
{Rosenbrock(100, 100)} & 0.084$\pm$0.013 & \textbf{0.081}$\pm$0.012 & 0.9$\pm$0.156 & 0.925$\pm$0.172 \\
{Rosenbrock(300, 100)} & \textbf{0.09}$\pm$0.064 & 0.116$\pm$0.078 & 0.971$\pm$0.222 & 1.001$\pm$0.217 \\
{Stybtang(200, 200)} & \textbf{0.043}$\pm$0.018 & 0.054$\pm$0.024 & 0.698$\pm$0.05 & 0.732$\pm$0.034 \\
\bottomrule
\end{tabular}
\caption{Mean Squared Error(MSE) averaged from five runs. The best results are bolded.  \cmt{of GP surrogate model based on different training settings. The results were averaged over five runs. Top 1 best method is bolded. For MAP estimation, we place Uniform prior and Gamma prior over lengthscales. For Uniform prior, we set it as Uniform(1E-10, 30.0). For Gamma prior, we set it as Gamma(3.0, 6.0).}}
\label{tb:mse-surrogate-gamm36}
\end{table*}

\begin{table*}[h!]
\small
\centering
\begin{tabular}{lcccc}
\toprule
%{\textit{Task}} &   MLE &  MAP-Uniform(1E-3, 30) & MAP-Gamma(3, 6)-LBFGS  &  MAP-Gamma(3, 6)-ADAM \\
\multirow{2}{*}{\textit{Task}} &   \multirow{2}{*}{MLE} &  \multirow{2}{*}{MAP-Uniform(1E-3, 30)} &  MAP-Gamma(3, 6)  &  MAP-Gamma(3, 6) \\
& & & LBFGS & ADAM\\
\midrule
{Mopta08(124)}      & \textbf{0.57}$\pm$0.08 & 0.542$\pm$0.104 & -1.337$\pm$0.058 & -1.715$\pm$0.212 \\
{Rover(60)}         & \textbf{-0.975}$\pm$0.216 & -1.062$\pm$0.286 & -1.24$\pm$0.111 & -1.322$\pm$0.073 \\
{DNA(180)}          & \textbf{-0.256}$\pm$0.261 & -0.388$\pm$0.35 & -1.426$\pm$0.054 & -2.026$\pm$0.183 \\
{SVM(388) }         & \textbf{0.581}$\pm$0.119 & 0.504$\pm$0.128 & -1.453$\pm$0.038 & -2.095$\pm$0.129 \\
{Ackley(150, 150)}  & 0.428$\pm$0.222 & 0.14$\pm$0.218 & \textbf{0.451}$\pm$0.088 & 0.445$\pm$0.087 \\
{Ackley(300, 150)}  & \textbf{0.232}$\pm$0.155 & -0.257$\pm$0.528 & -1.006$\pm$0.091 & -1.037$\pm$0.087 \\
{Hartmann6(300, 6)} & \textbf{1.2}$\pm$0.169 & 0.67$\pm$0.867 & -1.344$\pm$0.029 & -1.618$\pm$0.128 \\
{Rosenbrock(100, 100)} & \textbf{0.64}$\pm$0.081 & 0.606$\pm$0.1 & -1.308$\pm$0.083 & -1.598$\pm$0.42 \\
{Rosenbrock(300, 100)} & \textbf{0.518}$\pm$0.225 & 0.347$\pm$0.325 & -1.411$\pm$0.134 & -1.967$\pm$0.413 \\
{Stybtang(200, 200)} & \textbf{0.574}$\pm$0.164 & 0.421$\pm$0.228 & -1.251$\pm$0.017 & -1.41$\pm$0.067 \\
\bottomrule
\end{tabular}
\caption{Test log likelihood averaged from five runs. The best results are bolded. \cmt{of GP surrogate model based on different training settings. The results were averaged over five runs. Top 1 best method is bolded. For MAP estimation, we place Uniform prior and Gamma prior over length-scales. For Uniform prior, we set it as Uniform(1E-10, 30.0). For Gamma prior, we set it as Gamma(3.0, 6.0).}}
\label{tb:test-ll-surrogate-gamma36}
\end{table*}

\begin{figure*}[!ht]
    \centering
    \includegraphics[width=\textwidth]{BO ICLR 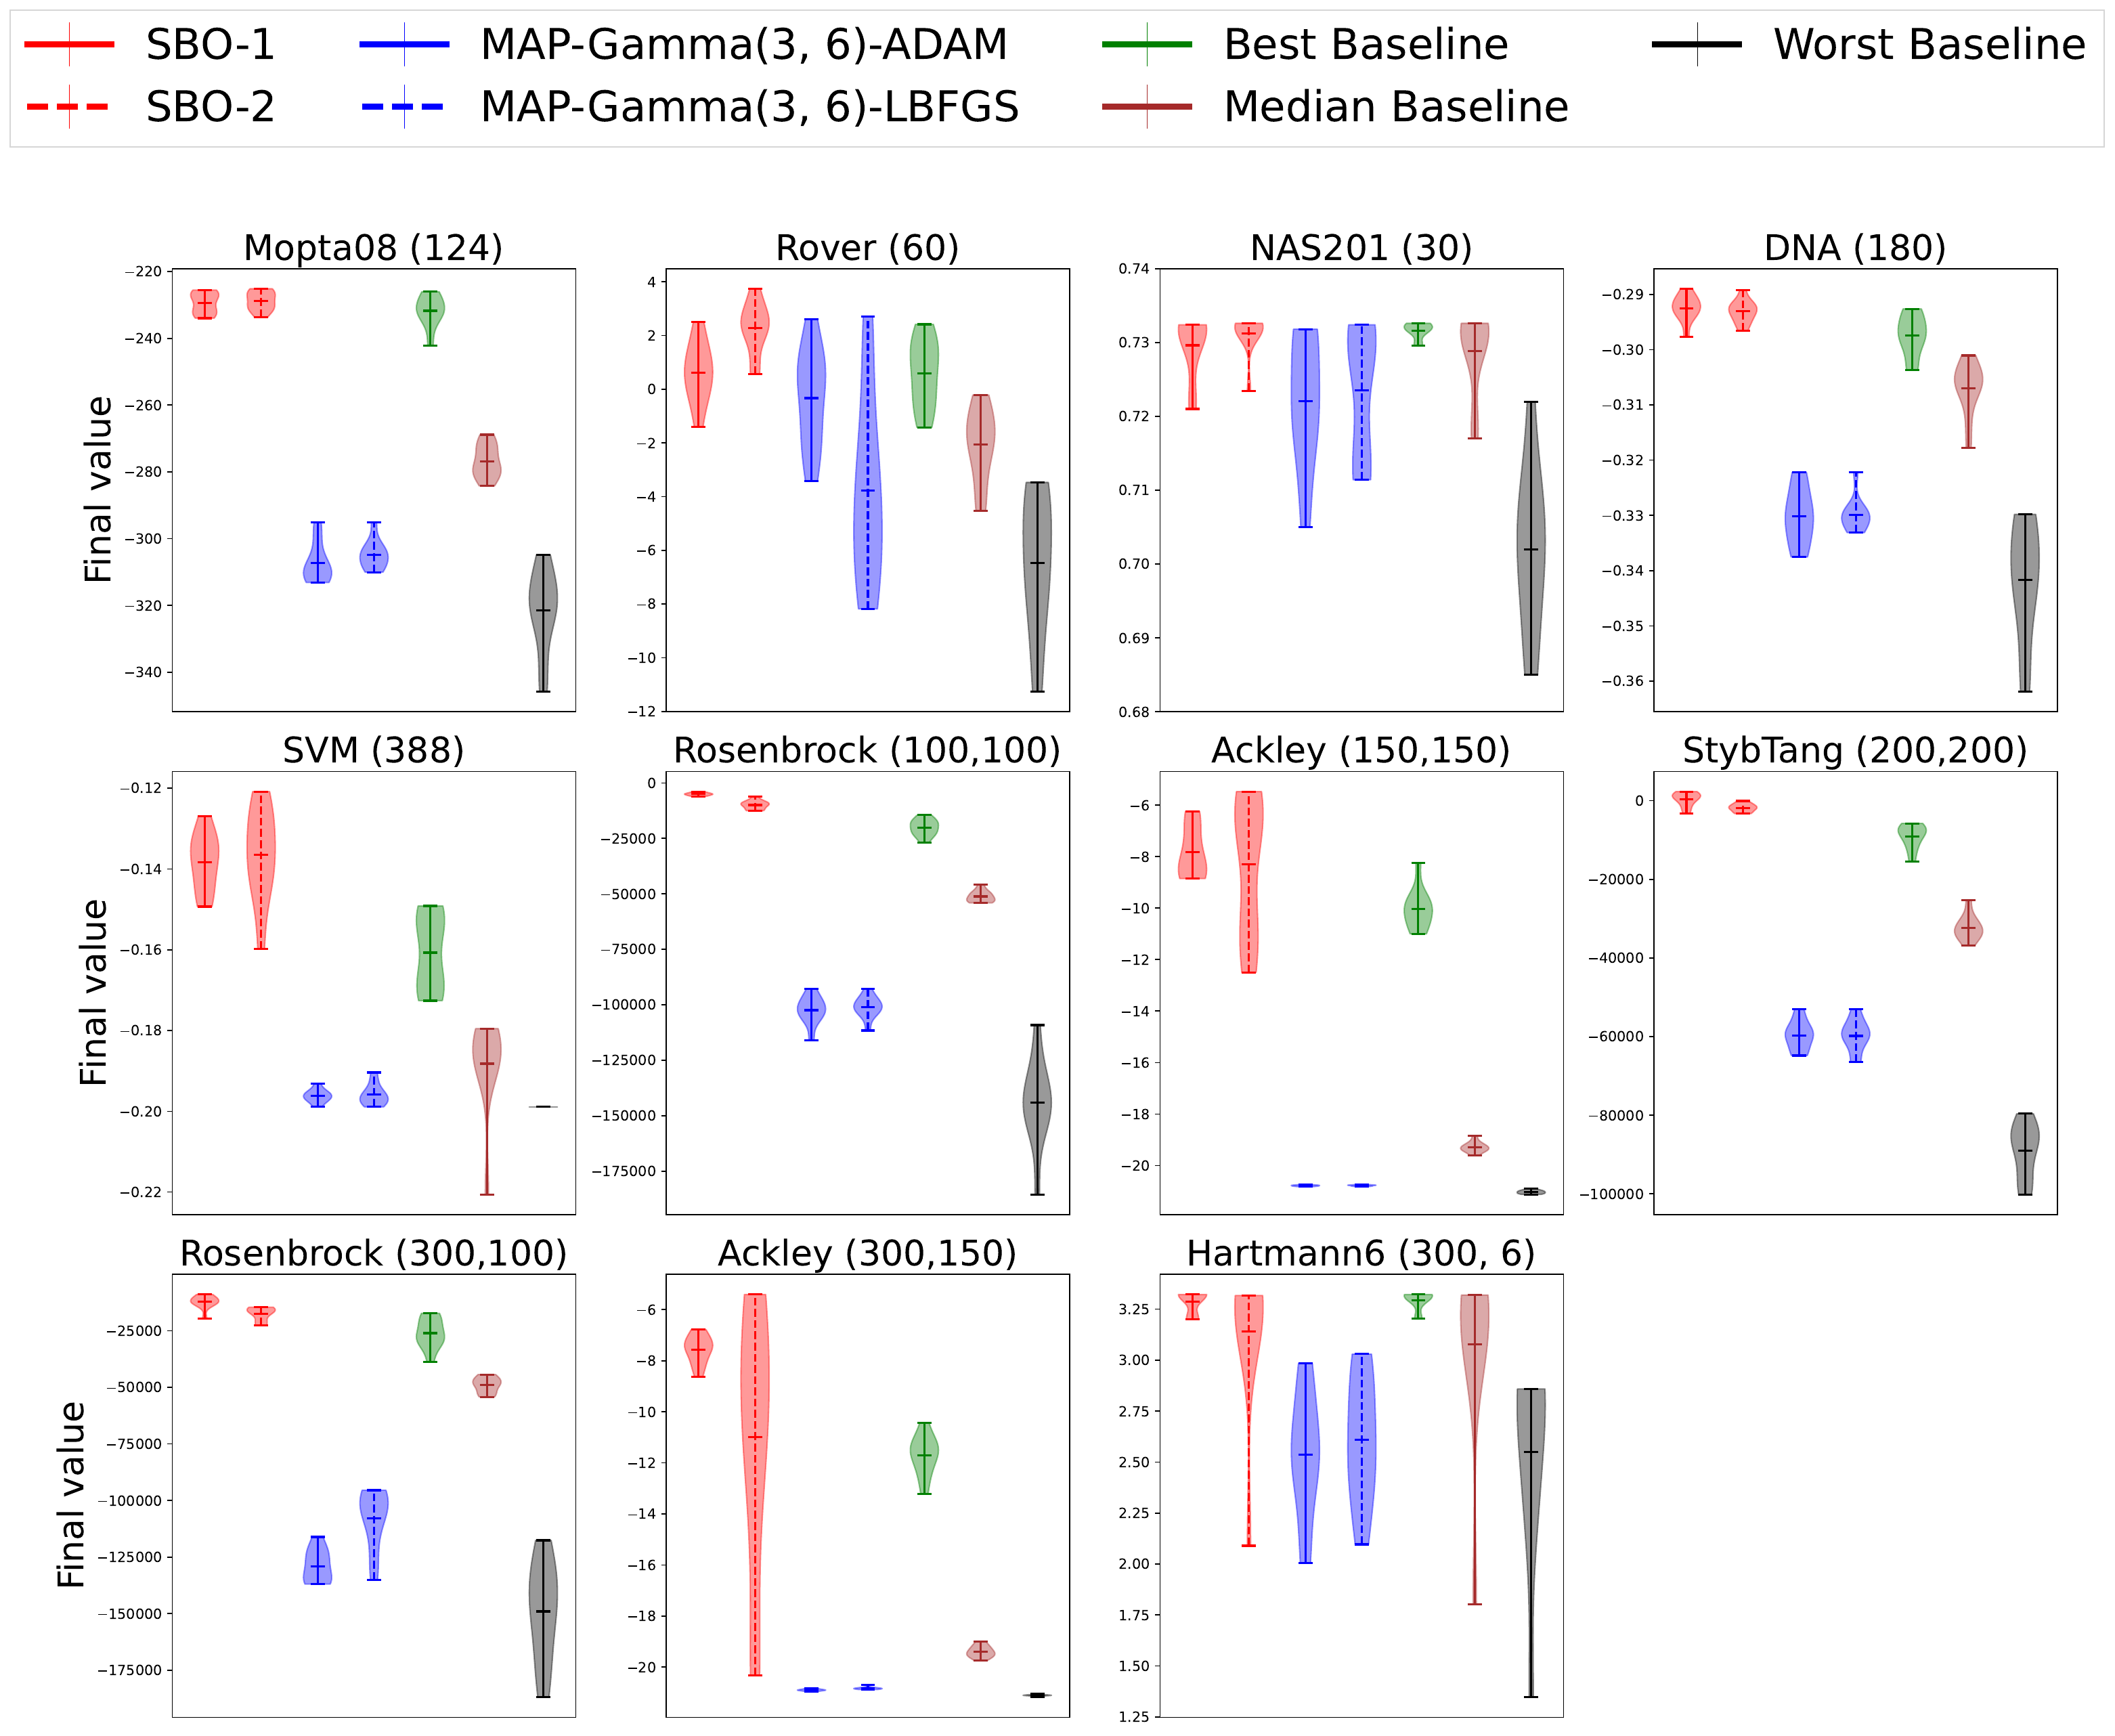}
    \caption{\small Ultimate optimization performance using a diffuse prior, Uniform(0.001, 30), \textit{vs.} a concentrated Gamma prior, Gamma(3,6),  over the length scale parameters. SBO-1 and SBO-2 use Uniform(0.001, 30). \cmt{Maximum Function Value Obtained at the end of optimization loop. The results were collect from 10 runs.}}
    \label{fig:final-Gamma36}
\end{figure*}

\begin{figure*}[!ht]
    \centering
    \includegraphics[width=\textwidth]{BO ICLR 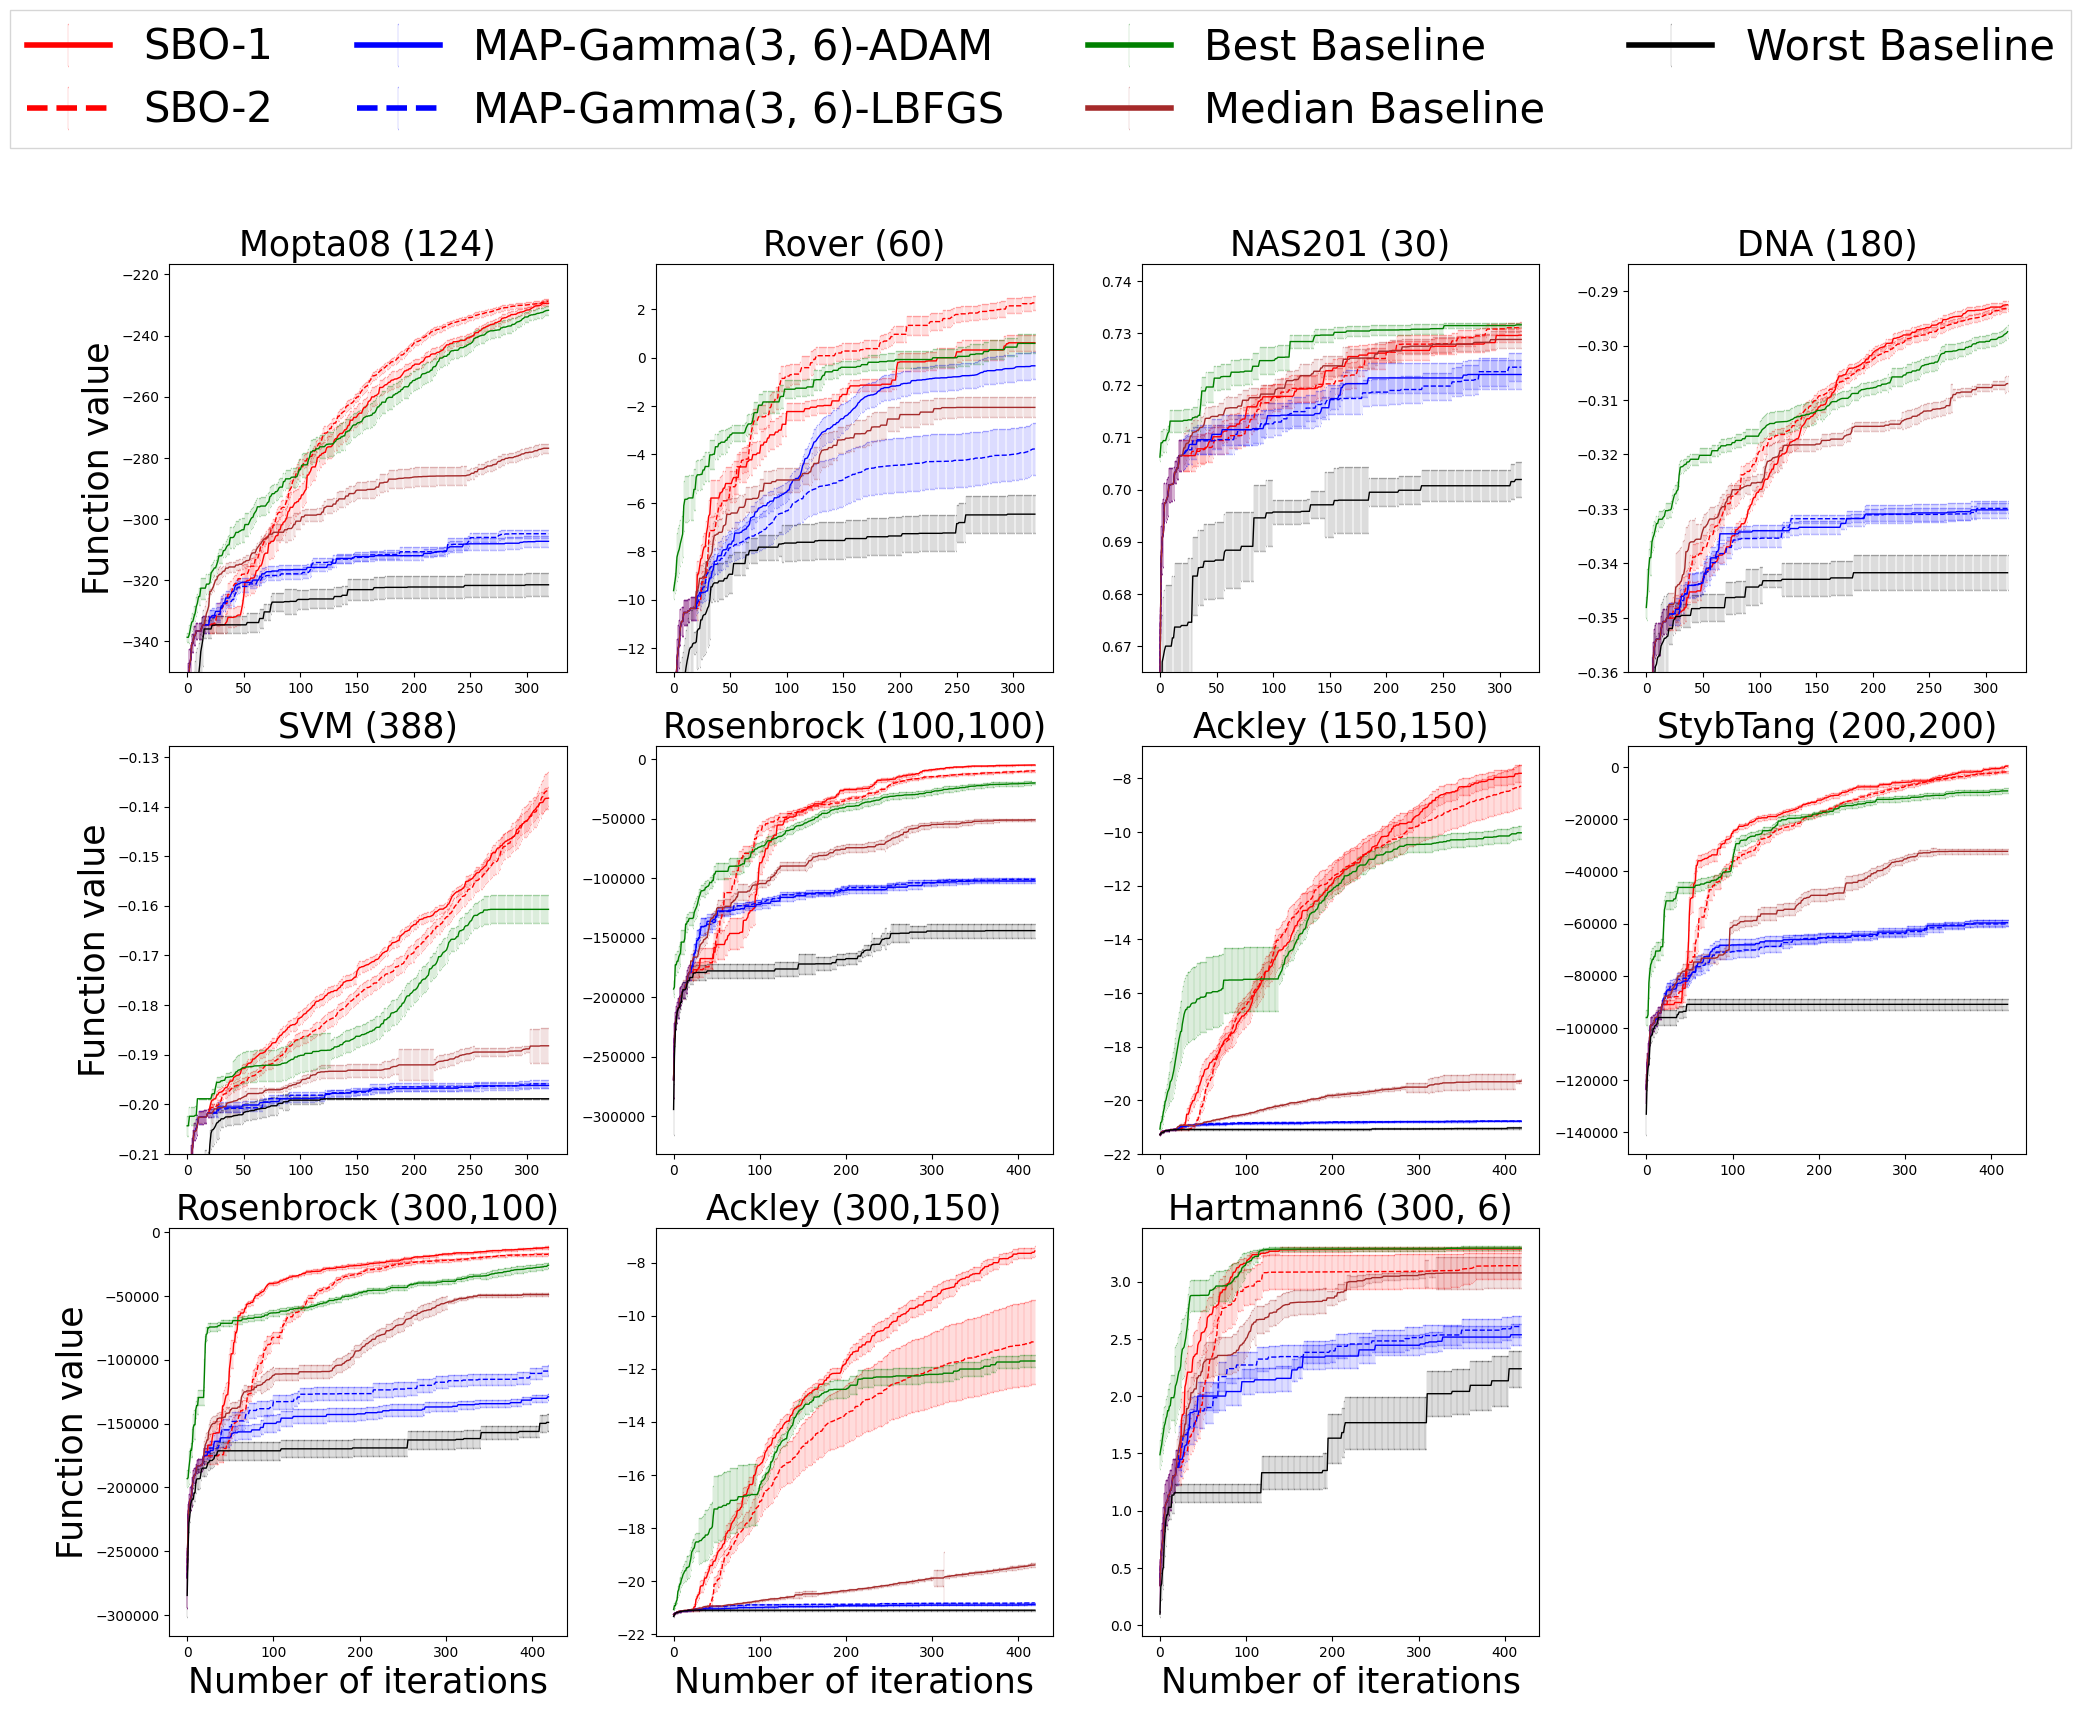}
    \caption{\small Runtime optimization performance using a diffuse prior, Uniform(0.001, 30), \textit{vs.} a concentrated Gamma prior, Gamma(3,6),  over the length scale parameters. SBO-1 and SBO-2 use Uniform(0.001, 30). \cmt{
    Maximum Function Value Obtained at the end of optimization loop. The results were collect from 10 runs.}}
    \label{fig:runtime-Gamma36}
\end{figure*}

\subsection{Alternative Acquisition Functions}
Next, we examined two other popular acquisition functions used in BO: Expected Improvement (EI) and Thompson sampling (TS). 
At each step, EI computes the expected improvement upon the best sample so far, 
\begin{align}
    \text{EI}(\x) = (\mu(\x) - f(\x^*) )\Psi\left(\frac{\mu(\x) - f(\x^*)}{\sqrt{v(\x)}}\right) + \sqrt{v(\x)}\Phi\left(\frac{\mu(\x)-f(\x^*)}{\sqrt{v(\x)}}\right),
\end{align}
where $\Psi(\cdot)$ and $\Phi(\cdot)$ are the CDF and PDF of the standard Gaussian distribution, $\x^*$ is the best sample that gives the largest function value among all the queries up to the current step, 
$\mu(\x)$ and $\sqrt{v(\x)}$ are the posterior mean and standard deviation of $f(\x)$ given current training data. We used BOTorch to maximize EI through L-BFGS. To conduct TS at each step, we used Sobol Sequence~\citep{sobol1967distribution} to sample 3K inputs in the domain, and jointly sampled the 3K function values from the GP posterior. We then selected the input with the largest function value as the next query. We denote this method by TS-3K. To explore more input candidates, we also employed the Lancos and conjugate gradient descent to approximate the posterior covariance matrix, and sampled 10K input candidates from Sobol Sequence. We denote this method as TS-10K. We used BOTorch implementation of both methods. We used ARD Mat\'ern kernel and MLE training at each step. 

The ultimate and runtime optimization performance for using EI, TS-3K and TS-10K, are shown in Fig. \ref{fig:final-acqf} and \ref{fig:running-acqf}, respectively. As we can see, in most cases, such as Mopta08 (128), SVM (388), DNA (180) and Rosenbrock (100, 100), both EI and TS perform worse than UCB, and also worse than the best baseline. On Ackley(150, 150) and Ackley(300, 150), the performance of EI and TS are even among the worst.
%\xuc{For all benchmarks besides Hartmann6, EI performed better than TS-3k and TS-10k. Interestingly, Thompson sampling performed rather well on Hartmann 6, which is better than UCB and EI with MLE training, but still inferior than UCB with MAP estimation and LBFGS as optimization.}

The limitation of EI might arise from the gradient vanishing during the optimization, as pointed by the recent work~\citep{ament2024unexpected}. A remedy is to use log-EI as the acquisition function. The failure of the TS might be due to the high-dimension of the input space. A few thousand  candidates might not be sufficient to cover the whole space; as a result, the selected queries are inferior in indicating  the best direction to optimize the target function. %\xuc{Also, unlike EI and UCB, the scale of exploration for Thompson sampling depends purely on the quantity of random point generator.}
\begin{figure*}[!ht]
    \centering
    \includegraphics[width=\textwidth]{BO ICLR 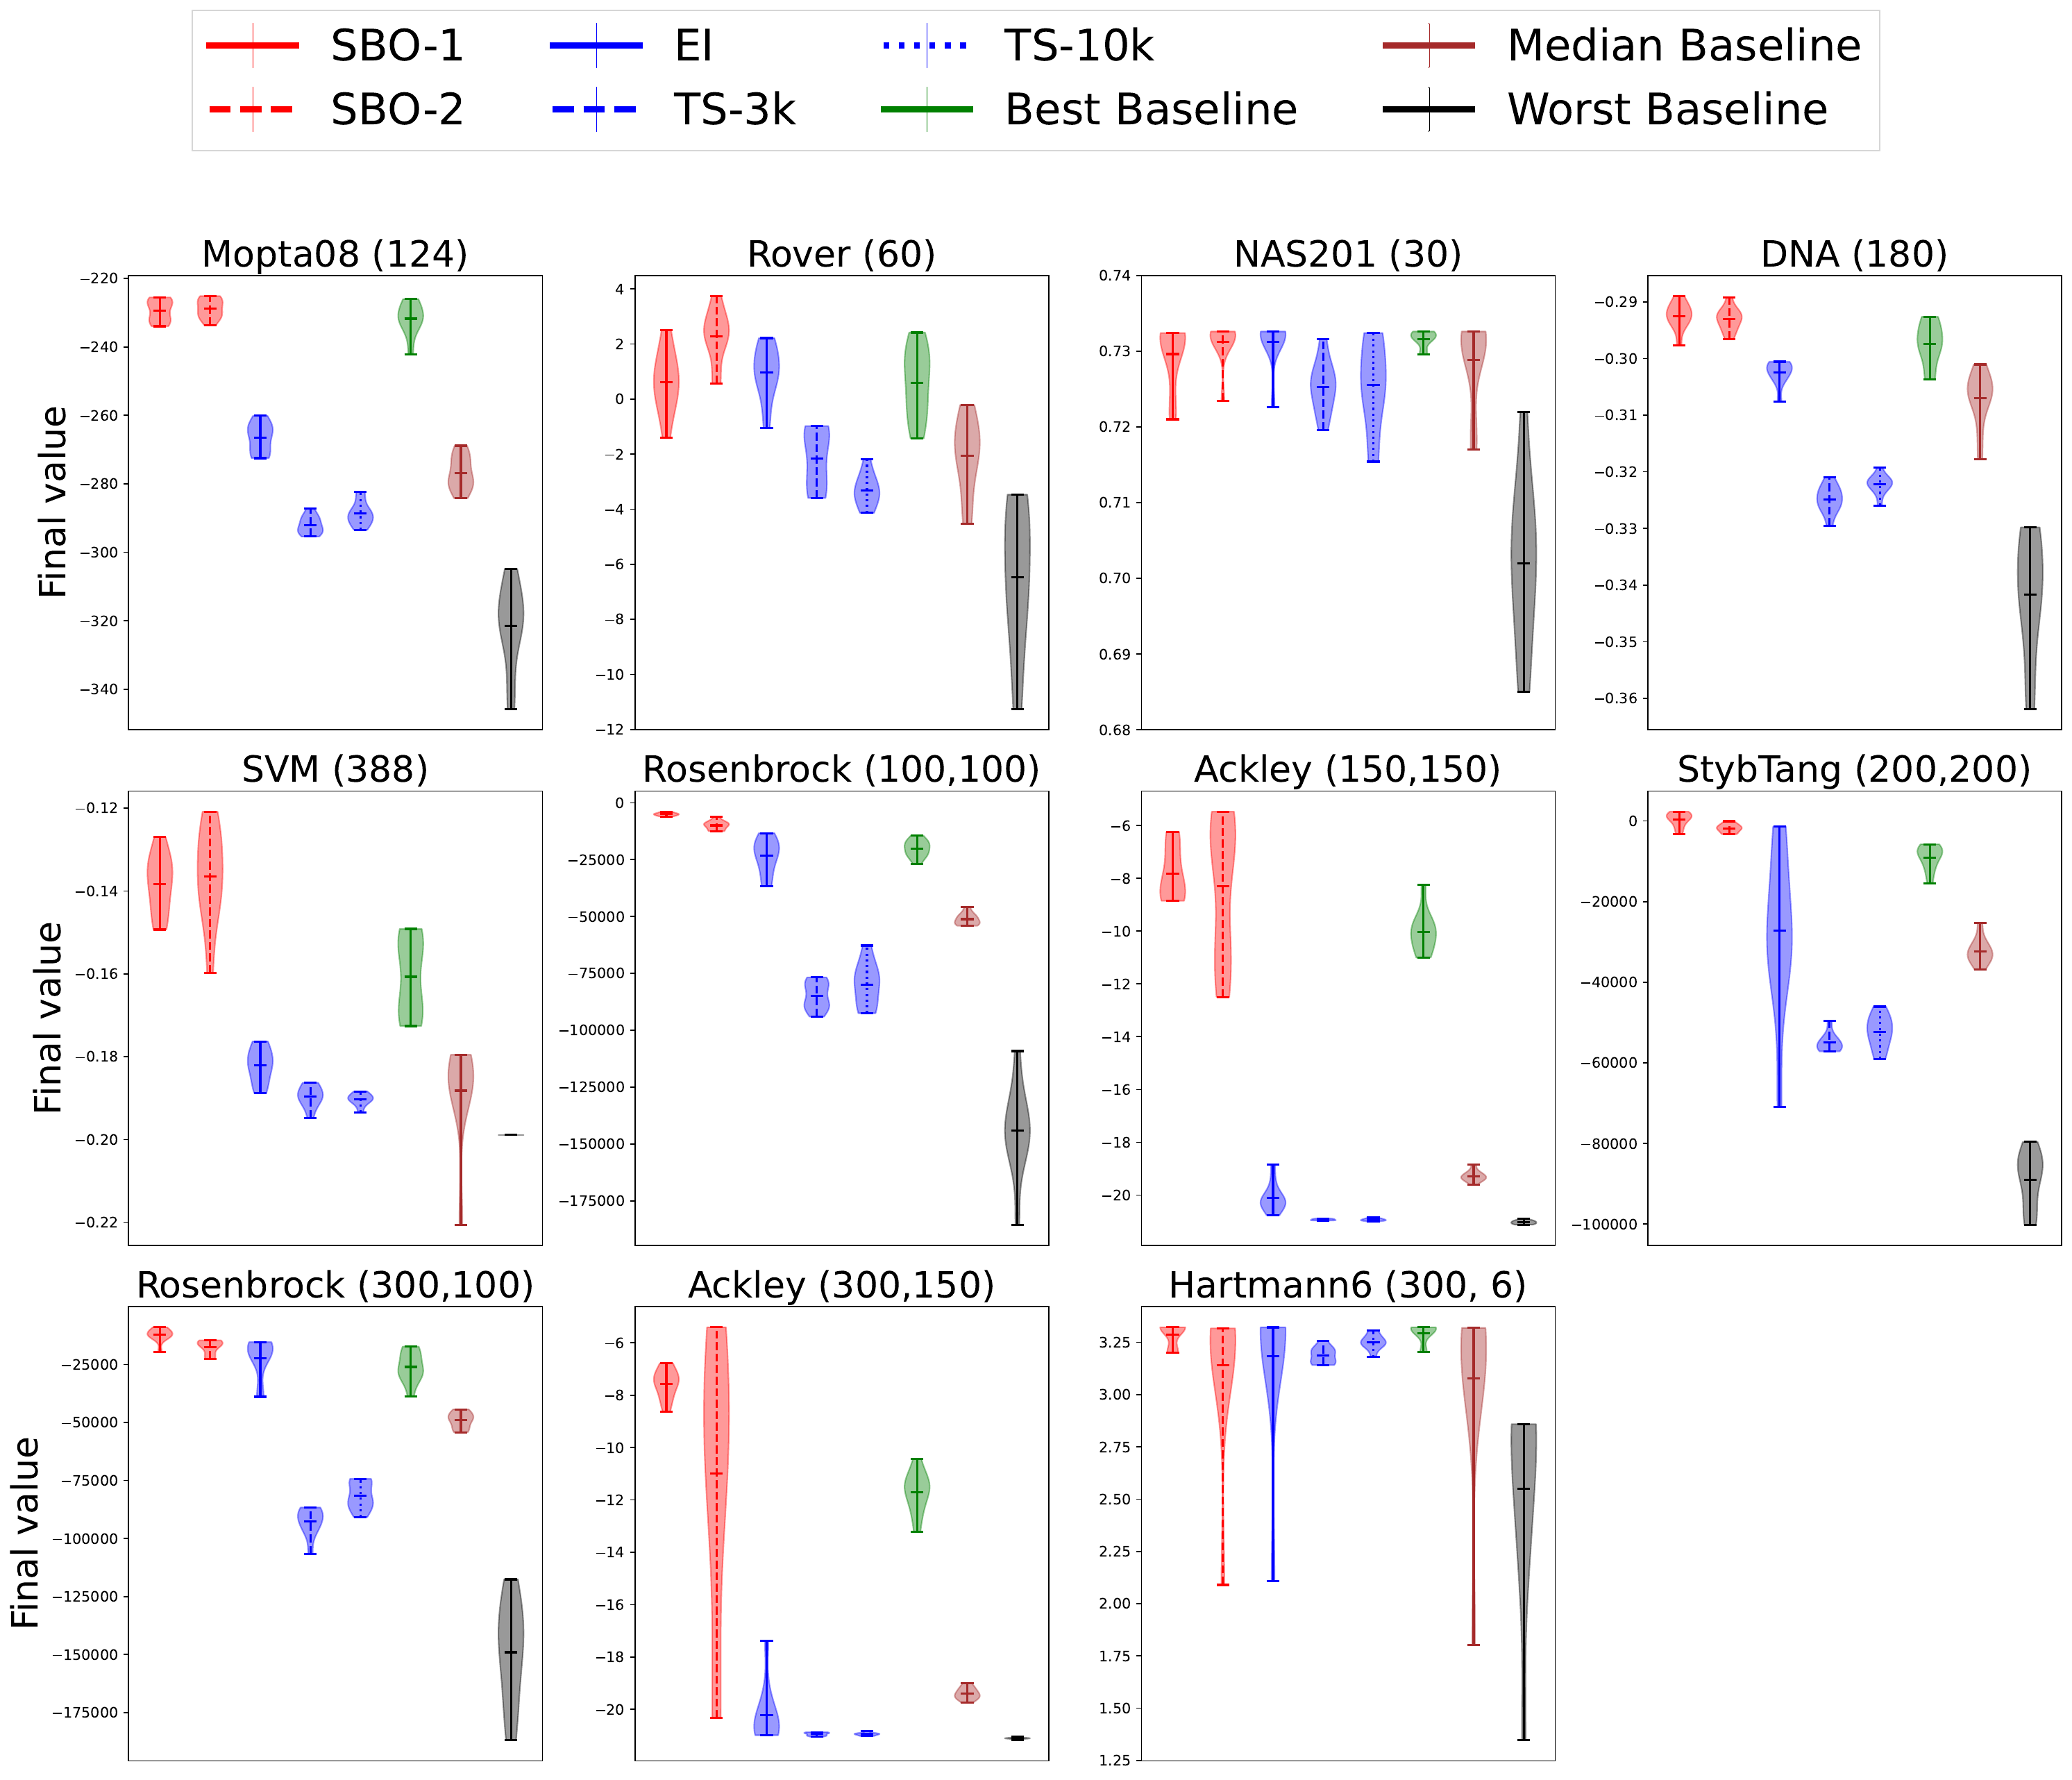}
    \caption{\small Ultimate performance with different acquisition functions. Note that SBO-1 and SBO-2 use UCB. \cmt{Maximum Function Value Obtained at the end of optimization loop. The results were collect from 10 runs.}}
    \label{fig:final-acqf}
\end{figure*}
\begin{figure*}[!ht]
    \centering
    \includegraphics[width=\textwidth]{BO ICLR 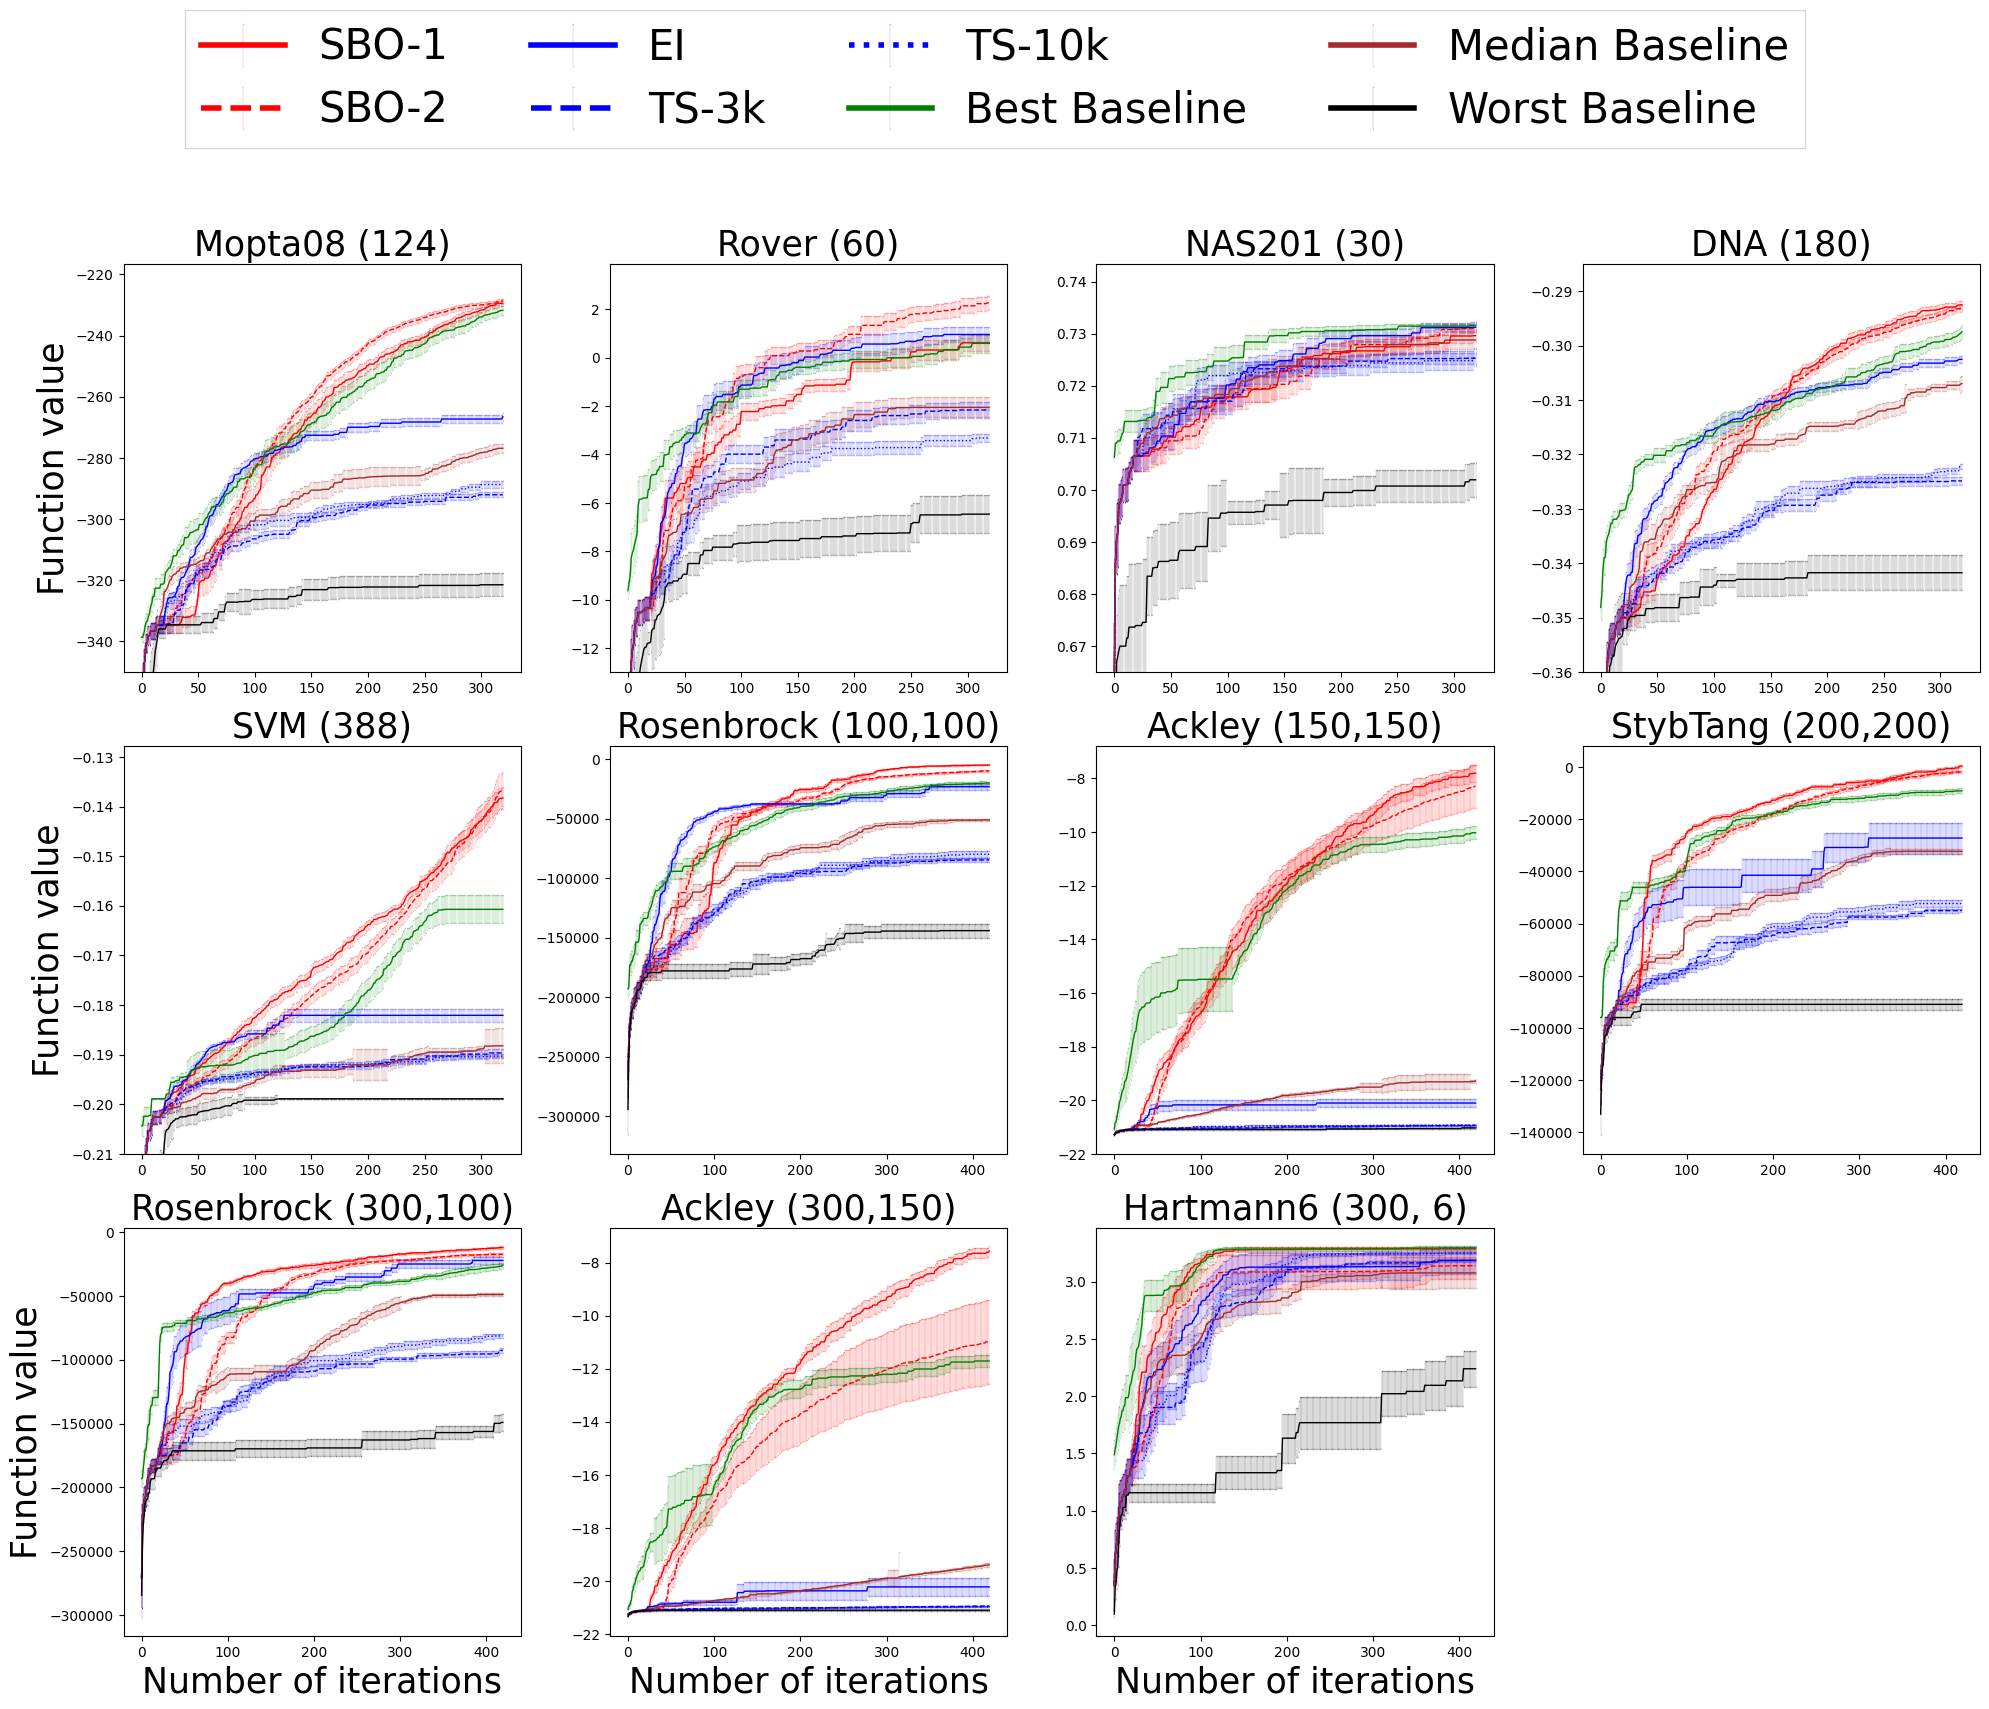}
    \caption{\small Runtime performance with different acquisition functions. Note that SBO-1 and SBO-2 use UCB. \cmt{Maximum Function Value Obtained at the end of optimization loop. The results were collect from 10 runs.}}
    \label{fig:running-acqf}
\end{figure*}



\subsection{Using Square Exponential (SE) kernels}
Third, we considered another widely used kernel in BO, namely, the SE kernel. We tested with ARD SE and SE kernel using a single length-scale parameter. We used MLE training and UCB $(\lambda=1.5)$ to run BO. As depicted in Fig. \ref{fig:final-SE} and \ref{fig:running-SE}, with smaller optimization dimensions, such as Mopta08 (124), NAS201 (3) and DNA (180), the performance of SE is among the best. However, with higher dimensions, \eg above 200, the performance of SE drops substantially, such as in SVM (388) and Ackley(300, 150). 

%although in several benchmarks(Mopta08, NAS201), SE also achieves the best performance, in other benchmarks \xuc{that are above 200 dimensions, it's performance starts to degenerate quickly. For the function(SVM) with the highest dimension that we tested, SE kernel performance is even similar to the worst baselines.}

We argue that the inferior performance might be due to that the vanilla SE kernel is not powerful enough to enable GP to well capture high-dimensional functions. %We observe that the value of the SE kernel is only determined by the square of the distance  C
Consider a single length-scale parameter. 
we observe that the value of the SE kernel is determined by the squared distance between the inputs, 
\begin{align}
  \kappa_{\text{SE}}(\x, \x') = a\exp\left(-\eta \|\x-\x'\|^2\right).
\end{align}
With the growth of the input dimension $d$, the kernel function value decays much faster than the increase of the distance: a squared decay coupling with the exponential decay. The learning can be easily driven to adapt to a sparse, diagonal-dominant covariance matrix, which roughly treats each data point as independent. This can make the learning fail to capture the correlation between function values, and result in inferior learning performance. By contrast, the value of the Mat\'ern kernel (see \eqref{eq:matern}) is dominated by the distance rather than the squared distance. Therefore, with the growth of the distance, the kernel function value decays much slower than the SE kernel. It is easier for the optimization to adjust the length-scale parameter so as to avoid ``diagonal-like'' covariance matrices. Consequently, the correlation between function values can be better captured in the high dimensional input space. 

To verify our argument, we examined the GP learning performance with ARD SE kernel and ARD Mat\'ern kernel. We used Rosenbrock(d,d) and Hartmann6(d, 6) as test cases. The former is a ``full-rank'' function, namely, all the $d$ input variables are relevant to the function value. The latter has a ``low-rank'' structure in that only the first 6 variables out of the $d$ input variables determines the function value.  For each test case, we increased the input dimension from 50 to 300. We randomly generated 500 training examples and 100 test examples. We then trained each method with MLE, and examined the mean square error (MSE) and the test log likelihood. We repeated the training and test procedure for five times, and report the average MSE, average test log likelihood, and the standard deviations in Fig. \ref{fig:func-learn-SE}. 

As we can see, in both test cases, when the input dimension $d$ does not exceed 150, the performance of using SE and Mat\'ern-5/2 is close, in terms of both MSE and log likelihood. The two curves almost overlap.  However, for $d>150$ in both test scenarios, the MSE significantly escalates when employing the SE kernel, accompanied by a substantial decrease in the test log likelihood. These observations suggest a failure of the SE kernel in effectively learning the target function. 
In comparison, employing the Mat\'ern kernel maintains a consistently favorable prediction performance even when $d>150$. On the Rosenbrock dataset, the MSE gradually increases while the test log likelihood decreases, following a roughly linear trend. This outcome is expected as, with the rise in input dimension $d$, more training examples are necessary to sustain comparable performance. Furthermore, on the Hartmann6 dataset, little variation is observed in both MSE and test log likelihood with increasing the input dimension when using the Mat\'ern kernel. This suggests that the GP has effectively discerned the pertinent input variables and mitigated the influence of irrelevant ones. In summary, these results collectively underscore the advantage of employing Mat\'ern kernels for learning high-dimensional functions. It is worth noting that the most recent work~\citep{hvarfner2024vanilla} designs a log-normal prior over each length-scale parameter to overcome the learning issue with the ARD SE kernel. 






%As a comparison, the prediction performance of using Mat\'ern kernel maintains a reasonably well level when $d>150$. On Robsenbrock, the MSE gradually increases while the test log likelihood gradually decreases (roughly in a linear fasion). This is reasonable, because with the increase of input dimension $d$, more training examples are expected to maintain the same performance. In addition, it is interesting to see that on Hartmann6, the MSE and test log likelihood of using Mat\'ern kernel varied little along with the increase of the input dimension. It  implied that the GP has identified the underlying relevant input variables, and removed the influence of irrelevant variables. Overall, the results together have demonstrated the advantage of using Mat\'ern kernels for high-dimensional function learning. 


\begin{figure*}[t]
    \centering
    \includegraphics[width=0.8\textwidth]{BO ICLR 2025/figs/ablation/Mater vs RBF.pdf}
    \caption{\small Learning high-dimension functions with different kernels. We trained on 500 points, and tested on 100 points. Results shown with mean and standard deviation over 5 runs.}
    \label{fig:func-learn-SE}
\end{figure*}
\begin{figure*}[!ht]
    \centering
    \includegraphics[width=\textwidth]{BO ICLR 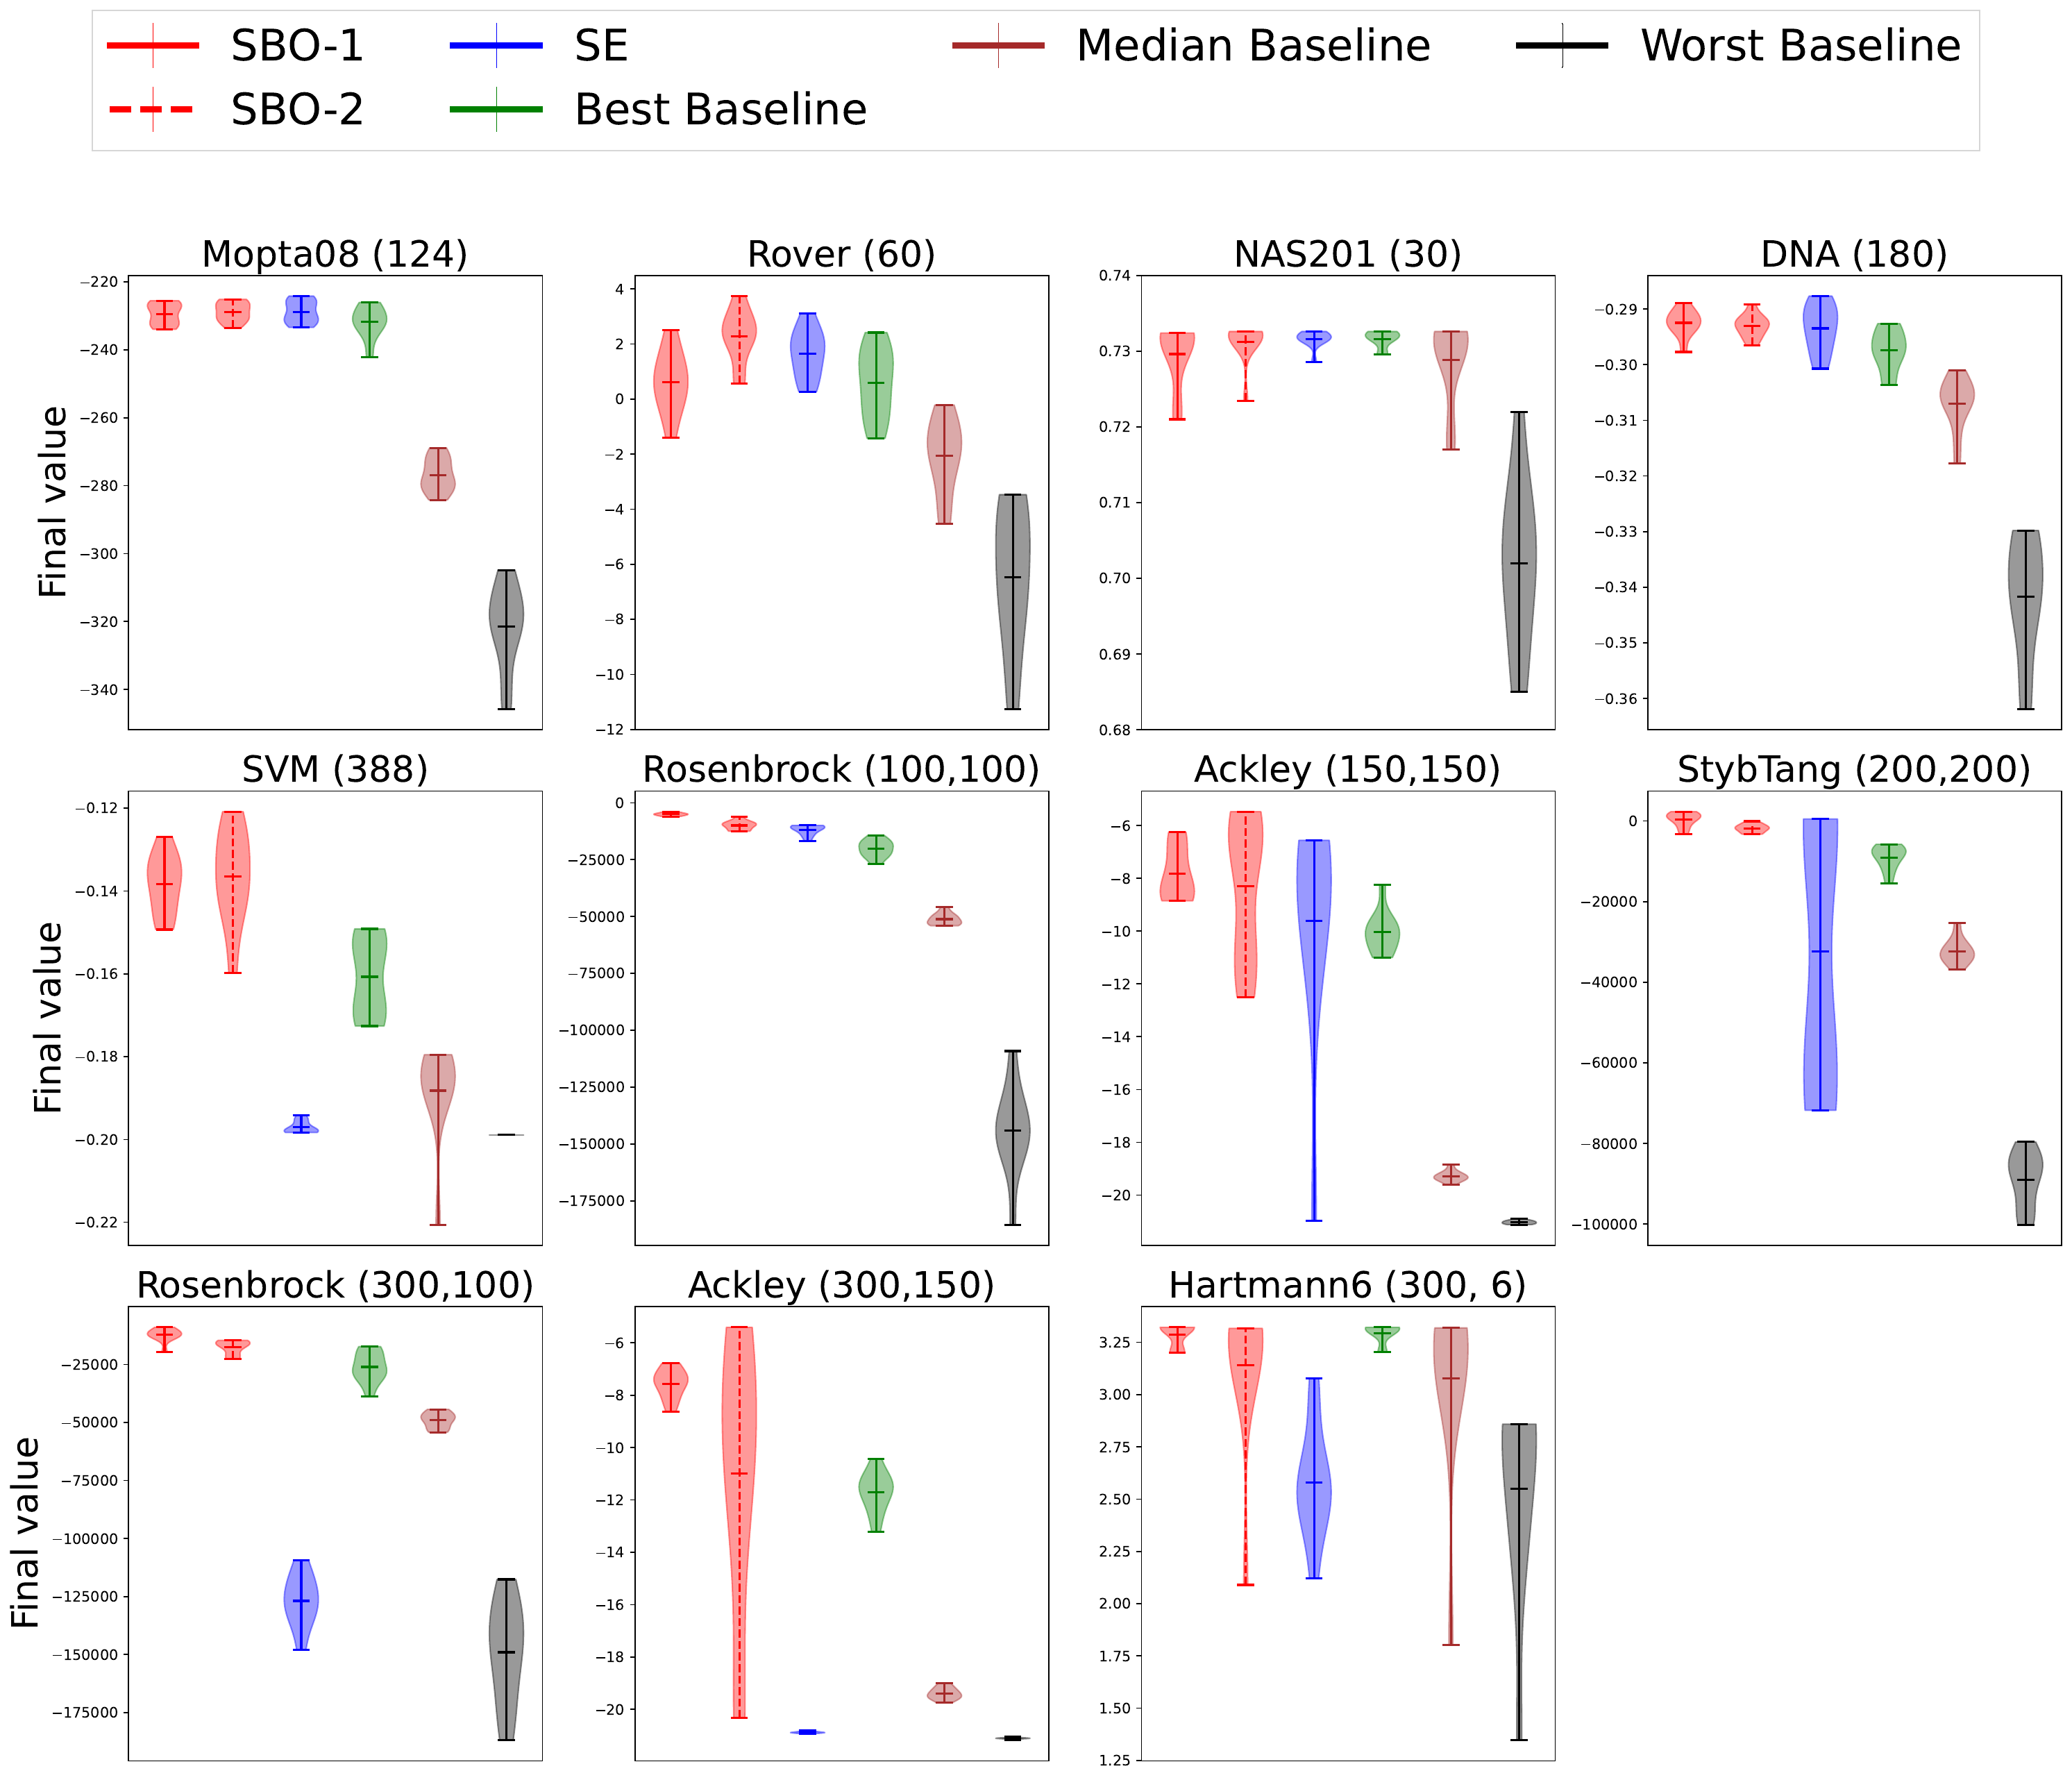}
    \caption{\small Ultimate optimization performance with different kernels. Note that SBO-1 and SBO-2 use Mat\'ern-5/2 kernel.
    \cmt{Maximum Function Value Obtained at the end of optimization loop. The results were collect from 10 runs.}}
    \label{fig:final-SE}
\end{figure*}
\begin{figure*}[!ht]
    \centering
    \includegraphics[width=\textwidth]{BO ICLR 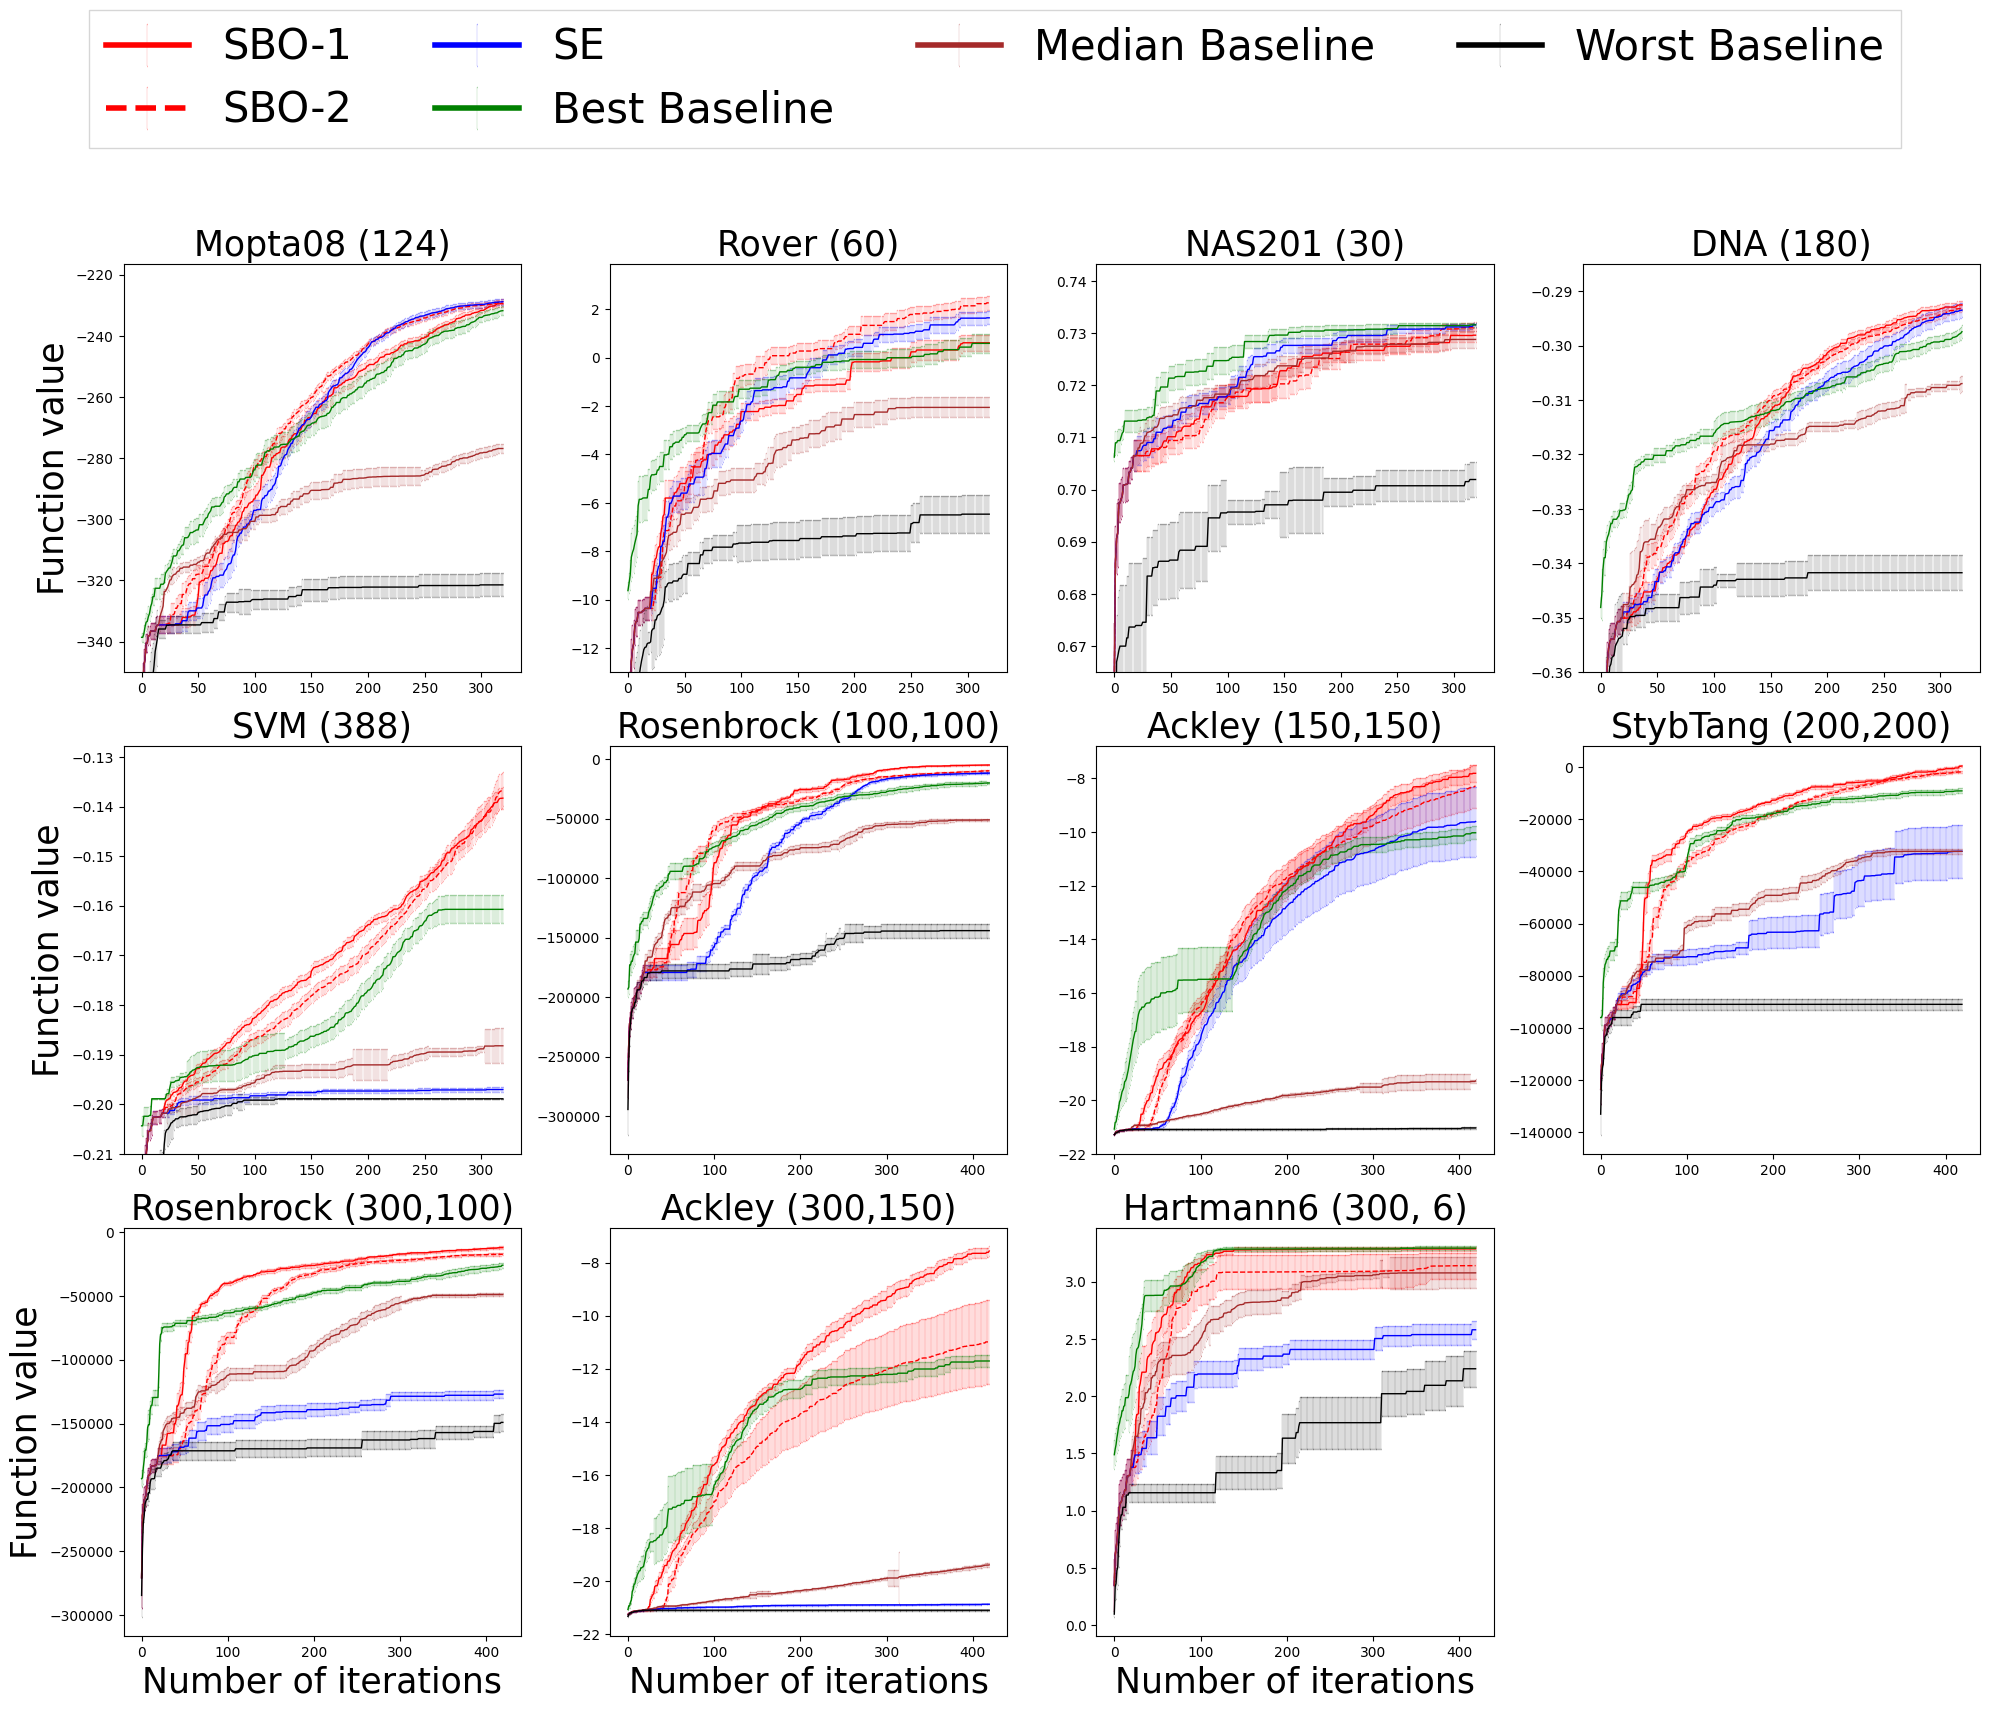}
    \caption{\small Runtime optimization performance with different kernels. Note that SBO-1 and SBO-2 use Mat\'ern-5/2 kernel. \cmt{Maximum Function Value Obtained at the end of optimization loop. The results were collect from 10 runs.}}
    \label{fig:running-SE}
\end{figure*}




\subsection{Different Choice of $\lambda$ in UCB}\label{sect:lam-choice}
%\xuc{I moved previous ablation section(sec B) to here.}

Finally, we examined how the exploration parameter $\lambda$ in UCB (see \eqref{eq:ucb}) influences the performance in high-dimensional optimization. To this end, we used ARD Ma\'ern kernel and varied $\lambda$ from \{0.5, 1.0, 1.5, 2.0\}. We conducted MLE training via ADAM optimization. %We conducted MLE for GP training at each step. 
We show the ultimate and runtime optimization performance in Fig. \ref{fig:final-lambda} and \ref{fig:running-lambda}, respectively. 
It can be seen that, in most benchmarks (Mopta08, Rover, NAS201, DNA, \etc), the performance with different $\lambda$'s is close. However, on DNA, SVM and Ackley, the performance of $\lambda=0.5$ is typically worse than the bigger choice of $\lambda$. This might be due to that those problems are more challenging (\eg Ackley has many local minima), a larger exploration level ($\lambda$) is needed to identify better optimization outcomes. 

%\xuc{As we can see, for majority benchmark functions(Mopta08, Rover, DNA, SVM, Rosenbrock(100, 100), StybTang), GP-ARD with MLE training achieved better BO performance than the best SOTA HDBO method. And there is a clear gap between $\lambda$=0.5 and other choice of $\lambda$ on DNA, SVM, Ackley, Rosenbrock(300, 100), where the performance of $\lambda$=0.5 being significantly inferior. For functions(Ackley) that are known with local optimal, we can see that a larger $\lambda$ will yield better BO performance.}

\begin{figure*}[!ht]
    \centering
    \includegraphics[width=\textwidth]{BO ICLR 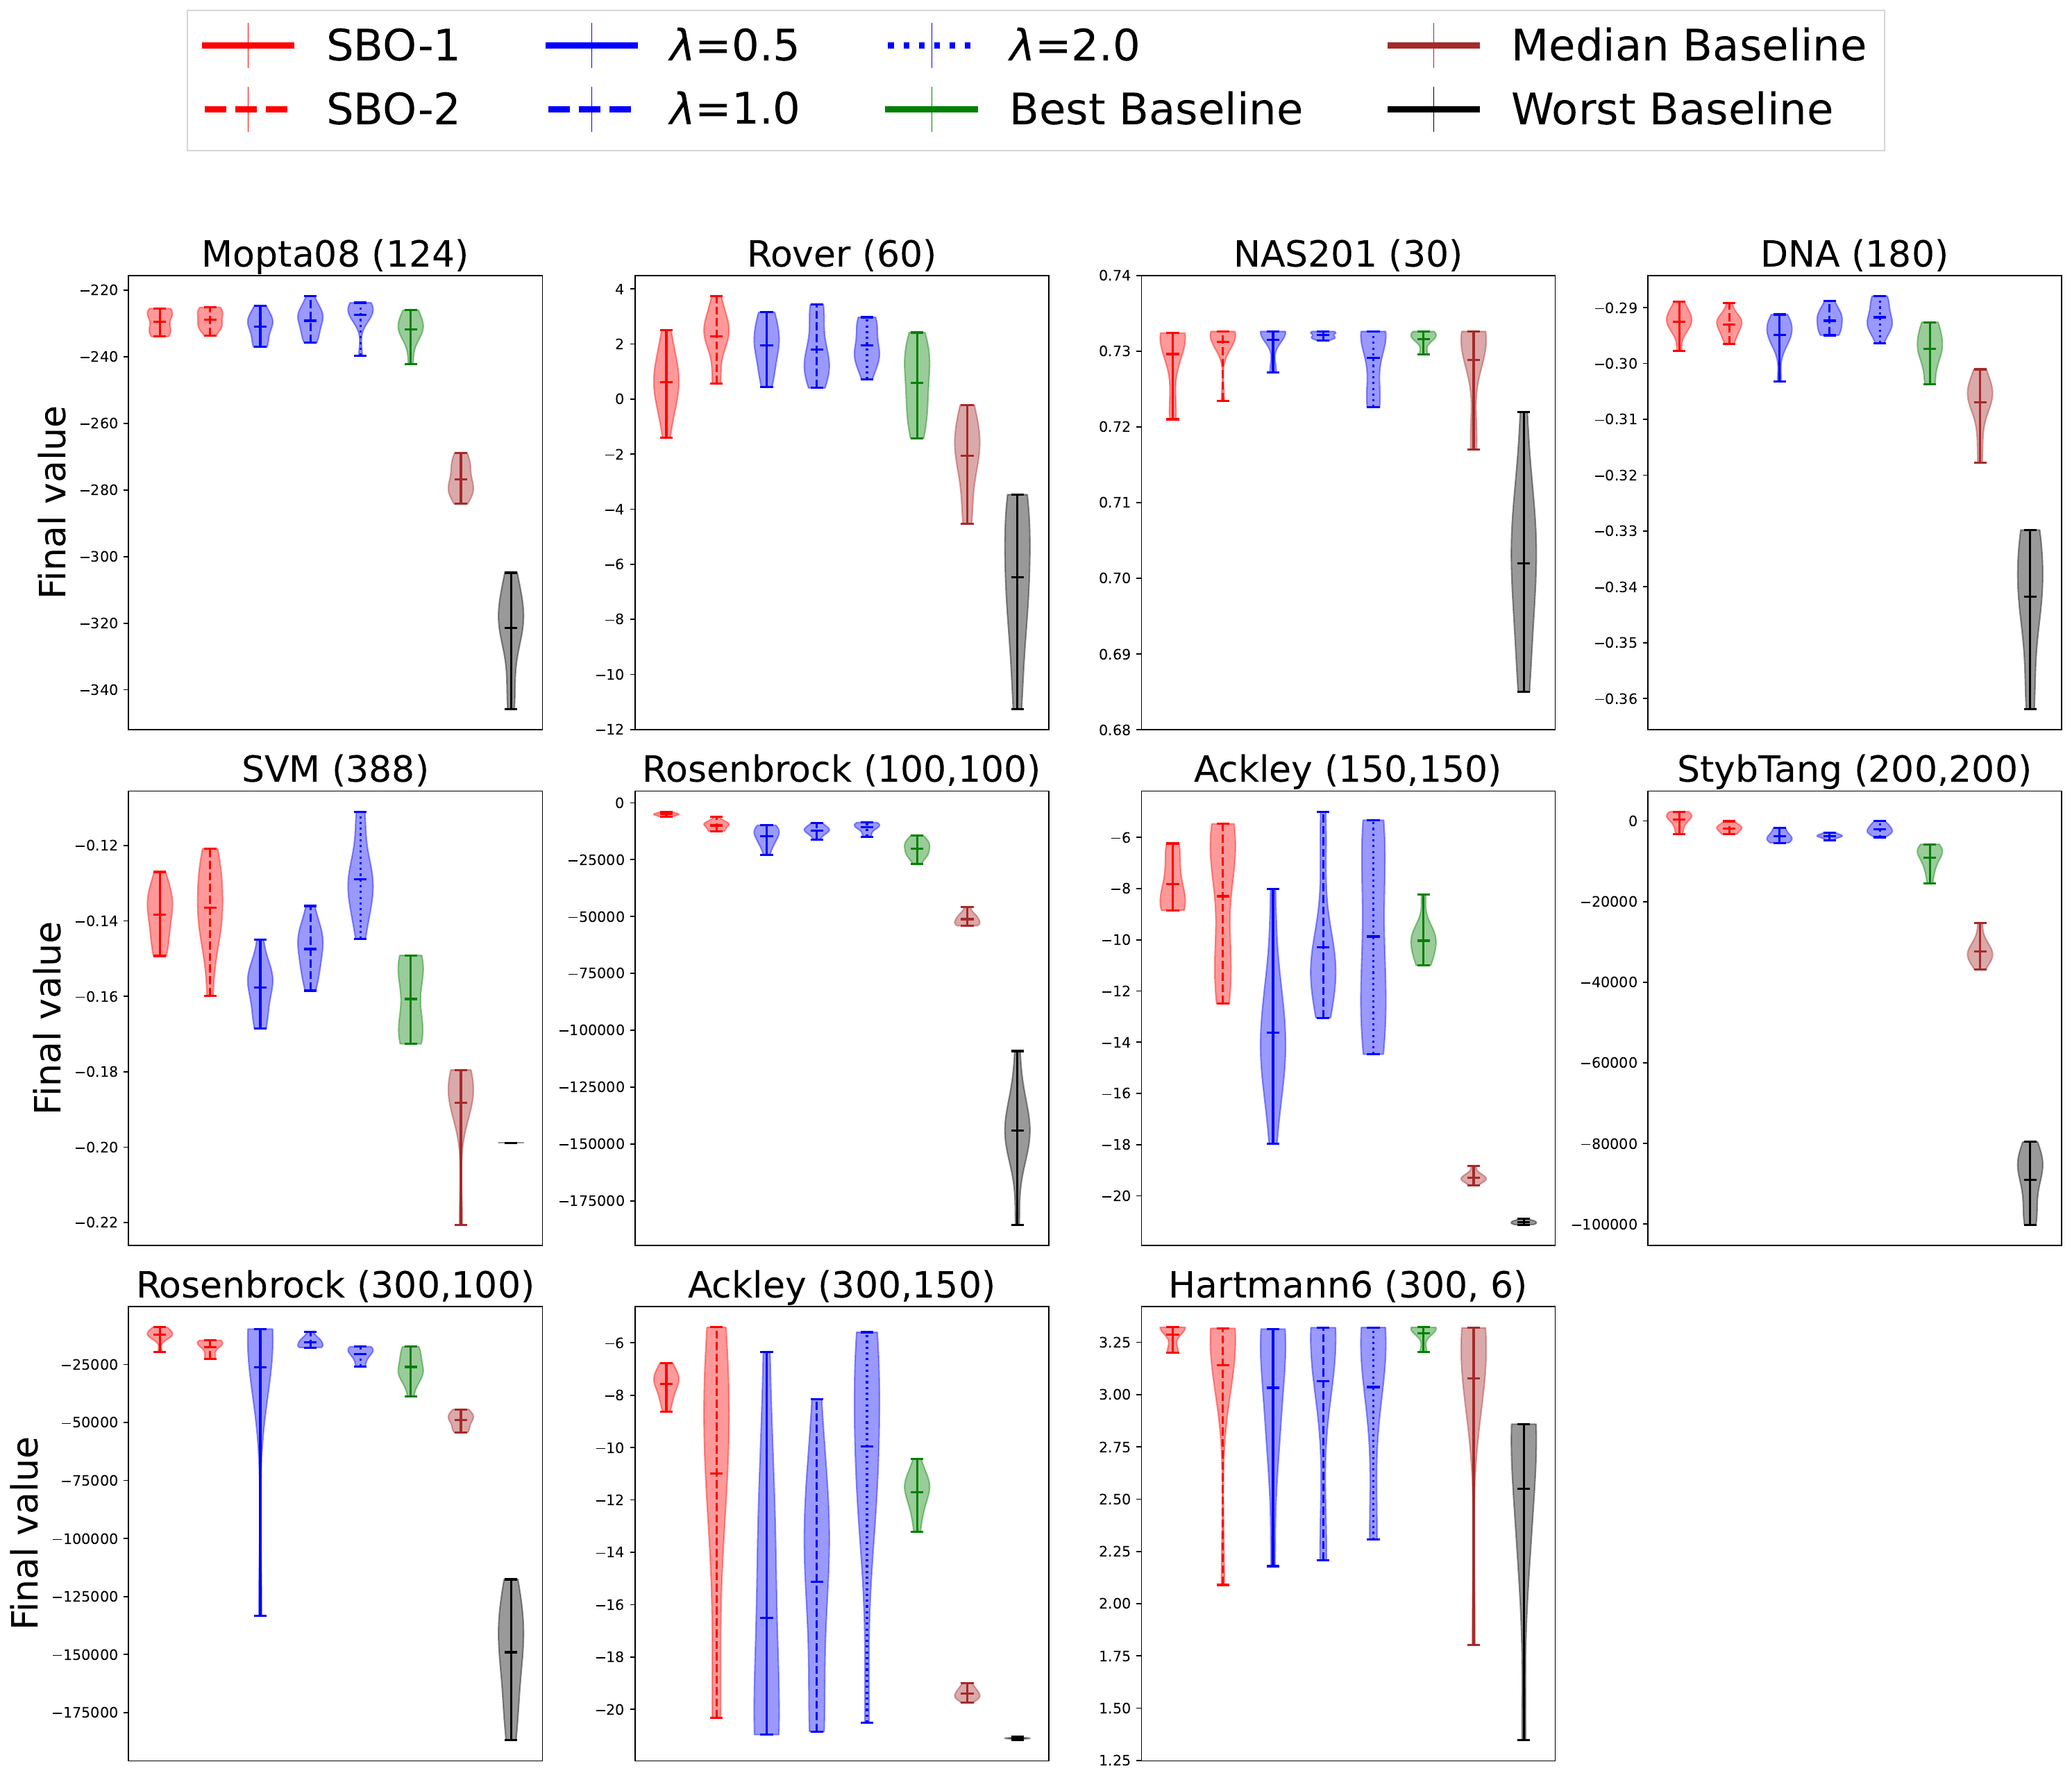}
    \caption{\small Ultimate optimization performance with different exploration level  $\lambda$ in UCB. Note that SBO-1 and SBO-2 use $\lambda=1.5$.
    \cmt{Maximum Function Value Obtained at the end of optimization loop. The results were collect from 10 runs. $\lambda$ varied from \{0.5, 1.0, 1.5, 2.0\}.}}
    \label{fig:final-lambda}
\end{figure*}
\begin{figure*}[!ht]
    \centering
    \includegraphics[width=\textwidth]{BO ICLR 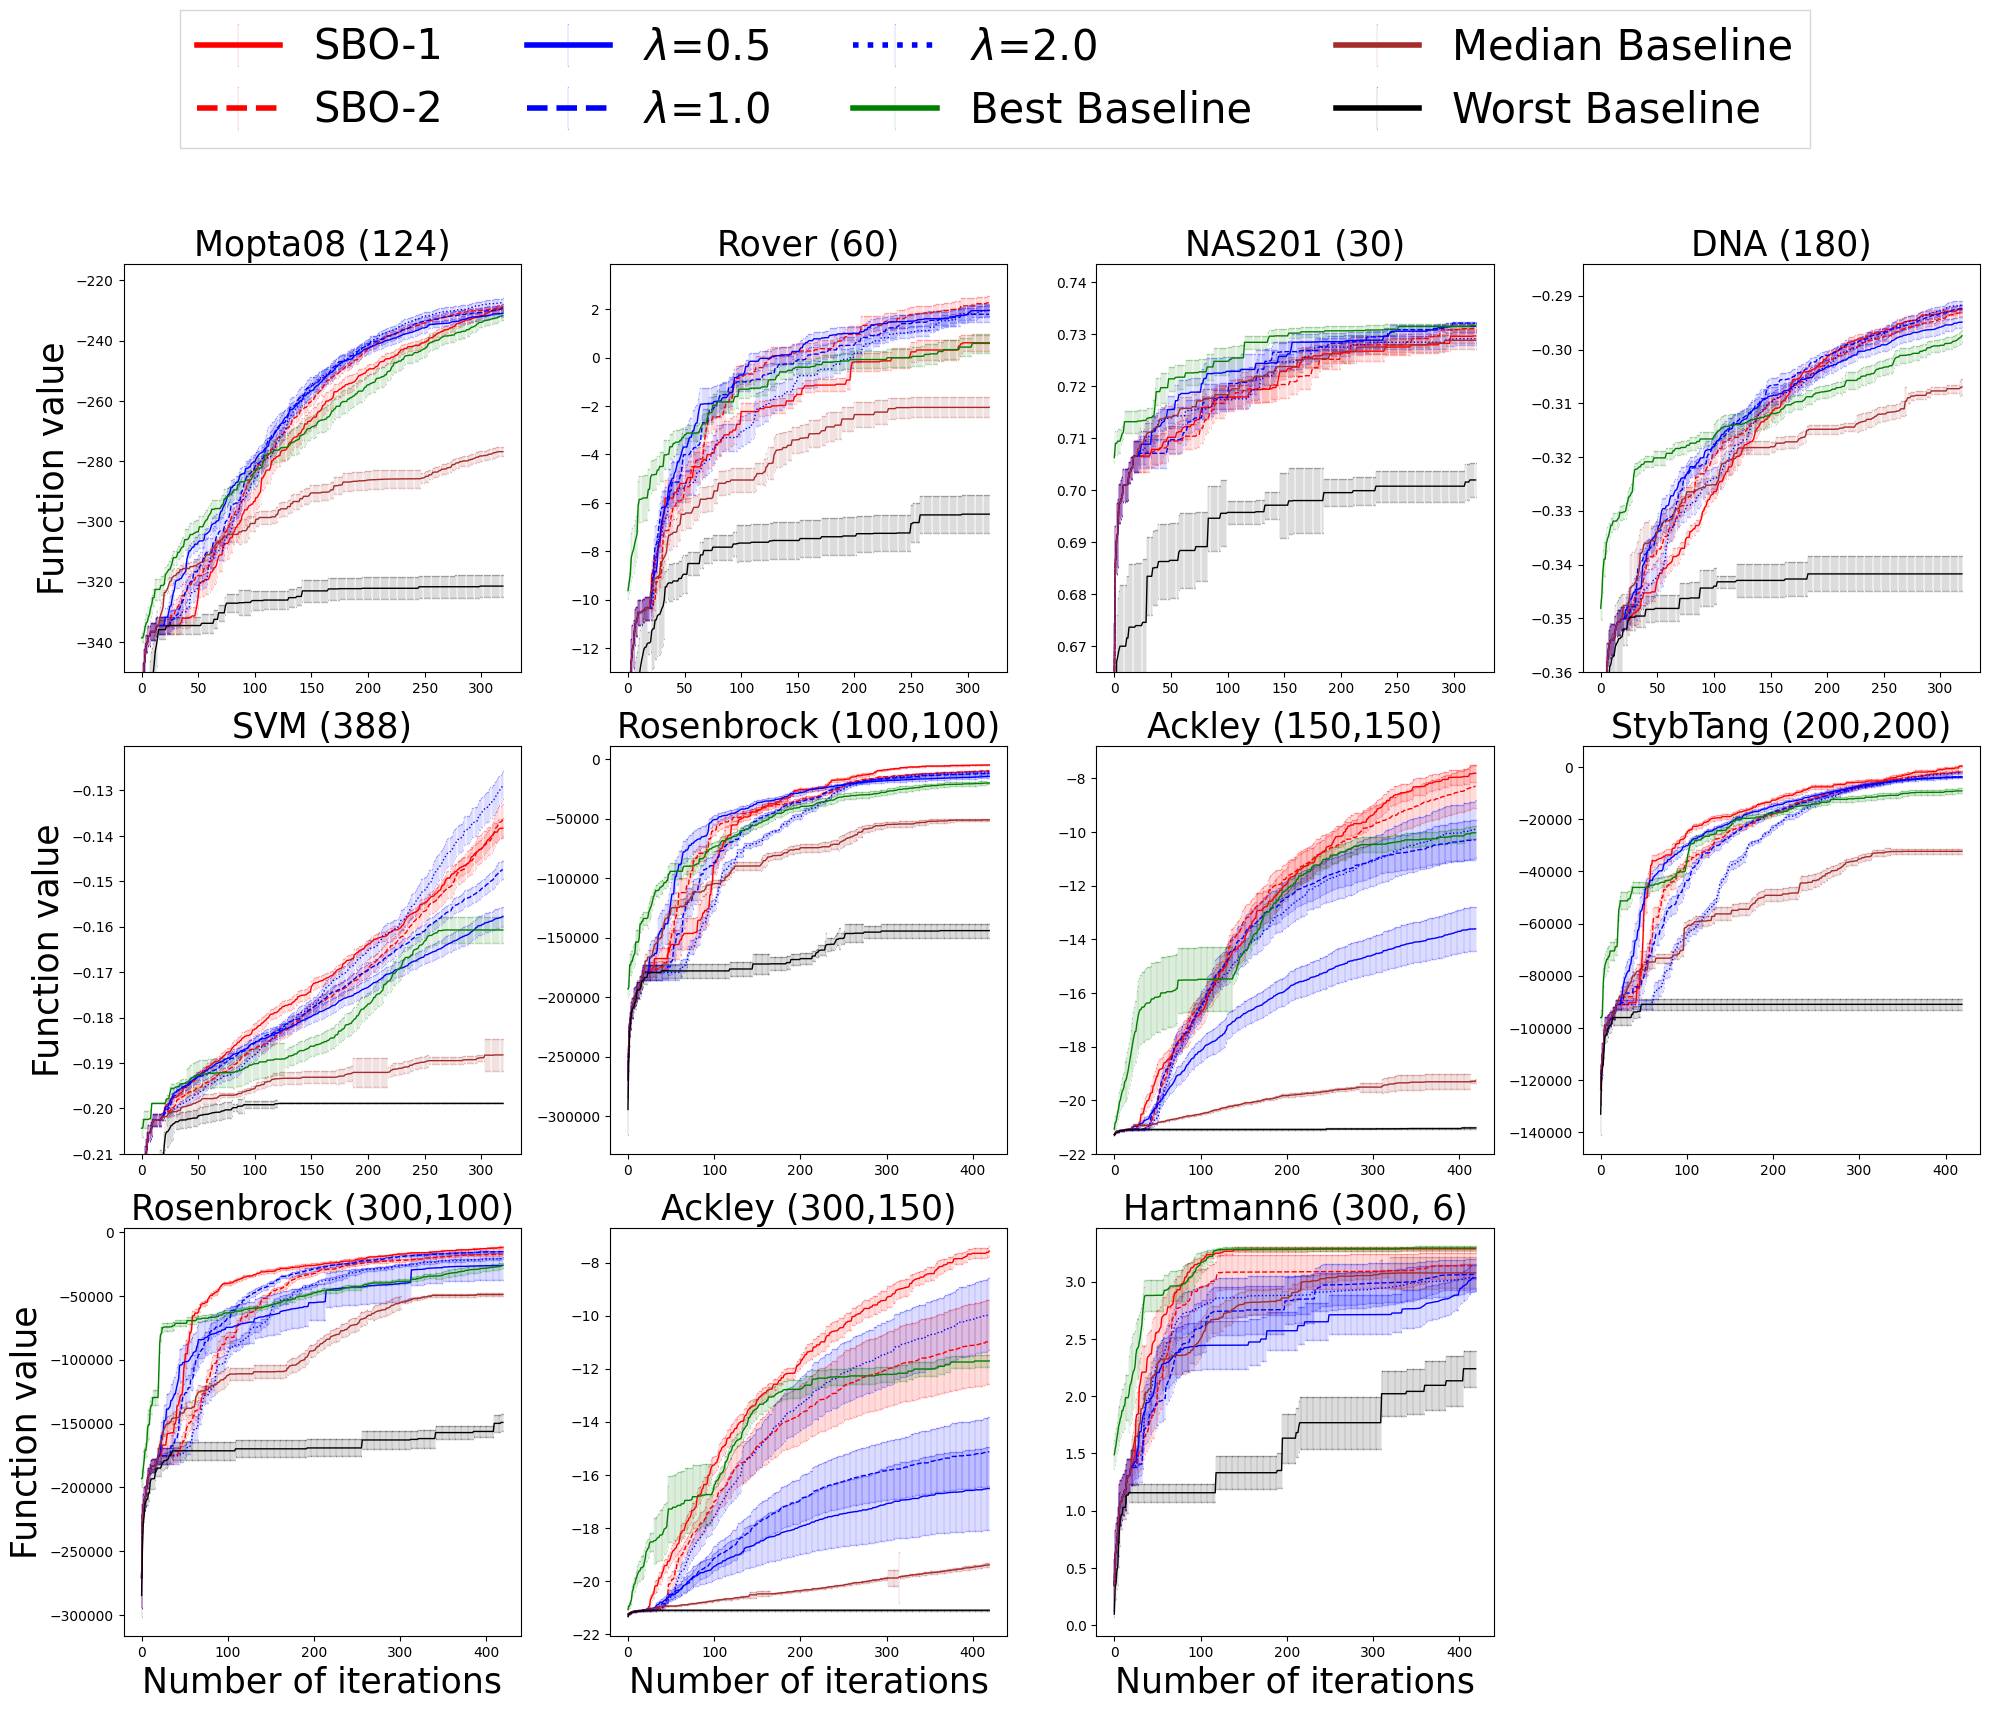}
    \caption{\small Runtime optimization performance with different exploration level  $\lambda$ in UCB. Note that SBO-1 and SBO-2 use $\lambda=1.5$. \cmt{Maximum Function Value Obtained at the end of optimization loop. The results were collect from 10 runs. $\lambda$ varied from \{0.5, 1.0, 1.5, 2.0\}.}}
    \label{fig:running-lambda}
\end{figure*}

\section{Limitation and Discussion}
\label{sec:limitation}
We evaluated Standard Bayesian Optimization on 5 real-world benchmarks and 6 synthetic functions that are most commonly used in previous HDBO works. We acknowledge that there are infinitely more  high-dimensional optimization problems that can be used for evaluation. In general, we hope after our work, future HDBO paper can include Standard BO with proper settings as their baseline methods. Hence, we can attain a better understanding about the potential of Standard BO in high dimensional functions. Moreover, we will seek for theoretical justifications and guarantees on SBO in high-dimensional settings.  We would like to also seek for a theoretical explanation of the failure modes. 
